# Supplementary material for: MSGCorep: A package for corepresentations of magnetic space groups
Source: arXiv:2211.10740 source file (2022-11-19)
Supplement: Supplementary file 1 [file msgcorep-SM.pdf]

# MSGCorep: A package for corepresentations of magnetic space groups

Gui-Bin Liu<sup>a,b,\*</sup>, Zeying Zhang<sup>c</sup>, Zhi-Ming Yu<sup>a,b</sup>, Yugui Yao<sup>a,b,†</sup>

<sup>a</sup>Centre for Quantum Physics, Key Laboratory of Advanced Optoelectronic Quantum Architecture and Measurement (MOE),  
School of Physics, Beijing Institute of Technology, Beijing 100081, China

<sup>b</sup>Beijing Key Laboratory of Nanophotonics and Ultrafine Optoelectronic Systems, School of Physics,  
Beijing Institute of Technology, Beijing 100081, China

<sup>c</sup>College of Mathematics and Physics, Beijing University of Chemical Technology, Beijing 100029, China

## Contents

|          |                                         |           |
|----------|-----------------------------------------|-----------|
| <b>1</b> | <b>Get help in the package MSGCorep</b> | <b>2</b>  |
| <b>2</b> | <b>Error message</b>                    | <b>3</b>  |
| <b>3</b> | <b>MSG numbers and symbols</b>          | <b>4</b>  |
| <b>4</b> | <b>MSG elements</b>                     | <b>35</b> |

---

\*Corresponding author: gbliu@bit.edu.cn

†Corresponding author: ygyao@bit.edu.cn

# 1 Get help in the package MSGCorep

Users can use `?` to browse all available functions in the `MSGCorep` package, to search functions whose names contain certain string via asterisk wildcard, and to get the help information of a specific function. Users can also use `Options` to know the available options of a function and their default values. Examples are shown as follow.

```
In[183]:= ? MSGCorep`*
```

▼ MSGCorep`

|                     |                       |                           |
|---------------------|-----------------------|---------------------------|
| BCTab7d2            | libMLGCorep           | showMLGCorep              |
| BNStoOG             | lookupMLGCorep        | showMPGCorep              |
| checkMLGCorep       | MagRotTimes           | showMPGCorepDirectProduct |
| checkMSGCorep       | MPGCorepDirectProduct | showMPGInfo               |
| DMagRotTimes        | MPGInfo               | showMSGCorep              |
| DMSGinvSeitz        | MSGCorepDirectProduct | showMSGCorepDirectProduct |
| DMSGpowerSeitz      | MSGinvSeitz           | showMSGSeitz              |
| DMSGSeitzTimes      | MSGpowerSeitz         | showMSGSym                |
| generateLibMLGCorep | MSGSeitzTimes         | type1MSGSymText           |
| getBandCorep        | MSGSymBC              | type1MSGSymTextBC         |
| getMagKStar         | MSGSymBNS             | type1num                  |
| getMLGCorep         | MSGSymOG              | type2MSGSymText           |
| getMLGCorepMat      | MSGSymStd             | type2MSGSymTextBC         |
| getMLGElem          | MSGSymText            | type2num                  |
| getMPGCorep         | MSGSymTextBC          | type3kpairDict            |
| getMPGElem          | MSGSymTextOG          | type3MSGSymText           |
| getMSGCorep         | MSGtype               | type3MSGSymTextBC         |
| getMSGCorepMat      | OGtoBNS               | type3nums                 |
| getMSGElem          | powerDMagRot          | type3USubInfo             |
| getMSGType          | powerMagRot           | type4AUTrans              |
| index2subSG         | readMagTrace          | type4MSGSymText           |
| invDMagRot          | showBandCorep         | type4MSGSymTextBC         |
| invMagRot           | showMagRot            | type4nums                 |

```
In[189]:= ? MSGCorep`*MLG*
```

▼ MSGCorep`

|                     |                |             |                |
|---------------------|----------------|-------------|----------------|
| checkMLGCorep       | getMLGCorep    | getMLGElem  | lookupMLGCorep |
| generateLibMLGCorep | getMLGCorepMat | libMLGCorep | showMLGCorep   |

```
In[190]:= ? getBandCorep
```

Three usages:

```
getBandCorep[{sgno,mno}, traceData, ikOrListOrSpan, ibOrListOrSpan]
```

```
getBandCorep[{sgno,mno}, traceData, ikOrListOrSpan]
```

```
getBandCorep[{sgno,mno}, traceData]
```

This function gives the magnetic–little–group coreps of the Bloch states for the  $k$  points specified by `ikOrListOrSpan` and bands specified by `ibOrListOrSpan`. If `ikOrListOrSpan` and `ibOrListOrSpan` are not specified, coreps of all  $k$  points and all bands are given. `traceData` is the result of `readMagTrace`. Note that the `trace.txt` file should be generated using a BC standard cell, or else the `traceData` may lead to errors of `getBandCorep`. Default options are "CompressDegeneracy"→True, "showdim"→True and "abcOrBasVec"→None. When numeric basic vectors or lattice constants are specified for "abcOrBasVec", the names of some high–symmetry  $k$  lines can be identified correctly.

```
In[192]:= Options[showMLGCorep]
Out[192]= {uNumeric → False, corep → All, elem → All, rotmat → True,
           trace → False, spin → downup, abcOrBasVec → None, linewidth → 2, maxDim → 4}
```

## 2 Error message

Most functions support error messages. When wrong inputs are received, functions will give hints for correct inputs. For example, when a wrong MSG number, such as {225, 3}, is input, functions such as **getMSGElem**, **getMLGElem**, **showMLGCorep**, and **showMSGCorep** will hint the right MSG numbers beginning with 225.

```
In[188]:= getMSGElem[{225, 3}]
getMSGElem: for MSG 225.num, num should be in {116, 117, {118, 119, 120}, {121}}.
Refer to:
```

|         |                      |     |
|---------|----------------------|-----|
| 225.116 | Fm $\bar{3}$ m       | I   |
| 225.117 | Fm $\bar{3}$ m1'     | II  |
| 225.118 | Fm' $\bar{3}$ 'm     | III |
| 225.119 | Fm $\bar{3}$ m'      | III |
| 225.120 | Fm' $\bar{3}$ 'm'    | III |
| 225.121 | F $_s$ m $\bar{3}$ m | IV  |

```
Out[188]=
$Aborted
```

Available k-point names are given when a wrong k-point name is input.

```
In[199]:= showMLGCorep[{225, 119}, "T"]
kBCCoord: kname T is not in { $\Gamma$ , X, L, W,  $\Delta$ ,  $\Lambda$ ,  $\Sigma$ , S, Z, Q}
Out[199]=
$Aborted
```

Available inputs for magnetic point groups are given when a wrong input is received.

```
In[222]:= getMPGElem[15]
getMPGElem: Use any item as input listed as follow:
{15, 1} "15.1" "15.1.53" "4/mmm"
{15, 2} "15.2" "15.2.54" "4/mmm1'"
{15, 3} "15.3" "15.3.55" "4/m'mm"
{15, 4} "15.4" "15.4.56" "4'/mm'm"
{15, 5} "15.5" "15.5.57" "4'/m'm'm"
{15, 6} "15.6" "15.6.58" "4/mm'm'"
{15, 7} "15.7" "15.7.59" "4/m'm'm'"
Out[222]=
$Aborted
```

### 3 MSG numbers and symbols

Users can use `showMSGSym[family]` to show the correspondence between BNS and OG notations for the MSGs specified by `family`. Here `family` can be an integer for the MSG family number in the range [1,230], a list of integers or a span for the family numbers. By default, the family numbers are shown in BNS order, but they will be shown in OG order if the option "`family`" $\rightarrow$ "OG" is used. The BNS symbols in BC orientation are also shown for comparison if they are different from the standard BNS symbols, but if they are the same with the standard BNS symbols only right arrows are shown meaning "the same with the left". In the following two examples, `showMSGSym[1;;5]` shows the MSGs with the BNS family numbers from 1 to 5, and `showMSGSym[5,"family" $\rightarrow$ "OG"]` shows the MSGs with the OG family number 5. If `family` is omitted, running `showMSGSym[]` will show all the 1651 MSGs, and output information is the same with Table S1.

In[223]:= `showMSGSym[1 ;; 5]`

Out[223]=

| BNS<br>Number | BNS<br>Symbol                 | BNS (BC)<br>Symbol            | OG<br>Number | OG<br>Symbol                   | Type |
|---------------|-------------------------------|-------------------------------|--------------|--------------------------------|------|
| 1.1           | P1                            | $\leftarrow$                  | 1.1.1        | P1                             | I    |
| 1.2           | P11'                          | $\leftarrow$                  | 1.2.2        | P11'                           | II   |
| 1.3           | P <sub>s</sub> 1              | $\leftarrow$                  | 1.3.3        | P <sub>2s</sub> 1              | IV   |
| 2.4           | P $\bar{1}$                   | $\leftarrow$                  | 2.1.4        | P $\bar{1}$                    | I    |
| 2.5           | P $\bar{1}$ 1'                | $\leftarrow$                  | 2.2.5        | P $\bar{1}$ 1'                 | II   |
| 2.6           | P $\bar{1}$ '                 | $\leftarrow$                  | 2.3.6        | P $\bar{1}$ '                  | III  |
| 2.7           | P <sub>s</sub> $\bar{1}$      | $\leftarrow$                  | 2.4.7        | P <sub>2s</sub> $\bar{1}$      | IV   |
| 3.1           | P2                            | $\leftarrow$                  | 3.1.8        | P2                             | I    |
| 3.2           | P21'                          | $\leftarrow$                  | 3.2.9        | P21'                           | II   |
| 3.3           | P2'                           | $\leftarrow$                  | 3.3.10       | P2'                            | III  |
| 3.4           | P <sub>a</sub> 2              | $\leftarrow$                  | 3.4.11       | P <sub>2a</sub> 2              | IV   |
| 3.5           | P <sub>b</sub> 2              | P <sub>c</sub> 2              | 3.5.12       | P <sub>2b</sub> 2              | IV   |
| 3.6           | P <sub>c</sub> 2              | P <sub>B</sub> 2              | 5.5.23       | C <sub>p</sub> 2               | IV   |
| 4.7           | P2 <sub>1</sub>               | $\leftarrow$                  | 4.1.15       | P2 <sub>1</sub>                | I    |
| 4.8           | P2 <sub>1</sub> 1'            | $\leftarrow$                  | 4.2.16       | P2 <sub>1</sub> 1'             | II   |
| 4.9           | P2 <sub>1</sub> '             | $\leftarrow$                  | 4.3.17       | P2 <sub>1</sub> '              | III  |
| 4.10          | P <sub>a</sub> 2 <sub>1</sub> | $\leftarrow$                  | 4.4.18       | P <sub>2a</sub> 2 <sub>1</sub> | IV   |
| 4.11          | P <sub>b</sub> 2 <sub>1</sub> | P <sub>c</sub> 2 <sub>1</sub> | 3.7.14       | P <sub>2b</sub> 2'             | IV   |
| 4.12          | P <sub>c</sub> 2 <sub>1</sub> | P <sub>B</sub> 2 <sub>1</sub> | 5.6.24       | C <sub>p</sub> 2'              | IV   |
| 5.13          | C2                            | B2                            | 5.1.19       | C2                             | I    |
| 5.14          | C21'                          | B21'                          | 5.2.20       | C21'                           | II   |
| 5.15          | C2'                           | B2'                           | 5.3.21       | C2'                            | III  |
| 5.16          | C <sub>c</sub> 2              | B <sub>b</sub> 2              | 5.4.22       | C <sub>2c</sub> 2              | IV   |
| 5.17          | C <sub>a</sub> 2              | B <sub>a</sub> 2              | 3.6.13       | P <sub>c</sub> 2               | IV   |

In[224]:= `showMSGSym[5, "family"  $\rightarrow$  "OG"]`

Out[224]=

| OG<br>Number | OG<br>Symbol      | BNS<br>Number | BNS<br>Symbol                 | BNS (BC)<br>Symbol            | Type |
|--------------|-------------------|---------------|-------------------------------|-------------------------------|------|
| 5.1.19       | C2                | 5.13          | C2                            | B2                            | I    |
| 5.2.20       | C21'              | 5.14          | C21'                          | B21'                          | II   |
| 5.3.21       | C2'               | 5.15          | C2'                           | B2'                           | III  |
| 5.4.22       | C <sub>2c</sub> 2 | 5.16          | C <sub>c</sub> 2              | B <sub>b</sub> 2              | IV   |
| 5.5.23       | C <sub>p</sub> 2  | 3.6           | P <sub>c</sub> 2              | P <sub>B</sub> 2              | IV   |
| 5.6.24       | C <sub>p</sub> 2' | 4.12          | P <sub>c</sub> 2 <sub>1</sub> | P <sub>B</sub> 2 <sub>1</sub> | IV   |

Table S1: List of both BNS and OG notations for MSGs.

| BNS Number | BNS Symbol   | BNS (BC) Symbol | OG Number | OG Symbol       | Type |
|------------|--------------|-----------------|-----------|-----------------|------|
| 1.1        | $P1$         | $\leftarrow$    | 1.1.1     | $P1$            | I    |
| 1.2        | $P11'$       | $\leftarrow$    | 1.2.2     | $P11'$          | II   |
| 1.3        | $P_s1$       | $\leftarrow$    | 1.3.3     | $P_{2s}1$       | IV   |
| 2.4        | $P1$         | $\leftarrow$    | 2.1.4     | $P1$            | I    |
| 2.5        | $P\bar{1}1'$ | $\leftarrow$    | 2.2.5     | $P\bar{1}1'$    | II   |
| 2.6        | $P\bar{1}'$  | $\leftarrow$    | 2.3.6     | $P\bar{1}'$     | III  |
| 2.7        | $P_s\bar{1}$ | $\leftarrow$    | 2.4.7     | $P_{2s}\bar{1}$ | IV   |
| 3.1        | $P2$         | $\leftarrow$    | 3.1.8     | $P2$            | I    |
| 3.2        | $P21'$       | $\leftarrow$    | 3.2.9     | $P21'$          | II   |
| 3.3        | $P2'$        | $\leftarrow$    | 3.3.10    | $P2'$           | III  |
| 3.4        | $P_a2$       | $\leftarrow$    | 3.4.11    | $P_{2a}2$       | IV   |
| 3.5        | $P_b2$       | $P_c2$          | 3.5.12    | $P_{2b}2$       | IV   |
| 3.6        | $P_C2$       | $P_B2$          | 5.5.23    | $C_P2$          | IV   |
| 4.7        | $P2_1$       | $\leftarrow$    | 4.1.15    | $P2_1$          | I    |
| 4.8        | $P2_11'$     | $\leftarrow$    | 4.2.16    | $P2_11'$        | II   |
| 4.9        | $P2'_1$      | $\leftarrow$    | 4.3.17    | $P2'_1$         | III  |
| 4.10       | $P_a2_1$     | $\leftarrow$    | 4.4.18    | $P_{2a}2_1$     | IV   |
| 4.11       | $P_b2_1$     | $P_c2_1$        | 3.7.14    | $P_{2b}2'$      | IV   |
| 4.12       | $P_C2_1$     | $P_B2_1$        | 5.6.24    | $C_P2'$         | IV   |
| 5.13       | $C2$         | $B2$            | 5.1.19    | $C2$            | I    |
| 5.14       | $C21'$       | $B21'$          | 5.2.20    | $C21'$          | II   |
| 5.15       | $C2'$        | $B2'$           | 5.3.21    | $C2'$           | III  |
| 5.16       | $C_c2$       | $B_b2$          | 5.4.22    | $C_{2c}2$       | IV   |
| 5.17       | $C_a2$       | $B_a2$          | 3.6.13    | $P_C2$          | IV   |
| 6.18       | $Pm$         | $\leftarrow$    | 6.1.25    | $Pm$            | I    |
| 6.19       | $Pm1'$       | $\leftarrow$    | 6.2.26    | $Pm1'$          | II   |
| 6.20       | $Pm'$        | $\leftarrow$    | 6.3.27    | $Pm'$           | III  |
| 6.21       | $P_am$       | $\leftarrow$    | 6.4.28    | $P_{2a}m$       | IV   |
| 6.22       | $P_bm$       | $P_cm$          | 6.5.29    | $P_{2b}m$       | IV   |
| 6.23       | $P_Cm$       | $P_Bm$          | 8.5.42    | $C_Pm$          | IV   |
| 7.24       | $Pc$         | $Pb$            | 7.1.32    | $Pc$            | I    |
| 7.25       | $Pc1'$       | $Pb1'$          | 7.2.33    | $Pc1'$          | II   |
| 7.26       | $Pc'$        | $Pb'$           | 7.3.34    | $Pc'$           | III  |
| 7.27       | $P_ac$       | $P_ab$          | 7.4.35    | $P_{2a}c$       | IV   |
| 7.28       | $P_cc$       | $P_bb$          | 6.7.31    | $P_{2c}m'$      | IV   |
| 7.29       | $P_bc$       | $P_cb$          | 7.5.36    | $P_{2b}c$       | IV   |
| 7.30       | $P_Cc$       | $P_Bb$          | 9.4.48    | $C_Pc$          | IV   |
| 7.31       | $P_{Ac}$     | $P_{Ab}$        | 8.7.44    | $C_Pm'$         | IV   |
| 8.32       | $Cm$         | $Bm$            | 8.1.38    | $Cm$            | I    |
| 8.33       | $Cm1'$       | $Bm1'$          | 8.2.39    | $Cm1'$          | II   |
| 8.34       | $Cm'$        | $Bm'$           | 8.3.40    | $Cm'$           | III  |
| 8.35       | $C_cm$       | $B_bm$          | 8.4.41    | $C_{2c}m$       | IV   |
| 8.36       | $C_am$       | $B_am$          | 6.6.30    | $P_Cm$          | IV   |
| 9.37       | $Cc$         | $Bb$            | 9.1.45    | $Cc$            | I    |
| 9.38       | $Cc1'$       | $Bb1'$          | 9.2.46    | $Cc1'$          | II   |
| 9.39       | $Cc'$        | $Bb'$           | 9.3.47    | $Cc'$           | III  |
| 9.40       | $C_cc$       | $B_bb$          | 8.6.43    | $C_{2c}m'$      | IV   |
| 9.41       | $C_ac$       | $B_ab$          | 7.6.37    | $P_Cc$          | IV   |
| 10.42      | $P2/m$       | $\leftarrow$    | 10.1.49   | $P2/m$          | I    |
| 10.43      | $P2/m1'$     | $\leftarrow$    | 10.2.50   | $P2/m1'$        | II   |
| 10.44      | $P2'/m$      | $\leftarrow$    | 10.3.51   | $P2'/m$         | III  |
| 10.45      | $P2/m'$      | $\leftarrow$    | 10.4.52   | $P2/m'$         | III  |
| 10.46      | $P2'/m'$     | $\leftarrow$    | 10.5.53   | $P2'/m'$        | III  |
| 10.47      | $P_a2/m$     | $\leftarrow$    | 10.6.54   | $P_{2a}2/m$     | IV   |
| 10.48      | $P_b2/m$     | $P_c2/m$        | 10.7.55   | $P_{2b}2/m$     | IV   |

| BNS<br>Number | BNS<br>Symbol | BNS (BC)<br>Symbol | OG<br>Number | OG<br>Symbol   | Type |
|---------------|---------------|--------------------|--------------|----------------|------|
| 10.49         | $P_C2/m$      | $P_B2/m$           | 12.7.72      | $C_P2/m$       | IV   |
| 11.50         | $P2_1/m$      | $\leftarrow$       | 11.1.59      | $P2_1/m$       | I    |
| 11.51         | $P2_1/m1'$    | $\leftarrow$       | 11.2.60      | $P2_1/m1'$     | II   |
| 11.52         | $P2'_1/m$     | $\leftarrow$       | 11.3.61      | $P2'_1/m$      | III  |
| 11.53         | $P2_1/m'$     | $\leftarrow$       | 11.4.62      | $P2_1/m'$      | III  |
| 11.54         | $P2'_1/m'$    | $\leftarrow$       | 11.5.63      | $P2'_1/m'$     | III  |
| 11.55         | $P_a2_1/m$    | $\leftarrow$       | 11.6.64      | $P_{2a}2_1/m$  | IV   |
| 11.56         | $P_b2_1/m$    | $P_c2_1/m$         | 10.9.57      | $P_{2b}2'/m$   | IV   |
| 11.57         | $P_C2_1/m$    | $P_B2_1/m$         | 12.9.74      | $C_P2'/m$      | IV   |
| 12.58         | $C2/m$        | $B2/m$             | 12.1.66      | $C2/m$         | I    |
| 12.59         | $C2/m1'$      | $B2/m1'$           | 12.2.67      | $C2/m1'$       | II   |
| 12.60         | $C2'/m$       | $B2'/m$            | 12.3.68      | $C2'/m$        | III  |
| 12.61         | $C2/m'$       | $B2/m'$            | 12.4.69      | $C2/m'$        | III  |
| 12.62         | $C2'/m'$      | $B2'/m'$           | 12.5.70      | $C2'/m'$       | III  |
| 12.63         | $C_c2/m$      | $B_b2/m$           | 12.6.71      | $C_{2c}2/m$    | IV   |
| 12.64         | $C_a2/m$      | $B_a2/m$           | 10.8.56      | $P_C2/m$       | IV   |
| 13.65         | $P2/c$        | $P2/b$             | 13.1.77      | $P2/c$         | I    |
| 13.66         | $P2/c1'$      | $P2/b1'$           | 13.2.78      | $P2/c1'$       | II   |
| 13.67         | $P2'/c$       | $P2'/b$            | 13.3.79      | $P2'/c$        | III  |
| 13.68         | $P2/c'$       | $P2/b'$            | 13.4.80      | $P2/c'$        | III  |
| 13.69         | $P2'/c'$      | $P2'/b'$           | 13.5.81      | $P2'/c'$       | III  |
| 13.70         | $P_a2/c$      | $P_a2/b$           | 13.6.82      | $P_{2a}2/c$    | IV   |
| 13.71         | $P_b2/c$      | $P_c2/b$           | 13.7.83      | $P_{2b}2/c$    | IV   |
| 13.72         | $P_c2/c$      | $P_b2/b$           | 10.10.58     | $P_{2c}2/m'$   | IV   |
| 13.73         | $P_A2/c$      | $P_A2/b$           | 12.10.75     | $C_P2/m'$      | IV   |
| 13.74         | $P_C2/c$      | $P_B2/b$           | 15.6.97      | $C_P2/c$       | IV   |
| 14.75         | $P2_1/c$      | $P2_1/b$           | 14.1.86      | $P2_1/c$       | I    |
| 14.76         | $P2_1/c1'$    | $P2_1/b1'$         | 14.2.87      | $P2_1/c1'$     | II   |
| 14.77         | $P2'_1/c$     | $P2'_1/b$          | 14.3.88      | $P2'_1/c$      | III  |
| 14.78         | $P2_1/c'$     | $P2_1/b'$          | 14.4.89      | $P2_1/c'$      | III  |
| 14.79         | $P2'_1/c'$    | $P2'_1/b'$         | 14.5.90      | $P2'_1/c'$     | III  |
| 14.80         | $P_a2_1/c$    | $P_a2_1/b$         | 14.6.91      | $P_{2a}2_1/c$  | IV   |
| 14.81         | $P_b2_1/c$    | $P_c2_1/b$         | 13.9.85      | $P_{2b}2'/c$   | IV   |
| 14.82         | $P_c2_1/c$    | $P_b2_1/b$         | 11.7.65      | $P_{2c}2_1/m'$ | IV   |
| 14.83         | $P_A2_1/c$    | $P_A2_1/b$         | 12.11.76     | $C_P2'/m'$     | IV   |
| 14.84         | $P_C2_1/c$    | $P_B2_1/b$         | 15.7.98      | $C_P2'/c$      | IV   |
| 15.85         | $C2/c$        | $B2/b$             | 15.1.92      | $C2/c$         | I    |
| 15.86         | $C2/c1'$      | $B2/b1'$           | 15.2.93      | $C2/c1'$       | II   |
| 15.87         | $C2'/c$       | $B2'/b$            | 15.3.94      | $C2'/c$        | III  |
| 15.88         | $C2/c'$       | $B2/b'$            | 15.4.95      | $C2/c'$        | III  |
| 15.89         | $C2'/c'$      | $B2'/b'$           | 15.5.96      | $C2'/c'$       | III  |
| 15.90         | $C_c2/c$      | $B_b2/b$           | 12.8.73      | $C_{2c}2/m'$   | IV   |
| 15.91         | $C_a2/c$      | $B_a2/b$           | 13.8.84      | $P_C2/c$       | IV   |
| 16.1          | $P222$        | $\leftarrow$       | 16.1.99      | $P222$         | I    |
| 16.2          | $P2221'$      | $\leftarrow$       | 16.2.100     | $P2221'$       | II   |
| 16.3          | $P2'2'2$      | $\leftarrow$       | 16.3.101     | $P2'2'2$       | III  |
| 16.4          | $P_a222$      | $\leftarrow$       | 16.4.102     | $P_{2a}222$    | IV   |
| 16.5          | $P_C222$      | $\leftarrow$       | 21.6.134     | $C_P222$       | IV   |
| 16.6          | $P_I222$      | $\leftarrow$       | 23.4.148     | $I_P222$       | IV   |
| 17.7          | $P222_1$      | $\leftarrow$       | 17.1.106     | $P222_1$       | I    |
| 17.8          | $P222_11'$    | $\leftarrow$       | 17.2.107     | $P222_11'$     | II   |
| 17.9          | $P2'2'2_1$    | $\leftarrow$       | 17.3.108     | $P2'2'2_1$     | III  |
| 17.10         | $P22'2'_1$    | $\leftarrow$       | 17.4.109     | $P22'2'_1$     | III  |
| 17.11         | $P_a222_1$    | $\leftarrow$       | 17.5.110     | $P_{2a}222_1$  | IV   |
| 17.12         | $P_c222_1$    | $\leftarrow$       | 16.7.105     | $P_{2c}22'2'$  | IV   |

| BNS<br>Number | BNS<br>Symbol   | BNS (BC)<br>Symbol | OG<br>Number | OG<br>Symbol      | Type |
|---------------|-----------------|--------------------|--------------|-------------------|------|
| 17.13         | $P_A222_1$      | $\leftarrow$       | 21.10.138    | $C_P22'2'$        | IV   |
| 17.14         | $P_C222_1$      | $\leftarrow$       | 20.5.126     | $C_P222_1$        | IV   |
| 17.15         | $P_I222_1$      | $\leftarrow$       | 24.5.154     | $I_P2'_12'_12_1$  | IV   |
| 18.16         | $P2_12_12$      | $\leftarrow$       | 18.1.113     | $P2_12_12$        | I    |
| 18.17         | $P2_12_121'$    | $\leftarrow$       | 18.2.114     | $P2_12_121'$      | II   |
| 18.18         | $P2'_12'_12$    | $\leftarrow$       | 18.3.115     | $P2'_12'_12$      | III  |
| 18.19         | $P2_12'_12'$    | $\leftarrow$       | 18.4.116     | $P2_12'_12'$      | III  |
| 18.20         | $P_a2_12_12$    | $\leftarrow$       | 17.7.112     | $P_{2a}2'2'2_1$   | IV   |
| 18.21         | $P_c2_12_12$    | $\leftarrow$       | 18.5.117     | $P_{2c}2_12_12$   | IV   |
| 18.22         | $P_A2_12_12$    | $\leftarrow$       | 20.7.128     | $C_P22'2'_1$      | IV   |
| 18.23         | $P_C2_12_12$    | $\leftarrow$       | 21.9.137     | $C_P2'2'2$        | IV   |
| 18.24         | $P_I2_12_12$    | $\leftarrow$       | 23.5.149     | $I_P2'2'2$        | IV   |
| 19.25         | $P2_12_12_1$    | $\leftarrow$       | 19.1.119     | $P2_12_12_1$      | I    |
| 19.26         | $P2_12_12_11'$  | $\leftarrow$       | 19.2.120     | $P2_12_12_11'$    | II   |
| 19.27         | $P2'_12'_12_1$  | $\leftarrow$       | 19.3.121     | $P2'_12'_12_1$    | III  |
| 19.28         | $P_a2_12_12_1$  | $\leftarrow$       | 18.6.118     | $P_{2c}2_12'_12'$ | IV   |
| 19.29         | $P_C2_12_12_1$  | $\leftarrow$       | 20.6.127     | $C_P2'2'2_1$      | IV   |
| 19.30         | $P_I2_12_12_1$  | $\leftarrow$       | 24.4.153     | $I_P2_12_12_1$    | IV   |
| 20.31         | $C'222_1$       | $\leftarrow$       | 20.1.122     | $C'222_1$         | I    |
| 20.32         | $C'222_11'$     | $\leftarrow$       | 20.2.123     | $C'222_11'$       | II   |
| 20.33         | $C'2'2'2_1$     | $\leftarrow$       | 20.3.124     | $C'2'2'2_1$       | III  |
| 20.34         | $C'22'2'_1$     | $\leftarrow$       | 20.4.125     | $C'22'2'_1$       | III  |
| 20.35         | $C_c222_1$      | $\leftarrow$       | 21.8.136     | $C_{2c}22'2'$     | IV   |
| 20.36         | $C_a222_1$      | $\leftarrow$       | 17.6.111     | $P_C222_1$        | IV   |
| 20.37         | $C_A222_1$      | $\leftarrow$       | 22.5.144     | $F_C22'2'$        | IV   |
| 21.38         | $C'222$         | $\leftarrow$       | 21.1.129     | $C'222$           | I    |
| 21.39         | $C'2221'$       | $\leftarrow$       | 21.2.130     | $C'2221'$         | II   |
| 21.40         | $C'2'2'2$       | $\leftarrow$       | 21.3.131     | $C'2'2'2$         | III  |
| 21.41         | $C'22'2'$       | $\leftarrow$       | 21.4.132     | $C'22'2'$         | III  |
| 21.42         | $C_c222$        | $\leftarrow$       | 21.5.133     | $C_{2c}222$       | IV   |
| 21.43         | $C_a222$        | $\leftarrow$       | 16.5.103     | $P_C222$          | IV   |
| 21.44         | $C_A222$        | $\leftarrow$       | 22.4.143     | $F_C222$          | IV   |
| 22.45         | $F'222$         | $\leftarrow$       | 22.1.140     | $F'222$           | I    |
| 22.46         | $F'2221'$       | $\leftarrow$       | 22.2.141     | $F'2221'$         | II   |
| 22.47         | $F'2'2'2$       | $\leftarrow$       | 22.3.142     | $F'2'2'2$         | III  |
| 22.48         | $F_s222$        | $\leftarrow$       | 16.6.104     | $P_F222$          | IV   |
| 23.49         | $I'222$         | $\leftarrow$       | 23.1.145     | $I'222$           | I    |
| 23.50         | $I'2221'$       | $\leftarrow$       | 23.2.146     | $I'2221'$         | II   |
| 23.51         | $I'2'2'2$       | $\leftarrow$       | 23.3.147     | $I'2'2'2$         | III  |
| 23.52         | $I_c222$        | $\leftarrow$       | 21.7.135     | $C_I222$          | IV   |
| 24.53         | $I'2_12_12_1$   | $\leftarrow$       | 24.1.150     | $I'2_12_12_1$     | I    |
| 24.54         | $I'2_12_12_11'$ | $\leftarrow$       | 24.2.151     | $I'2_12_12_11'$   | II   |
| 24.55         | $I'2'_12'_12_1$ | $\leftarrow$       | 24.3.152     | $I'2'_12'_12_1$   | III  |
| 24.56         | $I_c2_12_12_1$  | $\leftarrow$       | 21.11.139    | $C_I2'2'22'$      | IV   |
| 25.57         | $Pmm2$          | $\leftarrow$       | 25.1.155     | $Pmm2$            | I    |
| 25.58         | $Pmm21'$        | $\leftarrow$       | 25.2.156     | $Pmm21'$          | II   |
| 25.59         | $Pm'm'2'$       | $\leftarrow$       | 25.3.157     | $Pm'm'2'$         | III  |
| 25.60         | $Pm'm'2$        | $\leftarrow$       | 25.4.158     | $Pm'm'2$          | III  |
| 25.61         | $P_cmm2$        | $\leftarrow$       | 25.5.159     | $P_{2c}mm2$       | IV   |
| 25.62         | $P_a2mm2$       | $\leftarrow$       | 25.6.160     | $P_{2a}mm2$       | IV   |
| 25.63         | $P_Cmm2$        | $\leftarrow$       | 35.6.241     | $C_Pmm2$          | IV   |
| 25.64         | $P_Amm2$        | $\leftarrow$       | 38.7.271     | $A_Pmm2$          | IV   |
| 25.65         | $P_Imm2$        | $\leftarrow$       | 44.5.328     | $I_Pmm2$          | IV   |
| 26.66         | $Pmc2_1$        | $\leftarrow$       | 26.1.168     | $Pmc2_1$          | I    |
| 26.67         | $Pmc2_11'$      | $\leftarrow$       | 26.2.169     | $Pmc2_11'$        | II   |

| BNS<br>Number | BNS<br>Symbol | BNS (BC)<br>Symbol | OG<br>Number | OG<br>Symbol     | Type |
|---------------|---------------|--------------------|--------------|------------------|------|
| 26.68         | $Pm'c2'_1$    | $\leftarrow$       | 26.3.170     | $Pm'c2'_1$       | III  |
| 26.69         | $Pmc'2'_1$    | $\leftarrow$       | 26.4.171     | $Pmc'2'_1$       | III  |
| 26.70         | $Pm'c'2_1$    | $\leftarrow$       | 26.5.172     | $Pm'c'2_1$       | III  |
| 26.71         | $P_a mc2_1$   | $\leftarrow$       | 26.6.173     | $P_{2a} mc2_1$   | IV   |
| 26.72         | $P_b mc2_1$   | $\leftarrow$       | 26.7.174     | $P_{2b} mc2_1$   | IV   |
| 26.73         | $P_c mc2_1$   | $\leftarrow$       | 25.10.164    | $P_{2c} mm'2'$   | IV   |
| 26.74         | $P_A mc2_1$   | $\leftarrow$       | 38.11.275    | $A_P mm'2'$      | IV   |
| 26.75         | $P_B mc2_1$   | $\leftarrow$       | 39.10.287    | $A_P b'm2'$      | IV   |
| 26.76         | $P_C mc2_1$   | $\leftarrow$       | 36.6.254     | $C_P mc2_1$      | IV   |
| 26.77         | $P_I mc2_1$   | $\leftarrow$       | 46.8.345     | $I_P ma'2'$      | IV   |
| 27.78         | $Pcc2$        | $\leftarrow$       | 27.1.178     | $Pcc2$           | I    |
| 27.79         | $Pcc21'$      | $\leftarrow$       | 27.2.179     | $Pcc21'$         | II   |
| 27.80         | $Pc'c2'$      | $\leftarrow$       | 27.3.180     | $Pc'c2'$         | III  |
| 27.81         | $Pc'c'2$      | $\leftarrow$       | 27.4.181     | $Pc'c'2$         | III  |
| 27.82         | $P_ccc2$      | $\leftarrow$       | 25.11.165    | $P_{2c} m'm'2$   | IV   |
| 27.83         | $P_a cc2$     | $\leftarrow$       | 27.5.182     | $P_{2a} cc2$     | IV   |
| 27.84         | $P_C cc2$     | $\leftarrow$       | 37.5.262     | $C_P cc2$        | IV   |
| 27.85         | $P_A cc2$     | $\leftarrow$       | 39.12.289    | $A_P b'm'2$      | IV   |
| 27.86         | $P_I cc2$     | $\leftarrow$       | 45.5.335     | $I_P ba2$        | IV   |
| 28.87         | $Pma2$        | $Pbm2$             | 28.1.185     | $Pma2$           | I    |
| 28.88         | $Pma21'$      | $Pbm21'$           | 28.2.186     | $Pma21'$         | II   |
| 28.89         | $Pm'a2'$      | $Pbm'2'$           | 28.3.187     | $Pm'a2'$         | III  |
| 28.90         | $Pma'2'$      | $Pb'm2'$           | 28.4.188     | $Pma'2'$         | III  |
| 28.91         | $Pm'a'2$      | $Pb'm'2$           | 28.5.189     | $Pm'a'2$         | III  |
| 28.92         | $P_a ma2$     | $P_b bm2$          | 25.12.166    | $P_{2a} m'm'2$   | IV   |
| 28.93         | $P_b ma2$     | $P_a bm2$          | 28.6.190     | $P_{2b} ma2$     | IV   |
| 28.94         | $P_c ma2$     | $P_c bm2$          | 28.7.191     | $P_{2c} ma2$     | IV   |
| 28.95         | $P_A ma2$     | $P_B bm2$          | 40.6.296     | $A_P ma2$        | IV   |
| 28.96         | $P_B ma2$     | $P_A bm2$          | 39.7.284     | $A_P bm2$        | IV   |
| 28.97         | $P_C ma2$     | $P_C bm2$          | 35.10.245    | $C_P m'm2'$      | IV   |
| 28.98         | $P_I ma2$     | $P_I bm2$          | 46.6.343     | $I_P ma2$        | IV   |
| 29.99         | $Pca2_1$      | $Pbc2_1$           | 29.1.198     | $Pca2_1$         | I    |
| 29.100        | $Pca2_11'$    | $Pbc2_11'$         | 29.2.199     | $Pca2_11'$       | II   |
| 29.101        | $Pc'a2'_1$    | $Pbc'2'_1$         | 29.3.200     | $Pc'a2'_1$       | III  |
| 29.102        | $Pca'2'_1$    | $Pb'c2'_1$         | 29.4.201     | $Pca'2'_1$       | III  |
| 29.103        | $Pc'a'2_1$    | $Pb'c'2_1$         | 29.5.202     | $Pc'a'2_1$       | III  |
| 29.104        | $P_a ca2_1$   | $P_b bc2_1$        | 26.10.177    | $P_{2b} m'c'2_1$ | IV   |
| 29.105        | $P_b ca2_1$   | $P_a bc2_1$        | 29.6.203     | $P_{2b} ca2_1$   | IV   |
| 29.106        | $P_c ca2_1$   | $P_c bc2_1$        | 28.10.194    | $P_{2c} m'a2'$   | IV   |
| 29.107        | $P_A ca2_1$   | $P_B bc2_1$        | 41.7.306     | $A_P b'a2'$      | IV   |
| 29.108        | $P_B ca2_1$   | $P_A bc2_1$        | 39.11.288    | $A_P bm'2'$      | IV   |
| 29.109        | $P_C ca2_1$   | $P_C bc2_1$        | 36.7.255     | $C_P m'c2'_1$    | IV   |
| 29.110        | $P_I ca2_1$   | $P_I bc2_1$        | 45.6.336     | $I_P ba'2'$      | IV   |
| 30.111        | $Pnc2$        | $\leftarrow$       | 30.1.205     | $Pnc2$           | I    |
| 30.112        | $Pnc21'$      | $\leftarrow$       | 30.2.206     | $Pnc21'$         | II   |
| 30.113        | $Pn'c2'$      | $\leftarrow$       | 30.3.207     | $Pn'c2'$         | III  |
| 30.114        | $Pnc'2'$      | $\leftarrow$       | 30.4.208     | $Pnc'2'$         | III  |
| 30.115        | $Pn'c'2$      | $\leftarrow$       | 30.5.209     | $Pn'c'2$         | III  |
| 30.116        | $P_a nc2$     | $\leftarrow$       | 30.6.210     | $P_{2a} nc2$     | IV   |
| 30.117        | $P_b nc2$     | $\leftarrow$       | 27.7.184     | $P_{2b} c'c2'$   | IV   |
| 30.118        | $P_c nc2$     | $\leftarrow$       | 28.12.196    | $P_{2c} m'a'2$   | IV   |
| 30.119        | $P_A nc2$     | $\leftarrow$       | 38.12.276    | $A_P m'm'2$      | IV   |
| 30.120        | $P_B nc2$     | $\leftarrow$       | 41.9.308     | $A_P b'a'2$      | IV   |
| 30.121        | $P_C nc2$     | $\leftarrow$       | 37.6.263     | $C_P c'c2'$      | IV   |
| 30.122        | $P_I nc2$     | $\leftarrow$       | 46.9.346     | $I_P m'a'2$      | IV   |
| 31.123        | $Pmn2_1$      | $Pnm2_1$           | 31.1.212     | $Pmn2_1$         | I    |



| BNS<br>Number | BNS<br>Symbol | BNS (BC)<br>Symbol | OG<br>Number | OG<br>Symbol     | Type |
|---------------|---------------|--------------------|--------------|------------------|------|
| 31.124        | $Pmn2_11'$    | $Pnm2_11'$         | 31.2.213     | $Pmn2_11'$       | II   |
| 31.125        | $Pm'n2'_1$    | $Pnm'2'_1$         | 31.3.214     | $Pm'n2'_1$       | III  |
| 31.126        | $Pmn'2'_1$    | $Pn'm2'_1$         | 31.4.215     | $Pmn'2'_1$       | III  |
| 31.127        | $Pm'n'2_1$    | $Pn'm'2_1$         | 31.5.216     | $Pm'n'2_1$       | III  |
| 31.128        | $P_a mn2_1$   | $P_b nm2_1$        | 26.9.176     | $P_{2a} mc'2'_1$ | IV   |
| 31.129        | $P_b mn2_1$   | $P_a nm2_1$        | 31.6.217     | $P_{2b} mn2_1$   | IV   |
| 31.130        | $P_c mn2_1$   | $P_c nm2_1$        | 28.11.195    | $P_{2c} ma'2'$   | IV   |
| 31.131        | $P_A mn2_1$   | $P_B nm2_1$        | 40.8.298     | $A_P ma'2'$      | IV   |
| 31.132        | $P_B mn2_1$   | $P_A nm2_1$        | 38.10.274    | $A_P m'm2'$      | IV   |
| 31.133        | $P_C mn2_1$   | $P_C nm2_1$        | 36.8.256     | $C_P mc'2'_1$    | IV   |
| 31.134        | $P_I mn2_1$   | $P_I nm2_1$        | 44.6.329     | $I_P mm'2'$      | IV   |
| 32.135        | $Pba2$        | $\leftarrow$       | 32.1.219     | $Pba2$           | I    |
| 32.136        | $Pba21'$      | $\leftarrow$       | 32.2.220     | $Pba21'$         | II   |
| 32.137        | $Pb'a2'$      | $\leftarrow$       | 32.3.221     | $Pb'a2'$         | III  |
| 32.138        | $Pb'a'2$      | $\leftarrow$       | 32.4.222     | $Pb'a'2$         | III  |
| 32.139        | $P_c ba2$     | $\leftarrow$       | 32.5.223     | $P_{2c} ba2$     | IV   |
| 32.140        | $P_a ba2$     | $\leftarrow$       | 28.9.193     | $P_{2b} m'a2'$   | IV   |
| 32.141        | $P_C ba2$     | $\leftarrow$       | 35.11.246    | $C_P m'm'2$      | IV   |
| 32.142        | $P_A ba2$     | $\leftarrow$       | 41.6.305     | $A_P ba2$        | IV   |
| 32.143        | $P_I ba2$     | $\leftarrow$       | 45.7.337     | $I_P b'a'2$      | IV   |
| 33.144        | $Pna2_1$      | $Pbn2_1$           | 33.1.226     | $Pna2_1$         | I    |
| 33.145        | $Pna2_11'$    | $Pbn2_11'$         | 33.2.227     | $Pna2_11'$       | II   |
| 33.146        | $Pn'a2'_1$    | $Pbn'2'_1$         | 33.3.228     | $Pn'a2'_1$       | III  |
| 33.147        | $Pna'2'_1$    | $Pb'n2'_1$         | 33.4.229     | $Pna'2'_1$       | III  |
| 33.148        | $Pn'a'2_1$    | $Pb'n'2_1$         | 33.5.230     | $Pn'a'2_1$       | III  |
| 33.149        | $P_a na2_1$   | $P_b bn2_1$        | 31.7.218     | $P_{2b} m'n2'_1$ | IV   |
| 33.150        | $P_b na2_1$   | $P_a bn2_1$        | 29.7.204     | $P_{2b} c'a'2_1$ | IV   |
| 33.151        | $P_c na2_1$   | $P_c bn2_1$        | 32.6.224     | $P_{2c} b'a2'$   | IV   |
| 33.152        | $P_A na2_1$   | $P_B bn2_1$        | 40.7.297     | $A_P m'a2'$      | IV   |
| 33.153        | $P_B na2_1$   | $P_A bn2_1$        | 41.8.307     | $A_P ba'2'$      | IV   |
| 33.154        | $P_C na2_1$   | $P_C bn2_1$        | 36.9.257     | $C_P m'c'2_1$    | IV   |
| 33.155        | $P_I na2_1$   | $P_I bn2_1$        | 46.7.344     | $I_P m'a2'$      | IV   |
| 34.156        | $Pnn2$        | $\leftarrow$       | 34.1.231     | $Pnn2$           | I    |
| 34.157        | $Pnn21'$      | $\leftarrow$       | 34.2.232     | $Pnn21'$         | II   |
| 34.158        | $Pn'n2'$      | $\leftarrow$       | 34.3.233     | $Pn'n2'$         | III  |
| 34.159        | $Pn'n'2$      | $\leftarrow$       | 34.4.234     | $Pn'n'2$         | III  |
| 34.160        | $P_a nn2$     | $\leftarrow$       | 30.7.211     | $P_{2a} nc'2'$   | IV   |
| 34.161        | $P_c nn2$     | $\leftarrow$       | 32.7.225     | $P_{2c} b'a'2$   | IV   |
| 34.162        | $P_A nn2$     | $\leftarrow$       | 40.9.299     | $A_P m'a'2$      | IV   |
| 34.163        | $P_C nn2$     | $\leftarrow$       | 37.7.264     | $C_P c'c'2$      | IV   |
| 34.164        | $P_I nn2$     | $\leftarrow$       | 44.7.330     | $I_P m'm'2$      | IV   |
| 35.165        | $Cmm2$        | $\leftarrow$       | 35.1.236     | $Cmm2$           | I    |
| 35.166        | $Cmm21'$      | $\leftarrow$       | 35.2.237     | $Cmm21'$         | II   |
| 35.167        | $Cm'm2'$      | $\leftarrow$       | 35.3.238     | $Cm'm2'$         | III  |
| 35.168        | $Cm'm'2$      | $\leftarrow$       | 35.4.239     | $Cm'm'2$         | III  |
| 35.169        | $C_c mm2$     | $\leftarrow$       | 35.5.240     | $C_{2c} mm2$     | IV   |
| 35.170        | $C_a mm2$     | $\leftarrow$       | 25.7.161     | $P_C mm2$        | IV   |
| 35.171        | $C_A mm2$     | $\leftarrow$       | 42.5.313     | $F_C mm2$        | IV   |
| 36.172        | $Cmc2_1$      | $Ccm2_1$           | 36.1.249     | $Cmc2_1$         | I    |
| 36.173        | $Cmc2_11'$    | $Ccm2_11'$         | 36.2.250     | $Cmc2_11'$       | II   |
| 36.174        | $Cm'c2'_1$    | $Ccm'2'_1$         | 36.3.251     | $Cm'c2'_1$       | III  |
| 36.175        | $Cmc'2'_1$    | $Cc'm2'_1$         | 36.4.252     | $Cmc'2'_1$       | III  |
| 36.176        | $Cm'c'2_1$    | $Cc'm'2_1$         | 36.5.253     | $Cm'c'2_1$       | III  |
| 36.177        | $C_c mc2_1$   | $C_c cm2_1$        | 35.8.243     | $C_{2c} m'm2'$   | IV   |
| 36.178        | $C_a mc2_1$   | $C_a cm2_1$        | 26.8.175     | $P_C mc2_1$      | IV   |

| BNS<br>Number | BNS<br>Symbol | BNS (BC)<br>Symbol | OG<br>Number | OG<br>Symbol    | Type |
|---------------|---------------|--------------------|--------------|-----------------|------|
| 36.179        | $C_Amc2_1$    | $C_Acm2_1$         | 42.7.315     | $F_Cmm'm'2'$    | IV   |
| 37.180        | $Ccc2$        | $\leftarrow$       | 37.1.258     | $Ccc2$          | I    |
| 37.181        | $Ccc21'$      | $\leftarrow$       | 37.2.259     | $Ccc21'$        | II   |
| 37.182        | $Cc'c2'$      | $\leftarrow$       | 37.3.260     | $Cc'c2'$        | III  |
| 37.183        | $Cc'c'2$      | $\leftarrow$       | 37.4.261     | $Cc'c'2$        | III  |
| 37.184        | $C_ccc2$      | $\leftarrow$       | 35.9.244     | $C_{2c}m'm'2$   | IV   |
| 37.185        | $C_accc2$     | $\leftarrow$       | 27.6.183     | $P_Ccc2$        | IV   |
| 37.186        | $C_Acc2$      | $\leftarrow$       | 42.8.316     | $F_Cm'm'2$      | IV   |
| 38.187        | $Amm2$        | $Cm2m$             | 38.1.265     | $Amm2$          | I    |
| 38.188        | $Amm21'$      | $Cm2m1'$           | 38.2.266     | $Amm21'$        | II   |
| 38.189        | $Am'm2'$      | $Cm'2'm'$          | 38.3.267     | $Am'm2'$        | III  |
| 38.190        | $Amm'2'$      | $Cm'2'm$           | 38.4.268     | $Amm'2'$        | III  |
| 38.191        | $Am'm'2$      | $Cm'2m'$           | 38.5.269     | $Am'm'2$        | III  |
| 38.192        | $A_amm2$      | $C_cm2m$           | 38.6.270     | $A_{2a}mm2$     | IV   |
| 38.193        | $A_cmm2$      | $C_am2m$           | 25.8.162     | $P_Amm2$        | IV   |
| 38.194        | $A_Cmm2$      | $C_Am2m$           | 42.6.314     | $F_Amm2$        | IV   |
| 39.195        | $Abm2$        | $Cm2a$             | 39.1.278     | $Abm2$          | I    |
| 39.196        | $Abm21'$      | $Cm2a1'$           | 39.2.279     | $Abm21'$        | II   |
| 39.197        | $Ab'm2'$      | $Cm'2'a'$          | 39.3.280     | $Ab'm2'$        | III  |
| 39.198        | $Abm'2'$      | $Cm'2'a$           | 39.4.281     | $Abm'2'$        | III  |
| 39.199        | $Ab'm'2$      | $Cm'2a'$           | 39.5.282     | $Ab'm'2$        | III  |
| 39.200        | $A_abm2$      | $C_cm2a$           | 39.6.283     | $A_{2a}bm2$     | IV   |
| 39.201        | $A_cbm2$      | $C_am2a$           | 25.13.167    | $P_Am'm'2$      | IV   |
| 39.202        | $A_Cbm2$      | $C_Am2a$           | 42.9.317     | $F_Am'm'2'$     | IV   |
| 40.203        | $Ama2$        | $Cc2m$             | 40.1.291     | $Ama2$          | I    |
| 40.204        | $Ama21'$      | $Cc2m1'$           | 40.2.292     | $Ama21'$        | II   |
| 40.205        | $Am'a2'$      | $Cc'2'm'$          | 40.3.293     | $Am'a2'$        | III  |
| 40.206        | $Ama'2'$      | $Cc'2'm$           | 40.4.294     | $Ama'2'$        | III  |
| 40.207        | $Am'a'2$      | $Cc'2m'$           | 40.5.295     | $Am'a'2$        | III  |
| 40.208        | $A_ama2$      | $C_cc2m$           | 38.9.273     | $A_{2a}mm'm'2'$ | IV   |
| 40.209        | $A_cma2$      | $C_ac2m$           | 28.8.192     | $P_Ama2$        | IV   |
| 40.210        | $A_Cma2$      | $C_Ac2m$           | 42.10.318    | $F_Amm'm'2'$    | IV   |
| 41.211        | $Aba2$        | $Cc2a$             | 41.1.300     | $Aba2$          | I    |
| 41.212        | $Aba21'$      | $Cc2a1'$           | 41.2.301     | $Aba21'$        | II   |
| 41.213        | $Ab'a2'$      | $Cc'2'a'$          | 41.3.302     | $Ab'a2'$        | III  |
| 41.214        | $Aba'2'$      | $Cc'2'a$           | 41.4.303     | $Aba'2'$        | III  |
| 41.215        | $Ab'a'2$      | $Cc'2a'$           | 41.5.304     | $Ab'a'2$        | III  |
| 41.216        | $A_aba2$      | $C_cc2a$           | 39.9.286     | $A_{2a}b'm'2$   | IV   |
| 41.217        | $A_cba2$      | $C_ac2a$           | 28.13.197    | $P_Am'a'2$      | IV   |
| 41.218        | $A_Cba2$      | $C_Ac2a$           | 42.11.319    | $F_Am'm'2$      | IV   |
| 42.219        | $Fmm2$        | $\leftarrow$       | 42.1.309     | $Fmm2$          | I    |
| 42.220        | $Fmm21'$      | $\leftarrow$       | 42.2.310     | $Fmm21'$        | II   |
| 42.221        | $Fm'm2'$      | $\leftarrow$       | 42.3.311     | $Fm'm2'$        | III  |
| 42.222        | $Fm'm'2$      | $\leftarrow$       | 42.4.312     | $Fm'm'2$        | III  |
| 42.223        | $F_smm2$      | $\leftarrow$       | 25.9.163     | $P_Fmm2$        | IV   |
| 43.224        | $Fdd2$        | $\leftarrow$       | 43.1.320     | $Fdd2$          | I    |
| 43.225        | $Fdd21'$      | $\leftarrow$       | 43.2.321     | $Fdd21'$        | II   |
| 43.226        | $Fd'd2'$      | $\leftarrow$       | 43.3.322     | $Fd'd2'$        | III  |
| 43.227        | $Fd'd'2$      | $\leftarrow$       | 43.4.323     | $Fd'd'2$        | III  |
| 43.228        | $F_sdd2$      | $\leftarrow$       | 34.5.235     | $P_Fnn2$        | IV   |
| 44.229        | $Imm2$        | $\leftarrow$       | 44.1.324     | $Imm2$          | I    |
| 44.230        | $Imm21'$      | $\leftarrow$       | 44.2.325     | $Imm21'$        | II   |
| 44.231        | $Im'm2'$      | $\leftarrow$       | 44.3.326     | $Im'm2'$        | III  |
| 44.232        | $Im'm'2$      | $\leftarrow$       | 44.4.327     | $Im'm'2$        | III  |
| 44.233        | $I_cmm2$      | $\leftarrow$       | 35.7.242     | $C_Imm2$        | IV   |

| BNS<br>Number | BNS<br>Symbol | BNS (BC)<br>Symbol | OG<br>Number | OG<br>Symbol    | Type |
|---------------|---------------|--------------------|--------------|-----------------|------|
| 44.234        | $I_{amm}2$    | $\leftarrow$       | 38.8.272     | $A_{Imm}2$      | IV   |
| 45.235        | $Iba2$        | $\leftarrow$       | 45.1.331     | $Iba2$          | I    |
| 45.236        | $Iba21'$      | $\leftarrow$       | 45.2.332     | $Iba21'$        | II   |
| 45.237        | $Ib'a2'$      | $\leftarrow$       | 45.3.333     | $Ib'a2'$        | III  |
| 45.238        | $Ib'a'2$      | $\leftarrow$       | 45.4.334     | $Ib'a'2$        | III  |
| 45.239        | $I_cba2$      | $\leftarrow$       | 35.13.248    | $C_{Im'm'}2$    | IV   |
| 45.240        | $I_a ba2$     | $\leftarrow$       | 39.13.290    | $A_{Ib'm'}2$    | IV   |
| 46.241        | $Ima2$        | $Ibm2$             | 46.1.338     | $Ima2$          | I    |
| 46.242        | $Ima21'$      | $Ibm21'$           | 46.2.339     | $Ima21'$        | II   |
| 46.243        | $Im'a2'$      | $Ibm'2'$           | 46.3.340     | $Im'a2'$        | III  |
| 46.244        | $Ima'2'$      | $Ib'm'2'$          | 46.4.341     | $Ima'2'$        | III  |
| 46.245        | $Im'a'2$      | $Ib'm'2$           | 46.5.342     | $Im'a'2$        | III  |
| 46.246        | $I_cma2$      | $I_cbm2$           | 35.12.247    | $C_{Im'm'}2'$   | IV   |
| 46.247        | $I_a ma2$     | $I_bbm2$           | 38.13.277    | $A_{Im'm'}2$    | IV   |
| 46.248        | $I_b ma2$     | $I_abm2$           | 39.8.285     | $A_{Ibm}2$      | IV   |
| 47.249        | $Pmmm$        | $\leftarrow$       | 47.1.347     | $Pmmm$          | I    |
| 47.250        | $Pmmm1'$      | $\leftarrow$       | 47.2.348     | $Pmmm1'$        | II   |
| 47.251        | $Pm'mm$       | $\leftarrow$       | 47.3.349     | $Pm'mm$         | III  |
| 47.252        | $Pm'm'm$      | $\leftarrow$       | 47.4.350     | $Pm'm'm$        | III  |
| 47.253        | $Pm'm'm'$     | $\leftarrow$       | 47.5.351     | $Pm'm'm'$       | III  |
| 47.254        | $P_a mmm$     | $\leftarrow$       | 47.6.352     | $P_{2a} mmm$    | IV   |
| 47.255        | $P_C mmm$     | $\leftarrow$       | 65.9.553     | $C_P mmm$       | IV   |
| 47.256        | $P_I mmm$     | $\leftarrow$       | 71.6.626     | $I_P mmm$       | IV   |
| 48.257        | $Pnnn$        | $\leftarrow$       | 48.1.358     | $Pnnn$          | I    |
| 48.258        | $Pnnn1'$      | $\leftarrow$       | 48.2.359     | $Pnnn1'$        | II   |
| 48.259        | $Pn'nn$       | $\leftarrow$       | 48.3.360     | $Pn'nn$         | III  |
| 48.260        | $Pn'n'n$      | $\leftarrow$       | 48.4.361     | $Pn'n'n$        | III  |
| 48.261        | $Pn'n'n'$     | $\leftarrow$       | 48.5.362     | $Pn'n'n'$       | III  |
| 48.262        | $P_a nnn$     | $\leftarrow$       | 50.10.386    | $P_{2c} b'a'n$  | IV   |
| 48.263        | $P_C nnn$     | $\leftarrow$       | 66.13.576    | $C_P c'c'm'$    | IV   |
| 48.264        | $P_I nnn$     | $\leftarrow$       | 71.9.629     | $I_P m'm'm'$    | IV   |
| 49.265        | $Pccm$        | $\leftarrow$       | 49.1.364     | $Pccm$          | I    |
| 49.266        | $Pccm1'$      | $\leftarrow$       | 49.2.365     | $Pccm1'$        | II   |
| 49.267        | $Pc'cm$       | $\leftarrow$       | 49.3.366     | $Pc'cm$         | III  |
| 49.268        | $Pccm'$       | $\leftarrow$       | 49.4.367     | $Pccm'$         | III  |
| 49.269        | $Pc'c'm$      | $\leftarrow$       | 49.5.368     | $Pc'c'm$        | III  |
| 49.270        | $Pc'cm'$      | $\leftarrow$       | 49.6.369     | $Pc'cm'$        | III  |
| 49.271        | $Pc'c'm'$     | $\leftarrow$       | 49.7.370     | $Pc'c'm'$       | III  |
| 49.272        | $P_a ccm$     | $\leftarrow$       | 49.8.371     | $P_{2a} ccm$    | IV   |
| 49.273        | $P_c ccm$     | $\leftarrow$       | 47.10.356    | $P_{2c} m'm'm$  | IV   |
| 49.274        | $P_A ccm$     | $\leftarrow$       | 67.9.585     | $C_P mma$       | IV   |
| 49.275        | $P_C ccm$     | $\leftarrow$       | 66.8.571     | $C_P ccm$       | IV   |
| 49.276        | $P_I ccm$     | $\leftarrow$       | 72.8.637     | $I_P bam$       | IV   |
| 50.277        | $Pban$        | $\leftarrow$       | 50.1.377     | $Pban$          | I    |
| 50.278        | $Pban1'$      | $\leftarrow$       | 50.2.378     | $Pban1'$        | II   |
| 50.279        | $Pb'an$       | $\leftarrow$       | 50.3.379     | $Pb'an$         | III  |
| 50.280        | $Pban'$       | $\leftarrow$       | 50.4.380     | $Pban'$         | III  |
| 50.281        | $Pb'a'n$      | $\leftarrow$       | 50.5.381     | $Pb'a'n$        | III  |
| 50.282        | $Pb'an'$      | $\leftarrow$       | 50.6.382     | $Pb'an'$        | III  |
| 50.283        | $Pb'a'n'$     | $\leftarrow$       | 50.7.383     | $Pb'a'n'$       | III  |
| 50.284        | $P_a ban$     | $\leftarrow$       | 49.12.375    | $P_{2a} c'c'm'$ | IV   |
| 50.285        | $P_c ban$     | $\leftarrow$       | 50.8.384     | $P_{2c} ban$    | IV   |
| 50.286        | $P_A ban$     | $\leftarrow$       | 68.8.601     | $C_P cca$       | IV   |
| 50.287        | $P_C ban$     | $\leftarrow$       | 65.17.561    | $C_P m'm'm'$    | IV   |
| 50.288        | $P_I ban$     | $\leftarrow$       | 72.13.642    | $I_P b'a'm'$    | IV   |

| BNS<br>Number | BNS<br>Symbol | BNS (BC)<br>Symbol | OG<br>Number | OG<br>Symbol   | Type |
|---------------|---------------|--------------------|--------------|----------------|------|
| 51.289        | $Pmma$        | $Pcmm$             | 51.1.387     | $Pmma$         | I    |
| 51.290        | $Pmma1'$      | $Pcmm1'$           | 51.2.388     | $Pmma1'$       | II   |
| 51.291        | $Pm'ma$       | $Pcmm'$            | 51.3.389     | $Pm'ma$        | III  |
| 51.292        | $Pmm'a$       | $Pcm'm$            | 51.4.390     | $Pmm'a$        | III  |
| 51.293        | $Pmma'$       | $Pc'mm$            | 51.5.391     | $Pmma'$        | III  |
| 51.294        | $Pm'm'a$      | $Pcm'm'$           | 51.6.392     | $Pm'm'a$       | III  |
| 51.295        | $Pmm'a'$      | $Pc'm'm$           | 51.7.393     | $Pmm'a'$       | III  |
| 51.296        | $Pm'ma'$      | $Pc'mm'$           | 51.8.394     | $Pm'ma'$       | III  |
| 51.297        | $Pm'm'a'$     | $Pc'm'm'$          | 51.9.395     | $Pm'm'a'$      | III  |
| 51.298        | $P_a mma$     | $P_c mmm$          | 47.9.355     | $P_{2a} mmm'$  | IV   |
| 51.299        | $P_b mma$     | $P_b cmm$          | 51.10.396    | $P_{2b} mma$   | IV   |
| 51.300        | $P_c mma$     | $P_a cmm$          | 51.11.397    | $P_{2c} mma$   | IV   |
| 51.301        | $P_A mma$     | $P_C mmm$          | 63.10.520    | $C_P mcm$      | IV   |
| 51.302        | $P_B mma$     | $P_B cmm$          | 65.13.557    | $C_{Pm'} mm$   | IV   |
| 51.303        | $P_C mma$     | $P_A cmm$          | 67.14.590    | $C_P mm'a$     | IV   |
| 51.304        | $P_I mma$     | $P_I cmm$          | 74.8.657     | $I_P mma$      | IV   |
| 52.305        | $Pnna$        | $Pnan$             | 52.1.406     | $Pnna$         | I    |
| 52.306        | $Pnna1'$      | $Pnan1'$           | 52.2.407     | $Pnna1'$       | II   |
| 52.307        | $Pn'na$       | $Pn'an$            | 52.3.408     | $Pn'na$        | III  |
| 52.308        | $Pnn'a$       | $Pnan'$            | 52.4.409     | $Pnn'a$        | III  |
| 52.309        | $Pnna'$       | $Pna'n$            | 52.5.410     | $Pnna'$        | III  |
| 52.310        | $Pn'n'a$      | $Pn'an'$           | 52.6.411     | $Pn'n'a$       | III  |
| 52.311        | $Pnn'a'$      | $Pna'n'$           | 52.7.412     | $Pnn'a'$       | III  |
| 52.312        | $Pn'na'$      | $Pn'a'n$           | 52.8.413     | $Pn'na'$       | III  |
| 52.313        | $Pn'n'a'$     | $Pn'a'n'$          | 52.9.414     | $Pn'n'a'$      | III  |
| 52.314        | $P_a nna$     | $P_a nan$          | 53.13.427    | $P_{2b} m'na'$ | IV   |
| 52.315        | $P_b nna$     | $P_c nan$          | 50.9.385     | $P_{2c} b'an$  | IV   |
| 52.316        | $P_c nna$     | $P_b nan$          | 54.13.440    | $P_{2b} c'ca'$ | IV   |
| 52.317        | $P_A nna$     | $P_A nan$          | 66.12.575    | $C_P cc'm'$    | IV   |
| 52.318        | $P_B nna$     | $P_C nan$          | 63.17.527    | $C_{Pm'} c'm'$ | IV   |
| 52.319        | $P_C nna$     | $P_B nan$          | 68.11.604    | $C_P cc'a'$    | IV   |
| 52.320        | $P_I nna$     | $P_I nan$          | 74.9.658     | $I_P m'm'a$    | IV   |
| 53.321        | $Pmna$        | $Pnmb$             | 53.1.415     | $Pmna$         | I    |
| 53.322        | $Pmna1'$      | $Pnmb1'$           | 53.2.416     | $Pmna1'$       | II   |
| 53.323        | $Pm'na$       | $Pnm'b$            | 53.3.417     | $Pm'na$        | III  |
| 53.324        | $Pmn'a$       | $Pn'mb$            | 53.4.418     | $Pmn'a$        | III  |
| 53.325        | $Pmna'$       | $Pnmb'$            | 53.5.419     | $Pmna'$        | III  |
| 53.326        | $Pm'n'a$      | $Pn'm'b$           | 53.6.420     | $Pm'n'a$       | III  |
| 53.327        | $Pmn'a'$      | $Pn'mb'$           | 53.7.421     | $Pmn'a'$       | III  |
| 53.328        | $Pm'na'$      | $Pnm'b'$           | 53.8.422     | $Pm'na'$       | III  |
| 53.329        | $Pm'n'a'$     | $Pn'm'b'$          | 53.9.423     | $Pm'n'a'$      | III  |
| 53.330        | $P_a mna$     | $P_b nmb$          | 51.15.401    | $P_{2b} m'ma'$ | IV   |
| 53.331        | $P_b mna$     | $P_a nmb$          | 53.10.424    | $P_{2b} mna$   | IV   |
| 53.332        | $P_c mna$     | $P_c nmb$          | 49.11.374    | $P_{2a} c'c'm$ | IV   |
| 53.333        | $P_A mna$     | $P_B nmb$          | 66.9.572     | $C_P c'cm$     | IV   |
| 53.334        | $P_B mna$     | $P_A nmb$          | 65.16.560    | $C_{Pmm'} m'$  | IV   |
| 53.335        | $P_C mna$     | $P_C nmb$          | 64.15.542    | $C_P mc'a'$    | IV   |
| 53.336        | $P_I mna$     | $P_I nmb$          | 74.10.659    | $I_P mm'a'$    | IV   |
| 54.337        | $Pcca$        | $Pcaa$             | 54.1.428     | $Pcca$         | I    |
| 54.338        | $Pcca1'$      | $Pcaa1'$           | 54.2.429     | $Pcca1'$       | II   |
| 54.339        | $Pc'ca$       | $Pcaa'$            | 54.3.430     | $Pc'ca$        | III  |
| 54.340        | $Pcc'a$       | $Pca'a$            | 54.4.431     | $Pcc'a$        | III  |
| 54.341        | $Pcca'$       | $Pc'aa$            | 54.5.432     | $Pcca'$        | III  |
| 54.342        | $Pc'c'a$      | $Pca'a'$           | 54.6.433     | $Pc'c'a$       | III  |
| 54.343        | $Pcc'a'$      | $Pc'a'a'$          | 54.7.434     | $Pcc'a'$       | III  |
| 54.344        | $Pc'ca'$      | $Pc'aa'$           | 54.8.435     | $Pc'ca'$       | III  |

| BNS<br>Number | BNS<br>Symbol | BNS (BC)<br>Symbol | OG<br>Number | OG<br>Symbol  | Type |
|---------------|---------------|--------------------|--------------|---------------|------|
| 54.345        | $Pc'c'a'$     | $Pc'a'a'$          | 54.9.436     | $Pc'c'a'$     | III  |
| 54.346        | $P_{a}cca$    | $P_{c}caa$         | 49.10.373    | $P_{2a}ccm'$  | IV   |
| 54.347        | $P_{b}cca$    | $P_{b}caa$         | 54.10.437    | $P_{2b}cca$   | IV   |
| 54.348        | $P_{c}cca$    | $P_{a}caa$         | 51.18.404    | $P_{2c}m'm'a$ | IV   |
| 54.349        | $P_{A}cca$    | $P_{C}caa$         | 64.11.538    | $C_{Pm'}ca$   | IV   |
| 54.350        | $P_{B}cca$    | $P_{B}caa$         | 67.13.589    | $C_{Pm'}ma$   | IV   |
| 54.351        | $P_{C}cca$    | $P_{A}caa$         | 68.9.602     | $C_{Pc'}ca$   | IV   |
| 54.352        | $P_{I}cca$    | $P_{I}caa$         | 73.7.649     | $I_{Pb'}ca$   | IV   |
| 55.353        | $Pbam$        | $\leftarrow$       | 55.1.441     | $Pbam$        | I    |
| 55.354        | $Pbam1'$      | $\leftarrow$       | 55.2.442     | $Pbam1'$      | II   |
| 55.355        | $Pb'am$       | $\leftarrow$       | 55.3.443     | $Pb'am$       | III  |
| 55.356        | $Pbam'$       | $\leftarrow$       | 55.4.444     | $Pbam'$       | III  |
| 55.357        | $Pb'a'm$      | $\leftarrow$       | 55.5.445     | $Pb'a'm$      | III  |
| 55.358        | $Pb'am'$      | $\leftarrow$       | 55.6.446     | $Pb'am'$      | III  |
| 55.359        | $Pb'a'm'$     | $\leftarrow$       | 55.7.447     | $Pb'a'm'$     | III  |
| 55.360        | $P_{a}bam$    | $\leftarrow$       | 51.16.402    | $P_{2c}m'ma$  | IV   |
| 55.361        | $P_{c}bam$    | $\leftarrow$       | 55.8.448     | $P_{2c}bam$   | IV   |
| 55.362        | $P_{A}bam$    | $\leftarrow$       | 64.10.537    | $C_{Pm}ca$    | IV   |
| 55.363        | $P_{C}bam$    | $\leftarrow$       | 65.15.559    | $C_{Pm'm'm}$  | IV   |
| 55.364        | $P_{I}bam$    | $\leftarrow$       | 72.11.640    | $I_{Pb'a'm}$  | IV   |
| 56.365        | $Pccn$        | $\leftarrow$       | 56.1.451     | $Pccn$        | I    |
| 56.366        | $Pccn1'$      | $\leftarrow$       | 56.2.452     | $Pccn1'$      | II   |
| 56.367        | $Pc'cn$       | $\leftarrow$       | 56.3.453     | $Pc'cn$       | III  |
| 56.368        | $Pccn'$       | $\leftarrow$       | 56.4.454     | $Pccn'$       | III  |
| 56.369        | $Pc'c'n$      | $\leftarrow$       | 56.5.455     | $Pc'c'n$      | III  |
| 56.370        | $Pc'cn'$      | $\leftarrow$       | 56.6.456     | $Pc'cn'$      | III  |
| 56.371        | $Pc'c'n'$     | $\leftarrow$       | 56.7.457     | $Pc'c'n'$     | III  |
| 56.372        | $P_{a}ccn$    | $\leftarrow$       | 54.12.439    | $P_{2b}cca'$  | IV   |
| 56.373        | $P_{c}ccn$    | $\leftarrow$       | 59.10.487    | $P_{2c}m'm'n$ | IV   |
| 56.374        | $P_{A}ccn$    | $\leftarrow$       | 64.14.541    | $C_{Pm'}c'a$  | IV   |
| 56.375        | $P_{C}ccn$    | $\leftarrow$       | 66.10.573    | $C_{Pccm'}$   | IV   |
| 56.376        | $P_{I}ccn$    | $\leftarrow$       | 72.10.639    | $I_{Pbam'}$   | IV   |
| 57.377        | $Pbcm$        | $Pbma$             | 57.1.458     | $Pbcm$        | I    |
| 57.378        | $Pbcm1'$      | $Pbma1'$           | 57.2.459     | $Pbcm1'$      | II   |
| 57.379        | $Pb'cm$       | $Pbma'$            | 57.3.460     | $Pb'cm$       | III  |
| 57.380        | $Pbc'm$       | $Pb'ma$            | 57.4.461     | $Pbc'm$       | III  |
| 57.381        | $Pbcm'$       | $Pbm'a$            | 57.5.462     | $Pbcm'$       | III  |
| 57.382        | $Pb'c'm$      | $Pb'ma'$           | 57.6.463     | $Pb'c'm$      | III  |
| 57.383        | $Pbc'm'$      | $Pb'm'a$           | 57.7.464     | $Pbc'm'$      | III  |
| 57.384        | $Pb'cm'$      | $Pbm'a'$           | 57.8.465     | $Pb'cm'$      | III  |
| 57.385        | $Pb'c'm'$     | $Pb'm'a'$          | 57.9.466     | $Pb'c'm'$     | III  |
| 57.386        | $P_{a}bcm$    | $P_{c}bma$         | 57.10.467    | $P_{2a}bcm$   | IV   |
| 57.387        | $P_{b}bcm$    | $P_{a}bma$         | 51.17.403    | $P_{2c}mm'a$  | IV   |
| 57.388        | $P_{c}bcm$    | $P_{b}bma$         | 51.13.399    | $P_{2b}m'ma$  | IV   |
| 57.389        | $P_{A}bcm$    | $P_{C}bma$         | 67.15.591    | $C_{Pmma'}$   | IV   |
| 57.390        | $P_{B}bcm$    | $P_{A}bma$         | 64.13.540    | $C_{Pm}ca'$   | IV   |
| 57.391        | $P_{C}bcm$    | $P_{B}bma$         | 63.11.521    | $C_{Pm'}cm$   | IV   |
| 57.392        | $P_{I}bcm$    | $P_{I}bma$         | 72.9.638     | $I_{Pb'am}$   | IV   |
| 58.393        | $Pnnm$        | $\leftarrow$       | 58.1.471     | $Pnnm$        | I    |
| 58.394        | $Pnnm1'$      | $\leftarrow$       | 58.2.472     | $Pnnm1'$      | II   |
| 58.395        | $Pn'nm$       | $\leftarrow$       | 58.3.473     | $Pn'nm$       | III  |
| 58.396        | $Pnnm'$       | $\leftarrow$       | 58.4.474     | $Pnnm'$       | III  |
| 58.397        | $Pn'n'm$      | $\leftarrow$       | 58.5.475     | $Pn'n'm$      | III  |
| 58.398        | $Pnn'm'$      | $\leftarrow$       | 58.6.476     | $Pnn'm'$      | III  |
| 58.399        | $Pn'n'm'$     | $\leftarrow$       | 58.7.477     | $Pn'n'm'$     | III  |
| 58.400        | $P_{a}nnm$    | $\leftarrow$       | 53.12.426    | $P_{2b}mna'$  | IV   |

| BNS<br>Number | BNS<br>Symbol | BNS (BC)<br>Symbol | OG<br>Number | OG<br>Symbol    | Type |
|---------------|---------------|--------------------|--------------|-----------------|------|
| 58.401        | $P_cnnm$      | $\leftarrow$       | 55.10.450    | $P_{2c}b'a'm$   | IV   |
| 58.402        | $P_Annm$      | $\leftarrow$       | 63.15.525    | $C_Pmc'm'$      | IV   |
| 58.403        | $P_Cnnm$      | $\leftarrow$       | 66.11.574    | $C_Pc'c'm$      | IV   |
| 58.404        | $P_Innm$      | $\leftarrow$       | 71.8.628     | $I_Pm'm'm$      | IV   |
| 59.405        | $Pmmn$        | $\leftarrow$       | 59.1.478     | $Pmmn$          | I    |
| 59.406        | $Pmmn1'$      | $\leftarrow$       | 59.2.479     | $Pmmn1'$        | II   |
| 59.407        | $Pm'mn$       | $\leftarrow$       | 59.3.480     | $Pm'mn$         | III  |
| 59.408        | $Pmmn'$       | $\leftarrow$       | 59.4.481     | $Pmmn'$         | III  |
| 59.409        | $Pm'm'n$      | $\leftarrow$       | 59.5.482     | $Pm'm'n$        | III  |
| 59.410        | $Pmm'n'$      | $\leftarrow$       | 59.6.483     | $Pmm'n'$        | III  |
| 59.411        | $Pm'm'n'$     | $\leftarrow$       | 59.7.484     | $Pm'm'n'$       | III  |
| 59.412        | $P_a m m n$   | $\leftarrow$       | 51.14.400    | $P_{2b} m m a'$ | IV   |
| 59.413        | $P_c m m n$   | $\leftarrow$       | 59.8.485     | $P_{2c} m m n$  | IV   |
| 59.414        | $P_A m m n$   | $\leftarrow$       | 63.12.522    | $C_P m c' m$    | IV   |
| 59.415        | $P_C m m n$   | $\leftarrow$       | 65.14.558    | $C_P m m m'$    | IV   |
| 59.416        | $P_I m m n$   | $\leftarrow$       | 71.7.627     | $I_P m' m m$    | IV   |
| 60.417        | $Pbcn$        | $Pcnb$             | 60.1.488     | $Pbcn$          | I    |
| 60.418        | $Pbcn1'$      | $Pcnb1'$           | 60.2.489     | $Pbcn1'$        | II   |
| 60.419        | $Pb'cn$       | $Pc'nb$            | 60.3.490     | $Pb'cn$         | III  |
| 60.420        | $Pbc'n$       | $Pcnb'$            | 60.4.491     | $Pbc'n$         | III  |
| 60.421        | $Pbcn'$       | $Pcn'b$            | 60.5.492     | $Pbcn'$         | III  |
| 60.422        | $Pb'c'n$      | $Pc'nb'$           | 60.6.493     | $Pb'c'n$        | III  |
| 60.423        | $Pbc'n'$      | $Pcn'b'$           | 60.7.494     | $Pbc'n'$        | III  |
| 60.424        | $Pb'cn'$      | $Pc'n'b$           | 60.8.495     | $Pb'cn'$        | III  |
| 60.425        | $Pb'c'n'$     | $Pc'n'b'$          | 60.9.496     | $Pb'c'n'$       | III  |
| 60.426        | $P_a b c n$   | $P_a c n b$        | 54.11.438    | $P_{2b}c'ca$    | IV   |
| 60.427        | $P_b b c n$   | $P_c c n b$        | 57.13.470    | $P_{2a}bc'm'$   | IV   |
| 60.428        | $P_c b c n$   | $P_b c n b$        | 53.11.425    | $P_{2b}m'na$    | IV   |
| 60.429        | $P_A b c n$   | $P_A c n b$        | 64.17.544    | $C_Pm'c'a'$     | IV   |
| 60.430        | $P_B b c n$   | $P_C c n b$        | 68.10.603    | $C_Pcca'$       | IV   |
| 60.431        | $P_C b c n$   | $P_B c n b$        | 63.16.526    | $C_Pm'cm'$      | IV   |
| 60.432        | $P_I b c n$   | $P_I c n b$        | 72.12.641    | $I_Pb'am'$      | IV   |
| 61.433        | $Pbca$        | $Pcab$             | 61.1.497     | $Pbca$          | I    |
| 61.434        | $Pbca1'$      | $Pcab1'$           | 61.2.498     | $Pbca1'$        | II   |
| 61.435        | $Pb'ca$       | $Pc'ab$            | 61.3.499     | $Pb'ca$         | III  |
| 61.436        | $Pb'c'a$      | $Pc'a'b$           | 61.4.500     | $Pb'c'a$        | III  |
| 61.437        | $Pb'c'a'$     | $Pc'a'b'$          | 61.5.501     | $Pb'c'a'$       | III  |
| 61.438        | $P_a b c a$   | $P_a c a b$        | 57.12.469    | $P_{2a}bcm'$    | IV   |
| 61.439        | $P_C b c a$   | $P_C c a b$        | 64.16.543    | $C_Pm'ca'$      | IV   |
| 61.440        | $P_I b c a$   | $P_I c a b$        | 73.6.648     | $I_Pbca$        | IV   |
| 62.441        | $Pnma$        | $\leftarrow$       | 62.1.502     | $Pnma$          | I    |
| 62.442        | $Pnma1'$      | $\leftarrow$       | 62.2.503     | $Pnma1'$        | II   |
| 62.443        | $Pn'ma$       | $\leftarrow$       | 62.3.504     | $Pn'ma$         | III  |
| 62.444        | $Pnm'a$       | $\leftarrow$       | 62.4.505     | $Pnm'a$         | III  |
| 62.445        | $Pnma'$       | $\leftarrow$       | 62.5.506     | $Pnma'$         | III  |
| 62.446        | $Pn'm'a$      | $\leftarrow$       | 62.6.507     | $Pn'm'a$        | III  |
| 62.447        | $Pnm'a'$      | $\leftarrow$       | 62.7.508     | $Pnm'a'$        | III  |
| 62.448        | $Pn'ma'$      | $\leftarrow$       | 62.8.509     | $Pn'ma'$        | III  |
| 62.449        | $Pn'm'a'$     | $\leftarrow$       | 62.9.510     | $Pn'm'a'$       | III  |
| 62.450        | $P_a n m a$   | $\leftarrow$       | 59.9.486     | $P_{2c}m'mn$    | IV   |
| 62.451        | $P_b n m a$   | $\leftarrow$       | 55.9.449     | $P_{2c}b'am$    | IV   |
| 62.452        | $P_c n m a$   | $\leftarrow$       | 57.11.468    | $P_{2a}bc'm$    | IV   |
| 62.453        | $P_A n m a$   | $\leftarrow$       | 63.13.523    | $C_Pmcm'$       | IV   |
| 62.454        | $P_B n m a$   | $\leftarrow$       | 63.14.524    | $C_Pm'c'm$      | IV   |
| 62.455        | $P_C n m a$   | $\leftarrow$       | 64.12.539    | $C_Pmc'a$       | IV   |

| BNS<br>Number | BNS<br>Symbol | BNS (BC)<br>Symbol | OG<br>Number | OG<br>Symbol  | Type |
|---------------|---------------|--------------------|--------------|---------------|------|
| 62.456        | $P_1nma$      | $\leftarrow$       | 74.11.660    | $I_Pm'ma'$    | IV   |
| 63.457        | $Cmcm$        | $\leftarrow$       | 63.1.511     | $Cmcm$        | I    |
| 63.458        | $Cmcm1'$      | $\leftarrow$       | 63.2.512     | $Cmcm1'$      | II   |
| 63.459        | $Cm'cm$       | $\leftarrow$       | 63.3.513     | $Cm'cm$       | III  |
| 63.460        | $Cmc'm$       | $\leftarrow$       | 63.4.514     | $Cmc'm$       | III  |
| 63.461        | $Cmcm'$       | $\leftarrow$       | 63.5.515     | $Cmcm'$       | III  |
| 63.462        | $Cm'c'm$      | $\leftarrow$       | 63.6.516     | $Cm'c'm$      | III  |
| 63.463        | $Cmc'm'$      | $\leftarrow$       | 63.7.517     | $Cmc'm'$      | III  |
| 63.464        | $Cm'cm'$      | $\leftarrow$       | 63.8.518     | $Cm'cm'$      | III  |
| 63.465        | $Cm'c'm'$     | $\leftarrow$       | 63.9.519     | $Cm'c'm'$     | III  |
| 63.466        | $C_cmcm$      | $\leftarrow$       | 65.12.556    | $C_{2c}mm'm'$ | IV   |
| 63.467        | $C_amcm$      | $\leftarrow$       | 51.12.398    | $P_Amma$      | IV   |
| 63.468        | $C_Amcm$      | $\leftarrow$       | 69.7.611     | $F_Cm'mm$     | IV   |
| 64.469        | $Cmca$        | $\leftarrow$       | 64.1.528     | $Cmca$        | I    |
| 64.470        | $Cmca1'$      | $\leftarrow$       | 64.2.529     | $Cmca1'$      | II   |
| 64.471        | $Cm'ca$       | $\leftarrow$       | 64.3.530     | $Cm'ca$       | III  |
| 64.472        | $Cmc'a$       | $\leftarrow$       | 64.4.531     | $Cmc'a$       | III  |
| 64.473        | $Cmca'$       | $\leftarrow$       | 64.5.532     | $Cmca'$       | III  |
| 64.474        | $Cm'c'a$      | $\leftarrow$       | 64.6.533     | $Cm'c'a$      | III  |
| 64.475        | $Cmc'a'$      | $\leftarrow$       | 64.7.534     | $Cmc'a'$      | III  |
| 64.476        | $Cm'ca'$      | $\leftarrow$       | 64.8.535     | $Cm'ca'$      | III  |
| 64.477        | $Cm'c'a'$     | $\leftarrow$       | 64.9.536     | $Cm'c'a'$     | III  |
| 64.478        | $C_cmca$      | $\leftarrow$       | 67.11.587    | $C_{2c}m'ma$  | IV   |
| 64.479        | $C_amca$      | $\leftarrow$       | 51.19.405    | $P_Am'ma$     | IV   |
| 64.480        | $C_Amca$      | $\leftarrow$       | 69.10.614    | $F_Cmm'm'$    | IV   |
| 65.481        | $Cmmm$        | $\leftarrow$       | 65.1.545     | $Cmmm$        | I    |
| 65.482        | $Cmmm1'$      | $\leftarrow$       | 65.2.546     | $Cmmm1'$      | II   |
| 65.483        | $Cm'mm$       | $\leftarrow$       | 65.3.547     | $Cm'mm$       | III  |
| 65.484        | $Cmmm'$       | $\leftarrow$       | 65.4.548     | $Cmmm'$       | III  |
| 65.485        | $Cm'm'm$      | $\leftarrow$       | 65.5.549     | $Cm'm'm$      | III  |
| 65.486        | $Cmm'm'$      | $\leftarrow$       | 65.6.550     | $Cmm'm'$      | III  |
| 65.487        | $Cm'm'm'$     | $\leftarrow$       | 65.7.551     | $Cm'm'm'$     | III  |
| 65.488        | $C_cmmm$      | $\leftarrow$       | 65.8.552     | $C_{2c}mmm$   | IV   |
| 65.489        | $C_ammm$      | $\leftarrow$       | 47.7.353     | $P_Cmmm$      | IV   |
| 65.490        | $C_Ammm$      | $\leftarrow$       | 69.6.610     | $F_Cmmm$      | IV   |
| 66.491        | $Cccm$        | $\leftarrow$       | 66.1.564     | $Cccm$        | I    |
| 66.492        | $Cccm1'$      | $\leftarrow$       | 66.2.565     | $Cccm1'$      | II   |
| 66.493        | $Cc'cm$       | $\leftarrow$       | 66.3.566     | $Cc'cm$       | III  |
| 66.494        | $Cccm'$       | $\leftarrow$       | 66.4.567     | $Cccm'$       | III  |
| 66.495        | $Cc'c'm$      | $\leftarrow$       | 66.5.568     | $Cc'c'm$      | III  |
| 66.496        | $Ccc'm'$      | $\leftarrow$       | 66.6.569     | $Ccc'm'$      | III  |
| 66.497        | $Cc'c'm'$     | $\leftarrow$       | 66.7.570     | $Cc'c'm'$     | III  |
| 66.498        | $C_cccm$      | $\leftarrow$       | 65.11.555    | $C_{2c}m'm'm$ | IV   |
| 66.499        | $C_accm$      | $\leftarrow$       | 49.9.372     | $P_Cccm$      | IV   |
| 66.500        | $C_Accm$      | $\leftarrow$       | 69.9.613     | $F_Cm'm'm$    | IV   |
| 67.501        | $Cmma$        | $\leftarrow$       | 67.1.577     | $Cmma$        | I    |
| 67.502        | $Cmma1'$      | $\leftarrow$       | 67.2.578     | $Cmma1'$      | II   |
| 67.503        | $Cm'ma$       | $\leftarrow$       | 67.3.579     | $Cm'ma$       | III  |
| 67.504        | $Cmma'$       | $\leftarrow$       | 67.4.580     | $Cmma'$       | III  |
| 67.505        | $Cm'm'a$      | $\leftarrow$       | 67.5.581     | $Cm'm'a$      | III  |
| 67.506        | $Cmm'a'$      | $\leftarrow$       | 67.6.582     | $Cmm'a'$      | III  |
| 67.507        | $Cm'm'a'$     | $\leftarrow$       | 67.7.583     | $Cm'm'a'$     | III  |
| 67.508        | $C_cmma$      | $\leftarrow$       | 67.8.584     | $C_{2c}mma$   | IV   |
| 67.509        | $C_amma$      | $\leftarrow$       | 47.11.357    | $P_Cmmm'$     | IV   |
| 67.510        | $C_Amma$      | $\leftarrow$       | 69.8.612     | $F_Cmmm'$     | IV   |

| BNS<br>Number | BNS<br>Symbol | BNS (BC)<br>Symbol | OG<br>Number | OG<br>Symbol  | Type |
|---------------|---------------|--------------------|--------------|---------------|------|
| 68.511        | $Ccca$        | $\leftarrow$       | 68.1.594     | $Ccca$        | I    |
| 68.512        | $Ccca1'$      | $\leftarrow$       | 68.2.595     | $Ccca1'$      | II   |
| 68.513        | $Cc'ca$       | $\leftarrow$       | 68.3.596     | $Cc'ca$       | III  |
| 68.514        | $Ccca'$       | $\leftarrow$       | 68.4.597     | $Ccca'$       | III  |
| 68.515        | $Cc'c'a$      | $\leftarrow$       | 68.5.598     | $Cc'c'a$      | III  |
| 68.516        | $Ccc'a'$      | $\leftarrow$       | 68.6.599     | $Ccc'a'$      | III  |
| 68.517        | $Cc'c'a'$     | $\leftarrow$       | 68.7.600     | $Cc'c'a'$     | III  |
| 68.518        | $C_ccca$      | $\leftarrow$       | 67.12.588    | $C_{2c}m'm'a$ | IV   |
| 68.519        | $C_acca$      | $\leftarrow$       | 49.13.376    | $P_Cccm'$     | IV   |
| 68.520        | $C_Acca$      | $\leftarrow$       | 69.11.615    | $F_Cm'm'm'$   | IV   |
| 69.521        | $Fmmm$        | $\leftarrow$       | 69.1.605     | $Fmmm$        | I    |
| 69.522        | $Fmmm1'$      | $\leftarrow$       | 69.2.606     | $Fmmm1'$      | II   |
| 69.523        | $Fm'mm$       | $\leftarrow$       | 69.3.607     | $Fm'mm$       | III  |
| 69.524        | $Fm'm'm$      | $\leftarrow$       | 69.4.608     | $Fm'm'm$      | III  |
| 69.525        | $Fm'm'm'$     | $\leftarrow$       | 69.5.609     | $Fm'm'm'$     | III  |
| 69.526        | $F_smmm$      | $\leftarrow$       | 47.8.354     | $P_Fmmm$      | IV   |
| 70.527        | $Fddd$        | $\leftarrow$       | 70.1.616     | $Fddd$        | I    |
| 70.528        | $Fddd1'$      | $\leftarrow$       | 70.2.617     | $Fddd1'$      | II   |
| 70.529        | $Fd'dd$       | $\leftarrow$       | 70.3.618     | $Fd'dd$       | III  |
| 70.530        | $Fd'd'd$      | $\leftarrow$       | 70.4.619     | $Fd'd'd$      | III  |
| 70.531        | $Fd'd'd'$     | $\leftarrow$       | 70.5.620     | $Fd'd'd'$     | III  |
| 70.532        | $F_sddd$      | $\leftarrow$       | 48.6.363     | $P_Fnnn$      | IV   |
| 71.533        | $Immm$        | $\leftarrow$       | 71.1.621     | $Immm$        | I    |
| 71.534        | $Immm1'$      | $\leftarrow$       | 71.2.622     | $Immm1'$      | II   |
| 71.535        | $Im'mm$       | $\leftarrow$       | 71.3.623     | $Im'mm$       | III  |
| 71.536        | $Im'm'm$      | $\leftarrow$       | 71.4.624     | $Im'm'm$      | III  |
| 71.537        | $Im'm'm'$     | $\leftarrow$       | 71.5.625     | $Im'm'm'$     | III  |
| 71.538        | $I_cmmm$      | $\leftarrow$       | 65.10.554    | $C_Immm$      | IV   |
| 72.539        | $Ibam$        | $\leftarrow$       | 72.1.630     | $Ibam$        | I    |
| 72.540        | $Ibam1'$      | $\leftarrow$       | 72.2.631     | $Ibam1'$      | II   |
| 72.541        | $Ib'am$       | $\leftarrow$       | 72.3.632     | $Ib'am$       | III  |
| 72.542        | $Ibam'$       | $\leftarrow$       | 72.4.633     | $Ibam'$       | III  |
| 72.543        | $Ib'a'm$      | $\leftarrow$       | 72.5.634     | $Ib'a'm$      | III  |
| 72.544        | $Iba'm'$      | $\leftarrow$       | 72.6.635     | $Iba'm'$      | III  |
| 72.545        | $Ib'a'm'$     | $\leftarrow$       | 72.7.636     | $Ib'a'm'$     | III  |
| 72.546        | $I_cbam$      | $\leftarrow$       | 65.19.563    | $C_I m'm'm$   | IV   |
| 72.547        | $I_abam$      | $\leftarrow$       | 67.10.586    | $C_I mma$     | IV   |
| 73.548        | $Ibca$        | $\leftarrow$       | 73.1.643     | $Ibca$        | I    |
| 73.549        | $Ibca1'$      | $\leftarrow$       | 73.2.644     | $Ibca1'$      | II   |
| 73.550        | $Ib'ca$       | $\leftarrow$       | 73.3.645     | $Ib'ca$       | III  |
| 73.551        | $Ib'c'a$      | $\leftarrow$       | 73.4.646     | $Ib'c'a$      | III  |
| 73.552        | $Ib'c'a'$     | $\leftarrow$       | 73.5.647     | $Ib'c'a'$     | III  |
| 73.553        | $I_c bca$     | $\leftarrow$       | 67.17.593    | $C_I m'ma'$   | IV   |
| 74.554        | $Imma$        | $\leftarrow$       | 74.1.650     | $Imma$        | I    |
| 74.555        | $Imma1'$      | $\leftarrow$       | 74.2.651     | $Imma1'$      | II   |
| 74.556        | $Im'ma$       | $\leftarrow$       | 74.3.652     | $Im'ma$       | III  |
| 74.557        | $Imma'$       | $\leftarrow$       | 74.4.653     | $Imma'$       | III  |
| 74.558        | $Im'm'a$      | $\leftarrow$       | 74.5.654     | $Im'm'a$      | III  |
| 74.559        | $Imm'a'$      | $\leftarrow$       | 74.6.655     | $Imm'a'$      | III  |
| 74.560        | $Im'm'a'$     | $\leftarrow$       | 74.7.656     | $Im'm'a'$     | III  |
| 74.561        | $I_c mma$     | $\leftarrow$       | 67.16.592    | $C_I mm'a$    | IV   |
| 74.562        | $I_a mma$     | $\leftarrow$       | 65.18.562    | $C_I m'mm$    | IV   |
| 75.1          | $P4$          | $\leftarrow$       | 75.1.661     | $P4$          | I    |
| 75.2          | $P41'$        | $\leftarrow$       | 75.2.662     | $P41'$        | II   |
| 75.3          | $P4'$         | $\leftarrow$       | 75.3.663     | $P4'$         | III  |



| BNS<br>Number | BNS<br>Symbol | BNS (BC)<br>Symbol | OG<br>Number | OG<br>Symbol    | Type |
|---------------|---------------|--------------------|--------------|-----------------|------|
| 75.4          | $P_4$         | $\leftarrow$       | 75.4.664     | $P_{2c}4$       | IV   |
| 75.5          | $P_C4$        | $\leftarrow$       | 75.5.665     | $P_P4$          | IV   |
| 75.6          | $P_I4$        | $\leftarrow$       | 79.4.686     | $I_P4$          | IV   |
| 76.7          | $P4_1$        | $\leftarrow$       | 76.1.668     | $P4_1$          | I    |
| 76.8          | $P4_11'$      | $\leftarrow$       | 76.2.669     | $P4_11'$        | II   |
| 76.9          | $P4'_1$       | $\leftarrow$       | 76.3.670     | $P4'_1$         | III  |
| 76.10         | $P_c4_1$      | $\leftarrow$       | 77.4.675     | $P_{2c}4_2$     | IV   |
| 76.11         | $P_C4_1$      | $\leftarrow$       | 76.4.671     | $P_P4_1$        | IV   |
| 76.12         | $P_I4_1$      | $\leftarrow$       | 80.4.691     | $I_P4_1$        | IV   |
| 77.13         | $P4_2$        | $\leftarrow$       | 77.1.672     | $P4_2$          | I    |
| 77.14         | $P4_21'$      | $\leftarrow$       | 77.2.673     | $P4_21'$        | II   |
| 77.15         | $P4'_2$       | $\leftarrow$       | 77.3.674     | $P4'_2$         | III  |
| 77.16         | $P_c4_2$      | $\leftarrow$       | 75.7.667     | $P_{2c}4'_2$    | IV   |
| 77.17         | $P_C4_2$      | $\leftarrow$       | 77.5.676     | $P_P4_2$        | IV   |
| 77.18         | $P_I4_2$      | $\leftarrow$       | 79.5.687     | $I_P4'_2$       | IV   |
| 78.19         | $P4_3$        | $\leftarrow$       | 78.1.679     | $P4_3$          | I    |
| 78.20         | $P4_31'$      | $\leftarrow$       | 78.2.680     | $P4_31'$        | II   |
| 78.21         | $P4'_3$       | $\leftarrow$       | 78.3.681     | $P4'_3$         | III  |
| 78.22         | $P_c4_3$      | $\leftarrow$       | 77.7.678     | $P_{2c}4'_2$    | IV   |
| 78.23         | $P_C4_3$      | $\leftarrow$       | 78.4.682     | $P_P4_3$        | IV   |
| 78.24         | $P_I4_3$      | $\leftarrow$       | 80.5.692     | $I_P4'_1$       | IV   |
| 79.25         | $I4$          | $\leftarrow$       | 79.1.683     | $I4$            | I    |
| 79.26         | $I41'$        | $\leftarrow$       | 79.2.684     | $I41'$          | II   |
| 79.27         | $I4'$         | $\leftarrow$       | 79.3.685     | $I4'$           | III  |
| 79.28         | $I_c4$        | $\leftarrow$       | 75.6.666     | $P_I4$          | IV   |
| 80.29         | $I4_1$        | $\leftarrow$       | 80.1.688     | $I4_1$          | I    |
| 80.30         | $I4_11'$      | $\leftarrow$       | 80.2.689     | $I4_11'$        | II   |
| 80.31         | $I4'_1$       | $\leftarrow$       | 80.3.690     | $I4'_1$         | III  |
| 80.32         | $I_c4_1$      | $\leftarrow$       | 77.6.677     | $P_I4_2$        | IV   |
| 81.33         | $P\bar{4}$    | $\leftarrow$       | 81.1.693     | $P\bar{4}$      | I    |
| 81.34         | $P\bar{4}1'$  | $\leftarrow$       | 81.2.694     | $P\bar{4}1'$    | II   |
| 81.35         | $P\bar{4}'$   | $\leftarrow$       | 81.3.695     | $P\bar{4}'$     | III  |
| 81.36         | $P_c\bar{4}$  | $\leftarrow$       | 81.4.696     | $P_{2c}\bar{4}$ | IV   |
| 81.37         | $P_C\bar{4}$  | $\leftarrow$       | 81.5.697     | $P_P\bar{4}$    | IV   |
| 81.38         | $P_I\bar{4}$  | $\leftarrow$       | 82.4.702     | $I_P\bar{4}$    | IV   |
| 82.39         | $I\bar{4}$    | $\leftarrow$       | 82.1.699     | $I\bar{4}$      | I    |
| 82.40         | $I\bar{4}1'$  | $\leftarrow$       | 82.2.700     | $I\bar{4}1'$    | II   |
| 82.41         | $I\bar{4}'$   | $\leftarrow$       | 82.3.701     | $I\bar{4}'$     | III  |
| 82.42         | $I_c\bar{4}$  | $\leftarrow$       | 81.6.698     | $P_I\bar{4}$    | IV   |
| 83.43         | $P4/m$        | $\leftarrow$       | 83.1.703     | $P4/m$          | I    |
| 83.44         | $P4/m1'$      | $\leftarrow$       | 83.2.704     | $P4/m1'$        | II   |
| 83.45         | $P4'/m$       | $\leftarrow$       | 83.3.705     | $P4'/m$         | III  |
| 83.46         | $P4/m'$       | $\leftarrow$       | 83.4.706     | $P4/m'$         | III  |
| 83.47         | $P4'/m'$      | $\leftarrow$       | 83.5.707     | $P4'/m'$        | III  |
| 83.48         | $P_c4/m$      | $\leftarrow$       | 83.6.708     | $P_{2c}4/m$     | IV   |
| 83.49         | $P_C4/m$      | $\leftarrow$       | 83.7.709     | $P_P4/m$        | IV   |
| 83.50         | $P_I4/m$      | $\leftarrow$       | 87.6.738     | $I_P4/m$        | IV   |
| 84.51         | $P4_2/m$      | $\leftarrow$       | 84.1.713     | $P4_2/m$        | I    |
| 84.52         | $P4_2/m1'$    | $\leftarrow$       | 84.2.714     | $P4_2/m1'$      | II   |
| 84.53         | $P4'_2/m$     | $\leftarrow$       | 84.3.715     | $P4'_2/m$       | III  |
| 84.54         | $P4_2/m'$     | $\leftarrow$       | 84.4.716     | $P4_2/m'$       | III  |
| 84.55         | $P4'_2/m'$    | $\leftarrow$       | 84.5.717     | $P4'_2/m'$      | III  |
| 84.56         | $P_c4_2/m$    | $\leftarrow$       | 83.9.711     | $P_{2c}4'/m$    | IV   |
| 84.57         | $P_C4_2/m$    | $\leftarrow$       | 84.6.718     | $P_P4_2/m$      | IV   |
| 84.58         | $P_I4_2/m$    | $\leftarrow$       | 87.7.739     | $I_P4'/m$       | IV   |

| BNS<br>Number | BNS<br>Symbol | BNS (BC)<br>Symbol | OG<br>Number | OG<br>Symbol   | Type |
|---------------|---------------|--------------------|--------------|----------------|------|
| 85.59         | $P4/n$        | $\leftarrow$       | 85.1.720     | $P4/n$         | I    |
| 85.60         | $P4/n1'$      | $\leftarrow$       | 85.2.721     | $P4/n1'$       | II   |
| 85.61         | $P4'/n$       | $\leftarrow$       | 85.3.722     | $P4'/n$        | III  |
| 85.62         | $P4/n'$       | $\leftarrow$       | 85.4.723     | $P4/n'$        | III  |
| 85.63         | $P4'/n'$      | $\leftarrow$       | 85.5.724     | $P4'/n'$       | III  |
| 85.64         | $P_c4/n$      | $\leftarrow$       | 85.6.725     | $P_{2c}4/n$    | IV   |
| 85.65         | $P_C4/n$      | $\leftarrow$       | 83.10.712    | $P_P4/m'$      | IV   |
| 85.66         | $P_I4/n$      | $\leftarrow$       | 87.8.740     | $I_P4/m'$      | IV   |
| 86.67         | $P4_2/n$      | $\leftarrow$       | 86.1.727     | $P4_2/n$       | I    |
| 86.68         | $P4_2/n1'$    | $\leftarrow$       | 86.2.728     | $P4_2/n1'$     | II   |
| 86.69         | $P4'_2/n$     | $\leftarrow$       | 86.3.729     | $P4'_2/n$      | III  |
| 86.70         | $P4_2/n'$     | $\leftarrow$       | 86.4.730     | $P4_2/n'$      | III  |
| 86.71         | $P4'_2/n'$    | $\leftarrow$       | 86.5.731     | $P4'_2/n'$     | III  |
| 86.72         | $P_c4_2/n$    | $\leftarrow$       | 85.7.726     | $P_{2c}4'/n$   | IV   |
| 86.73         | $P_C4_2/n$    | $\leftarrow$       | 84.7.719     | $P_P4_2/m'$    | IV   |
| 86.74         | $P_I4_2/n$    | $\leftarrow$       | 87.9.741     | $I_P4'/m'$     | IV   |
| 87.75         | $I4/m$        | $\leftarrow$       | 87.1.733     | $I4/m$         | I    |
| 87.76         | $I4/m1'$      | $\leftarrow$       | 87.2.734     | $I4/m1'$       | II   |
| 87.77         | $I4'/m$       | $\leftarrow$       | 87.3.735     | $I4'/m$        | III  |
| 87.78         | $I4/m'$       | $\leftarrow$       | 87.4.736     | $I4/m'$        | III  |
| 87.79         | $I4'/m'$      | $\leftarrow$       | 87.5.737     | $I4'/m'$       | III  |
| 87.80         | $I_c4/m$      | $\leftarrow$       | 83.8.710     | $P_I4/m$       | IV   |
| 88.81         | $I4_1/a$      | $\leftarrow$       | 88.1.742     | $I4_1/a$       | I    |
| 88.82         | $I4_1/a1'$    | $\leftarrow$       | 88.2.743     | $I4_1/a1'$     | II   |
| 88.83         | $I4'_1/a$     | $\leftarrow$       | 88.3.744     | $I4'_1/a$      | III  |
| 88.84         | $I4_1/a'$     | $\leftarrow$       | 88.4.745     | $I4_1/a'$      | III  |
| 88.85         | $I4'_1/a'$    | $\leftarrow$       | 88.5.746     | $I4'_1/a'$     | III  |
| 88.86         | $I_c4_1/a$    | $\leftarrow$       | 86.6.732     | $P_I4_2/n$     | IV   |
| 89.87         | $P422$        | $\leftarrow$       | 89.1.747     | $P422$         | I    |
| 89.88         | $P4221'$      | $\leftarrow$       | 89.2.748     | $P4221'$       | II   |
| 89.89         | $P4'22'$      | $\leftarrow$       | 89.3.749     | $P4'22'$       | III  |
| 89.90         | $P42'2'$      | $\leftarrow$       | 89.4.750     | $P42'2'$       | III  |
| 89.91         | $P4'2'2$      | $\leftarrow$       | 89.5.751     | $P4'2'2$       | III  |
| 89.92         | $P_c422$      | $\leftarrow$       | 89.6.752     | $P_{2c}422$    | IV   |
| 89.93         | $P_C422$      | $\leftarrow$       | 89.7.753     | $P_P422$       | IV   |
| 89.94         | $P_I422$      | $\leftarrow$       | 97.6.810     | $I_P422$       | IV   |
| 90.95         | $P42_12$      | $\leftarrow$       | 90.1.757     | $P42_12$       | I    |
| 90.96         | $P42_121'$    | $\leftarrow$       | 90.2.758     | $P42_121'$     | II   |
| 90.97         | $P4'2_12'$    | $\leftarrow$       | 90.3.759     | $P4'2_12'$     | III  |
| 90.98         | $P42'_12'$    | $\leftarrow$       | 90.4.760     | $P42'_12'$     | III  |
| 90.99         | $P4'2'_12$    | $\leftarrow$       | 90.5.761     | $P4'2'_12$     | III  |
| 90.100        | $P_c42_12$    | $\leftarrow$       | 90.6.762     | $P_{2c}42_12$  | IV   |
| 90.101        | $P_C42_12$    | $\leftarrow$       | 89.10.756    | $P_P4'22'$     | IV   |
| 90.102        | $P_I42_12$    | $\leftarrow$       | 97.8.812     | $I_P42'2'$     | IV   |
| 91.103        | $P4_122$      | $\leftarrow$       | 91.1.764     | $P4_122$       | I    |
| 91.104        | $P4_1221'$    | $\leftarrow$       | 91.2.765     | $P4_1221'$     | II   |
| 91.105        | $P4'_122'$    | $\leftarrow$       | 91.3.766     | $P4'_122'$     | III  |
| 91.106        | $P4_12'2'$    | $\leftarrow$       | 91.4.767     | $P4_12'2'$     | III  |
| 91.107        | $P4'_12'2$    | $\leftarrow$       | 91.5.768     | $P4'_12'2$     | III  |
| 91.108        | $P_c4_122$    | $\leftarrow$       | 93.6.781     | $P_{2c}4_222'$ | IV   |
| 91.109        | $P_C4_122$    | $\leftarrow$       | 91.6.769     | $P_P4_122$     | IV   |
| 91.110        | $P_I4_122$    | $\leftarrow$       | 98.6.819     | $I_P4_122$     | IV   |
| 92.111        | $P4_12_12$    | $\leftarrow$       | 92.1.771     | $P4_12_12$     | I    |
| 92.112        | $P4_12_121'$  | $\leftarrow$       | 92.2.772     | $P4_12_121'$   | II   |
| 92.113        | $P4'_12_12'$  | $\leftarrow$       | 92.3.773     | $P4'_12_12'$   | III  |

| BNS<br>Number | BNS<br>Symbol | BNS (BC)<br>Symbol | OG<br>Number | OG<br>Symbol      | Type |
|---------------|---------------|--------------------|--------------|-------------------|------|
| 92.114        | $P4_12'_12'$  | $\leftarrow$       | 92.4.774     | $P4_12'_12'$      | III  |
| 92.115        | $P4'_12'_12$  | $\leftarrow$       | 92.5.775     | $P4'_12'_12$      | III  |
| 92.116        | $P_c4_12_12$  | $\leftarrow$       | 94.6.791     | $P_{2c}4_22_12$   | IV   |
| 92.117        | $P_C4_12_12$  | $\leftarrow$       | 91.7.770     | $P_P4'_122'$      | IV   |
| 92.118        | $P_I4_12_12$  | $\leftarrow$       | 98.8.821     | $I_P4_12'2'$      | IV   |
| 93.119        | $P4_222$      | $\leftarrow$       | 93.1.776     | $P4_222$          | I    |
| 93.120        | $P4_2221'$    | $\leftarrow$       | 93.2.777     | $P4_2221'$        | II   |
| 93.121        | $P4'_222'$    | $\leftarrow$       | 93.3.778     | $P4'_222'$        | III  |
| 93.122        | $P4_22'2'$    | $\leftarrow$       | 93.4.779     | $P4_22'2'$        | III  |
| 93.123        | $P4'_22'2$    | $\leftarrow$       | 93.5.780     | $P4'_22'2$        | III  |
| 93.124        | $P_c4_222$    | $\leftarrow$       | 89.9.755     | $P_{2c}4'22'$     | IV   |
| 93.125        | $P_C4_222$    | $\leftarrow$       | 93.7.782     | $P_P4_222$        | IV   |
| 93.126        | $P_I4_222$    | $\leftarrow$       | 97.7.811     | $I_P4'22'$        | IV   |
| 94.127        | $P4_22_12$    | $\leftarrow$       | 94.1.786     | $P4_22_12$        | I    |
| 94.128        | $P4_22_121'$  | $\leftarrow$       | 94.2.787     | $P4_22_121'$      | II   |
| 94.129        | $P4'_22_12'$  | $\leftarrow$       | 94.3.788     | $P4'_22_12'$      | III  |
| 94.130        | $P4_22'_12'$  | $\leftarrow$       | 94.4.789     | $P4_22'_12'$      | III  |
| 94.131        | $P4'_22'_12$  | $\leftarrow$       | 94.5.790     | $P4'_22'_12$      | III  |
| 94.132        | $P_c4_22_12$  | $\leftarrow$       | 90.7.763     | $P_{2c}4'2'_12$   | IV   |
| 94.133        | $P_C4_22_12$  | $\leftarrow$       | 93.10.785    | $P_P4'_222'$      | IV   |
| 94.134        | $P_I4_22_12$  | $\leftarrow$       | 97.9.813     | $I_P4'2'2$        | IV   |
| 95.135        | $P4_322$      | $\leftarrow$       | 95.1.793     | $P4_322$          | I    |
| 95.136        | $P4_3221'$    | $\leftarrow$       | 95.2.794     | $P4_3221'$        | II   |
| 95.137        | $P4'_322'$    | $\leftarrow$       | 95.3.795     | $P4'_322'$        | III  |
| 95.138        | $P4_32'2'$    | $\leftarrow$       | 95.4.796     | $P4_32'2'$        | III  |
| 95.139        | $P4'_32'2$    | $\leftarrow$       | 95.5.797     | $P4'_32'2$        | III  |
| 95.140        | $P_c4_322$    | $\leftarrow$       | 93.9.784     | $P_{2c}4'_222$    | IV   |
| 95.141        | $P_C4_322$    | $\leftarrow$       | 95.6.798     | $P_P4_322$        | IV   |
| 95.142        | $P_I4_322$    | $\leftarrow$       | 98.7.820     | $I_P4'_122'$      | IV   |
| 96.143        | $P4_32_12$    | $\leftarrow$       | 96.1.800     | $P4_32_12$        | I    |
| 96.144        | $P4_32_121'$  | $\leftarrow$       | 96.2.801     | $P4_32_121'$      | II   |
| 96.145        | $P4'_32_12'$  | $\leftarrow$       | 96.3.802     | $P4'_32_12'$      | III  |
| 96.146        | $P4_32'_12'$  | $\leftarrow$       | 96.4.803     | $P4_32'_12'$      | III  |
| 96.147        | $P4'_32'_12$  | $\leftarrow$       | 96.5.804     | $P4'_32'_12$      | III  |
| 96.148        | $P_c4_32_12$  | $\leftarrow$       | 94.7.792     | $P_{2c}4'_22'_12$ | IV   |
| 96.149        | $P_C4_32_12$  | $\leftarrow$       | 95.7.799     | $P_P4'_322'$      | IV   |
| 96.150        | $P_I4_32_12$  | $\leftarrow$       | 98.9.822     | $I_P4'_12'2$      | IV   |
| 97.151        | $I422$        | $\leftarrow$       | 97.1.805     | $I422$            | I    |
| 97.152        | $I4221'$      | $\leftarrow$       | 97.2.806     | $I4221'$          | II   |
| 97.153        | $I4'22'$      | $\leftarrow$       | 97.3.807     | $I4'22'$          | III  |
| 97.154        | $I42'2'$      | $\leftarrow$       | 97.4.808     | $I42'2'$          | III  |
| 97.155        | $I4'2'2$      | $\leftarrow$       | 97.5.809     | $I4'2'2$          | III  |
| 97.156        | $I_c422$      | $\leftarrow$       | 89.8.754     | $P_I422$          | IV   |
| 98.157        | $I4_122$      | $\leftarrow$       | 98.1.814     | $I4_122$          | I    |
| 98.158        | $I4_1221'$    | $\leftarrow$       | 98.2.815     | $I4_1221'$        | II   |
| 98.159        | $I4'_122'$    | $\leftarrow$       | 98.3.816     | $I4'_122'$        | III  |
| 98.160        | $I4_12'2'$    | $\leftarrow$       | 98.4.817     | $I4_12'2'$        | III  |
| 98.161        | $I4'_12'2$    | $\leftarrow$       | 98.5.818     | $I4'_12'2$        | III  |
| 98.162        | $I_c4_122$    | $\leftarrow$       | 93.8.783     | $P_I4_222'$       | IV   |
| 99.163        | $P4mm$        | $\leftarrow$       | 99.1.823     | $P4mm$            | I    |
| 99.164        | $P4mm1'$      | $\leftarrow$       | 99.2.824     | $P4mm1'$          | II   |
| 99.165        | $P4'm'm$      | $\leftarrow$       | 99.3.825     | $P4'm'm$          | III  |
| 99.166        | $P4'mm'$      | $\leftarrow$       | 99.4.826     | $P4'mm'$          | III  |
| 99.167        | $P4m'm'$      | $\leftarrow$       | 99.5.827     | $P4m'm'$          | III  |
| 99.168        | $P_c4mm$      | $\leftarrow$       | 99.6.828     | $P_{2c}4mm$       | IV   |

| BNS<br>Number | BNS<br>Symbol | BNS (BC)<br>Symbol | OG<br>Number | OG<br>Symbol  | Type |
|---------------|---------------|--------------------|--------------|---------------|------|
| 99.169        | $P_C4mm$      | $\leftarrow$       | 99.7.829     | $P_P4mm$      | IV   |
| 99.170        | $P_I4mm$      | $\leftarrow$       | 107.6.888    | $I_P4mm$      | IV   |
| 100.171       | $P4bm$        | $\leftarrow$       | 100.1.836    | $P4bm$        | I    |
| 100.172       | $P4bm1'$      | $\leftarrow$       | 100.2.837    | $P4bm1'$      | II   |
| 100.173       | $P4'b'm$      | $\leftarrow$       | 100.3.838    | $P4'b'm$      | III  |
| 100.174       | $P4'bm'$      | $\leftarrow$       | 100.4.839    | $P4'bm'$      | III  |
| 100.175       | $P4b'm'$      | $\leftarrow$       | 100.5.840    | $P4b'm'$      | III  |
| 100.176       | $P_c4bm$      | $\leftarrow$       | 100.6.841    | $P_{2c}4bm$   | IV   |
| 100.177       | $P_C4bm$      | $\leftarrow$       | 99.12.834    | $P_P4'mm'$    | IV   |
| 100.178       | $P_I4bm$      | $\leftarrow$       | 108.6.897    | $I_P4cm$      | IV   |
| 101.179       | $P4_2cm$      | $\leftarrow$       | 101.1.845    | $P4_2cm$      | I    |
| 101.180       | $P4_2cm1'$    | $\leftarrow$       | 101.2.846    | $P4_2cm1'$    | II   |
| 101.181       | $P4'_2c'm$    | $\leftarrow$       | 101.3.847    | $P4'_2c'm$    | III  |
| 101.182       | $P4'_2cm'$    | $\leftarrow$       | 101.4.848    | $P4'_2cm'$    | III  |
| 101.183       | $P4_2c'm'$    | $\leftarrow$       | 101.5.849    | $P4_2c'm'$    | III  |
| 101.184       | $P_c4_2cm$    | $\leftarrow$       | 99.9.831     | $P_{2c}4'm'm$ | IV   |
| 101.185       | $P_C4_2cm$    | $\leftarrow$       | 105.6.876    | $P_P4_2mc$    | IV   |
| 101.186       | $P_I4_2cm$    | $\leftarrow$       | 108.7.898    | $I_P4'c'm$    | IV   |
| 102.187       | $P4_2nm$      | $\leftarrow$       | 102.1.852    | $P4_2nm$      | I    |
| 102.188       | $P4_2nm1'$    | $\leftarrow$       | 102.2.853    | $P4_2nm1'$    | II   |
| 102.189       | $P4'_2n'm$    | $\leftarrow$       | 102.3.854    | $P4'_2n'm$    | III  |
| 102.190       | $P4'_2nm'$    | $\leftarrow$       | 102.4.855    | $P4'_2nm'$    | III  |
| 102.191       | $P4_2n'm'$    | $\leftarrow$       | 102.5.856    | $P4_2n'm'$    | III  |
| 102.192       | $P_c4_2nm$    | $\leftarrow$       | 100.7.842    | $P_{2c}4'b'm$ | IV   |
| 102.193       | $P_C4_2nm$    | $\leftarrow$       | 105.7.877    | $P_P4'_2mc'$  | IV   |
| 102.194       | $P_I4_2nm$    | $\leftarrow$       | 107.7.889    | $I_P4'm'm$    | IV   |
| 103.195       | $P4cc$        | $\leftarrow$       | 103.1.859    | $P4cc$        | I    |
| 103.196       | $P4cc1'$      | $\leftarrow$       | 103.2.860    | $P4cc1'$      | II   |
| 103.197       | $P4'c'c$      | $\leftarrow$       | 103.3.861    | $P4'c'c$      | III  |
| 103.198       | $P4'cc'$      | $\leftarrow$       | 103.4.862    | $P4'cc'$      | III  |
| 103.199       | $P4c'c'$      | $\leftarrow$       | 103.5.863    | $P4c'c'$      | III  |
| 103.200       | $P_c4cc$      | $\leftarrow$       | 99.11.833    | $P_{2c}4m'm'$ | IV   |
| 103.201       | $P_C4cc$      | $\leftarrow$       | 103.6.864    | $P_P4cc$      | IV   |
| 103.202       | $P_I4cc$      | $\leftarrow$       | 108.9.900    | $I_P4c'm'$    | IV   |
| 104.203       | $P4nc$        | $\leftarrow$       | 104.1.866    | $P4nc$        | I    |
| 104.204       | $P4nc1'$      | $\leftarrow$       | 104.2.867    | $P4nc1'$      | II   |
| 104.205       | $P4'n'c$      | $\leftarrow$       | 104.3.868    | $P4'n'c$      | III  |
| 104.206       | $P4'nc'$      | $\leftarrow$       | 104.4.869    | $P4'nc'$      | III  |
| 104.207       | $P4n'c'$      | $\leftarrow$       | 104.5.870    | $P4n'c'$      | III  |
| 104.208       | $P_c4nc$      | $\leftarrow$       | 100.9.844    | $P_{2c}4b'm'$ | IV   |
| 104.209       | $P_C4nc$      | $\leftarrow$       | 103.7.865    | $P_P4'cc'$    | IV   |
| 104.210       | $P_I4nc$      | $\leftarrow$       | 107.9.891    | $I_P4m'm'$    | IV   |
| 105.211       | $P4_2mc$      | $\leftarrow$       | 105.1.871    | $P4_2mc$      | I    |
| 105.212       | $P4_2mc1'$    | $\leftarrow$       | 105.2.872    | $P4_2mc1'$    | II   |
| 105.213       | $P4'_2m'c$    | $\leftarrow$       | 105.3.873    | $P4'_2m'c$    | III  |
| 105.214       | $P4'_2mc'$    | $\leftarrow$       | 105.4.874    | $P4'_2mc'$    | III  |
| 105.215       | $P4_2m'c'$    | $\leftarrow$       | 105.5.875    | $P4_2m'c'$    | III  |
| 105.216       | $P_c4_2mc$    | $\leftarrow$       | 99.10.832    | $P_{2c}4'mm'$ | IV   |
| 105.217       | $P_C4_2mc$    | $\leftarrow$       | 101.6.850    | $P_P4_2cm$    | IV   |
| 105.218       | $P_I4_2mc$    | $\leftarrow$       | 107.8.890    | $I_P4'mm'$    | IV   |
| 106.219       | $P4_2bc$      | $\leftarrow$       | 106.1.878    | $P4_2bc$      | I    |
| 106.220       | $P4_2bc1'$    | $\leftarrow$       | 106.2.879    | $P4_2bc1'$    | II   |
| 106.221       | $P4'_2b'c$    | $\leftarrow$       | 106.3.880    | $P4'_2b'c$    | III  |
| 106.222       | $P4'_2bc'$    | $\leftarrow$       | 106.4.881    | $P4'_2bc'$    | III  |
| 106.223       | $P4_2b'c'$    | $\leftarrow$       | 106.5.882    | $P4_2b'c'$    | III  |

| BNS<br>Number | BNS<br>Symbol    | BNS (BC)<br>Symbol | OG<br>Number | OG<br>Symbol        | Type |
|---------------|------------------|--------------------|--------------|---------------------|------|
| 106.224       | $P_c4_2bc$       | $\leftarrow$       | 100.8.843    | $P_{2c}4'bm'$       | IV   |
| 106.225       | $P_C4_2bc$       | $\leftarrow$       | 101.7.851    | $P_P4'_2cm'$        | IV   |
| 106.226       | $P_I4_2bc$       | $\leftarrow$       | 108.8.899    | $I_P4'_cm'$         | IV   |
| 107.227       | $I4mm$           | $\leftarrow$       | 107.1.883    | $I4mm$              | I    |
| 107.228       | $I4mm1'$         | $\leftarrow$       | 107.2.884    | $I4mm1'$            | II   |
| 107.229       | $I4'm'm$         | $\leftarrow$       | 107.3.885    | $I4'm'm$            | III  |
| 107.230       | $I4'mm'$         | $\leftarrow$       | 107.4.886    | $I4'mm'$            | III  |
| 107.231       | $I4m'm'$         | $\leftarrow$       | 107.5.887    | $I4m'm'$            | III  |
| 107.232       | $I_c4mm$         | $\leftarrow$       | 99.8.830     | $P_I4mm$            | IV   |
| 108.233       | $I4cm$           | $\leftarrow$       | 108.1.892    | $I4cm$              | I    |
| 108.234       | $I4cm1'$         | $\leftarrow$       | 108.2.893    | $I4cm1'$            | II   |
| 108.235       | $I4'c'm$         | $\leftarrow$       | 108.3.894    | $I4'c'm$            | III  |
| 108.236       | $I4'cm'$         | $\leftarrow$       | 108.4.895    | $I4'cm'$            | III  |
| 108.237       | $I4c'm'$         | $\leftarrow$       | 108.5.896    | $I4c'm'$            | III  |
| 108.238       | $I_c4cm$         | $\leftarrow$       | 99.13.835    | $P_I4m'm'$          | IV   |
| 109.239       | $I4_1md$         | $\leftarrow$       | 109.1.901    | $I4_1md$            | I    |
| 109.240       | $I4_1md1'$       | $\leftarrow$       | 109.2.902    | $I4_1md1'$          | II   |
| 109.241       | $I4'_1m'd$       | $\leftarrow$       | 109.3.903    | $I4'_1m'd$          | III  |
| 109.242       | $I4'_1md'$       | $\leftarrow$       | 109.4.904    | $I4'_1md'$          | III  |
| 109.243       | $I4_1m'd'$       | $\leftarrow$       | 109.5.905    | $I4_1m'd'$          | III  |
| 109.244       | $I_c4_1md$       | $\leftarrow$       | 102.6.857    | $P_I4_2nm$          | IV   |
| 110.245       | $I4_1cd$         | $\leftarrow$       | 110.1.906    | $I4_1cd$            | I    |
| 110.246       | $I4_1cd1'$       | $\leftarrow$       | 110.2.907    | $I4_1cd1'$          | II   |
| 110.247       | $I4'_1c'd$       | $\leftarrow$       | 110.3.908    | $I4'_1c'd$          | III  |
| 110.248       | $I4'_1cd'$       | $\leftarrow$       | 110.4.909    | $I4'_1cd'$          | III  |
| 110.249       | $I4_1c'd'$       | $\leftarrow$       | 110.5.910    | $I4_1c'd'$          | III  |
| 110.250       | $I_c4_1cd$       | $\leftarrow$       | 102.7.858    | $P_I4_2n'm'$        | IV   |
| 111.251       | $P\bar{4}2m$     | $\leftarrow$       | 111.1.911    | $P\bar{4}2m$        | I    |
| 111.252       | $P\bar{4}2m1'$   | $\leftarrow$       | 111.2.912    | $P\bar{4}2m1'$      | II   |
| 111.253       | $P\bar{4}'2'm$   | $\leftarrow$       | 111.3.913    | $P\bar{4}'2'm$      | III  |
| 111.254       | $P\bar{4}'2m'$   | $\leftarrow$       | 111.4.914    | $P\bar{4}'2m'$      | III  |
| 111.255       | $P\bar{4}2'm'$   | $\leftarrow$       | 111.5.915    | $P\bar{4}2'm'$      | III  |
| 111.256       | $P_c\bar{4}2m$   | $\leftarrow$       | 111.6.916    | $P_{2c}\bar{4}2m$   | IV   |
| 111.257       | $P_C\bar{4}2m$   | $\leftarrow$       | 115.7.947    | $P_P\bar{4}m2$      | IV   |
| 111.258       | $P_I\bar{4}2m$   | $\leftarrow$       | 121.6.990    | $I_P\bar{4}2m$      | IV   |
| 112.259       | $P\bar{4}2c$     | $\leftarrow$       | 112.1.922    | $P\bar{4}2c$        | I    |
| 112.260       | $P\bar{4}2c1'$   | $\leftarrow$       | 112.2.923    | $P\bar{4}2c1'$      | II   |
| 112.261       | $P\bar{4}'2'c$   | $\leftarrow$       | 112.3.924    | $P\bar{4}'2'c$      | III  |
| 112.262       | $P\bar{4}'2c'$   | $\leftarrow$       | 112.4.925    | $P\bar{4}'2c'$      | III  |
| 112.263       | $P\bar{4}2'c'$   | $\leftarrow$       | 112.5.926    | $P\bar{4}2'c'$      | III  |
| 112.264       | $P_c\bar{4}2c$   | $\leftarrow$       | 111.9.919    | $P_{2c}\bar{4}2'm'$ | IV   |
| 112.265       | $P_C\bar{4}2c$   | $\leftarrow$       | 116.6.956    | $P_P\bar{4}c2$      | IV   |
| 112.266       | $P_I\bar{4}2c$   | $\leftarrow$       | 121.8.992    | $I_P\bar{4}'2m'$    | IV   |
| 113.267       | $P\bar{4}2_1m$   | $\leftarrow$       | 113.1.929    | $P\bar{4}2_1m$      | I    |
| 113.268       | $P\bar{4}2_1m1'$ | $\leftarrow$       | 113.2.930    | $P\bar{4}2_1m1'$    | II   |
| 113.269       | $P\bar{4}'2'_1m$ | $\leftarrow$       | 113.3.931    | $P\bar{4}'2'_1m$    | III  |
| 113.270       | $P\bar{4}'2_1m'$ | $\leftarrow$       | 113.4.932    | $P\bar{4}'2_1m'$    | III  |
| 113.271       | $P\bar{4}2'_1m'$ | $\leftarrow$       | 113.5.933    | $P\bar{4}2'_1m'$    | III  |
| 113.272       | $P_c\bar{4}2_1m$ | $\leftarrow$       | 113.6.934    | $P_{2c}\bar{4}2_1m$ | IV   |
| 113.273       | $P_C\bar{4}2_1m$ | $\leftarrow$       | 115.10.950   | $P_P\bar{4}'m2'$    | IV   |
| 113.274       | $P_I\bar{4}2_1m$ | $\leftarrow$       | 121.7.991    | $I_P\bar{4}'2'm$    | IV   |
| 114.275       | $P\bar{4}2_1c$   | $\leftarrow$       | 114.1.936    | $P\bar{4}2_1c$      | I    |
| 114.276       | $P\bar{4}2_1c1'$ | $\leftarrow$       | 114.2.937    | $P\bar{4}2_1c1'$    | II   |
| 114.277       | $P\bar{4}'2'_1c$ | $\leftarrow$       | 114.3.938    | $P\bar{4}'2'_1c$    | III  |
| 114.278       | $P\bar{4}'2_1c'$ | $\leftarrow$       | 114.4.939    | $P\bar{4}'2_1c'$    | III  |

| BNS<br>Number | BNS<br>Symbol    | BNS (BC)<br>Symbol | OG<br>Number | OG<br>Symbol          | Type |
|---------------|------------------|--------------------|--------------|-----------------------|------|
| 114.279       | $P\bar{4}2_1'c'$ | $\leftarrow$       | 114.5.940    | $P\bar{4}2_1'c'$      | III  |
| 114.280       | $P_c\bar{4}2_1c$ | $\leftarrow$       | 113.7.935    | $P_{2c}\bar{4}'2_1m'$ | IV   |
| 114.281       | $P_C\bar{4}2_1c$ | $\leftarrow$       | 116.7.957    | $P_P\bar{4}'c2'$      | IV   |
| 114.282       | $P_I\bar{4}2_1c$ | $\leftarrow$       | 121.9.993    | $I_P\bar{4}2'm'$      | IV   |
| 115.283       | $P4m2$           | $\leftarrow$       | 115.1.941    | $P4m2$                | I    |
| 115.284       | $P\bar{4}m21'$   | $\leftarrow$       | 115.2.942    | $P\bar{4}m21'$        | II   |
| 115.285       | $P\bar{4}'m'2$   | $\leftarrow$       | 115.3.943    | $P\bar{4}'m'2$        | III  |
| 115.286       | $P\bar{4}'m2'$   | $\leftarrow$       | 115.4.944    | $P\bar{4}'m2'$        | III  |
| 115.287       | $P\bar{4}m'2'$   | $\leftarrow$       | 115.5.945    | $P\bar{4}m'2'$        | III  |
| 115.288       | $P_c\bar{4}m2$   | $\leftarrow$       | 115.6.946    | $P_{2c}\bar{4}m2$     | IV   |
| 115.289       | $P_C\bar{4}m2$   | $\leftarrow$       | 111.7.917    | $P_P\bar{4}2m$        | IV   |
| 115.290       | $P_I\bar{4}m2$   | $\leftarrow$       | 119.6.976    | $I_P\bar{4}m2$        | IV   |
| 116.291       | $P4c2$           | $\leftarrow$       | 116.1.951    | $P4c2$                | I    |
| 116.292       | $P\bar{4}c21'$   | $\leftarrow$       | 116.2.952    | $P\bar{4}c21'$        | II   |
| 116.293       | $P\bar{4}'c'2$   | $\leftarrow$       | 116.3.953    | $P\bar{4}'c'2$        | III  |
| 116.294       | $P\bar{4}'c2'$   | $\leftarrow$       | 116.4.954    | $P\bar{4}'c2'$        | III  |
| 116.295       | $P\bar{4}c'2'$   | $\leftarrow$       | 116.5.955    | $P\bar{4}c'2'$        | III  |
| 116.296       | $P_c\bar{4}c2$   | $\leftarrow$       | 115.9.949    | $P_{2c}\bar{4}'m'2$   | IV   |
| 116.297       | $P_C\bar{4}c2$   | $\leftarrow$       | 112.6.927    | $P_P\bar{4}2c$        | IV   |
| 116.298       | $P_I\bar{4}c2$   | $\leftarrow$       | 120.6.983    | $I_P\bar{4}c2$        | IV   |
| 117.299       | $P4b2$           | $\leftarrow$       | 117.1.958    | $P4b2$                | I    |
| 117.300       | $P\bar{4}b21'$   | $\leftarrow$       | 117.2.959    | $P\bar{4}b21'$        | II   |
| 117.301       | $P\bar{4}'b'2$   | $\leftarrow$       | 117.3.960    | $P\bar{4}'b'2$        | III  |
| 117.302       | $P\bar{4}'b2'$   | $\leftarrow$       | 117.4.961    | $P\bar{4}'b2'$        | III  |
| 117.303       | $P\bar{4}b'2'$   | $\leftarrow$       | 117.5.962    | $P\bar{4}b'2'$        | III  |
| 117.304       | $P_c\bar{4}b2$   | $\leftarrow$       | 117.6.963    | $P_{2c}\bar{4}b2$     | IV   |
| 117.305       | $P_C\bar{4}b2$   | $\leftarrow$       | 111.10.920   | $P_P\bar{4}'2m'$      | IV   |
| 117.306       | $P_I\bar{4}b2$   | $\leftarrow$       | 120.7.984    | $I_P\bar{4}c'2'$      | IV   |
| 118.307       | $P4n2$           | $\leftarrow$       | 118.1.965    | $P4n2$                | I    |
| 118.308       | $P\bar{4}n21'$   | $\leftarrow$       | 118.2.966    | $P\bar{4}n21'$        | II   |
| 118.309       | $P\bar{4}'n'2$   | $\leftarrow$       | 118.3.967    | $P\bar{4}'n'2$        | III  |
| 118.310       | $P\bar{4}'n2'$   | $\leftarrow$       | 118.4.968    | $P\bar{4}'n2'$        | III  |
| 118.311       | $P\bar{4}n'2'$   | $\leftarrow$       | 118.5.969    | $P\bar{4}n'2'$        | III  |
| 118.312       | $P_c\bar{4}n2$   | $\leftarrow$       | 117.7.964    | $P_{2c}\bar{4}'b'2$   | IV   |
| 118.313       | $P_C\bar{4}n2$   | $\leftarrow$       | 112.7.928    | $P_P\bar{4}'2c'$      | IV   |
| 118.314       | $P_I\bar{4}n2$   | $\leftarrow$       | 119.7.977    | $I_P\bar{4}'m'2$      | IV   |
| 119.315       | $I4m2$           | $\leftarrow$       | 119.1.971    | $I4m2$                | I    |
| 119.316       | $I\bar{4}m21'$   | $\leftarrow$       | 119.2.972    | $I\bar{4}m21'$        | II   |
| 119.317       | $I\bar{4}'m'2$   | $\leftarrow$       | 119.3.973    | $I\bar{4}'m'2$        | III  |
| 119.318       | $I\bar{4}'m2'$   | $\leftarrow$       | 119.4.974    | $I\bar{4}'m2'$        | III  |
| 119.319       | $I\bar{4}m'2'$   | $\leftarrow$       | 119.5.975    | $I\bar{4}m'2'$        | III  |
| 119.320       | $I_c\bar{4}m2$   | $\leftarrow$       | 111.8.918    | $P_I\bar{4}2m$        | IV   |
| 120.321       | $I4c2$           | $\leftarrow$       | 120.1.978    | $I4c2$                | I    |
| 120.322       | $I\bar{4}c21'$   | $\leftarrow$       | 120.2.979    | $I\bar{4}c21'$        | II   |
| 120.323       | $I\bar{4}'c'2$   | $\leftarrow$       | 120.3.980    | $I\bar{4}'c'2$        | III  |
| 120.324       | $I\bar{4}'c2'$   | $\leftarrow$       | 120.4.981    | $I\bar{4}'c2'$        | III  |
| 120.325       | $I\bar{4}c'2'$   | $\leftarrow$       | 120.5.982    | $I\bar{4}c'2'$        | III  |
| 120.326       | $I_c\bar{4}c2$   | $\leftarrow$       | 111.11.921   | $P_I\bar{4}'2m'$      | IV   |
| 121.327       | $I42m$           | $\leftarrow$       | 121.1.985    | $I42m$                | I    |
| 121.328       | $I\bar{4}2m1'$   | $\leftarrow$       | 121.2.986    | $I\bar{4}2m1'$        | II   |
| 121.329       | $I\bar{4}'2'm$   | $\leftarrow$       | 121.3.987    | $I\bar{4}'2'm$        | III  |
| 121.330       | $I\bar{4}'2m'$   | $\leftarrow$       | 121.4.988    | $I\bar{4}'2m'$        | III  |
| 121.331       | $I\bar{4}2'm'$   | $\leftarrow$       | 121.5.989    | $I\bar{4}2'm'$        | III  |
| 121.332       | $I_c\bar{4}2m$   | $\leftarrow$       | 115.8.948    | $P_I\bar{4}m2$        | IV   |
| 122.333       | $I42d$           | $\leftarrow$       | 122.1.994    | $I42d$                | I    |

| BNS<br>Number | BNS<br>Symbol  | BNS (BC)<br>Symbol | OG<br>Number | OG<br>Symbol   | Type |
|---------------|----------------|--------------------|--------------|----------------|------|
| 122.334       | $I\bar{4}2d1'$ | $\leftarrow$       | 122.2.995    | $I\bar{4}2d1'$ | II   |
| 122.335       | $I\bar{4}'2'd$ | $\leftarrow$       | 122.3.996    | $I\bar{4}'2'd$ | III  |
| 122.336       | $I\bar{4}'2d'$ | $\leftarrow$       | 122.4.997    | $I\bar{4}'2d'$ | III  |
| 122.337       | $I\bar{4}2'd'$ | $\leftarrow$       | 122.5.998    | $I\bar{4}2'd'$ | III  |
| 122.338       | $I_c\bar{4}2d$ | $\leftarrow$       | 118.6.970    | $P_I\bar{4}n2$ | IV   |
| 123.339       | $P4/mmm$       | $\leftarrow$       | 123.1.999    | $P4/mmm$       | I    |
| 123.340       | $P4/mmm1'$     | $\leftarrow$       | 123.2.1000   | $P4/mmm1'$     | II   |
| 123.341       | $P4/m'mm$      | $\leftarrow$       | 123.3.1001   | $P4/m'mm$      | III  |
| 123.342       | $P4'/mm'm$     | $\leftarrow$       | 123.4.1002   | $P4'/mm'm$     | III  |
| 123.343       | $P4'/mmm'$     | $\leftarrow$       | 123.5.1003   | $P4'/mmm'$     | III  |
| 123.344       | $P4'/m'm'm$    | $\leftarrow$       | 123.6.1004   | $P4'/m'm'm$    | III  |
| 123.345       | $P4/mm'm'$     | $\leftarrow$       | 123.7.1005   | $P4/mm'm'$     | III  |
| 123.346       | $P4'/m'mm'$    | $\leftarrow$       | 123.8.1006   | $P4'/m'mm'$    | III  |
| 123.347       | $P4/m'm'm'$    | $\leftarrow$       | 123.9.1007   | $P4/m'm'm'$    | III  |
| 123.348       | $P_c4/mmm$     | $\leftarrow$       | 123.10.1008  | $P_{c4}/mmm$   | IV   |
| 123.349       | $P_C4/mmm$     | $\leftarrow$       | 123.11.1009  | $P_P4/mmm$     | IV   |
| 123.350       | $P_I4/mmm$     | $\leftarrow$       | 139.10.1188  | $I_P4/mmm$     | IV   |
| 124.351       | $P4/mcc$       | $\leftarrow$       | 124.1.1018   | $P4/mcc$       | I    |
| 124.352       | $P4/mcc1'$     | $\leftarrow$       | 124.2.1019   | $P4/mcc1'$     | II   |
| 124.353       | $P4/m'cc$      | $\leftarrow$       | 124.3.1020   | $P4/m'cc$      | III  |
| 124.354       | $P4'/mc'c$     | $\leftarrow$       | 124.4.1021   | $P4'/mc'c$     | III  |
| 124.355       | $P4'/mcc'$     | $\leftarrow$       | 124.5.1022   | $P4'/mcc'$     | III  |
| 124.356       | $P4'/m'c'c$    | $\leftarrow$       | 124.6.1023   | $P4'/m'c'c$    | III  |
| 124.357       | $P4/mc'c'$     | $\leftarrow$       | 124.7.1024   | $P4/mc'c'$     | III  |
| 124.358       | $P4'/m'cc'$    | $\leftarrow$       | 124.8.1025   | $P4'/m'cc'$    | III  |
| 124.359       | $P4/m'c'c'$    | $\leftarrow$       | 124.9.1026   | $P4/m'c'c'$    | III  |
| 124.360       | $P_c4/mcc$     | $\leftarrow$       | 123.15.1013  | $P_{c4}/mm'm'$ | IV   |
| 124.361       | $P_C4/mcc$     | $\leftarrow$       | 124.10.1027  | $P_P4/mcc$     | IV   |
| 124.362       | $P_I4/mcc$     | $\leftarrow$       | 140.10.1205  | $I_P4/mcm$     | IV   |
| 125.363       | $P4/nbm$       | $\leftarrow$       | 125.1.1031   | $P4/nbm$       | I    |
| 125.364       | $P4/nbm1'$     | $\leftarrow$       | 125.2.1032   | $P4/nbm1'$     | II   |
| 125.365       | $P4/n'bm$      | $\leftarrow$       | 125.3.1033   | $P4/n'bm$      | III  |
| 125.366       | $P4'/nb'm$     | $\leftarrow$       | 125.4.1034   | $P4'/nb'm$     | III  |
| 125.367       | $P4'/nbm'$     | $\leftarrow$       | 125.5.1035   | $P4'/nbm'$     | III  |
| 125.368       | $P4'/n'b'm$    | $\leftarrow$       | 125.6.1036   | $P4'/n'b'm$    | III  |
| 125.369       | $P4/nb'm'$     | $\leftarrow$       | 125.7.1037   | $P4/nb'm'$     | III  |
| 125.370       | $P4'/n'bm'$    | $\leftarrow$       | 125.8.1038   | $P4'/n'bm'$    | III  |
| 125.371       | $P4/n'b'm'$    | $\leftarrow$       | 125.9.1039   | $P4/n'b'm'$    | III  |
| 125.372       | $P_c4/nbm$     | $\leftarrow$       | 125.10.1040  | $P_{c4}/nbm$   | IV   |
| 125.373       | $P_C4/nbm$     | $\leftarrow$       | 123.18.1016  | $P_P4'/m'mm'$  | IV   |
| 125.374       | $P_I4/nbm$     | $\leftarrow$       | 140.17.1212  | $I_P4/m'c'm'$  | IV   |
| 126.375       | $P4/nnc$       | $\leftarrow$       | 126.1.1044   | $P4/nnc$       | I    |
| 126.376       | $P4/nnc1'$     | $\leftarrow$       | 126.2.1045   | $P4/nnc1'$     | II   |
| 126.377       | $P4/n'nc$      | $\leftarrow$       | 126.3.1046   | $P4/n'nc$      | III  |
| 126.378       | $P4'/nn'c$     | $\leftarrow$       | 126.4.1047   | $P4'/nn'c$     | III  |
| 126.379       | $P4'/nnc'$     | $\leftarrow$       | 126.5.1048   | $P4'/nnc'$     | III  |
| 126.380       | $P4'/n'n'c$    | $\leftarrow$       | 126.6.1049   | $P4'/n'n'c$    | III  |
| 126.381       | $P4/nn'c'$     | $\leftarrow$       | 126.7.1050   | $P4/nn'c'$     | III  |
| 126.382       | $P4'/n'nc'$    | $\leftarrow$       | 126.8.1051   | $P4'/n'nc'$    | III  |
| 126.383       | $P4/n'n'c'$    | $\leftarrow$       | 126.9.1052   | $P4/n'n'c'$    | III  |
| 126.384       | $P_c4/nnc$     | $\leftarrow$       | 125.13.1043  | $P_{c4}/nb'm'$ | IV   |
| 126.385       | $P_C4/nnc$     | $\leftarrow$       | 124.13.1030  | $P_P4'/m'cc'$  | IV   |
| 126.386       | $P_I4/nnc$     | $\leftarrow$       | 139.17.1195  | $I_P4/m'm'm'$  | IV   |
| 127.387       | $P4/mbm$       | $\leftarrow$       | 127.1.1053   | $P4/mbm$       | I    |
| 127.388       | $P4/mbm1'$     | $\leftarrow$       | 127.2.1054   | $P4/mbm1'$     | II   |
| 127.389       | $P4/m'bm$      | $\leftarrow$       | 127.3.1055   | $P4/m'bm$      | III  |

| BNS<br>Number | BNS<br>Symbol | BNS (BC)<br>Symbol | OG<br>Number | OG<br>Symbol   | Type |
|---------------|---------------|--------------------|--------------|----------------|------|
| 127.390       | $P4'/mb'm$    | $\leftarrow$       | 127.4.1056   | $P4'/mb'm$     | III  |
| 127.391       | $P4'/mbm'$    | $\leftarrow$       | 127.5.1057   | $P4'/mbm'$     | III  |
| 127.392       | $P4'/m'b'm$   | $\leftarrow$       | 127.6.1058   | $P4'/m'b'm$    | III  |
| 127.393       | $P4/mb'b'm'$  | $\leftarrow$       | 127.7.1059   | $P4/mb'b'm'$   | III  |
| 127.394       | $P4'/m'bm'$   | $\leftarrow$       | 127.8.1060   | $P4'/m'bm'$    | III  |
| 127.395       | $P4/m'b'm'$   | $\leftarrow$       | 127.9.1061   | $P4/m'b'm'$    | III  |
| 127.396       | $P_c4/mbm$    | $\leftarrow$       | 127.10.1062  | $P_{c4}/mbm$   | IV   |
| 127.397       | $P_C4/mbm$    | $\leftarrow$       | 123.17.1015  | $P_P4'/mmm'$   | IV   |
| 127.398       | $P_I4/mbm$    | $\leftarrow$       | 140.15.1210  | $I_P4/mc'm'$   | IV   |
| 128.399       | $P4/mnc$      | $\leftarrow$       | 128.1.1066   | $P4/mnc$       | I    |
| 128.400       | $P4/mnc1'$    | $\leftarrow$       | 128.2.1067   | $P4/mnc1'$     | II   |
| 128.401       | $P4/m'nc$     | $\leftarrow$       | 128.3.1068   | $P4/m'nc$      | III  |
| 128.402       | $P4'/mn'c$    | $\leftarrow$       | 128.4.1069   | $P4'/mn'c$     | III  |
| 128.403       | $P4'/mnc'$    | $\leftarrow$       | 128.5.1070   | $P4'/mnc'$     | III  |
| 128.404       | $P4'/m'n'c$   | $\leftarrow$       | 128.6.1071   | $P4'/m'n'c$    | III  |
| 128.405       | $P4/mn'c'$    | $\leftarrow$       | 128.7.1072   | $P4/mn'c'$     | III  |
| 128.406       | $P4'/m'nc'$   | $\leftarrow$       | 128.8.1073   | $P4'/m'nc'$    | III  |
| 128.407       | $P4/m'n'c'$   | $\leftarrow$       | 128.9.1074   | $P4/m'n'c'$    | III  |
| 128.408       | $P_c4/mnc$    | $\leftarrow$       | 127.13.1065  | $P_{c4}/mb'm'$ | IV   |
| 128.409       | $P_C4/mnc$    | $\leftarrow$       | 124.12.1029  | $P_P4'/mcc'$   | IV   |
| 128.410       | $P_I4/mnc$    | $\leftarrow$       | 139.15.1193  | $I_P4/mm'm'$   | IV   |
| 129.411       | $P4/nmm$      | $\leftarrow$       | 129.1.1075   | $P4/nmm$       | I    |
| 129.412       | $P4/nmm1'$    | $\leftarrow$       | 129.2.1076   | $P4/nmm1'$     | II   |
| 129.413       | $P4/n'mm$     | $\leftarrow$       | 129.3.1077   | $P4/n'mm$      | III  |
| 129.414       | $P4'/nm'm$    | $\leftarrow$       | 129.4.1078   | $P4'/nm'm$     | III  |
| 129.415       | $P4'/nmm'$    | $\leftarrow$       | 129.5.1079   | $P4'/nmm'$     | III  |
| 129.416       | $P4'/n'm'm$   | $\leftarrow$       | 129.6.1080   | $P4'/n'm'm$    | III  |
| 129.417       | $P4/nm'm'$    | $\leftarrow$       | 129.7.1081   | $P4/nm'm'$     | III  |
| 129.418       | $P4'/n'mm'$   | $\leftarrow$       | 129.8.1082   | $P4'/n'mm'$    | III  |
| 129.419       | $P4/n'm'm'$   | $\leftarrow$       | 129.9.1083   | $P4/n'm'm'$    | III  |
| 129.420       | $P_c4/nmm$    | $\leftarrow$       | 129.10.1084  | $P_{c4}/nmm$   | IV   |
| 129.421       | $P_C4/nmm$    | $\leftarrow$       | 123.16.1014  | $P_P4/m'mm$    | IV   |
| 129.422       | $P_I4/nmm$    | $\leftarrow$       | 139.11.1189  | $I_P4/m'mm$    | IV   |
| 130.423       | $P4/ncc$      | $\leftarrow$       | 130.1.1088   | $P4/ncc$       | I    |
| 130.424       | $P4/ncc1'$    | $\leftarrow$       | 130.2.1089   | $P4/ncc1'$     | II   |
| 130.425       | $P4/n'cc$     | $\leftarrow$       | 130.3.1090   | $P4/n'cc$      | III  |
| 130.426       | $P4'/nc'c$    | $\leftarrow$       | 130.4.1091   | $P4'/nc'c$     | III  |
| 130.427       | $P4'/ncc'$    | $\leftarrow$       | 130.5.1092   | $P4'/ncc'$     | III  |
| 130.428       | $P4'/n'c'c$   | $\leftarrow$       | 130.6.1093   | $P4'/n'c'c$    | III  |
| 130.429       | $P4/nc'c'$    | $\leftarrow$       | 130.7.1094   | $P4/nc'c'$     | III  |
| 130.430       | $P4'/n'cc'$   | $\leftarrow$       | 130.8.1095   | $P4'/n'cc'$    | III  |
| 130.431       | $P4/n'c'c'$   | $\leftarrow$       | 130.9.1096   | $P4/n'c'c'$    | III  |
| 130.432       | $P_c4/ncc$    | $\leftarrow$       | 129.13.1087  | $P_{c4}/nm'm'$ | IV   |
| 130.433       | $P_C4/ncc$    | $\leftarrow$       | 124.11.1028  | $P_P4/m'cc$    | IV   |
| 130.434       | $P_I4/ncc$    | $\leftarrow$       | 140.11.1206  | $I_P4/m'cm$    | IV   |
| 131.435       | $P4_2/mmc$    | $\leftarrow$       | 131.1.1097   | $P4_2/mmc$     | I    |
| 131.436       | $P4_2/mmc1'$  | $\leftarrow$       | 131.2.1098   | $P4_2/mmc1'$   | II   |
| 131.437       | $P4_2/m'mc$   | $\leftarrow$       | 131.3.1099   | $P4_2/m'mc$    | III  |
| 131.438       | $P4_2'/mm'c$  | $\leftarrow$       | 131.4.1100   | $P4_2'/mm'c$   | III  |
| 131.439       | $P4_2'/mmc'$  | $\leftarrow$       | 131.5.1101   | $P4_2'/mmc'$   | III  |
| 131.440       | $P4_2'/m'm'c$ | $\leftarrow$       | 131.6.1102   | $P4_2'/m'm'c$  | III  |
| 131.441       | $P4_2/mm'c'$  | $\leftarrow$       | 131.7.1103   | $P4_2/mm'c'$   | III  |
| 131.442       | $P4_2'/m'mc'$ | $\leftarrow$       | 131.8.1104   | $P4_2'/m'mc'$  | III  |
| 131.443       | $P4_2/m'm'c'$ | $\leftarrow$       | 131.9.1105   | $P4_2/m'm'c'$  | III  |
| 131.444       | $P_c4_2/mmc$  | $\leftarrow$       | 123.14.1012  | $P_{c4}'/mmm'$ | IV   |
| 131.445       | $P_C4_2/mmc$  | $\leftarrow$       | 132.10.1119  | $P_P4_2/mcm$   | IV   |



| BNS<br>Number | BNS<br>Symbol  | BNS (BC)<br>Symbol | OG<br>Number | OG<br>Symbol      | Type |
|---------------|----------------|--------------------|--------------|-------------------|------|
| 131.446       | $P_{I4_2}/mmc$ | $\leftarrow$       | 139.13.1191  | $I_{P4'}'/mmm'$   | IV   |
| 132.447       | $P4_2/mcm$     | $\leftarrow$       | 132.1.1110   | $P4_2/mcm$        | I    |
| 132.448       | $P4_2/mcm1'$   | $\leftarrow$       | 132.2.1111   | $P4_2/mcm1'$      | II   |
| 132.449       | $P4_2/m'cm$    | $\leftarrow$       | 132.3.1112   | $P4_2/m'cm$       | III  |
| 132.450       | $P4_2'/mc'm$   | $\leftarrow$       | 132.4.1113   | $P4_2'/mc'm$      | III  |
| 132.451       | $P4_2'/mcm'$   | $\leftarrow$       | 132.5.1114   | $P4_2'/mcm'$      | III  |
| 132.452       | $P4_2'/m'c'm$  | $\leftarrow$       | 132.6.1115   | $P4_2'/m'c'm$     | III  |
| 132.453       | $P4_2'/mc'm'$  | $\leftarrow$       | 132.7.1116   | $P4_2'/mc'm'$     | III  |
| 132.454       | $P4_2'/m'cm'$  | $\leftarrow$       | 132.8.1117   | $P4_2'/m'cm'$     | III  |
| 132.455       | $P4_2'/m'c'm'$ | $\leftarrow$       | 132.9.1118   | $P4_2'/m'c'm'$    | III  |
| 132.456       | $P_{c4_2}/mcm$ | $\leftarrow$       | 123.13.1011  | $P_{2c4'}'/mm'm$  | IV   |
| 132.457       | $P_{C4_2}/mcm$ | $\leftarrow$       | 131.10.1106  | $P_{P4_2}/mmc$    | IV   |
| 132.458       | $P_{I4_2}/mcm$ | $\leftarrow$       | 140.13.1208  | $I_{P4'}'/mcm'$   | IV   |
| 133.459       | $P4_2/nbc$     | $\leftarrow$       | 133.1.1123   | $P4_2/nbc$        | I    |
| 133.460       | $P4_2/nbc1'$   | $\leftarrow$       | 133.2.1124   | $P4_2/nbc1'$      | II   |
| 133.461       | $P4_2/n'bc$    | $\leftarrow$       | 133.3.1125   | $P4_2/n'bc$       | III  |
| 133.462       | $P4_2'/nb'c$   | $\leftarrow$       | 133.4.1126   | $P4_2'/nb'c$      | III  |
| 133.463       | $P4_2'/nbc'$   | $\leftarrow$       | 133.5.1127   | $P4_2'/nbc'$      | III  |
| 133.464       | $P4_2'/n'b'c$  | $\leftarrow$       | 133.6.1128   | $P4_2'/n'b'c$     | III  |
| 133.465       | $P4_2'/nb'c'$  | $\leftarrow$       | 133.7.1129   | $P4_2'/nb'c'$     | III  |
| 133.466       | $P4_2'/n'bc'$  | $\leftarrow$       | 133.8.1130   | $P4_2'/n'bc'$     | III  |
| 133.467       | $P4_2'/n'b'c'$ | $\leftarrow$       | 133.9.1131   | $P4_2'/n'b'c'$    | III  |
| 133.468       | $P_{c4_2}/nbc$ | $\leftarrow$       | 125.12.1042  | $P_{2c4'}'/nbm'$  | IV   |
| 133.469       | $P_{C4_2}/nbc$ | $\leftarrow$       | 132.13.1122  | $P_{P4_2}'/m'cm'$ | IV   |
| 133.470       | $P_{I4_2}/nbc$ | $\leftarrow$       | 140.14.1209  | $I_{P4'}'/m'c'm$  | IV   |
| 134.471       | $P4_2/nnm$     | $\leftarrow$       | 134.1.1132   | $P4_2/nnm$        | I    |
| 134.472       | $P4_2/nnm1'$   | $\leftarrow$       | 134.2.1133   | $P4_2/nnm1'$      | II   |
| 134.473       | $P4_2/n'nm$    | $\leftarrow$       | 134.3.1134   | $P4_2/n'nm$       | III  |
| 134.474       | $P4_2'/nn'm$   | $\leftarrow$       | 134.4.1135   | $P4_2'/nn'm$      | III  |
| 134.475       | $P4_2'/nnm'$   | $\leftarrow$       | 134.5.1136   | $P4_2'/nnm'$      | III  |
| 134.476       | $P4_2'/n'n'm$  | $\leftarrow$       | 134.6.1137   | $P4_2'/n'n'm$     | III  |
| 134.477       | $P4_2'/nn'm'$  | $\leftarrow$       | 134.7.1138   | $P4_2'/nn'm'$     | III  |
| 134.478       | $P4_2'/n'nm'$  | $\leftarrow$       | 134.8.1139   | $P4_2'/n'nm'$     | III  |
| 134.479       | $P4_2'/n'n'm'$ | $\leftarrow$       | 134.9.1140   | $P4_2'/n'n'm'$    | III  |
| 134.480       | $P_{c4_2}/nnm$ | $\leftarrow$       | 125.11.1041  | $P_{2c4'}'/nb'm$  | IV   |
| 134.481       | $P_{C4_2}/nnm$ | $\leftarrow$       | 131.13.1109  | $P_{P4_2}'/m'mc'$ | IV   |
| 134.482       | $P_{I4_2}/nnm$ | $\leftarrow$       | 139.14.1192  | $I_{P4'}'/m'm'm$  | IV   |
| 135.483       | $P4_2/mbc$     | $\leftarrow$       | 135.1.1143   | $P4_2/mbc$        | I    |
| 135.484       | $P4_2/mbc1'$   | $\leftarrow$       | 135.2.1144   | $P4_2/mbc1'$      | II   |
| 135.485       | $P4_2/m'bc$    | $\leftarrow$       | 135.3.1145   | $P4_2/m'bc$       | III  |
| 135.486       | $P4_2'/mb'c$   | $\leftarrow$       | 135.4.1146   | $P4_2'/mb'c$      | III  |
| 135.487       | $P4_2'/mbc'$   | $\leftarrow$       | 135.5.1147   | $P4_2'/mbc'$      | III  |
| 135.488       | $P4_2'/m'b'c$  | $\leftarrow$       | 135.6.1148   | $P4_2'/m'b'c$     | III  |
| 135.489       | $P4_2'/mb'c'$  | $\leftarrow$       | 135.7.1149   | $P4_2'/mb'c'$     | III  |
| 135.490       | $P4_2'/m'bc'$  | $\leftarrow$       | 135.8.1150   | $P4_2'/m'bc'$     | III  |
| 135.491       | $P4_2'/m'b'c'$ | $\leftarrow$       | 135.9.1151   | $P4_2'/m'b'c'$    | III  |
| 135.492       | $P_{c4_2}/mbc$ | $\leftarrow$       | 127.12.1064  | $P_{2c4'}'/mbm'$  | IV   |
| 135.493       | $P_{C4_2}/mbc$ | $\leftarrow$       | 132.12.1121  | $P_{P4_2}'/mcm'$  | IV   |
| 135.494       | $P_{I4_2}/mbc$ | $\leftarrow$       | 140.12.1207  | $I_{P4'}'/mc'm$   | IV   |
| 136.495       | $P4_2/mnm$     | $\leftarrow$       | 136.1.1152   | $P4_2/mnm$        | I    |
| 136.496       | $P4_2/mnm1'$   | $\leftarrow$       | 136.2.1153   | $P4_2/mnm1'$      | II   |
| 136.497       | $P4_2/m'nm$    | $\leftarrow$       | 136.3.1154   | $P4_2/m'nm$       | III  |
| 136.498       | $P4_2'/mn'm$   | $\leftarrow$       | 136.4.1155   | $P4_2'/mn'm$      | III  |
| 136.499       | $P4_2'/mnm'$   | $\leftarrow$       | 136.5.1156   | $P4_2'/mnm'$      | III  |
| 136.500       | $P4_2'/m'n'm$  | $\leftarrow$       | 136.6.1157   | $P4_2'/m'n'm$     | III  |
| 136.501       | $P4_2'/mn'm'$  | $\leftarrow$       | 136.7.1158   | $P4_2'/mn'm'$     | III  |

| BNS<br>Number | BNS<br>Symbol  | BNS (BC)<br>Symbol | OG<br>Number | OG<br>Symbol     | Type |
|---------------|----------------|--------------------|--------------|------------------|------|
| 136.502       | $P4_2'/m'nm'$  | ←                  | 136.8.1159   | $P4_2'/m'nm'$    | III  |
| 136.503       | $P4_2'/m'n'm'$ | ←                  | 136.9.1160   | $P4_2'/m'n'm'$   | III  |
| 136.504       | $P_c4_2/mnm$   | ←                  | 127.11.1063  | $P_{c4}'/mb'm$   | IV   |
| 136.505       | $P_C4_2/mnm$   | ←                  | 131.12.1108  | $P_P4_2/mm'm'c'$ | IV   |
| 136.506       | $P_I4_2/mnm$   | ←                  | 139.12.1190  | $I_P4'/mm'm$     | IV   |
| 137.507       | $P4_2/nmc$     | ←                  | 137.1.1161   | $P4_2/nmc$       | I    |
| 137.508       | $P4_2/nmc1'$   | ←                  | 137.2.1162   | $P4_2/nmc1'$     | II   |
| 137.509       | $P4_2/n'mc$    | ←                  | 137.3.1163   | $P4_2/n'mc$      | III  |
| 137.510       | $P4_2'/nm'c$   | ←                  | 137.4.1164   | $P4_2'/nm'c$     | III  |
| 137.511       | $P4_2'/nmc'$   | ←                  | 137.5.1165   | $P4_2'/nmc'$     | III  |
| 137.512       | $P4_2'/n'm'c$  | ←                  | 137.6.1166   | $P4_2'/n'm'c$    | III  |
| 137.513       | $P4_2'/nm'c'$  | ←                  | 137.7.1167   | $P4_2'/nm'c'$    | III  |
| 137.514       | $P4_2'/n'mc'$  | ←                  | 137.8.1168   | $P4_2'/n'mc'$    | III  |
| 137.515       | $P4_2'/n'm'c'$ | ←                  | 137.9.1169   | $P4_2'/n'm'c'$   | III  |
| 137.516       | $P_c4_2/nmc$   | ←                  | 129.12.1086  | $P_{c4}'/nmm'$   | IV   |
| 137.517       | $P_C4_2/nmc$   | ←                  | 132.11.1120  | $P_P4_2/m'cm$    | IV   |
| 137.518       | $P_I4_2/nmc$   | ←                  | 139.16.1194  | $I_P4'/m'mm'$    | IV   |
| 138.519       | $P4_2/ncm$     | ←                  | 138.1.1170   | $P4_2/ncm$       | I    |
| 138.520       | $P4_2/ncm1'$   | ←                  | 138.2.1171   | $P4_2/ncm1'$     | II   |
| 138.521       | $P4_2/n'cm$    | ←                  | 138.3.1172   | $P4_2/n'cm$      | III  |
| 138.522       | $P4_2'/nc'm$   | ←                  | 138.4.1173   | $P4_2'/nc'm$     | III  |
| 138.523       | $P4_2'/ncm'$   | ←                  | 138.5.1174   | $P4_2'/ncm'$     | III  |
| 138.524       | $P4_2'/n'c'm$  | ←                  | 138.6.1175   | $P4_2'/n'c'm$    | III  |
| 138.525       | $P4_2'/nc'm'$  | ←                  | 138.7.1176   | $P4_2'/nc'm'$    | III  |
| 138.526       | $P4_2'/n'cm'$  | ←                  | 138.8.1177   | $P4_2'/n'cm'$    | III  |
| 138.527       | $P4_2'/n'c'm'$ | ←                  | 138.9.1178   | $P4_2'/n'c'm'$   | III  |
| 138.528       | $P_c4_2/ncm$   | ←                  | 129.11.1085  | $P_{c4}'/nm'm$   | IV   |
| 138.529       | $P_C4_2/ncm$   | ←                  | 131.11.1107  | $P_P4_2/m'mc$    | IV   |
| 138.530       | $P_I4_2/ncm$   | ←                  | 140.16.1211  | $I_P4'/m'cm'$    | IV   |
| 139.531       | $I4/mmm$       | ←                  | 139.1.1179   | $I4/mmm$         | I    |
| 139.532       | $I4/mmm1'$     | ←                  | 139.2.1180   | $I4/mmm1'$       | II   |
| 139.533       | $I4/m'mm$      | ←                  | 139.3.1181   | $I4/m'mm$        | III  |
| 139.534       | $I4'/mm'm$     | ←                  | 139.4.1182   | $I4'/mm'm$       | III  |
| 139.535       | $I4'/mmm'$     | ←                  | 139.5.1183   | $I4'/mmm'$       | III  |
| 139.536       | $I4'/m'm'm$    | ←                  | 139.6.1184   | $I4'/m'm'm$      | III  |
| 139.537       | $I4'/mm'm'$    | ←                  | 139.7.1185   | $I4'/mm'm'$      | III  |
| 139.538       | $I4'/m'mm'$    | ←                  | 139.8.1186   | $I4'/m'mm'$      | III  |
| 139.539       | $I4'/m'm'm'$   | ←                  | 139.9.1187   | $I4'/m'm'm'$     | III  |
| 139.540       | $I_c4/mmm$     | ←                  | 123.12.1010  | $P_I4/mmm$       | IV   |
| 140.541       | $I4/mcm$       | ←                  | 140.1.1196   | $I4/mcm$         | I    |
| 140.542       | $I4/mcm1'$     | ←                  | 140.2.1197   | $I4/mcm1'$       | II   |
| 140.543       | $I4/m'cm$      | ←                  | 140.3.1198   | $I4/m'cm$        | III  |
| 140.544       | $I4'/mc'm$     | ←                  | 140.4.1199   | $I4'/mc'm$       | III  |
| 140.545       | $I4'/mcm'$     | ←                  | 140.5.1200   | $I4'/mcm'$       | III  |
| 140.546       | $I4'/m'c'm$    | ←                  | 140.6.1201   | $I4'/m'c'm$      | III  |
| 140.547       | $I4'/mc'm'$    | ←                  | 140.7.1202   | $I4'/mc'm'$      | III  |
| 140.548       | $I4'/m'cm'$    | ←                  | 140.8.1203   | $I4'/m'cm'$      | III  |
| 140.549       | $I4'/m'c'm'$   | ←                  | 140.9.1204   | $I4'/m'c'm'$     | III  |
| 140.550       | $I_c4/mcm$     | ←                  | 123.19.1017  | $P_I4/mm'm'$     | IV   |
| 141.551       | $I4_1/amd$     | ←                  | 141.1.1213   | $I4_1/amd$       | I    |
| 141.552       | $I4_1/amd1'$   | ←                  | 141.2.1214   | $I4_1/amd1'$     | II   |
| 141.553       | $I4_1/a'md$    | ←                  | 141.3.1215   | $I4_1/a'md$      | III  |
| 141.554       | $I4_1'/am'd$   | ←                  | 141.4.1216   | $I4_1'/am'd$     | III  |
| 141.555       | $I4_1'/amd'$   | ←                  | 141.5.1217   | $I4_1'/amd'$     | III  |
| 141.556       | $I4_1'/a'm'd$  | ←                  | 141.6.1218   | $I4_1'/a'm'd$    | III  |
| 141.557       | $I4_1'/am'd'$  | ←                  | 141.7.1219   | $I4_1'/am'd'$    | III  |

| BNS<br>Number | BNS<br>Symbol | BNS (BC)<br>Symbol | OG<br>Number | OG<br>Symbol    | Type |
|---------------|---------------|--------------------|--------------|-----------------|------|
| 141.558       | $I4_1'/a'md'$ | $\leftarrow$       | 141.8.1220   | $I4_1'/a'md'$   | III  |
| 141.559       | $I4_1/a'm'd'$ | $\leftarrow$       | 141.9.1221   | $I4_1/a'm'd'$   | III  |
| 141.560       | $I_c4_1/amd$  | $\leftarrow$       | 134.10.1141  | $P_I4_2/nnm$    | IV   |
| 142.561       | $I4_1/acd$    | $\leftarrow$       | 142.1.1222   | $I4_1/acd$      | I    |
| 142.562       | $I4_1/acd1'$  | $\leftarrow$       | 142.2.1223   | $I4_1/acd1'$    | II   |
| 142.563       | $I4_1/a'cd$   | $\leftarrow$       | 142.3.1224   | $I4_1/a'cd$     | III  |
| 142.564       | $I4_1'/ac'd$  | $\leftarrow$       | 142.4.1225   | $I4_1'/ac'd$    | III  |
| 142.565       | $I4_1'/acd'$  | $\leftarrow$       | 142.5.1226   | $I4_1'/acd'$    | III  |
| 142.566       | $I4_1'/a'c'd$ | $\leftarrow$       | 142.6.1227   | $I4_1'/a'c'd$   | III  |
| 142.567       | $I4_1/ac'd'$  | $\leftarrow$       | 142.7.1228   | $I4_1/ac'd'$    | III  |
| 142.568       | $I4_1'/a'cd'$ | $\leftarrow$       | 142.8.1229   | $I4_1'/a'cd'$   | III  |
| 142.569       | $I4_1/a'c'd'$ | $\leftarrow$       | 142.9.1230   | $I4_1/a'c'd'$   | III  |
| 142.570       | $I_c4_1/acd$  | $\leftarrow$       | 134.11.1142  | $P_I4_2/nn'm'$  | IV   |
| 143.1         | $P3$          | $\leftarrow$       | 143.1.1231   | $P3$            | I    |
| 143.2         | $P31'$        | $\leftarrow$       | 143.2.1232   | $P31'$          | II   |
| 143.3         | $P_c3$        | $\leftarrow$       | 143.3.1233   | $P_{2c}3$       | IV   |
| 144.4         | $P3_1$        | $\leftarrow$       | 144.1.1234   | $P3_1$          | I    |
| 144.5         | $P3_11'$      | $\leftarrow$       | 144.2.1235   | $P3_11'$        | II   |
| 144.6         | $P_c3_1$      | $\leftarrow$       | 145.3.1239   | $P_{2c}3_1$     | IV   |
| 145.7         | $P3_2$        | $\leftarrow$       | 145.1.1237   | $P3_2$          | I    |
| 145.8         | $P3_21'$      | $\leftarrow$       | 145.2.1238   | $P3_21'$        | II   |
| 145.9         | $P_c3_2$      | $\leftarrow$       | 144.3.1236   | $P_{2c}3_2$     | IV   |
| 146.10        | $R3$          | $\leftarrow$       | 146.1.1240   | $R3$            | I    |
| 146.11        | $R31'$        | $\leftarrow$       | 146.2.1241   | $R31'$          | II   |
| 146.12        | $R_I3$        | $\leftarrow$       | 146.3.1242   | $R_R3$          | IV   |
| 147.13        | $P\bar{3}$    | $\leftarrow$       | 147.1.1243   | $P\bar{3}$      | I    |
| 147.14        | $P\bar{3}1'$  | $\leftarrow$       | 147.2.1244   | $P\bar{3}1'$    | II   |
| 147.15        | $P\bar{3}'$   | $\leftarrow$       | 147.3.1245   | $P\bar{3}'$     | III  |
| 147.16        | $P_c\bar{3}$  | $\leftarrow$       | 147.4.1246   | $P_{2c}\bar{3}$ | IV   |
| 148.17        | $R\bar{3}$    | $\leftarrow$       | 148.1.1247   | $R\bar{3}$      | I    |
| 148.18        | $R\bar{3}1'$  | $\leftarrow$       | 148.2.1248   | $R\bar{3}1'$    | II   |
| 148.19        | $R\bar{3}'$   | $\leftarrow$       | 148.3.1249   | $R\bar{3}'$     | III  |
| 148.20        | $R_I\bar{3}$  | $\leftarrow$       | 148.4.1250   | $R_R\bar{3}$    | IV   |
| 149.21        | $P312$        | $\leftarrow$       | 149.1.1251   | $P312$          | I    |
| 149.22        | $P3121'$      | $\leftarrow$       | 149.2.1252   | $P3121'$        | II   |
| 149.23        | $P312'$       | $\leftarrow$       | 149.3.1253   | $P312'$         | III  |
| 149.24        | $P_c312$      | $\leftarrow$       | 149.4.1254   | $P_{2c}312$     | IV   |
| 150.25        | $P321$        | $\leftarrow$       | 150.1.1255   | $P321$          | I    |
| 150.26        | $P3211'$      | $\leftarrow$       | 150.2.1256   | $P3211'$        | II   |
| 150.27        | $P32'1$       | $\leftarrow$       | 150.3.1257   | $P32'1$         | III  |
| 150.28        | $P_c321$      | $\leftarrow$       | 150.4.1258   | $P_{2c}321$     | IV   |
| 151.29        | $P3_112$      | $\leftarrow$       | 151.1.1259   | $P3_112$        | I    |
| 151.30        | $P3_1121'$    | $\leftarrow$       | 151.2.1260   | $P3_1121'$      | II   |
| 151.31        | $P3_112'$     | $\leftarrow$       | 151.3.1261   | $P3_112'$       | III  |
| 151.32        | $P_c3_112$    | $\leftarrow$       | 153.4.1270   | $P_{2c}3_112'$  | IV   |
| 152.33        | $P3_121$      | $\leftarrow$       | 152.1.1263   | $P3_121$        | I    |
| 152.34        | $P3_1211'$    | $\leftarrow$       | 152.2.1264   | $P3_1211'$      | II   |
| 152.35        | $P3_12'1$     | $\leftarrow$       | 152.3.1265   | $P3_12'1$       | III  |
| 152.36        | $P_c3_121$    | $\leftarrow$       | 154.4.1274   | $P_{2c}3_12'1$  | IV   |
| 153.37        | $P3_212$      | $\leftarrow$       | 153.1.1267   | $P3_212$        | I    |
| 153.38        | $P3_2121'$    | $\leftarrow$       | 153.2.1268   | $P3_2121'$      | II   |
| 153.39        | $P3_212'$     | $\leftarrow$       | 153.3.1269   | $P3_212'$       | III  |
| 153.40        | $P_c3_212$    | $\leftarrow$       | 151.4.1262   | $P_{2c}3_212$   | IV   |
| 154.41        | $P3_221$      | $\leftarrow$       | 154.1.1271   | $P3_221$        | I    |
| 154.42        | $P3_2211'$    | $\leftarrow$       | 154.2.1272   | $P3_2211'$      | II   |

| BNS<br>Number | BNS<br>Symbol  | BNS (BC)<br>Symbol | OG<br>Number | OG<br>Symbol       | Type |
|---------------|----------------|--------------------|--------------|--------------------|------|
| 154.43        | $P3_22'1$      | $\leftarrow$       | 154.3.1273   | $P3_22'1$          | III  |
| 154.44        | $P_c3_221$     | $\leftarrow$       | 152.4.1266   | $P_{2c}3_221$      | IV   |
| 155.45        | $R32$          | $\leftarrow$       | 155.1.1275   | $R32$              | I    |
| 155.46        | $R321'$        | $\leftarrow$       | 155.2.1276   | $R321'$            | II   |
| 155.47        | $R32'$         | $\leftarrow$       | 155.3.1277   | $R32'$             | III  |
| 155.48        | $R_I32$        | $\leftarrow$       | 155.4.1278   | $R_R32$            | IV   |
| 156.49        | $P3m1$         | $\leftarrow$       | 156.1.1279   | $P3m1$             | I    |
| 156.50        | $P3m11'$       | $\leftarrow$       | 156.2.1280   | $P3m11'$           | II   |
| 156.51        | $P3m'1$        | $\leftarrow$       | 156.3.1281   | $P3m'1$            | III  |
| 156.52        | $P_c3m1$       | $\leftarrow$       | 156.4.1282   | $P_{2c}3m1$        | IV   |
| 157.53        | $P31m$         | $\leftarrow$       | 157.1.1284   | $P31m$             | I    |
| 157.54        | $P31m1'$       | $\leftarrow$       | 157.2.1285   | $P31m1'$           | II   |
| 157.55        | $P31m'$        | $\leftarrow$       | 157.3.1286   | $P31m'$            | III  |
| 157.56        | $P_c31m$       | $\leftarrow$       | 157.4.1287   | $P_{2c}31m$        | IV   |
| 158.57        | $P3c1$         | $\leftarrow$       | 158.1.1289   | $P3c1$             | I    |
| 158.58        | $P3c11'$       | $\leftarrow$       | 158.2.1290   | $P3c11'$           | II   |
| 158.59        | $P3c'1$        | $\leftarrow$       | 158.3.1291   | $P3c'1$            | III  |
| 158.60        | $P_c3c1$       | $\leftarrow$       | 156.5.1283   | $P_{2c}3m'1$       | IV   |
| 159.61        | $P31c$         | $\leftarrow$       | 159.1.1292   | $P31c$             | I    |
| 159.62        | $P31c1'$       | $\leftarrow$       | 159.2.1293   | $P31c1'$           | II   |
| 159.63        | $P31c'$        | $\leftarrow$       | 159.3.1294   | $P31c'$            | III  |
| 159.64        | $P_c31c$       | $\leftarrow$       | 157.5.1288   | $P_{2c}31m'$       | IV   |
| 160.65        | $R3m$          | $\leftarrow$       | 160.1.1295   | $R3m$              | I    |
| 160.66        | $R3m1'$        | $\leftarrow$       | 160.2.1296   | $R3m1'$            | II   |
| 160.67        | $R3m'$         | $\leftarrow$       | 160.3.1297   | $R3m'$             | III  |
| 160.68        | $R_I3m$        | $\leftarrow$       | 160.4.1298   | $R_R3m$            | IV   |
| 161.69        | $R3c$          | $\leftarrow$       | 161.1.1300   | $R3c$              | I    |
| 161.70        | $R3c1'$        | $\leftarrow$       | 161.2.1301   | $R3c1'$            | II   |
| 161.71        | $R3c'$         | $\leftarrow$       | 161.3.1302   | $R3c'$             | III  |
| 161.72        | $R_I3c$        | $\leftarrow$       | 160.5.1299   | $R_R3m'$           | IV   |
| 162.73        | $P\bar{3}1m$   | $\leftarrow$       | 162.1.1303   | $P\bar{3}1m$       | I    |
| 162.74        | $P\bar{3}1m1'$ | $\leftarrow$       | 162.2.1304   | $P\bar{3}1m1'$     | II   |
| 162.75        | $P\bar{3}'1m$  | $\leftarrow$       | 162.3.1305   | $P\bar{3}'1m$      | III  |
| 162.76        | $P\bar{3}'1m'$ | $\leftarrow$       | 162.4.1306   | $P\bar{3}'1m'$     | III  |
| 162.77        | $P\bar{3}1m'$  | $\leftarrow$       | 162.5.1307   | $P\bar{3}1m'$      | III  |
| 162.78        | $P_c\bar{3}1m$ | $\leftarrow$       | 162.6.1308   | $P_{2c}\bar{3}1m$  | IV   |
| 163.79        | $P\bar{3}1c$   | $\leftarrow$       | 163.1.1310   | $P\bar{3}1c$       | I    |
| 163.80        | $P\bar{3}1c1'$ | $\leftarrow$       | 163.2.1311   | $P\bar{3}1c1'$     | II   |
| 163.81        | $P\bar{3}'1c$  | $\leftarrow$       | 163.3.1312   | $P\bar{3}'1c$      | III  |
| 163.82        | $P\bar{3}'1c'$ | $\leftarrow$       | 163.4.1313   | $P\bar{3}'1c'$     | III  |
| 163.83        | $P\bar{3}1c'$  | $\leftarrow$       | 163.5.1314   | $P\bar{3}1c'$      | III  |
| 163.84        | $P_c\bar{3}1c$ | $\leftarrow$       | 162.7.1309   | $P_{2c}\bar{3}1m'$ | IV   |
| 164.85        | $P3m1$         | $\leftarrow$       | 164.1.1315   | $P3m1$             | I    |
| 164.86        | $P3m11'$       | $\leftarrow$       | 164.2.1316   | $P3m11'$           | II   |
| 164.87        | $P\bar{3}'m1$  | $\leftarrow$       | 164.3.1317   | $P\bar{3}'m1$      | III  |
| 164.88        | $P\bar{3}'m'1$ | $\leftarrow$       | 164.4.1318   | $P\bar{3}'m'1$     | III  |
| 164.89        | $P\bar{3}m'1$  | $\leftarrow$       | 164.5.1319   | $P\bar{3}m'1$      | III  |
| 164.90        | $P_c\bar{3}m1$ | $\leftarrow$       | 164.6.1320   | $P_{2c}\bar{3}m1$  | IV   |
| 165.91        | $P\bar{3}c1$   | $\leftarrow$       | 165.1.1322   | $P\bar{3}c1$       | I    |
| 165.92        | $P\bar{3}c11'$ | $\leftarrow$       | 165.2.1323   | $P\bar{3}c11'$     | II   |
| 165.93        | $P\bar{3}'c1$  | $\leftarrow$       | 165.3.1324   | $P\bar{3}'c1$      | III  |
| 165.94        | $P\bar{3}'c'1$ | $\leftarrow$       | 165.4.1325   | $P\bar{3}'c'1$     | III  |
| 165.95        | $P\bar{3}c'1$  | $\leftarrow$       | 165.5.1326   | $P\bar{3}c'1$      | III  |
| 165.96        | $P_c\bar{3}c1$ | $\leftarrow$       | 164.7.1321   | $P_{2c}\bar{3}m'1$ | IV   |
| 166.97        | $R3m$          | $\leftarrow$       | 166.1.1327   | $R3m$              | I    |

| BNS<br>Number | BNS<br>Symbol | BNS (BC)<br>Symbol | OG<br>Number | OG<br>Symbol    | Type |
|---------------|---------------|--------------------|--------------|-----------------|------|
| 166.98        | $R\bar{3}m1'$ | $\leftarrow$       | 166.2.1328   | $R\bar{3}m1'$   | II   |
| 166.99        | $R\bar{3}'m$  | $\leftarrow$       | 166.3.1329   | $R\bar{3}'m$    | III  |
| 166.100       | $R\bar{3}'m'$ | $\leftarrow$       | 166.4.1330   | $R\bar{3}'m'$   | III  |
| 166.101       | $R\bar{3}m'$  | $\leftarrow$       | 166.5.1331   | $R\bar{3}m'$    | III  |
| 166.102       | $R_I\bar{3}m$ | $\leftarrow$       | 166.6.1332   | $R_R\bar{3}m$   | IV   |
| 167.103       | $R\bar{3}c$   | $\leftarrow$       | 167.1.1334   | $R\bar{3}c$     | I    |
| 167.104       | $R\bar{3}c1'$ | $\leftarrow$       | 167.2.1335   | $R\bar{3}c1'$   | II   |
| 167.105       | $R\bar{3}'c$  | $\leftarrow$       | 167.3.1336   | $R\bar{3}'c$    | III  |
| 167.106       | $R\bar{3}'c'$ | $\leftarrow$       | 167.4.1337   | $R\bar{3}'c'$   | III  |
| 167.107       | $R\bar{3}c'$  | $\leftarrow$       | 167.5.1338   | $R\bar{3}c'$    | III  |
| 167.108       | $R_I\bar{3}c$ | $\leftarrow$       | 166.7.1333   | $R_R\bar{3}m'$  | IV   |
| 168.109       | $P6$          | $\leftarrow$       | 168.1.1339   | $P6$            | I    |
| 168.110       | $P61'$        | $\leftarrow$       | 168.2.1340   | $P61'$          | II   |
| 168.111       | $P6'$         | $\leftarrow$       | 168.3.1341   | $P6'$           | III  |
| 168.112       | $P_c6$        | $\leftarrow$       | 168.4.1342   | $P_{2c}6$       | IV   |
| 169.113       | $P6_1$        | $\leftarrow$       | 169.1.1344   | $P6_1$          | I    |
| 169.114       | $P6_11'$      | $\leftarrow$       | 169.2.1345   | $P6_11'$        | II   |
| 169.115       | $P6'_1$       | $\leftarrow$       | 169.3.1346   | $P6'_1$         | III  |
| 169.116       | $P_c6_1$      | $\leftarrow$       | 171.4.1353   | $P_{2c}6_2$     | IV   |
| 170.117       | $P6_5$        | $\leftarrow$       | 170.1.1347   | $P6_5$          | I    |
| 170.118       | $P6_51'$      | $\leftarrow$       | 170.2.1348   | $P6_51'$        | II   |
| 170.119       | $P6'_5$       | $\leftarrow$       | 170.3.1349   | $P6'_5$         | III  |
| 170.120       | $P_c6_5$      | $\leftarrow$       | 172.5.1359   | $P_{2c}6'_4$    | IV   |
| 171.121       | $P6_2$        | $\leftarrow$       | 171.1.1350   | $P6_2$          | I    |
| 171.122       | $P6_21'$      | $\leftarrow$       | 171.2.1351   | $P6_21'$        | II   |
| 171.123       | $P6'_2$       | $\leftarrow$       | 171.3.1352   | $P6'_2$         | III  |
| 171.124       | $P_c6_2$      | $\leftarrow$       | 172.4.1358   | $P_{2c}6_4$     | IV   |
| 172.125       | $P6_4$        | $\leftarrow$       | 172.1.1355   | $P6_4$          | I    |
| 172.126       | $P6_41'$      | $\leftarrow$       | 172.2.1356   | $P6_41'$        | II   |
| 172.127       | $P6'_4$       | $\leftarrow$       | 172.3.1357   | $P6'_4$         | III  |
| 172.128       | $P_c6_4$      | $\leftarrow$       | 171.5.1354   | $P_{2c}6'_2$    | IV   |
| 173.129       | $P6_3$        | $\leftarrow$       | 173.1.1360   | $P6_3$          | I    |
| 173.130       | $P6_31'$      | $\leftarrow$       | 173.2.1361   | $P6_31'$        | II   |
| 173.131       | $P6'_3$       | $\leftarrow$       | 173.3.1362   | $P6'_3$         | III  |
| 173.132       | $P_c6_3$      | $\leftarrow$       | 168.5.1343   | $P_{2c}6'$      | IV   |
| 174.133       | $P\bar{6}$    | $\leftarrow$       | 174.1.1363   | $P\bar{6}$      | I    |
| 174.134       | $P\bar{6}1'$  | $\leftarrow$       | 174.2.1364   | $P\bar{6}1'$    | II   |
| 174.135       | $P\bar{6}'$   | $\leftarrow$       | 174.3.1365   | $P\bar{6}'$     | III  |
| 174.136       | $P_c\bar{6}$  | $\leftarrow$       | 174.4.1366   | $P_{2c}\bar{6}$ | IV   |
| 175.137       | $P6/m$        | $\leftarrow$       | 175.1.1367   | $P6/m$          | I    |
| 175.138       | $P6/m1'$      | $\leftarrow$       | 175.2.1368   | $P6/m1'$        | II   |
| 175.139       | $P6'/m$       | $\leftarrow$       | 175.3.1369   | $P6'/m$         | III  |
| 175.140       | $P6/m'$       | $\leftarrow$       | 175.4.1370   | $P6/m'$         | III  |
| 175.141       | $P6'/m'$      | $\leftarrow$       | 175.5.1371   | $P6'/m'$        | III  |
| 175.142       | $P_c6/m$      | $\leftarrow$       | 175.6.1372   | $P_{2c}6/m$     | IV   |
| 176.143       | $P6_3/m$      | $\leftarrow$       | 176.1.1374   | $P6_3/m$        | I    |
| 176.144       | $P6_3/m1'$    | $\leftarrow$       | 176.2.1375   | $P6_3/m1'$      | II   |
| 176.145       | $P6'_3/m$     | $\leftarrow$       | 176.3.1376   | $P6'_3/m$       | III  |
| 176.146       | $P6_3/m'$     | $\leftarrow$       | 176.4.1377   | $P6_3/m'$       | III  |
| 176.147       | $P6'_3/m'$    | $\leftarrow$       | 176.5.1378   | $P6'_3/m'$      | III  |
| 176.148       | $P_c6_3/m$    | $\leftarrow$       | 175.7.1373   | $P_{2c}6'/m$    | IV   |
| 177.149       | $P622$        | $\leftarrow$       | 177.1.1379   | $P622$          | I    |
| 177.150       | $P6221'$      | $\leftarrow$       | 177.2.1380   | $P6221'$        | II   |
| 177.151       | $P6'2'2$      | $\leftarrow$       | 177.3.1381   | $P6'2'2$        | III  |
| 177.152       | $P6'22'$      | $\leftarrow$       | 177.4.1382   | $P6'22'$        | III  |

| BNS<br>Number | BNS<br>Symbol | BNS (BC)<br>Symbol | OG<br>Number | OG<br>Symbol     | Type |
|---------------|---------------|--------------------|--------------|------------------|------|
| 177.153       | $P6_2'2'$     | $\leftarrow$       | 177.5.1383   | $P6_2'2'$        | III  |
| 177.154       | $P_c6_22$     | $\leftarrow$       | 177.6.1384   | $P_{2c}6_22$     | IV   |
| 178.155       | $P6_122$      | $\leftarrow$       | 178.1.1386   | $P6_122$         | I    |
| 178.156       | $P6_1221'$    | $\leftarrow$       | 178.2.1387   | $P6_1221'$       | II   |
| 178.157       | $P6_1'2'2$    | $\leftarrow$       | 178.3.1388   | $P6_1'2'2$       | III  |
| 178.158       | $P6_1'22'$    | $\leftarrow$       | 178.4.1389   | $P6_1'22'$       | III  |
| 178.159       | $P6_12'2'$    | $\leftarrow$       | 178.5.1390   | $P6_12'2'$       | III  |
| 178.160       | $P_c6_122$    | $\leftarrow$       | 180.6.1401   | $P_{2c}6_222'$   | IV   |
| 179.161       | $P6_522$      | $\leftarrow$       | 179.1.1391   | $P6_522$         | I    |
| 179.162       | $P6_5221'$    | $\leftarrow$       | 179.2.1392   | $P6_5221'$       | II   |
| 179.163       | $P6_5'2'2$    | $\leftarrow$       | 179.3.1393   | $P6_5'2'2$       | III  |
| 179.164       | $P6_5'22'$    | $\leftarrow$       | 179.4.1394   | $P6_5'22'$       | III  |
| 179.165       | $P6_52'2'$    | $\leftarrow$       | 179.5.1395   | $P6_52'2'$       | III  |
| 179.166       | $P_c6_522$    | $\leftarrow$       | 181.7.1409   | $P_{2c}6_4'2'2'$ | IV   |
| 180.167       | $P6_222$      | $\leftarrow$       | 180.1.1396   | $P6_222$         | I    |
| 180.168       | $P6_2221'$    | $\leftarrow$       | 180.2.1397   | $P6_2221'$       | II   |
| 180.169       | $P6_2'2'2$    | $\leftarrow$       | 180.3.1398   | $P6_2'2'2$       | III  |
| 180.170       | $P6_2'22'$    | $\leftarrow$       | 180.4.1399   | $P6_2'22'$       | III  |
| 180.171       | $P6_22'2'$    | $\leftarrow$       | 180.5.1400   | $P6_22'2'$       | III  |
| 180.172       | $P_c6_222$    | $\leftarrow$       | 181.6.1408   | $P_{2c}6_422'$   | IV   |
| 181.173       | $P6_422$      | $\leftarrow$       | 181.1.1403   | $P6_422$         | I    |
| 181.174       | $P6_4221'$    | $\leftarrow$       | 181.2.1404   | $P6_4221'$       | II   |
| 181.175       | $P6_4'2'2$    | $\leftarrow$       | 181.3.1405   | $P6_4'2'2$       | III  |
| 181.176       | $P6_4'22'$    | $\leftarrow$       | 181.4.1406   | $P6_4'22'$       | III  |
| 181.177       | $P6_42'2'$    | $\leftarrow$       | 181.5.1407   | $P6_42'2'$       | III  |
| 181.178       | $P_c6_422$    | $\leftarrow$       | 180.7.1402   | $P_{2c}6_2'22$   | IV   |
| 182.179       | $P6_322$      | $\leftarrow$       | 182.1.1410   | $P6_322$         | I    |
| 182.180       | $P6_3221'$    | $\leftarrow$       | 182.2.1411   | $P6_3221'$       | II   |
| 182.181       | $P6_3'2'2$    | $\leftarrow$       | 182.3.1412   | $P6_3'2'2$       | III  |
| 182.182       | $P6_3'22'$    | $\leftarrow$       | 182.4.1413   | $P6_3'22'$       | III  |
| 182.183       | $P6_32'2'$    | $\leftarrow$       | 182.5.1414   | $P6_32'2'$       | III  |
| 182.184       | $P_c6_322$    | $\leftarrow$       | 177.7.1385   | $P_{2c}6'22'$    | IV   |
| 183.185       | $P6mm$        | $\leftarrow$       | 183.1.1415   | $P6mm$           | I    |
| 183.186       | $P6mm1'$      | $\leftarrow$       | 183.2.1416   | $P6mm1'$         | II   |
| 183.187       | $P6'm'm$      | $\leftarrow$       | 183.3.1417   | $P6'm'm$         | III  |
| 183.188       | $P6'mm'$      | $\leftarrow$       | 183.4.1418   | $P6'mm'$         | III  |
| 183.189       | $P6m'm'$      | $\leftarrow$       | 183.5.1419   | $P6m'm'$         | III  |
| 183.190       | $P_c6mm$      | $\leftarrow$       | 183.6.1420   | $P_{2c}6mm$      | IV   |
| 184.191       | $P6cc$        | $\leftarrow$       | 184.1.1424   | $P6cc$           | I    |
| 184.192       | $P6cc1'$      | $\leftarrow$       | 184.2.1425   | $P6cc1'$         | II   |
| 184.193       | $P6'c'c$      | $\leftarrow$       | 184.3.1426   | $P6'c'c$         | III  |
| 184.194       | $P6'cc'$      | $\leftarrow$       | 184.4.1427   | $P6'cc'$         | III  |
| 184.195       | $P6c'c'$      | $\leftarrow$       | 184.5.1428   | $P6c'c'$         | III  |
| 184.196       | $P_c6cc$      | $\leftarrow$       | 183.9.1423   | $P_{2c}6m'm'$    | IV   |
| 185.197       | $P6_3cm$      | $\leftarrow$       | 185.1.1429   | $P6_3cm$         | I    |
| 185.198       | $P6_3cm1'$    | $\leftarrow$       | 185.2.1430   | $P6_3cm1'$       | II   |
| 185.199       | $P6_3'c'm$    | $\leftarrow$       | 185.3.1431   | $P6_3'c'm$       | III  |
| 185.200       | $P6_3'cm'$    | $\leftarrow$       | 185.4.1432   | $P6_3'cm'$       | III  |
| 185.201       | $P6_3c'm'$    | $\leftarrow$       | 185.5.1433   | $P6_3c'm'$       | III  |
| 185.202       | $P_c6_3cm$    | $\leftarrow$       | 183.7.1421   | $P_{2c}6'm'm$    | IV   |
| 186.203       | $P6_3mc$      | $\leftarrow$       | 186.1.1434   | $P6_3mc$         | I    |
| 186.204       | $P6_3mc1'$    | $\leftarrow$       | 186.2.1435   | $P6_3mc1'$       | II   |
| 186.205       | $P6_3'm'c$    | $\leftarrow$       | 186.3.1436   | $P6_3'm'c$       | III  |
| 186.206       | $P6_3'mc'$    | $\leftarrow$       | 186.4.1437   | $P6_3'mc'$       | III  |
| 186.207       | $P6_3m'c'$    | $\leftarrow$       | 186.5.1438   | $P6_3m'c'$       | III  |

| BNS<br>Number | BNS<br>Symbol   | BNS (BC)<br>Symbol | OG<br>Number | OG<br>Symbol        | Type |
|---------------|-----------------|--------------------|--------------|---------------------|------|
| 186.208       | $P_c6_3mc$      | $\leftarrow$       | 183.8.1422   | $P_{2c}6'mm'$       | IV   |
| 187.209       | $P\bar{6}m2$    | $\leftarrow$       | 187.1.1439   | $P\bar{6}m2$        | I    |
| 187.210       | $P\bar{6}m21'$  | $\leftarrow$       | 187.2.1440   | $P\bar{6}m21'$      | II   |
| 187.211       | $P\bar{6}'m'2$  | $\leftarrow$       | 187.3.1441   | $P\bar{6}'m'2$      | III  |
| 187.212       | $P\bar{6}'m'2'$ | $\leftarrow$       | 187.4.1442   | $P\bar{6}'m'2'$     | III  |
| 187.213       | $P\bar{6}m'2'$  | $\leftarrow$       | 187.5.1443   | $P\bar{6}m'2'$      | III  |
| 187.214       | $P_c\bar{6}m2$  | $\leftarrow$       | 187.6.1444   | $P_{2c}\bar{6}m2$   | IV   |
| 188.215       | $P\bar{6}c2$    | $\leftarrow$       | 188.1.1446   | $P\bar{6}c2$        | I    |
| 188.216       | $P\bar{6}c21'$  | $\leftarrow$       | 188.2.1447   | $P\bar{6}c21'$      | II   |
| 188.217       | $P\bar{6}'c'2$  | $\leftarrow$       | 188.3.1448   | $P\bar{6}'c'2$      | III  |
| 188.218       | $P\bar{6}'c'2'$ | $\leftarrow$       | 188.4.1449   | $P\bar{6}'c'2'$     | III  |
| 188.219       | $P\bar{6}c'2'$  | $\leftarrow$       | 188.5.1450   | $P\bar{6}c'2'$      | III  |
| 188.220       | $P_c\bar{6}c2$  | $\leftarrow$       | 187.7.1445   | $P_{2c}\bar{6}'m'2$ | IV   |
| 189.221       | $P\bar{6}2m$    | $\leftarrow$       | 189.1.1451   | $P\bar{6}2m$        | I    |
| 189.222       | $P\bar{6}2m1'$  | $\leftarrow$       | 189.2.1452   | $P\bar{6}2m1'$      | II   |
| 189.223       | $P\bar{6}'2'm$  | $\leftarrow$       | 189.3.1453   | $P\bar{6}'2'm$      | III  |
| 189.224       | $P\bar{6}'2m'$  | $\leftarrow$       | 189.4.1454   | $P\bar{6}'2m'$      | III  |
| 189.225       | $P\bar{6}2'm'$  | $\leftarrow$       | 189.5.1455   | $P\bar{6}2'm'$      | III  |
| 189.226       | $P_c\bar{6}2m$  | $\leftarrow$       | 189.6.1456   | $P_{2c}\bar{6}2m$   | IV   |
| 190.227       | $P\bar{6}2c$    | $\leftarrow$       | 190.1.1458   | $P\bar{6}2c$        | I    |
| 190.228       | $P\bar{6}2c1'$  | $\leftarrow$       | 190.2.1459   | $P\bar{6}2c1'$      | II   |
| 190.229       | $P\bar{6}'2'c$  | $\leftarrow$       | 190.3.1460   | $P\bar{6}'2'c$      | III  |
| 190.230       | $P\bar{6}'2c'$  | $\leftarrow$       | 190.4.1461   | $P\bar{6}'2c'$      | III  |
| 190.231       | $P\bar{6}2'c'$  | $\leftarrow$       | 190.5.1462   | $P\bar{6}2'c'$      | III  |
| 190.232       | $P_c\bar{6}2c$  | $\leftarrow$       | 189.7.1457   | $P_{2c}\bar{6}'2m'$ | IV   |
| 191.233       | $P6/mmm$        | $\leftarrow$       | 191.1.1463   | $P6/mmm$            | I    |
| 191.234       | $P6/mmm1'$      | $\leftarrow$       | 191.2.1464   | $P6/mmm1'$          | II   |
| 191.235       | $P6/m'mm$       | $\leftarrow$       | 191.3.1465   | $P6/m'mm$           | III  |
| 191.236       | $P6'/mm'm$      | $\leftarrow$       | 191.4.1466   | $P6'/mm'm$          | III  |
| 191.237       | $P6'/mmm'$      | $\leftarrow$       | 191.5.1467   | $P6'/mmm'$          | III  |
| 191.238       | $P6'/m'm'm$     | $\leftarrow$       | 191.6.1468   | $P6'/m'm'm$         | III  |
| 191.239       | $P6'/m'mm'$     | $\leftarrow$       | 191.7.1469   | $P6'/m'mm'$         | III  |
| 191.240       | $P6/mm'm'm'$    | $\leftarrow$       | 191.8.1470   | $P6/mm'm'm'$        | III  |
| 191.241       | $P6/m'm'm'm'$   | $\leftarrow$       | 191.9.1471   | $P6/m'm'm'm'$       | III  |
| 191.242       | $P_c6/mmm$      | $\leftarrow$       | 191.10.1472  | $P_{2c}6/mmm$       | IV   |
| 192.243       | $P6/mcc$        | $\leftarrow$       | 192.1.1476   | $P6/mcc$            | I    |
| 192.244       | $P6/mcc1'$      | $\leftarrow$       | 192.2.1477   | $P6/mcc1'$          | II   |
| 192.245       | $P6/m'cc$       | $\leftarrow$       | 192.3.1478   | $P6/m'cc$           | III  |
| 192.246       | $P6'/mc'c$      | $\leftarrow$       | 192.4.1479   | $P6'/mc'c$          | III  |
| 192.247       | $P6'/mcc'$      | $\leftarrow$       | 192.5.1480   | $P6'/mcc'$          | III  |
| 192.248       | $P6'/m'c'c$     | $\leftarrow$       | 192.6.1481   | $P6'/m'c'c$         | III  |
| 192.249       | $P6'/m'cc'$     | $\leftarrow$       | 192.7.1482   | $P6'/m'cc'$         | III  |
| 192.250       | $P6/mc'c'$      | $\leftarrow$       | 192.8.1483   | $P6/mc'c'$          | III  |
| 192.251       | $P6/m'c'c'$     | $\leftarrow$       | 192.9.1484   | $P6/m'c'c'$         | III  |
| 192.252       | $P_c6/mcc$      | $\leftarrow$       | 191.13.1475  | $P_{2c}6/mm'm'm'$   | IV   |
| 193.253       | $P6_3/mcm$      | $\leftarrow$       | 193.1.1485   | $P6_3/mcm$          | I    |
| 193.254       | $P6_3/mcm1'$    | $\leftarrow$       | 193.2.1486   | $P6_3/mcm1'$        | II   |
| 193.255       | $P6_3/m'cm$     | $\leftarrow$       | 193.3.1487   | $P6_3/m'cm$         | III  |
| 193.256       | $P6'_3/mc'm$    | $\leftarrow$       | 193.4.1488   | $P6'_3/mc'm$        | III  |
| 193.257       | $P6'_3/mcm'$    | $\leftarrow$       | 193.5.1489   | $P6'_3/mcm'$        | III  |
| 193.258       | $P6'_3/m'c'm$   | $\leftarrow$       | 193.6.1490   | $P6'_3/m'c'm$       | III  |
| 193.259       | $P6'_3/m'cm'$   | $\leftarrow$       | 193.7.1491   | $P6'_3/m'cm'$       | III  |
| 193.260       | $P6_3/mc'm'm'$  | $\leftarrow$       | 193.8.1492   | $P6_3/mc'm'm'$      | III  |
| 193.261       | $P6_3/m'c'm'm'$ | $\leftarrow$       | 193.9.1493   | $P6_3/m'c'm'm'$     | III  |
| 193.262       | $P_c6_3/mcm$    | $\leftarrow$       | 191.11.1473  | $P_{2c}6'/mm'm'm$   | IV   |

| BNS<br>Number | BNS<br>Symbol  | BNS (BC)<br>Symbol | OG<br>Number | OG<br>Symbol     | Type |
|---------------|----------------|--------------------|--------------|------------------|------|
| 194.263       | $P6_3/mmc$     | $\leftarrow$       | 194.1.1494   | $P6_3/mmc$       | I    |
| 194.264       | $P6_3/mmc1'$   | $\leftarrow$       | 194.2.1495   | $P6_3/mmc1'$     | II   |
| 194.265       | $P6_3/m'mc$    | $\leftarrow$       | 194.3.1496   | $P6_3/m'mc$      | III  |
| 194.266       | $P6_3'/mm'c$   | $\leftarrow$       | 194.4.1497   | $P6_3'/mm'c$     | III  |
| 194.267       | $P6_3'/mmc'$   | $\leftarrow$       | 194.5.1498   | $P6_3'/mmc'$     | III  |
| 194.268       | $P6_3'/m'm'c$  | $\leftarrow$       | 194.6.1499   | $P6_3'/m'm'c$    | III  |
| 194.269       | $P6_3'/m'mc'$  | $\leftarrow$       | 194.7.1500   | $P6_3'/m'mc'$    | III  |
| 194.270       | $P6_3'/mm'c'$  | $\leftarrow$       | 194.8.1501   | $P6_3'/mm'c'$    | III  |
| 194.271       | $P6_3'/m'm'c'$ | $\leftarrow$       | 194.9.1502   | $P6_3'/m'm'c'$   | III  |
| 194.272       | $P_63/mmc$     | $\leftarrow$       | 191.12.1474  | $P_{2c}6'/mmm'$  | IV   |
| 195.1         | $P23$          | $\leftarrow$       | 195.1.1503   | $P23$            | I    |
| 195.2         | $P231'$        | $\leftarrow$       | 195.2.1504   | $P231'$          | II   |
| 195.3         | $P_I23$        | $\leftarrow$       | 197.3.1510   | $I_P23$          | IV   |
| 196.4         | $F23$          | $\leftarrow$       | 196.1.1506   | $F23$            | I    |
| 196.5         | $F231'$        | $\leftarrow$       | 196.2.1507   | $F231'$          | II   |
| 196.6         | $F_s23$        | $\leftarrow$       | 195.3.1505   | $P_F23$          | IV   |
| 197.7         | $I23$          | $\leftarrow$       | 197.1.1508   | $I23$            | I    |
| 197.8         | $I231'$        | $\leftarrow$       | 197.2.1509   | $I231'$          | II   |
| 198.9         | $P2_13$        | $\leftarrow$       | 198.1.1511   | $P2_13$          | I    |
| 198.10        | $P2_131'$      | $\leftarrow$       | 198.2.1512   | $P2_131'$        | II   |
| 198.11        | $P_I2_13$      | $\leftarrow$       | 199.3.1515   | $I_P2_13$        | IV   |
| 199.12        | $I2_13$        | $\leftarrow$       | 199.1.1513   | $I2_13$          | I    |
| 199.13        | $I2_131'$      | $\leftarrow$       | 199.2.1514   | $I2_131'$        | II   |
| 200.14        | $Pm\bar{3}$    | $\leftarrow$       | 200.1.1516   | $Pm\bar{3}$      | I    |
| 200.15        | $Pm\bar{3}1'$  | $\leftarrow$       | 200.2.1517   | $Pm\bar{3}1'$    | II   |
| 200.16        | $Pm'\bar{3}'$  | $\leftarrow$       | 200.3.1518   | $Pm'\bar{3}'$    | III  |
| 200.17        | $P_I m\bar{3}$ | $\leftarrow$       | 204.4.1533   | $I_P m\bar{3}$   | IV   |
| 201.18        | $Pn\bar{3}$    | $\leftarrow$       | 201.1.1520   | $Pn\bar{3}$      | I    |
| 201.19        | $Pn\bar{3}1'$  | $\leftarrow$       | 201.2.1521   | $Pn\bar{3}1'$    | II   |
| 201.20        | $Pn'\bar{3}'$  | $\leftarrow$       | 201.3.1522   | $Pn'\bar{3}'$    | III  |
| 201.21        | $P_I n\bar{3}$ | $\leftarrow$       | 204.5.1534   | $I_P m'\bar{3}'$ | IV   |
| 202.22        | $Fm\bar{3}$    | $\leftarrow$       | 202.1.1524   | $Fm\bar{3}$      | I    |
| 202.23        | $Fm\bar{3}1'$  | $\leftarrow$       | 202.2.1525   | $Fm\bar{3}1'$    | II   |
| 202.24        | $Fm'\bar{3}'$  | $\leftarrow$       | 202.3.1526   | $Fm'\bar{3}'$    | III  |
| 202.25        | $F_s m\bar{3}$ | $\leftarrow$       | 200.4.1519   | $P_F m\bar{3}$   | IV   |
| 203.26        | $Fd\bar{3}$    | $\leftarrow$       | 203.1.1527   | $Fd\bar{3}$      | I    |
| 203.27        | $Fd\bar{3}1'$  | $\leftarrow$       | 203.2.1528   | $Fd\bar{3}1'$    | II   |
| 203.28        | $Fd'\bar{3}'$  | $\leftarrow$       | 203.3.1529   | $Fd'\bar{3}'$    | III  |
| 203.29        | $F_s d\bar{3}$ | $\leftarrow$       | 201.4.1523   | $P_F n\bar{3}$   | IV   |
| 204.30        | $Im\bar{3}$    | $\leftarrow$       | 204.1.1530   | $Im\bar{3}$      | I    |
| 204.31        | $Im\bar{3}1'$  | $\leftarrow$       | 204.2.1531   | $Im\bar{3}1'$    | II   |
| 204.32        | $Im'\bar{3}'$  | $\leftarrow$       | 204.3.1532   | $Im'\bar{3}'$    | III  |
| 205.33        | $Pa\bar{3}$    | $\leftarrow$       | 205.1.1535   | $Pa\bar{3}$      | I    |
| 205.34        | $Pa\bar{3}1'$  | $\leftarrow$       | 205.2.1536   | $Pa\bar{3}1'$    | II   |
| 205.35        | $Pa'\bar{3}'$  | $\leftarrow$       | 205.3.1537   | $Pa'\bar{3}'$    | III  |
| 205.36        | $P_I a\bar{3}$ | $\leftarrow$       | 206.4.1541   | $I_P a\bar{3}'$  | IV   |
| 206.37        | $Ia\bar{3}$    | $\leftarrow$       | 206.1.1538   | $Ia\bar{3}$      | I    |
| 206.38        | $Ia\bar{3}1'$  | $\leftarrow$       | 206.2.1539   | $Ia\bar{3}1'$    | II   |
| 206.39        | $Ia'\bar{3}'$  | $\leftarrow$       | 206.3.1540   | $Ia'\bar{3}'$    | III  |
| 207.40        | $P432$         | $\leftarrow$       | 207.1.1542   | $P432$           | I    |
| 207.41        | $P4321'$       | $\leftarrow$       | 207.2.1543   | $P4321'$         | II   |
| 207.42        | $P4'32'$       | $\leftarrow$       | 207.3.1544   | $P4'32'$         | III  |
| 207.43        | $P_I 432$      | $\leftarrow$       | 211.4.1559   | $I_P 432$        | IV   |
| 208.44        | $P4_232$       | $\leftarrow$       | 208.1.1546   | $P4_232$         | I    |
| 208.45        | $P4_2321'$     | $\leftarrow$       | 208.2.1547   | $P4_2321'$       | II   |



| BNS<br>Number | BNS<br>Symbol   | BNS (BC)<br>Symbol | OG<br>Number | OG<br>Symbol    | Type |
|---------------|-----------------|--------------------|--------------|-----------------|------|
| 208.46        | $P4_2'32'$      | $\leftarrow$       | 208.3.1548   | $P4_2'32'$      | III  |
| 208.47        | $P_I4_232$      | $\leftarrow$       | 211.5.1560   | $I_P4_2'32'$    | IV   |
| 209.48        | $F432$          | $\leftarrow$       | 209.1.1550   | $F432$          | I    |
| 209.49        | $F4321'$        | $\leftarrow$       | 209.2.1551   | $F4321'$        | II   |
| 209.50        | $F4'32'$        | $\leftarrow$       | 209.3.1552   | $F4'32'$        | III  |
| 209.51        | $F_s432$        | $\leftarrow$       | 207.4.1545   | $P_F432$        | IV   |
| 210.52        | $F4_132$        | $\leftarrow$       | 210.1.1553   | $F4_132$        | I    |
| 210.53        | $F4_1321'$      | $\leftarrow$       | 210.2.1554   | $F4_1321'$      | II   |
| 210.54        | $F4_1'32'$      | $\leftarrow$       | 210.3.1555   | $F4_1'32'$      | III  |
| 210.55        | $F_s4_132$      | $\leftarrow$       | 208.4.1549   | $P_F4_232$      | IV   |
| 211.56        | $I432$          | $\leftarrow$       | 211.1.1556   | $I432$          | I    |
| 211.57        | $I4321'$        | $\leftarrow$       | 211.2.1557   | $I4321'$        | II   |
| 211.58        | $I4'32'$        | $\leftarrow$       | 211.3.1558   | $I4'32'$        | III  |
| 212.59        | $P4_332$        | $\leftarrow$       | 212.1.1561   | $P4_332$        | I    |
| 212.60        | $P4_3321'$      | $\leftarrow$       | 212.2.1562   | $P4_3321'$      | II   |
| 212.61        | $P4_3'32'$      | $\leftarrow$       | 212.3.1563   | $P4_3'32'$      | III  |
| 212.62        | $P_I4_332$      | $\leftarrow$       | 214.4.1570   | $I_P4_132$      | IV   |
| 213.63        | $P4_132$        | $\leftarrow$       | 213.1.1564   | $P4_132$        | I    |
| 213.64        | $P4_1321'$      | $\leftarrow$       | 213.2.1565   | $P4_1321'$      | II   |
| 213.65        | $P4_1'32'$      | $\leftarrow$       | 213.3.1566   | $P4_1'32'$      | III  |
| 213.66        | $P_I4_132$      | $\leftarrow$       | 214.5.1571   | $I_P4_1'32'$    | IV   |
| 214.67        | $I4_132$        | $\leftarrow$       | 214.1.1567   | $I4_132$        | I    |
| 214.68        | $I4_1321'$      | $\leftarrow$       | 214.2.1568   | $I4_1321'$      | II   |
| 214.69        | $I4_1'32'$      | $\leftarrow$       | 214.3.1569   | $I4_1'32'$      | III  |
| 215.70        | $P43m$          | $\leftarrow$       | 215.1.1572   | $P43m$          | I    |
| 215.71        | $P43m1'$        | $\leftarrow$       | 215.2.1573   | $P43m1'$        | II   |
| 215.72        | $P4'3m'$        | $\leftarrow$       | 215.3.1574   | $P4'3m'$        | III  |
| 215.73        | $P_I43m$        | $\leftarrow$       | 217.4.1583   | $I_P43m$        | IV   |
| 216.74        | $F43m$          | $\leftarrow$       | 216.1.1577   | $F43m$          | I    |
| 216.75        | $F43m1'$        | $\leftarrow$       | 216.2.1578   | $F43m1'$        | II   |
| 216.76        | $F4'3m'$        | $\leftarrow$       | 216.3.1579   | $F4'3m'$        | III  |
| 216.77        | $F_s43m$        | $\leftarrow$       | 215.4.1575   | $P_F43m$        | IV   |
| 217.78        | $I43m$          | $\leftarrow$       | 217.1.1580   | $I43m$          | I    |
| 217.79        | $I43m1'$        | $\leftarrow$       | 217.2.1581   | $I43m1'$        | II   |
| 217.80        | $I4'3m'$        | $\leftarrow$       | 217.3.1582   | $I4'3m'$        | III  |
| 218.81        | $P43n$          | $\leftarrow$       | 218.1.1585   | $P43n$          | I    |
| 218.82        | $P43n1'$        | $\leftarrow$       | 218.2.1586   | $P43n1'$        | II   |
| 218.83        | $P4'3n'$        | $\leftarrow$       | 218.3.1587   | $P4'3n'$        | III  |
| 218.84        | $P_I43n$        | $\leftarrow$       | 217.5.1584   | $I_P4'3m'$      | IV   |
| 219.85        | $F43c$          | $\leftarrow$       | 219.1.1588   | $F43c$          | I    |
| 219.86        | $F43c1'$        | $\leftarrow$       | 219.2.1589   | $F43c1'$        | II   |
| 219.87        | $F4'3c'$        | $\leftarrow$       | 219.3.1590   | $F4'3c'$        | III  |
| 219.88        | $F_s43c$        | $\leftarrow$       | 215.5.1576   | $P_F4'3m'$      | IV   |
| 220.89        | $I43d$          | $\leftarrow$       | 220.1.1591   | $I43d$          | I    |
| 220.90        | $I43d1'$        | $\leftarrow$       | 220.2.1592   | $I43d1'$        | II   |
| 220.91        | $I4'3d'$        | $\leftarrow$       | 220.3.1593   | $I4'3d'$        | III  |
| 221.92        | $Pm3m$          | $\leftarrow$       | 221.1.1594   | $Pm3m$          | I    |
| 221.93        | $Pm\bar{3}m1'$  | $\leftarrow$       | 221.2.1595   | $Pm\bar{3}m1'$  | II   |
| 221.94        | $Pm'3'm$        | $\leftarrow$       | 221.3.1596   | $Pm'3'm$        | III  |
| 221.95        | $Pm\bar{3}m'$   | $\leftarrow$       | 221.4.1597   | $Pm\bar{3}m'$   | III  |
| 221.96        | $Pm'3'm'$       | $\leftarrow$       | 221.5.1598   | $Pm'3'm'$       | III  |
| 221.97        | $P_I m\bar{3}m$ | $\leftarrow$       | 229.6.1643   | $I_P m\bar{3}m$ | IV   |
| 222.98        | $Pn3n$          | $\leftarrow$       | 222.1.1601   | $Pn3n$          | I    |
| 222.99        | $Pn\bar{3}n1'$  | $\leftarrow$       | 222.2.1602   | $Pn\bar{3}n1'$  | II   |
| 222.100       | $Pn'3'n$        | $\leftarrow$       | 222.3.1603   | $Pn'3'n$        | III  |

| BNS<br>Number | BNS<br>Symbol          | BNS (BC)<br>Symbol | OG<br>Number | OG<br>Symbol        | Type |
|---------------|------------------------|--------------------|--------------|---------------------|------|
| 222.101       | $Pn\bar{3}n'$          | $\leftarrow$       | 222.4.1604   | $Pn\bar{3}n'$       | III  |
| 222.102       | $Pn'\bar{3}'n'$        | $\leftarrow$       | 222.5.1605   | $Pn'\bar{3}'n'$     | III  |
| 222.103       | $P_{I\bar{n}}\bar{3}n$ | $\leftarrow$       | 229.9.1646   | $I_{Pm'}\bar{3}'m'$ | IV   |
| 223.104       | $Pm\bar{3}n$           | $\leftarrow$       | 223.1.1606   | $Pm\bar{3}n$        | I    |
| 223.105       | $Pm\bar{3}n1'$         | $\leftarrow$       | 223.2.1607   | $Pm\bar{3}n1'$      | II   |
| 223.106       | $Pm'\bar{3}'n$         | $\leftarrow$       | 223.3.1608   | $Pm'\bar{3}'n$      | III  |
| 223.107       | $Pm\bar{3}n'$          | $\leftarrow$       | 223.4.1609   | $Pm\bar{3}n'$       | III  |
| 223.108       | $Pm'\bar{3}'n'$        | $\leftarrow$       | 223.5.1610   | $Pm'\bar{3}'n'$     | III  |
| 223.109       | $P_{Im}\bar{3}n$       | $\leftarrow$       | 229.8.1645   | $I_{Pm}\bar{3}m'$   | IV   |
| 224.110       | $Pn\bar{3}m$           | $\leftarrow$       | 224.1.1611   | $Pn\bar{3}m$        | I    |
| 224.111       | $Pn\bar{3}m1'$         | $\leftarrow$       | 224.2.1612   | $Pn\bar{3}m1'$      | II   |
| 224.112       | $Pn'\bar{3}'m$         | $\leftarrow$       | 224.3.1613   | $Pn'\bar{3}'m$      | III  |
| 224.113       | $Pn\bar{3}m'$          | $\leftarrow$       | 224.4.1614   | $Pn\bar{3}m'$       | III  |
| 224.114       | $Pn'\bar{3}'m'$        | $\leftarrow$       | 224.5.1615   | $Pn'\bar{3}'m'$     | III  |
| 224.115       | $P_{In}\bar{3}m$       | $\leftarrow$       | 229.7.1644   | $I_{Pm'}\bar{3}'m$  | IV   |
| 225.116       | $Fm\bar{3}m$           | $\leftarrow$       | 225.1.1618   | $Fm\bar{3}m$        | I    |
| 225.117       | $Fm\bar{3}m1'$         | $\leftarrow$       | 225.2.1619   | $Fm\bar{3}m1'$      | II   |
| 225.118       | $Fm'\bar{3}'m$         | $\leftarrow$       | 225.3.1620   | $Fm'\bar{3}'m$      | III  |
| 225.119       | $Fm\bar{3}m'$          | $\leftarrow$       | 225.4.1621   | $Fm\bar{3}m'$       | III  |
| 225.120       | $Fm'\bar{3}'m'$        | $\leftarrow$       | 225.5.1622   | $Fm'\bar{3}'m'$     | III  |
| 225.121       | $F_s m\bar{3}m$        | $\leftarrow$       | 221.6.1599   | $P_{Fm}\bar{3}m$    | IV   |
| 226.122       | $Fm\bar{3}c$           | $\leftarrow$       | 226.1.1623   | $Fm\bar{3}c$        | I    |
| 226.123       | $Fm\bar{3}c1'$         | $\leftarrow$       | 226.2.1624   | $Fm\bar{3}c1'$      | II   |
| 226.124       | $Fm'\bar{3}'c$         | $\leftarrow$       | 226.3.1625   | $Fm'\bar{3}'c$      | III  |
| 226.125       | $Fm\bar{3}c'$          | $\leftarrow$       | 226.4.1626   | $Fm\bar{3}c'$       | III  |
| 226.126       | $Fm'\bar{3}'c'$        | $\leftarrow$       | 226.5.1627   | $Fm'\bar{3}'c'$     | III  |
| 226.127       | $F_s m\bar{3}c$        | $\leftarrow$       | 221.7.1600   | $P_{Fm}\bar{3}m'$   | IV   |
| 227.128       | $Fd\bar{3}m$           | $\leftarrow$       | 227.1.1628   | $Fd\bar{3}m$        | I    |
| 227.129       | $Fd\bar{3}m1'$         | $\leftarrow$       | 227.2.1629   | $Fd\bar{3}m1'$      | II   |
| 227.130       | $Fd'\bar{3}'m$         | $\leftarrow$       | 227.3.1630   | $Fd'\bar{3}'m$      | III  |
| 227.131       | $Fd\bar{3}m'$          | $\leftarrow$       | 227.4.1631   | $Fd\bar{3}m'$       | III  |
| 227.132       | $Fd'\bar{3}'m'$        | $\leftarrow$       | 227.5.1632   | $Fd'\bar{3}'m'$     | III  |
| 227.133       | $F_s d\bar{3}m$        | $\leftarrow$       | 224.6.1616   | $P_{Fn}\bar{3}m$    | IV   |
| 228.134       | $Fd\bar{3}c$           | $\leftarrow$       | 228.1.1633   | $Fd\bar{3}c$        | I    |
| 228.135       | $Fd\bar{3}c1'$         | $\leftarrow$       | 228.2.1634   | $Fd\bar{3}c1'$      | II   |
| 228.136       | $Fd'\bar{3}'c$         | $\leftarrow$       | 228.3.1635   | $Fd'\bar{3}'c$      | III  |
| 228.137       | $Fd\bar{3}c'$          | $\leftarrow$       | 228.4.1636   | $Fd\bar{3}c'$       | III  |
| 228.138       | $Fd'\bar{3}'c'$        | $\leftarrow$       | 228.5.1637   | $Fd'\bar{3}'c'$     | III  |
| 228.139       | $F_s d\bar{3}c$        | $\leftarrow$       | 224.7.1617   | $P_{Fn}\bar{3}m'$   | IV   |
| 229.140       | $Im\bar{3}m$           | $\leftarrow$       | 229.1.1638   | $Im\bar{3}m$        | I    |
| 229.141       | $Im\bar{3}m1'$         | $\leftarrow$       | 229.2.1639   | $Im\bar{3}m1'$      | II   |
| 229.142       | $Im'\bar{3}'m$         | $\leftarrow$       | 229.3.1640   | $Im'\bar{3}'m$      | III  |
| 229.143       | $Im\bar{3}m'$          | $\leftarrow$       | 229.4.1641   | $Im\bar{3}m'$       | III  |
| 229.144       | $Im'\bar{3}'m'$        | $\leftarrow$       | 229.5.1642   | $Im'\bar{3}'m'$     | III  |
| 230.145       | $Ia\bar{3}d$           | $\leftarrow$       | 230.1.1647   | $Ia\bar{3}d$        | I    |
| 230.146       | $Ia\bar{3}d1'$         | $\leftarrow$       | 230.2.1648   | $Ia\bar{3}d1'$      | II   |
| 230.147       | $Ia'\bar{3}'d$         | $\leftarrow$       | 230.3.1649   | $Ia'\bar{3}'d$      | III  |
| 230.148       | $Ia\bar{3}d'$          | $\leftarrow$       | 230.4.1650   | $Ia\bar{3}d'$       | III  |
| 230.149       | $Ia'\bar{3}'d'$        | $\leftarrow$       | 230.5.1651   | $Ia'\bar{3}'d'$     | III  |

## 4 MSG elements

The group elements of all 1651 MSGs are listed in Table S2. The MSG symbols in the parentheses are those in BC orientation which are different from the standard BNS symbols. Notice two points:

- The elements of each MSG are the same with the result of `getMSGElem` in the same order.
- The elements of each MSG actually conform to the BC orientation.

Index for quick reference

|        |        |        |        |        |        |        |        |        |        |        |        |
|--------|--------|--------|--------|--------|--------|--------|--------|--------|--------|--------|--------|
| 1.1    | 1.2    | 1.3    | 2.4    | 2.5    | 2.6    | 2.7    | 3.1    | 3.2    | 3.3    | 3.4    | 3.5    |
| 3.6    | 4.7    | 4.8    | 4.9    | 4.10   | 4.11   | 4.12   | 5.13   | 5.14   | 5.15   | 5.16   | 5.17   |
| 6.18   | 6.19   | 6.20   | 6.21   | 6.22   | 6.23   | 7.24   | 7.25   | 7.26   | 7.27   | 7.28   | 7.29   |
| 7.30   | 7.31   | 8.32   | 8.33   | 8.34   | 8.35   | 8.36   | 9.37   | 9.38   | 9.39   | 9.40   | 9.41   |
| 10.42  | 10.43  | 10.44  | 10.45  | 10.46  | 10.47  | 10.48  | 10.49  | 11.50  | 11.51  | 11.52  | 11.53  |
| 11.54  | 11.55  | 11.56  | 11.57  | 12.58  | 12.59  | 12.60  | 12.61  | 12.62  | 12.63  | 12.64  | 13.65  |
| 13.66  | 13.67  | 13.68  | 13.69  | 13.70  | 13.71  | 13.72  | 13.73  | 13.74  | 14.75  | 14.76  | 14.77  |
| 14.78  | 14.79  | 14.80  | 14.81  | 14.82  | 14.83  | 14.84  | 15.85  | 15.86  | 15.87  | 15.88  | 15.89  |
| 15.90  | 15.91  | 16.1   | 16.2   | 16.3   | 16.4   | 16.5   | 16.6   | 17.7   | 17.8   | 17.9   | 17.10  |
| 17.11  | 17.12  | 17.13  | 17.14  | 17.15  | 18.16  | 18.17  | 18.18  | 18.19  | 18.20  | 18.21  | 18.22  |
| 18.23  | 18.24  | 19.25  | 19.26  | 19.27  | 19.28  | 19.29  | 19.30  | 20.31  | 20.32  | 20.33  | 20.34  |
| 20.35  | 20.36  | 20.37  | 21.38  | 21.39  | 21.40  | 21.41  | 21.42  | 21.43  | 21.44  | 22.45  | 22.46  |
| 22.47  | 22.48  | 23.49  | 23.50  | 23.51  | 23.52  | 24.53  | 24.54  | 24.55  | 24.56  | 25.57  | 25.58  |
| 25.59  | 25.60  | 25.61  | 25.62  | 25.63  | 25.64  | 25.65  | 26.66  | 26.67  | 26.68  | 26.69  | 26.70  |
| 26.71  | 26.72  | 26.73  | 26.74  | 26.75  | 26.76  | 26.77  | 27.78  | 27.79  | 27.80  | 27.81  | 27.82  |
| 27.83  | 27.84  | 27.85  | 27.86  | 28.87  | 28.88  | 28.89  | 28.90  | 28.91  | 28.92  | 28.93  | 28.94  |
| 28.95  | 28.96  | 28.97  | 28.98  | 29.99  | 29.100 | 29.101 | 29.102 | 29.103 | 29.104 | 29.105 | 29.106 |
| 29.107 | 29.108 | 29.109 | 29.110 | 30.111 | 30.112 | 30.113 | 30.114 | 30.115 | 30.116 | 30.117 | 30.118 |
| 30.119 | 30.120 | 30.121 | 30.122 | 31.123 | 31.124 | 31.125 | 31.126 | 31.127 | 31.128 | 31.129 | 31.130 |
| 31.131 | 31.132 | 31.133 | 31.134 | 32.135 | 32.136 | 32.137 | 32.138 | 32.139 | 32.140 | 32.141 | 32.142 |
| 32.143 | 33.144 | 33.145 | 33.146 | 33.147 | 33.148 | 33.149 | 33.150 | 33.151 | 33.152 | 33.153 | 33.154 |
| 33.155 | 34.156 | 34.157 | 34.158 | 34.159 | 34.160 | 34.161 | 34.162 | 34.163 | 34.164 | 35.165 | 35.166 |
| 35.167 | 35.168 | 35.169 | 35.170 | 35.171 | 36.172 | 36.173 | 36.174 | 36.175 | 36.176 | 36.177 | 36.178 |
| 36.179 | 37.180 | 37.181 | 37.182 | 37.183 | 37.184 | 37.185 | 37.186 | 38.187 | 38.188 | 38.189 | 38.190 |
| 38.191 | 38.192 | 38.193 | 38.194 | 39.195 | 39.196 | 39.197 | 39.198 | 39.199 | 39.200 | 39.201 | 39.202 |
| 40.203 | 40.204 | 40.205 | 40.206 | 40.207 | 40.208 | 40.209 | 40.210 | 41.211 | 41.212 | 41.213 | 41.214 |
| 41.215 | 41.216 | 41.217 | 41.218 | 42.219 | 42.220 | 42.221 | 42.222 | 42.223 | 43.224 | 43.225 | 43.226 |
| 43.227 | 43.228 | 44.229 | 44.230 | 44.231 | 44.232 | 44.233 | 44.234 | 45.235 | 45.236 | 45.237 | 45.238 |
| 45.239 | 45.240 | 46.241 | 46.242 | 46.243 | 46.244 | 46.245 | 46.246 | 46.247 | 46.248 | 47.249 | 47.250 |
| 47.251 | 47.252 | 47.253 | 47.254 | 47.255 | 47.256 | 48.257 | 48.258 | 48.259 | 48.260 | 48.261 | 48.262 |
| 48.263 | 48.264 | 49.265 | 49.266 | 49.267 | 49.268 | 49.269 | 49.270 | 49.271 | 49.272 | 49.273 | 49.274 |
| 49.275 | 49.276 | 50.277 | 50.278 | 50.279 | 50.280 | 50.281 | 50.282 | 50.283 | 50.284 | 50.285 | 50.286 |
| 50.287 | 50.288 | 51.289 | 51.290 | 51.291 | 51.292 | 51.293 | 51.294 | 51.295 | 51.296 | 51.297 | 51.298 |
| 51.299 | 51.300 | 51.301 | 51.302 | 51.303 | 51.304 | 52.305 | 52.306 | 52.307 | 52.308 | 52.309 | 52.310 |
| 52.311 | 52.312 | 52.313 | 52.314 | 52.315 | 52.316 | 52.317 | 52.318 | 52.319 | 52.320 | 53.321 | 53.322 |
| 53.323 | 53.324 | 53.325 | 53.326 | 53.327 | 53.328 | 53.329 | 53.330 | 53.331 | 53.332 | 53.333 | 53.334 |
| 53.335 | 53.336 | 54.337 | 54.338 | 54.339 | 54.340 | 54.341 | 54.342 | 54.343 | 54.344 | 54.345 | 54.346 |
| 54.347 | 54.348 | 54.349 | 54.350 | 54.351 | 54.352 | 55.353 | 55.354 | 55.355 | 55.356 | 55.357 | 55.358 |
| 55.359 | 55.360 | 55.361 | 55.362 | 55.363 | 55.364 | 56.365 | 56.366 | 56.367 | 56.368 | 56.369 | 56.370 |
| 56.371 | 56.372 | 56.373 | 56.374 | 56.375 | 56.376 | 57.377 | 57.378 | 57.379 | 57.380 | 57.381 | 57.382 |
| 57.383 | 57.384 | 57.385 | 57.386 | 57.387 | 57.388 | 57.389 | 57.390 | 57.391 | 57.392 | 58.393 | 58.394 |
| 58.395 | 58.396 | 58.397 | 58.398 | 58.399 | 58.400 | 58.401 | 58.402 | 58.403 | 58.404 | 59.405 | 59.406 |
| 59.407 | 59.408 | 59.409 | 59.410 | 59.411 | 59.412 | 59.413 | 59.414 | 59.415 | 59.416 | 60.417 | 60.418 |
| 60.419 | 60.420 | 60.421 | 60.422 | 60.423 | 60.424 | 60.425 | 60.426 | 60.427 | 60.428 | 60.429 | 60.430 |
| 60.431 | 60.432 | 61.433 | 61.434 | 61.435 | 61.436 | 61.437 | 61.438 | 61.439 | 61.440 | 62.441 | 62.442 |

|         |         |         |         |         |         |         |         |         |         |         |         |
|---------|---------|---------|---------|---------|---------|---------|---------|---------|---------|---------|---------|
| 62.443  | 62.444  | 62.445  | 62.446  | 62.447  | 62.448  | 62.449  | 62.450  | 62.451  | 62.452  | 62.453  | 62.454  |
| 62.455  | 62.456  | 63.457  | 63.458  | 63.459  | 63.460  | 63.461  | 63.462  | 63.463  | 63.464  | 63.465  | 63.466  |
| 63.467  | 63.468  | 64.469  | 64.470  | 64.471  | 64.472  | 64.473  | 64.474  | 64.475  | 64.476  | 64.477  | 64.478  |
| 64.479  | 64.480  | 65.481  | 65.482  | 65.483  | 65.484  | 65.485  | 65.486  | 65.487  | 65.488  | 65.489  | 65.490  |
| 66.491  | 66.492  | 66.493  | 66.494  | 66.495  | 66.496  | 66.497  | 66.498  | 66.499  | 66.500  | 67.501  | 67.502  |
| 67.503  | 67.504  | 67.505  | 67.506  | 67.507  | 67.508  | 67.509  | 67.510  | 68.511  | 68.512  | 68.513  | 68.514  |
| 68.515  | 68.516  | 68.517  | 68.518  | 68.519  | 68.520  | 69.521  | 69.522  | 69.523  | 69.524  | 69.525  | 69.526  |
| 70.527  | 70.528  | 70.529  | 70.530  | 70.531  | 70.532  | 71.533  | 71.534  | 71.535  | 71.536  | 71.537  | 71.538  |
| 72.539  | 72.540  | 72.541  | 72.542  | 72.543  | 72.544  | 72.545  | 72.546  | 72.547  | 73.548  | 73.549  | 73.550  |
| 73.551  | 73.552  | 73.553  | 74.554  | 74.555  | 74.556  | 74.557  | 74.558  | 74.559  | 74.560  | 74.561  | 74.562  |
| 75.1    | 75.2    | 75.3    | 75.4    | 75.5    | 75.6    | 76.7    | 76.8    | 76.9    | 76.10   | 76.11   | 76.12   |
| 77.13   | 77.14   | 77.15   | 77.16   | 77.17   | 77.18   | 78.19   | 78.20   | 78.21   | 78.22   | 78.23   | 78.24   |
| 79.25   | 79.26   | 79.27   | 79.28   | 80.29   | 80.30   | 80.31   | 80.32   | 81.33   | 81.34   | 81.35   | 81.36   |
| 81.37   | 81.38   | 82.39   | 82.40   | 82.41   | 82.42   | 83.43   | 83.44   | 83.45   | 83.46   | 83.47   | 83.48   |
| 83.49   | 83.50   | 84.51   | 84.52   | 84.53   | 84.54   | 84.55   | 84.56   | 84.57   | 84.58   | 85.59   | 85.60   |
| 85.61   | 85.62   | 85.63   | 85.64   | 85.65   | 85.66   | 86.67   | 86.68   | 86.69   | 86.70   | 86.71   | 86.72   |
| 86.73   | 86.74   | 87.75   | 87.76   | 87.77   | 87.78   | 87.79   | 87.80   | 88.81   | 88.82   | 88.83   | 88.84   |
| 88.85   | 88.86   | 89.87   | 89.88   | 89.89   | 89.90   | 89.91   | 89.92   | 89.93   | 89.94   | 90.95   | 90.96   |
| 90.97   | 90.98   | 90.99   | 90.100  | 90.101  | 90.102  | 91.103  | 91.104  | 91.105  | 91.106  | 91.107  | 91.108  |
| 91.109  | 91.110  | 92.111  | 92.112  | 92.113  | 92.114  | 92.115  | 92.116  | 92.117  | 92.118  | 93.119  | 93.120  |
| 93.121  | 93.122  | 93.123  | 93.124  | 93.125  | 93.126  | 94.127  | 94.128  | 94.129  | 94.130  | 94.131  | 94.132  |
| 94.133  | 94.134  | 95.135  | 95.136  | 95.137  | 95.138  | 95.139  | 95.140  | 95.141  | 95.142  | 96.143  | 96.144  |
| 96.145  | 96.146  | 96.147  | 96.148  | 96.149  | 96.150  | 97.151  | 97.152  | 97.153  | 97.154  | 97.155  | 97.156  |
| 98.157  | 98.158  | 98.159  | 98.160  | 98.161  | 98.162  | 99.163  | 99.164  | 99.165  | 99.166  | 99.167  | 99.168  |
| 99.169  | 99.170  | 100.171 | 100.172 | 100.173 | 100.174 | 100.175 | 100.176 | 100.177 | 100.178 | 101.179 | 101.180 |
| 101.181 | 101.182 | 101.183 | 101.184 | 101.185 | 101.186 | 102.187 | 102.188 | 102.189 | 102.190 | 102.191 | 102.192 |
| 102.193 | 102.194 | 103.195 | 103.196 | 103.197 | 103.198 | 103.199 | 103.200 | 103.201 | 103.202 | 104.203 | 104.204 |
| 104.205 | 104.206 | 104.207 | 104.208 | 104.209 | 104.210 | 105.211 | 105.212 | 105.213 | 105.214 | 105.215 | 105.216 |
| 105.217 | 105.218 | 106.219 | 106.220 | 106.221 | 106.222 | 106.223 | 106.224 | 106.225 | 106.226 | 107.227 | 107.228 |
| 107.229 | 107.230 | 107.231 | 107.232 | 108.233 | 108.234 | 108.235 | 108.236 | 108.237 | 108.238 | 109.239 | 109.240 |
| 109.241 | 109.242 | 109.243 | 109.244 | 110.245 | 110.246 | 110.247 | 110.248 | 110.249 | 110.250 | 111.251 | 111.252 |
| 111.253 | 111.254 | 111.255 | 111.256 | 111.257 | 111.258 | 112.259 | 112.260 | 112.261 | 112.262 | 112.263 | 112.264 |
| 112.265 | 112.266 | 113.267 | 113.268 | 113.269 | 113.270 | 113.271 | 113.272 | 113.273 | 113.274 | 114.275 | 114.276 |
| 114.277 | 114.278 | 114.279 | 114.280 | 114.281 | 114.282 | 115.283 | 115.284 | 115.285 | 115.286 | 115.287 | 115.288 |
| 115.289 | 115.290 | 116.291 | 116.292 | 116.293 | 116.294 | 116.295 | 116.296 | 116.297 | 116.298 | 117.299 | 117.300 |
| 117.301 | 117.302 | 117.303 | 117.304 | 117.305 | 117.306 | 118.307 | 118.308 | 118.309 | 118.310 | 118.311 | 118.312 |
| 118.313 | 118.314 | 119.315 | 119.316 | 119.317 | 119.318 | 119.319 | 119.320 | 120.321 | 120.322 | 120.323 | 120.324 |
| 120.325 | 120.326 | 121.327 | 121.328 | 121.329 | 121.330 | 121.331 | 121.332 | 122.333 | 122.334 | 122.335 | 122.336 |
| 122.337 | 122.338 | 123.339 | 123.340 | 123.341 | 123.342 | 123.343 | 123.344 | 123.345 | 123.346 | 123.347 | 123.348 |
| 123.349 | 123.350 | 124.351 | 124.352 | 124.353 | 124.354 | 124.355 | 124.356 | 124.357 | 124.358 | 124.359 | 124.360 |
| 124.361 | 124.362 | 125.363 | 125.364 | 125.365 | 125.366 | 125.367 | 125.368 | 125.369 | 125.370 | 125.371 | 125.372 |
| 125.373 | 125.374 | 126.375 | 126.376 | 126.377 | 126.378 | 126.379 | 126.380 | 126.381 | 126.382 | 126.383 | 126.384 |
| 126.385 | 126.386 | 127.387 | 127.388 | 127.389 | 127.390 | 127.391 | 127.392 | 127.393 | 127.394 | 127.395 | 127.396 |
| 127.397 | 127.398 | 128.399 | 128.400 | 128.401 | 128.402 | 128.403 | 128.404 | 128.405 | 128.406 | 128.407 | 128.408 |
| 128.409 | 128.410 | 129.411 | 129.412 | 129.413 | 129.414 | 129.415 | 129.416 | 129.417 | 129.418 | 129.419 | 129.420 |
| 129.421 | 129.422 | 130.423 | 130.424 | 130.425 | 130.426 | 130.427 | 130.428 | 130.429 | 130.430 | 130.431 | 130.432 |
| 130.433 | 130.434 | 131.435 | 131.436 | 131.437 | 131.438 | 131.439 | 131.440 | 131.441 | 131.442 | 131.443 | 131.444 |
| 131.445 | 131.446 | 132.447 | 132.448 | 132.449 | 132.450 | 132.451 | 132.452 | 132.453 | 132.454 | 132.455 | 132.456 |
| 132.457 | 132.458 | 133.459 | 133.460 | 133.461 | 133.462 | 133.463 | 133.464 | 133.465 | 133.466 | 133.467 | 133.468 |
| 133.469 | 133.470 | 134.471 | 134.472 | 134.473 | 134.474 | 134.475 | 134.476 | 134.477 | 134.478 | 134.479 | 134.480 |
| 134.481 | 134.482 | 135.483 | 135.484 | 135.485 | 135.486 | 135.487 | 135.488 | 135.489 | 135.490 | 135.491 | 135.492 |
| 135.493 | 135.494 | 136.495 | 136.496 | 136.497 | 136.498 | 136.499 | 136.500 | 136.501 | 136.502 | 136.503 | 136.504 |
| 136.505 | 136.506 | 137.507 | 137.508 | 137.509 | 137.510 | 137.511 | 137.512 | 137.513 | 137.514 | 137.515 | 137.516 |
| 137.517 | 137.518 | 138.519 | 138.520 | 138.521 | 138.522 | 138.523 | 138.524 | 138.525 | 138.526 | 138.527 | 138.528 |
| 138.529 | 138.530 | 139.531 | 139.532 | 139.533 | 139.534 | 139.535 | 139.536 | 139.537 | 139.538 | 139.539 | 139.540 |
| 140.541 | 140.542 | 140.543 | 140.544 | 140.545 | 140.546 | 140.547 | 140.548 | 140.549 | 140.550 | 141.551 | 141.552 |
| 141.553 | 141.554 | 141.555 | 141.556 | 141.557 | 141.558 | 141.559 | 141.560 | 142.561 | 142.562 | 142.563 | 142.564 |
| 142.565 | 142.566 | 142.567 | 142.568 | 142.569 | 142.570 | 143.1   | 143.2   | 143.3   | 144.4   | 144.5   | 144.6   |

---

|         |         |         |         |         |         |         |         |         |         |         |         |
|---------|---------|---------|---------|---------|---------|---------|---------|---------|---------|---------|---------|
| 145.7   | 145.8   | 145.9   | 146.10  | 146.11  | 146.12  | 147.13  | 147.14  | 147.15  | 147.16  | 148.17  | 148.18  |
| 148.19  | 148.20  | 149.21  | 149.22  | 149.23  | 149.24  | 150.25  | 150.26  | 150.27  | 150.28  | 151.29  | 151.30  |
| 151.31  | 151.32  | 152.33  | 152.34  | 152.35  | 152.36  | 153.37  | 153.38  | 153.39  | 153.40  | 154.41  | 154.42  |
| 154.43  | 154.44  | 155.45  | 155.46  | 155.47  | 155.48  | 156.49  | 156.50  | 156.51  | 156.52  | 157.53  | 157.54  |
| 157.55  | 157.56  | 158.57  | 158.58  | 158.59  | 158.60  | 159.61  | 159.62  | 159.63  | 159.64  | 160.65  | 160.66  |
| 160.67  | 160.68  | 161.69  | 161.70  | 161.71  | 161.72  | 162.73  | 162.74  | 162.75  | 162.76  | 162.77  | 162.78  |
| 163.79  | 163.80  | 163.81  | 163.82  | 163.83  | 163.84  | 164.85  | 164.86  | 164.87  | 164.88  | 164.89  | 164.90  |
| 165.91  | 165.92  | 165.93  | 165.94  | 165.95  | 165.96  | 166.97  | 166.98  | 166.99  | 166.100 | 166.101 | 166.102 |
| 167.103 | 167.104 | 167.105 | 167.106 | 167.107 | 167.108 | 168.109 | 168.110 | 168.111 | 168.112 | 169.113 | 169.114 |
| 169.115 | 169.116 | 170.117 | 170.118 | 170.119 | 170.120 | 171.121 | 171.122 | 171.123 | 171.124 | 172.125 | 172.126 |
| 172.127 | 172.128 | 173.129 | 173.130 | 173.131 | 173.132 | 174.133 | 174.134 | 174.135 | 174.136 | 175.137 | 175.138 |
| 175.139 | 175.140 | 175.141 | 175.142 | 176.143 | 176.144 | 176.145 | 176.146 | 176.147 | 176.148 | 177.149 | 177.150 |
| 177.151 | 177.152 | 177.153 | 177.154 | 178.155 | 178.156 | 178.157 | 178.158 | 178.159 | 178.160 | 179.161 | 179.162 |
| 179.163 | 179.164 | 179.165 | 179.166 | 180.167 | 180.168 | 180.169 | 180.170 | 180.171 | 180.172 | 181.173 | 181.174 |
| 181.175 | 181.176 | 181.177 | 181.178 | 182.179 | 182.180 | 182.181 | 182.182 | 182.183 | 182.184 | 183.185 | 183.186 |
| 183.187 | 183.188 | 183.189 | 183.190 | 184.191 | 184.192 | 184.193 | 184.194 | 184.195 | 184.196 | 185.197 | 185.198 |
| 185.199 | 185.200 | 185.201 | 185.202 | 186.203 | 186.204 | 186.205 | 186.206 | 186.207 | 186.208 | 187.209 | 187.210 |
| 187.211 | 187.212 | 187.213 | 187.214 | 188.215 | 188.216 | 188.217 | 188.218 | 188.219 | 188.220 | 189.221 | 189.222 |
| 189.223 | 189.224 | 189.225 | 189.226 | 190.227 | 190.228 | 190.229 | 190.230 | 190.231 | 190.232 | 191.233 | 191.234 |
| 191.235 | 191.236 | 191.237 | 191.238 | 191.239 | 191.240 | 191.241 | 191.242 | 192.243 | 192.244 | 192.245 | 192.246 |
| 192.247 | 192.248 | 192.249 | 192.250 | 192.251 | 192.252 | 193.253 | 193.254 | 193.255 | 193.256 | 193.257 | 193.258 |
| 193.259 | 193.260 | 193.261 | 193.262 | 194.263 | 194.264 | 194.265 | 194.266 | 194.267 | 194.268 | 194.269 | 194.270 |
| 194.271 | 194.272 | 195.1   | 195.2   | 195.3   | 196.4   | 196.5   | 196.6   | 197.7   | 197.8   | 198.9   | 198.10  |
| 198.11  | 199.12  | 199.13  | 200.14  | 200.15  | 200.16  | 200.17  | 201.18  | 201.19  | 201.20  | 201.21  | 202.22  |
| 202.23  | 202.24  | 202.25  | 203.26  | 203.27  | 203.28  | 203.29  | 204.30  | 204.31  | 204.32  | 205.33  | 205.34  |
| 205.35  | 205.36  | 206.37  | 206.38  | 206.39  | 207.40  | 207.41  | 207.42  | 207.43  | 208.44  | 208.45  | 208.46  |
| 208.47  | 209.48  | 209.49  | 209.50  | 209.51  | 210.52  | 210.53  | 210.54  | 210.55  | 211.56  | 211.57  | 211.58  |
| 212.59  | 212.60  | 212.61  | 212.62  | 213.63  | 213.64  | 213.65  | 213.66  | 214.67  | 214.68  | 214.69  | 215.70  |
| 215.71  | 215.72  | 215.73  | 216.74  | 216.75  | 216.76  | 216.77  | 217.78  | 217.79  | 217.80  | 218.81  | 218.82  |
| 218.83  | 218.84  | 219.85  | 219.86  | 219.87  | 219.88  | 220.89  | 220.90  | 220.91  | 221.92  | 221.93  | 221.94  |
| 221.95  | 221.96  | 221.97  | 222.98  | 222.99  | 222.100 | 222.101 | 222.102 | 222.103 | 223.104 | 223.105 | 223.106 |
| 223.107 | 223.108 | 223.109 | 224.110 | 224.111 | 224.112 | 224.113 | 224.114 | 224.115 | 225.116 | 225.117 | 225.118 |
| 225.119 | 225.120 | 225.121 | 226.122 | 226.123 | 226.124 | 226.125 | 226.126 | 226.127 | 227.128 | 227.129 | 227.130 |
| 227.131 | 227.132 | 227.133 | 228.134 | 228.135 | 228.136 | 228.137 | 228.138 | 228.139 | 229.140 | 229.141 | 229.142 |
| 229.143 | 229.144 | 230.145 | 230.146 | 230.147 | 230.148 | 230.149 |         |         |         |         |         |

Table S2: List of MSG elements.

| No.  | Symbol            | Elements                                                                                             |
|------|-------------------|------------------------------------------------------------------------------------------------------|
| 1.1  | $P1$              | $\{E 000\}$                                                                                          |
| 1.2  | $P11'$            | $\{E 000\}, \{E 000\}'$                                                                              |
| 1.3  | $P_s1$            | $\{E 000\}, \{E \frac{1}{2}00\}'$                                                                    |
| 2.4  | $P\bar{1}$        | $\{E 000\}, \{I 000\}$                                                                               |
| 2.5  | $P\bar{1}1'$      | $\{E 000\}, \{I 000\}, \{E 000\}', \{I 000\}'$                                                       |
| 2.6  | $P\bar{1}'$       | $\{E 000\}, \{I 000\}'$                                                                              |
| 2.7  | $P_s\bar{1}$      | $\{E 000\}, \{I 000\}, \{E \frac{1}{2}00\}', \{I \frac{1}{2}00\}'$                                   |
| 3.1  | $P2$              | $\{E 000\}, \{C_{2z} 000\}$                                                                          |
| 3.2  | $P21'$            | $\{E 000\}, \{C_{2z} 000\}, \{E 000\}', \{C_{2z} 000\}'$                                             |
| 3.3  | $P2'$             | $\{E 000\}, \{C_{2z} 000\}'$                                                                         |
| 3.4  | $P_a2$            | $\{E 000\}, \{C_{2z} 000\}, \{E 0\frac{1}{2}0\}', \{C_{2z} 0\frac{1}{2}0\}'$                         |
| 3.5  | $P_b2 (P_c2)$     | $\{E 000\}, \{C_{2z} 000\}, \{E 00\frac{1}{2}\}', \{C_{2z} 00\frac{1}{2}\}'$                         |
| 3.6  | $P_C2 (P_B2)$     | $\{E 000\}, \{C_{2z} 000\}, \{E 0\frac{1}{2}\frac{1}{2}\}', \{C_{2z} 0\frac{1}{2}\frac{1}{2}\}'$     |
| 4.7  | $P2_1$            | $\{E 000\}, \{C_{2z} 00\frac{1}{2}\}$                                                                |
| 4.8  | $P2_11'$          | $\{E 000\}, \{C_{2z} 00\frac{1}{2}\}, \{E 000\}', \{C_{2z} 00\frac{1}{2}\}'$                         |
| 4.9  | $P2_1'$           | $\{E 000\}, \{C_{2z} 00\frac{1}{2}\}'$                                                               |
| 4.10 | $P_a2_1$          | $\{E 000\}, \{C_{2z} 00\frac{1}{2}\}, \{E 0\frac{1}{2}0\}', \{C_{2z} 0\frac{1}{2}\frac{1}{2}\}'$     |
| 4.11 | $P_b2_1 (P_c2_1)$ | $\{E 000\}, \{C_{2z} 00\frac{1}{2}\}, \{E 00\frac{1}{2}\}', \{C_{2z} 000\}'$                         |
| 4.12 | $P_C2_1 (P_B2_1)$ | $\{E 000\}, \{C_{2z} 00\frac{1}{2}\}, \{E 0\frac{1}{2}\frac{1}{2}\}', \{C_{2z} 0\frac{1}{2}0\}'$     |
| 5.13 | $C2 (B2)$         | $\{E 000\}, \{C_{2z} 000\}$                                                                          |
| 5.14 | $C21' (B21')$     | $\{E 000\}, \{C_{2z} 000\}, \{E 000\}', \{C_{2z} 000\}'$                                             |
| 5.15 | $C2' (B2')$       | $\{E 000\}, \{C_{2z} 000\}'$                                                                         |
| 5.16 | $C_c2 (B_b2)$     | $\{E 000\}, \{C_{2z} 000\}, \{E \frac{1}{2}00\}', \{C_{2z} \frac{1}{2}00\}'$                         |
| 5.17 | $C_a2 (B_a2)$     | $\{E 000\}, \{C_{2z} 000\}, \{E 0\frac{1}{2}\frac{1}{2}\}', \{C_{2z} 0\frac{1}{2}\frac{1}{2}\}'$     |
| 6.18 | $Pm$              | $\{E 000\}, \{\sigma_z 000\}$                                                                        |
| 6.19 | $Pm1'$            | $\{E 000\}, \{\sigma_z 000\}, \{E 000\}', \{\sigma_z 000\}'$                                         |
| 6.20 | $Pm'$             | $\{E 000\}, \{\sigma_z 000\}'$                                                                       |
| 6.21 | $P_am$            | $\{E 000\}, \{\sigma_z 000\}, \{E 0\frac{1}{2}0\}', \{\sigma_z 0\frac{1}{2}0\}'$                     |
| 6.22 | $P_bm (P_cm)$     | $\{E 000\}, \{\sigma_z 000\}, \{E 00\frac{1}{2}\}', \{\sigma_z 00\frac{1}{2}\}'$                     |
| 6.23 | $P_Cm (P_Bm)$     | $\{E 000\}, \{\sigma_z 000\}, \{E 0\frac{1}{2}\frac{1}{2}\}', \{\sigma_z 0\frac{1}{2}\frac{1}{2}\}'$ |
| 7.24 | $Pc (Pb)$         | $\{E 000\}, \{\sigma_z \frac{1}{2}00\}$                                                              |
| 7.25 | $Pc1' (Pb1')$     | $\{E 000\}, \{\sigma_z \frac{1}{2}00\}, \{E 000\}', \{\sigma_z \frac{1}{2}00\}'$                     |
| 7.26 | $Pc' (Pb')$       | $\{E 000\}, \{\sigma_z \frac{1}{2}00\}'$                                                             |
| 7.27 | $P_ac (P_ab)$     | $\{E 000\}, \{\sigma_z \frac{1}{2}00\}, \{E 0\frac{1}{2}0\}', \{\sigma_z \frac{1}{2}\frac{1}{2}0\}'$ |
| 7.28 | $P_cc (P_bb)$     | $\{E 000\}, \{\sigma_z \frac{1}{2}00\}, \{E \frac{1}{2}00\}', \{\sigma_z 000\}'$                     |
| 7.29 | $P_bc (P_cb)$     | $\{E 000\}, \{\sigma_z \frac{1}{2}00\}, \{E 00\frac{1}{2}\}', \{\sigma_z \frac{1}{2}0\frac{1}{2}\}'$ |

| No.   | Symbol                    | Elements                                                                                                                                                                                             |
|-------|---------------------------|------------------------------------------------------------------------------------------------------------------------------------------------------------------------------------------------------|
| 7.30  | $P_Cc$ ( $P_Bb$ )         | $\{E 000\}, \{\sigma_z \frac{1}{2}00\}, \{E 0\frac{1}{2}\frac{1}{2}\}', \{\sigma_z \frac{1}{2}\frac{1}{2}\frac{1}{2}\}'$                                                                             |
| 7.31  | $P_Ac$ ( $P_Ab$ )         | $\{E 000\}, \{\sigma_z \frac{1}{2}00\}, \{E \frac{1}{2}0\frac{1}{2}\}', \{\sigma_z 00\frac{1}{2}\}'$                                                                                                 |
| 8.32  | $Cm$ ( $Bm$ )             | $\{E 000\}, \{\sigma_z 000\}$                                                                                                                                                                        |
| 8.33  | $Cm1'$ ( $Bm1'$ )         | $\{E 000\}, \{\sigma_z 000\}, \{E 000\}', \{\sigma_z 000\}'$                                                                                                                                         |
| 8.34  | $Cm'$ ( $Bm'$ )           | $\{E 000\}, \{\sigma_z 000\}'$                                                                                                                                                                       |
| 8.35  | $C_cm$ ( $B_bm$ )         | $\{E 000\}, \{\sigma_z 000\}, \{E \frac{1}{2}00\}', \{\sigma_z \frac{1}{2}00\}'$                                                                                                                     |
| 8.36  | $C_am$ ( $B_am$ )         | $\{E 000\}, \{\sigma_z 000\}, \{E 0\frac{1}{2}\frac{1}{2}\}', \{\sigma_z 0\frac{1}{2}\frac{1}{2}\}'$                                                                                                 |
| 9.37  | $Cc$ ( $Bb$ )             | $\{E 000\}, \{\sigma_z \frac{1}{2}00\}$                                                                                                                                                              |
| 9.38  | $Cc1'$ ( $Bb1'$ )         | $\{E 000\}, \{\sigma_z \frac{1}{2}00\}, \{E 000\}', \{\sigma_z \frac{1}{2}00\}'$                                                                                                                     |
| 9.39  | $Cc'$ ( $Bb'$ )           | $\{E 000\}, \{\sigma_z \frac{1}{2}00\}'$                                                                                                                                                             |
| 9.40  | $C_cc$ ( $B_bb$ )         | $\{E 000\}, \{\sigma_z \frac{1}{2}00\}, \{E \frac{1}{2}00\}', \{\sigma_z 000\}'$                                                                                                                     |
| 9.41  | $C_ac$ ( $B_ab$ )         | $\{E 000\}, \{\sigma_z \frac{1}{2}00\}, \{E 0\frac{1}{2}\frac{1}{2}\}', \{\sigma_z \frac{1}{2}\frac{1}{2}\frac{1}{2}\}'$                                                                             |
| 10.42 | $P2/m$                    | $\{E 000\}, \{C_{2z} 000\}, \{I 000\}, \{\sigma_z 000\}$                                                                                                                                             |
| 10.43 | $P2/m1'$                  | $\{E 000\}, \{C_{2z} 000\}, \{I 000\}, \{\sigma_z 000\}, \{E 000\}', \{C_{2z} 000\}', \{I 000\}', \{\sigma_z 000\}'$                                                                                 |
| 10.44 | $P2'/m$                   | $\{E 000\}, \{C_{2z} 000\}', \{I 000\}', \{\sigma_z 000\}$                                                                                                                                           |
| 10.45 | $P2/m'$                   | $\{E 000\}, \{C_{2z} 000\}, \{I 000\}', \{\sigma_z 000\}'$                                                                                                                                           |
| 10.46 | $P2'/m'$                  | $\{E 000\}, \{C_{2z} 000\}', \{I 000\}, \{\sigma_z 000\}'$                                                                                                                                           |
| 10.47 | $P_a2/m$                  | $\{E 000\}, \{C_{2z} 000\}, \{I 000\}, \{\sigma_z 000\}, \{E 0\frac{1}{2}0\}', \{C_{2z} 0\frac{1}{2}0\}', \{I 0\frac{1}{2}0\}', \{\sigma_z 0\frac{1}{2}0\}'$                                         |
| 10.48 | $P_b2/m$ ( $P_c2/m$ )     | $\{E 000\}, \{C_{2z} 000\}, \{I 000\}, \{\sigma_z 000\}, \{E 00\frac{1}{2}\}', \{C_{2z} 00\frac{1}{2}\}', \{I 00\frac{1}{2}\}', \{\sigma_z 00\frac{1}{2}\}'$                                         |
| 10.49 | $P_C2/m$ ( $P_B2/m$ )     | $\{E 000\}, \{C_{2z} 000\}, \{I 000\}, \{\sigma_z 000\}, \{E 0\frac{1}{2}\frac{1}{2}\}', \{C_{2z} 0\frac{1}{2}\frac{1}{2}\}', \{I 0\frac{1}{2}\frac{1}{2}\}', \{\sigma_z 0\frac{1}{2}\frac{1}{2}\}'$ |
| 11.50 | $P2_1/m$                  | $\{E 000\}, \{C_{2z} 00\frac{1}{2}\}, \{I 00\frac{1}{2}\}, \{\sigma_z 000\}$                                                                                                                         |
| 11.51 | $P2_1/m1'$                | $\{E 000\}, \{C_{2z} 00\frac{1}{2}\}, \{I 00\frac{1}{2}\}, \{\sigma_z 000\}, \{E 000\}', \{C_{2z} 00\frac{1}{2}\}', \{I 00\frac{1}{2}\}', \{\sigma_z 000\}'$                                         |
| 11.52 | $P2_1'/m$                 | $\{E 000\}, \{C_{2z} 00\frac{1}{2}\}', \{I 00\frac{1}{2}\}', \{\sigma_z 000\}$                                                                                                                       |
| 11.53 | $P2_1/m'$                 | $\{E 000\}, \{C_{2z} 00\frac{1}{2}\}, \{I 00\frac{1}{2}\}', \{\sigma_z 000\}'$                                                                                                                       |
| 11.54 | $P2_1'/m'$                | $\{E 000\}, \{C_{2z} 00\frac{1}{2}\}', \{I 00\frac{1}{2}\}, \{\sigma_z 000\}'$                                                                                                                       |
| 11.55 | $P_a2_1/m$                | $\{E 000\}, \{C_{2z} 00\frac{1}{2}\}, \{I 00\frac{1}{2}\}, \{\sigma_z 000\}, \{E 0\frac{1}{2}0\}', \{C_{2z} 0\frac{1}{2}\frac{1}{2}\}', \{I 0\frac{1}{2}\frac{1}{2}\}', \{\sigma_z 0\frac{1}{2}0\}'$ |
| 11.56 | $P_b2_1/m$ ( $P_c2_1/m$ ) | $\{E 000\}, \{C_{2z} 00\frac{1}{2}\}, \{I 00\frac{1}{2}\}, \{\sigma_z 000\}, \{E 00\frac{1}{2}\}', \{C_{2z} 000\}', \{I 000\}', \{\sigma_z 00\frac{1}{2}\}'$                                         |
| 11.57 | $P_C2_1/m$ ( $P_B2_1/m$ ) | $\{E 000\}, \{C_{2z} 00\frac{1}{2}\}, \{I 00\frac{1}{2}\}, \{\sigma_z 000\}, \{E 0\frac{1}{2}\frac{1}{2}\}', \{C_{2z} 0\frac{1}{2}0\}', \{I 0\frac{1}{2}0\}', \{\sigma_z 0\frac{1}{2}\frac{1}{2}\}'$ |
| 12.58 | $C2/m$ ( $B2/m$ )         | $\{E 000\}, \{C_{2z} 000\}, \{I 000\}, \{\sigma_z 000\}$                                                                                                                                             |
| 12.59 | $C2/m1'$ ( $B2/m1'$ )     | $\{E 000\}, \{C_{2z} 000\}, \{I 000\}, \{\sigma_z 000\}, \{E 000\}', \{C_{2z} 000\}', \{I 000\}', \{\sigma_z 000\}'$                                                                                 |
| 12.60 | $C2'/m$ ( $B2'/m$ )       | $\{E 000\}, \{C_{2z} 000\}', \{I 000\}', \{\sigma_z 000\}$                                                                                                                                           |
| 12.61 | $C2/m'$ ( $B2/m'$ )       | $\{E 000\}, \{C_{2z} 000\}, \{I 000\}', \{\sigma_z 000\}'$                                                                                                                                           |
| 12.62 | $C2'/m'$ ( $B2'/m'$ )     | $\{E 000\}, \{C_{2z} 000\}', \{I 000\}, \{\sigma_z 000\}'$                                                                                                                                           |
| 12.63 | $C_c2/m$ ( $B_b2/m$ )     | $\{E 000\}, \{C_{2z} 000\}, \{I 000\}, \{\sigma_z 000\}, \{E \frac{1}{2}00\}', \{C_{2z} \frac{1}{2}00\}', \{I \frac{1}{2}00\}', \{\sigma_z \frac{1}{2}00\}'$                                         |
| 12.64 | $C_a2/m$ ( $B_a2/m$ )     | $\{E 000\}, \{C_{2z} 000\}, \{I 000\}, \{\sigma_z 000\}, \{E 0\frac{1}{2}\frac{1}{2}\}', \{C_{2z} 0\frac{1}{2}\frac{1}{2}\}', \{I 0\frac{1}{2}\frac{1}{2}\}', \{\sigma_z 0\frac{1}{2}\frac{1}{2}\}'$ |
| 13.65 | $P2/c$ ( $P2/b$ )         | $\{E 000\}, \{C_{2z} 000\}, \{I \frac{1}{2}00\}, \{\sigma_z \frac{1}{2}00\}$                                                                                                                         |

| No.   | Symbol                | Elements                                                                                                                                                                                                                                           |
|-------|-----------------------|----------------------------------------------------------------------------------------------------------------------------------------------------------------------------------------------------------------------------------------------------|
| 13.66 | $P2/c1' (P2/b1')$     | $\{E 000\}, \{C_{2z} 000\}, \{I \frac{1}{2}00\}, \{\sigma_z \frac{1}{2}00\}, \{E 000\}', \{C_{2z} 000\}', \{I \frac{1}{2}00\}', \{\sigma_z \frac{1}{2}00\}'$                                                                                       |
| 13.67 | $P2'/c (P2'/b)$       | $\{E 000\}, \{C_{2z} 000\}', \{I \frac{1}{2}00\}', \{\sigma_z \frac{1}{2}00\}$                                                                                                                                                                     |
| 13.68 | $P2/c' (P2/b')$       | $\{E 000\}, \{C_{2z} 000\}, \{I \frac{1}{2}00\}', \{\sigma_z \frac{1}{2}00\}'$                                                                                                                                                                     |
| 13.69 | $P2'/c' (P2'/b')$     | $\{E 000\}, \{C_{2z} 000\}', \{I \frac{1}{2}00\}, \{\sigma_z \frac{1}{2}00\}'$                                                                                                                                                                     |
| 13.70 | $P_a2/c (P_a2/b)$     | $\{E 000\}, \{C_{2z} 000\}, \{I \frac{1}{2}00\}, \{\sigma_z \frac{1}{2}00\}, \{E 0\frac{1}{2}0\}', \{C_{2z} 0\frac{1}{2}0\}', \{I \frac{1}{2}\frac{1}{2}0\}', \{\sigma_z \frac{1}{2}\frac{1}{2}0\}'$                                               |
| 13.71 | $P_b2/c (P_c2/b)$     | $\{E 000\}, \{C_{2z} 000\}, \{I \frac{1}{2}00\}, \{\sigma_z \frac{1}{2}00\}, \{E 00\frac{1}{2}\}', \{C_{2z} 00\frac{1}{2}\}', \{I 0\frac{1}{2}\frac{1}{2}\}', \{\sigma_z 0\frac{1}{2}\frac{1}{2}\}'$                                               |
| 13.72 | $P_c2/c (P_b2/b)$     | $\{E 000\}, \{C_{2z} 000\}, \{I \frac{1}{2}00\}, \{\sigma_z \frac{1}{2}00\}, \{E \frac{1}{2}00\}', \{C_{2z} \frac{1}{2}00\}', \{I 000\}', \{\sigma_z 000\}'$                                                                                       |
| 13.73 | $P_A2/c (P_A2/b)$     | $\{E 000\}, \{C_{2z} 000\}, \{I \frac{1}{2}00\}, \{\sigma_z \frac{1}{2}00\}, \{E \frac{1}{2}0\frac{1}{2}\}', \{C_{2z} \frac{1}{2}0\frac{1}{2}\}', \{I 00\frac{1}{2}\}', \{\sigma_z 00\frac{1}{2}\}'$                                               |
| 13.74 | $P_C2/c (P_B2/b)$     | $\{E 000\}, \{C_{2z} 000\}, \{I \frac{1}{2}00\}, \{\sigma_z \frac{1}{2}00\}, \{E 0\frac{1}{2}\frac{1}{2}\}', \{C_{2z} 0\frac{1}{2}\frac{1}{2}\}', \{I \frac{1}{2}\frac{1}{2}\frac{1}{2}\}', \{\sigma_z \frac{1}{2}\frac{1}{2}\frac{1}{2}\}'$       |
| 14.75 | $P2_1/c (P2_1/b)$     | $\{E 000\}, \{C_{2z} 00\frac{1}{2}\}, \{I \frac{1}{2}0\frac{1}{2}\}, \{\sigma_z \frac{1}{2}00\}$                                                                                                                                                   |
| 14.76 | $P2_1/c1' (P2_1/b1')$ | $\{E 000\}, \{C_{2z} 00\frac{1}{2}\}, \{I \frac{1}{2}0\frac{1}{2}\}, \{\sigma_z \frac{1}{2}00\}, \{E 000\}', \{C_{2z} 00\frac{1}{2}\}', \{I \frac{1}{2}0\frac{1}{2}\}', \{\sigma_z \frac{1}{2}00\}'$                                               |
| 14.77 | $P2'_1/c (P2'_1/b)$   | $\{E 000\}, \{C_{2z} 00\frac{1}{2}\}', \{I \frac{1}{2}0\frac{1}{2}\}', \{\sigma_z \frac{1}{2}00\}$                                                                                                                                                 |
| 14.78 | $P2_1/c' (P2_1/b')$   | $\{E 000\}, \{C_{2z} 00\frac{1}{2}\}, \{I \frac{1}{2}0\frac{1}{2}\}', \{\sigma_z \frac{1}{2}00\}'$                                                                                                                                                 |
| 14.79 | $P2'_1/c' (P2'_1/b')$ | $\{E 000\}, \{C_{2z} 00\frac{1}{2}\}', \{I \frac{1}{2}0\frac{1}{2}\}, \{\sigma_z \frac{1}{2}00\}'$                                                                                                                                                 |
| 14.80 | $P_a2_1/c (P_a2_1/b)$ | $\{E 000\}, \{C_{2z} 00\frac{1}{2}\}, \{I \frac{1}{2}0\frac{1}{2}\}, \{\sigma_z \frac{1}{2}00\}, \{E 0\frac{1}{2}0\}', \{C_{2z} 0\frac{1}{2}\frac{1}{2}\}', \{I \frac{1}{2}\frac{1}{2}\frac{1}{2}\}', \{\sigma_z \frac{1}{2}\frac{1}{2}0\}'$       |
| 14.81 | $P_b2_1/c (P_c2_1/b)$ | $\{E 000\}, \{C_{2z} 00\frac{1}{2}\}, \{I \frac{1}{2}0\frac{1}{2}\}, \{\sigma_z \frac{1}{2}00\}, \{E 00\frac{1}{2}\}', \{C_{2z} 000\}', \{I \frac{1}{2}00\}', \{\sigma_z 0\frac{1}{2}\frac{1}{2}\}'$                                               |
| 14.82 | $P_c2_1/c (P_b2_1/b)$ | $\{E 000\}, \{C_{2z} 00\frac{1}{2}\}, \{I \frac{1}{2}0\frac{1}{2}\}, \{\sigma_z \frac{1}{2}00\}, \{E \frac{1}{2}00\}', \{C_{2z} \frac{1}{2}0\frac{1}{2}\}', \{I 00\frac{1}{2}\}', \{\sigma_z 000\}'$                                               |
| 14.83 | $P_A2_1/c (P_A2_1/b)$ | $\{E 000\}, \{C_{2z} 00\frac{1}{2}\}, \{I \frac{1}{2}0\frac{1}{2}\}, \{\sigma_z \frac{1}{2}00\}, \{E \frac{1}{2}0\frac{1}{2}\}', \{C_{2z} \frac{1}{2}00\}', \{I 000\}', \{\sigma_z 00\frac{1}{2}\}'$                                               |
| 14.84 | $P_C2_1/c (P_B2_1/b)$ | $\{E 000\}, \{C_{2z} 00\frac{1}{2}\}, \{I \frac{1}{2}0\frac{1}{2}\}, \{\sigma_z \frac{1}{2}00\}, \{E 0\frac{1}{2}\frac{1}{2}\}', \{C_{2z} 0\frac{1}{2}0\}', \{I \frac{1}{2}\frac{1}{2}0\}', \{\sigma_z \frac{1}{2}\frac{1}{2}\frac{1}{2}\}'$       |
| 15.85 | $C2/c (B2/b)$         | $\{E 000\}, \{C_{2z} 000\}, \{I \frac{1}{2}00\}, \{\sigma_z \frac{1}{2}00\}$                                                                                                                                                                       |
| 15.86 | $C2/c1' (B2/b1')$     | $\{E 000\}, \{C_{2z} 000\}, \{I \frac{1}{2}00\}, \{\sigma_z \frac{1}{2}00\}, \{E 000\}', \{C_{2z} 000\}', \{I \frac{1}{2}00\}', \{\sigma_z \frac{1}{2}00\}'$                                                                                       |
| 15.87 | $C2'/c (B2'/b)$       | $\{E 000\}, \{C_{2z} 000\}', \{I \frac{1}{2}00\}', \{\sigma_z \frac{1}{2}00\}$                                                                                                                                                                     |
| 15.88 | $C2/c' (B2/b')$       | $\{E 000\}, \{C_{2z} 000\}, \{I \frac{1}{2}00\}', \{\sigma_z \frac{1}{2}00\}'$                                                                                                                                                                     |
| 15.89 | $C2'/c' (B2'/b')$     | $\{E 000\}, \{C_{2z} 000\}', \{I \frac{1}{2}00\}, \{\sigma_z \frac{1}{2}00\}'$                                                                                                                                                                     |
| 15.90 | $C_c2/c (B_b2/b)$     | $\{E 000\}, \{C_{2z} 000\}, \{I \frac{1}{2}00\}, \{\sigma_z \frac{1}{2}00\}, \{E \frac{1}{2}00\}', \{C_{2z} \frac{1}{2}00\}', \{I 000\}', \{\sigma_z 000\}'$                                                                                       |
| 15.91 | $C_a2/c (B_a2/b)$     | $\{E 000\}, \{C_{2z} 000\}, \{I \frac{1}{2}00\}, \{\sigma_z \frac{1}{2}00\}, \{E 0\frac{1}{2}\frac{1}{2}\}', \{C_{2z} 0\frac{1}{2}\frac{1}{2}\}', \{I \frac{1}{2}\frac{1}{2}\frac{1}{2}\}', \{\sigma_z \frac{1}{2}\frac{1}{2}\frac{1}{2}\}'$       |
| 16.1  | $P222$                | $\{E 000\}, \{C_{2x} 000\}, \{C_{2y} 000\}, \{C_{2z} 000\}$                                                                                                                                                                                        |
| 16.2  | $P2221'$              | $\{E 000\}, \{C_{2x} 000\}, \{C_{2y} 000\}, \{C_{2z} 000\}, \{E 000\}', \{C_{2x} 000\}', \{C_{2y} 000\}', \{C_{2z} 000\}'$                                                                                                                         |
| 16.3  | $P2'2'2$              | $\{E 000\}, \{C_{2x} 000\}', \{C_{2y} 000\}', \{C_{2z} 000\}$                                                                                                                                                                                      |
| 16.4  | $P_a222$              | $\{E 000\}, \{C_{2x} 000\}, \{C_{2y} 000\}, \{C_{2z} 000\}, \{E 0\frac{1}{2}0\}', \{C_{2x} 0\frac{1}{2}0\}', \{C_{2y} 0\frac{1}{2}0\}', \{C_{2z} 0\frac{1}{2}0\}'$                                                                                 |
| 16.5  | $P_C222$              | $\{E 000\}, \{C_{2x} 000\}, \{C_{2y} 000\}, \{C_{2z} 000\}, \{E \frac{1}{2}\frac{1}{2}0\}', \{C_{2x} \frac{1}{2}\frac{1}{2}0\}', \{C_{2y} \frac{1}{2}\frac{1}{2}0\}', \{C_{2z} \frac{1}{2}\frac{1}{2}0\}'$                                         |
| 16.6  | $P_I222$              | $\{E 000\}, \{C_{2x} 000\}, \{C_{2y} 000\}, \{C_{2z} 000\}, \{E \frac{1}{2}\frac{1}{2}\frac{1}{2}\}', \{C_{2x} \frac{1}{2}\frac{1}{2}\frac{1}{2}\}', \{C_{2y} \frac{1}{2}\frac{1}{2}\frac{1}{2}\}', \{C_{2z} \frac{1}{2}\frac{1}{2}\frac{1}{2}\}'$ |
| 17.7  | $P222_1$              | $\{E 000\}, \{C_{2x} 00\frac{1}{2}\}, \{C_{2y} 000\}, \{C_{2z} 00\frac{1}{2}\}$                                                                                                                                                                    |
| 17.8  | $P222_11'$            | $\{E 000\}, \{C_{2x} 00\frac{1}{2}\}, \{C_{2y} 000\}, \{C_{2z} 00\frac{1}{2}\}, \{E 000\}', \{C_{2x} 00\frac{1}{2}\}', \{C_{2y} 000\}', \{C_{2z} 00\frac{1}{2}\}'$                                                                                 |
| 17.9  | $P2'2'2_1$            | $\{E 000\}, \{C_{2x} 00\frac{1}{2}\}', \{C_{2y} 000\}', \{C_{2z} 00\frac{1}{2}\}$                                                                                                                                                                  |
| 17.10 | $P22'2'_1$            | $\{E 000\}, \{C_{2x} 00\frac{1}{2}\}, \{C_{2y} 000\}', \{C_{2z} 00\frac{1}{2}\}'$                                                                                                                                                                  |



| No.   | Symbol         | Elements                                                                                                                                                                                                                                           |
|-------|----------------|----------------------------------------------------------------------------------------------------------------------------------------------------------------------------------------------------------------------------------------------------|
| 17.11 | $P_a222_1$     | $\{E 000\}, \{C_{2x} 00\frac{1}{2}\}, \{C_{2y} 000\}, \{C_{2z} 00\frac{1}{2}\}, \{E 0\frac{1}{2}0\}', \{C_{2x} 0\frac{1}{2}\frac{1}{2}\}', \{C_{2y} 0\frac{1}{2}0\}', \{C_{2z} 0\frac{1}{2}\frac{1}{2}\}'$                                         |
| 17.12 | $P_c222_1$     | $\{E 000\}, \{C_{2x} 00\frac{1}{2}\}, \{C_{2y} 000\}, \{C_{2z} 00\frac{1}{2}\}, \{E 00\frac{1}{2}\}', \{C_{2x} 000\}', \{C_{2y} 00\frac{1}{2}\}', \{C_{2z} 000\}'$                                                                                 |
| 17.13 | $P_A222_1$     | $\{E 000\}, \{C_{2x} 00\frac{1}{2}\}, \{C_{2y} 000\}, \{C_{2z} 00\frac{1}{2}\}, \{E \frac{1}{2}0\frac{1}{2}\}', \{C_{2x} \frac{1}{2}00\}', \{C_{2y} \frac{1}{2}0\frac{1}{2}\}', \{C_{2z} \frac{1}{2}00\}'$                                         |
| 17.14 | $P_C222_1$     | $\{E 000\}, \{C_{2x} 00\frac{1}{2}\}, \{C_{2y} 000\}, \{C_{2z} 00\frac{1}{2}\}, \{E \frac{1}{2}\frac{1}{2}0\}', \{C_{2x} \frac{1}{2}\frac{1}{2}\frac{1}{2}\}', \{C_{2y} \frac{1}{2}\frac{1}{2}0\}', \{C_{2z} \frac{1}{2}\frac{1}{2}\frac{1}{2}\}'$ |
| 17.15 | $P_I222_1$     | $\{E 000\}, \{C_{2x} 00\frac{1}{2}\}, \{C_{2y} 000\}, \{C_{2z} 00\frac{1}{2}\}, \{E \frac{1}{2}\frac{1}{2}\frac{1}{2}\}', \{C_{2x} \frac{1}{2}\frac{1}{2}0\}', \{C_{2y} \frac{1}{2}\frac{1}{2}\frac{1}{2}\}', \{C_{2z} \frac{1}{2}\frac{1}{2}0\}'$ |
| 18.16 | $P2_12_12$     | $\{E 000\}, \{C_{2x} \frac{1}{2}\frac{1}{2}0\}, \{C_{2y} \frac{1}{2}\frac{1}{2}0\}, \{C_{2z} 000\}$                                                                                                                                                |
| 18.17 | $P2_12_121'$   | $\{E 000\}, \{C_{2x} \frac{1}{2}\frac{1}{2}0\}, \{C_{2y} \frac{1}{2}\frac{1}{2}0\}, \{C_{2z} 000\}, \{E 000\}', \{C_{2x} \frac{1}{2}\frac{1}{2}0\}', \{C_{2y} \frac{1}{2}\frac{1}{2}0\}', \{C_{2z} 000\}'$                                         |
| 18.18 | $P2_1'2_1'2$   | $\{E 000\}, \{C_{2x} \frac{1}{2}\frac{1}{2}0\}', \{C_{2y} \frac{1}{2}\frac{1}{2}0\}', \{C_{2z} 000\}$                                                                                                                                              |
| 18.19 | $P2_1'2_1'2'$  | $\{E 000\}, \{C_{2x} \frac{1}{2}\frac{1}{2}0\}, \{C_{2y} \frac{1}{2}\frac{1}{2}0\}', \{C_{2z} 000\}'$                                                                                                                                              |
| 18.20 | $P_a2_12_12$   | $\{E 000\}, \{C_{2x} \frac{1}{2}\frac{1}{2}0\}, \{C_{2y} \frac{1}{2}\frac{1}{2}0\}, \{C_{2z} 000\}, \{E 0\frac{1}{2}0\}', \{C_{2x} \frac{1}{2}00\}', \{C_{2y} \frac{1}{2}00\}', \{C_{2z} 0\frac{1}{2}0\}'$                                         |
| 18.21 | $P_c2_12_12$   | $\{E 000\}, \{C_{2x} \frac{1}{2}\frac{1}{2}0\}, \{C_{2y} \frac{1}{2}\frac{1}{2}0\}, \{C_{2z} 000\}, \{E 00\frac{1}{2}\}', \{C_{2x} \frac{1}{2}\frac{1}{2}\frac{1}{2}\}', \{C_{2y} \frac{1}{2}\frac{1}{2}\frac{1}{2}\}', \{C_{2z} 00\frac{1}{2}\}'$ |
| 18.22 | $P_A2_12_12$   | $\{E 000\}, \{C_{2x} \frac{1}{2}\frac{1}{2}0\}, \{C_{2y} \frac{1}{2}\frac{1}{2}0\}, \{C_{2z} 000\}, \{E \frac{1}{2}0\frac{1}{2}\}', \{C_{2x} 0\frac{1}{2}\frac{1}{2}\}', \{C_{2y} 0\frac{1}{2}\frac{1}{2}\}', \{C_{2z} \frac{1}{2}0\frac{1}{2}\}'$ |
| 18.23 | $P_C2_12_12$   | $\{E 000\}, \{C_{2x} \frac{1}{2}\frac{1}{2}0\}, \{C_{2y} \frac{1}{2}\frac{1}{2}0\}, \{C_{2z} 000\}, \{E \frac{1}{2}\frac{1}{2}0\}', \{C_{2x} 000\}', \{C_{2y} 000\}', \{C_{2z} \frac{1}{2}\frac{1}{2}0\}'$                                         |
| 18.24 | $P_I2_12_12$   | $\{E 000\}, \{C_{2x} \frac{1}{2}\frac{1}{2}0\}, \{C_{2y} \frac{1}{2}\frac{1}{2}0\}, \{C_{2z} 000\}, \{E \frac{1}{2}\frac{1}{2}\frac{1}{2}\}', \{C_{2x} 00\frac{1}{2}\}', \{C_{2y} 00\frac{1}{2}\}', \{C_{2z} \frac{1}{2}\frac{1}{2}\frac{1}{2}\}'$ |
| 19.25 | $P2_12_12_1$   | $\{E 000\}, \{C_{2x} 0\frac{1}{2}\frac{1}{2}\}, \{C_{2y} \frac{1}{2}\frac{1}{2}0\}, \{C_{2z} \frac{1}{2}0\frac{1}{2}\}$                                                                                                                            |
| 19.26 | $P2_12_12_11'$ | $\{E 000\}, \{C_{2x} 0\frac{1}{2}\frac{1}{2}\}, \{C_{2y} \frac{1}{2}\frac{1}{2}0\}, \{C_{2z} \frac{1}{2}0\frac{1}{2}\}, \{E 000\}', \{C_{2x} 0\frac{1}{2}\frac{1}{2}\}', \{C_{2y} \frac{1}{2}\frac{1}{2}0\}', \{C_{2z} \frac{1}{2}0\frac{1}{2}\}'$ |
| 19.27 | $P2_1'2_1'2_1$ | $\{E 000\}, \{C_{2x} 0\frac{1}{2}\frac{1}{2}\}', \{C_{2y} \frac{1}{2}\frac{1}{2}0\}', \{C_{2z} \frac{1}{2}0\frac{1}{2}\}$                                                                                                                          |
| 19.28 | $P_a2_12_12_1$ | $\{E 000\}, \{C_{2x} 0\frac{1}{2}\frac{1}{2}\}, \{C_{2y} \frac{1}{2}\frac{1}{2}0\}, \{C_{2z} \frac{1}{2}0\frac{1}{2}\}, \{E 0\frac{1}{2}0\}', \{C_{2x} 00\frac{1}{2}\}', \{C_{2y} \frac{1}{2}00\}', \{C_{2z} \frac{1}{2}\frac{1}{2}\frac{1}{2}\}'$ |
| 19.29 | $P_C2_12_12_1$ | $\{E 000\}, \{C_{2x} 0\frac{1}{2}\frac{1}{2}\}, \{C_{2y} \frac{1}{2}\frac{1}{2}0\}, \{C_{2z} \frac{1}{2}0\frac{1}{2}\}, \{E \frac{1}{2}\frac{1}{2}0\}', \{C_{2x} \frac{1}{2}0\frac{1}{2}\}', \{C_{2y} 000\}', \{C_{2z} 0\frac{1}{2}\frac{1}{2}\}'$ |
| 19.30 | $P_I2_12_12_1$ | $\{E 000\}, \{C_{2x} 0\frac{1}{2}\frac{1}{2}\}, \{C_{2y} \frac{1}{2}\frac{1}{2}0\}, \{C_{2z} \frac{1}{2}0\frac{1}{2}\}, \{E \frac{1}{2}\frac{1}{2}\frac{1}{2}\}', \{C_{2x} \frac{1}{2}00\}', \{C_{2y} 00\frac{1}{2}\}', \{C_{2z} 0\frac{1}{2}0\}'$ |
| 20.31 | $C222_1$       | $\{E 000\}, \{C_{2x} 000\}, \{C_{2y} 00\frac{1}{2}\}, \{C_{2z} 00\frac{1}{2}\}$                                                                                                                                                                    |
| 20.32 | $C222_11'$     | $\{E 000\}, \{C_{2x} 000\}, \{C_{2y} 00\frac{1}{2}\}, \{C_{2z} 00\frac{1}{2}\}, \{E 000\}', \{C_{2x} 000\}', \{C_{2y} 00\frac{1}{2}\}', \{C_{2z} 00\frac{1}{2}\}'$                                                                                 |
| 20.33 | $C2'2'2_1$     | $\{E 000\}, \{C_{2x} 000\}', \{C_{2y} 00\frac{1}{2}\}', \{C_{2z} 00\frac{1}{2}\}$                                                                                                                                                                  |
| 20.34 | $C22'2'_1$     | $\{E 000\}, \{C_{2x} 000\}, \{C_{2y} 00\frac{1}{2}\}', \{C_{2z} 00\frac{1}{2}\}'$                                                                                                                                                                  |
| 20.35 | $C_c222_1$     | $\{E 000\}, \{C_{2x} 000\}, \{C_{2y} 00\frac{1}{2}\}, \{C_{2z} 00\frac{1}{2}\}, \{E 00\frac{1}{2}\}', \{C_{2x} 00\frac{1}{2}\}', \{C_{2y} 000\}', \{C_{2z} 000\}'$                                                                                 |
| 20.36 | $C_a222_1$     | $\{E 000\}, \{C_{2x} 000\}, \{C_{2y} 00\frac{1}{2}\}, \{C_{2z} 00\frac{1}{2}\}, \{E \frac{1}{2}\frac{1}{2}0\}', \{C_{2x} \frac{1}{2}\frac{1}{2}0\}', \{C_{2y} \frac{1}{2}\frac{1}{2}\frac{1}{2}\}', \{C_{2z} \frac{1}{2}\frac{1}{2}\frac{1}{2}\}'$ |
| 20.37 | $C_A222_1$     | $\{E 000\}, \{C_{2x} 000\}, \{C_{2y} 00\frac{1}{2}\}, \{C_{2z} 00\frac{1}{2}\}, \{E \frac{1}{2}\frac{1}{2}\frac{1}{2}\}', \{C_{2x} \frac{1}{2}\frac{1}{2}\frac{1}{2}\}', \{C_{2y} \frac{1}{2}\frac{1}{2}0\}', \{C_{2z} \frac{1}{2}\frac{1}{2}0\}'$ |
| 21.38 | $C'222$        | $\{E 000\}, \{C_{2x} 000\}, \{C_{2y} 000\}, \{C_{2z} 000\}$                                                                                                                                                                                        |
| 21.39 | $C'2221'$      | $\{E 000\}, \{C_{2x} 000\}, \{C_{2y} 000\}, \{C_{2z} 000\}, \{E 000\}', \{C_{2x} 000\}', \{C_{2y} 000\}', \{C_{2z} 000\}'$                                                                                                                         |
| 21.40 | $C2'2'2$       | $\{E 000\}, \{C_{2x} 000\}', \{C_{2y} 000\}', \{C_{2z} 000\}$                                                                                                                                                                                      |
| 21.41 | $C22'2'$       | $\{E 000\}, \{C_{2x} 000\}, \{C_{2y} 000\}', \{C_{2z} 000\}'$                                                                                                                                                                                      |
| 21.42 | $C_c222$       | $\{E 000\}, \{C_{2x} 000\}, \{C_{2y} 000\}, \{C_{2z} 000\}, \{E 00\frac{1}{2}\}', \{C_{2x} 00\frac{1}{2}\}', \{C_{2y} 00\frac{1}{2}\}', \{C_{2z} 00\frac{1}{2}\}'$                                                                                 |
| 21.43 | $C_a222$       | $\{E 000\}, \{C_{2x} 000\}, \{C_{2y} 000\}, \{C_{2z} 000\}, \{E \frac{1}{2}\frac{1}{2}0\}', \{C_{2x} \frac{1}{2}\frac{1}{2}0\}', \{C_{2y} \frac{1}{2}\frac{1}{2}0\}', \{C_{2z} \frac{1}{2}\frac{1}{2}0\}'$                                         |
| 21.44 | $C_A222$       | $\{E 000\}, \{C_{2x} 000\}, \{C_{2y} 000\}, \{C_{2z} 000\}, \{E \frac{1}{2}\frac{1}{2}\frac{1}{2}\}', \{C_{2x} \frac{1}{2}\frac{1}{2}\frac{1}{2}\}', \{C_{2y} \frac{1}{2}\frac{1}{2}\frac{1}{2}\}', \{C_{2z} \frac{1}{2}\frac{1}{2}\frac{1}{2}\}'$ |
| 22.45 | $F222$         | $\{E 000\}, \{C_{2x} 000\}, \{C_{2y} 000\}, \{C_{2z} 000\}$                                                                                                                                                                                        |
| 22.46 | $F2221'$       | $\{E 000\}, \{C_{2x} 000\}, \{C_{2y} 000\}, \{C_{2z} 000\}, \{E 000\}', \{C_{2x} 000\}', \{C_{2y} 000\}', \{C_{2z} 000\}'$                                                                                                                         |

| No.   | Symbol         | Elements                                                                                                                                                                                                                                                   |
|-------|----------------|------------------------------------------------------------------------------------------------------------------------------------------------------------------------------------------------------------------------------------------------------------|
| 22.47 | $F2'2'2$       | $\{E 000\}, \{C_{2x} 000\}', \{C_{2y} 000\}', \{C_{2z} 000\}$                                                                                                                                                                                              |
| 22.48 | $F_s222$       | $\{E 000\}, \{C_{2x} 000\}, \{C_{2y} 000\}, \{C_{2z} 000\}, \{E \frac{1}{2}\frac{1}{2}\frac{1}{2}\}', \{C_{2x} \frac{1}{2}\frac{1}{2}\frac{1}{2}\}', \{C_{2y} \frac{1}{2}\frac{1}{2}\frac{1}{2}\}', \{C_{2z} \frac{1}{2}\frac{1}{2}\frac{1}{2}\}'$         |
| 23.49 | $I222$         | $\{E 000\}, \{C_{2x} 000\}, \{C_{2y} 000\}, \{C_{2z} 000\}$                                                                                                                                                                                                |
| 23.50 | $I2221'$       | $\{E 000\}, \{C_{2x} 000\}, \{C_{2y} 000\}, \{C_{2z} 000\}, \{E 000\}', \{C_{2x} 000\}', \{C_{2y} 000\}', \{C_{2z} 000\}'$                                                                                                                                 |
| 23.51 | $I2'2'2$       | $\{E 000\}, \{C_{2x} 000\}', \{C_{2y} 000\}', \{C_{2z} 000\}$                                                                                                                                                                                              |
| 23.52 | $I_c222$       | $\{E 000\}, \{C_{2x} 000\}, \{C_{2y} 000\}, \{C_{2z} 000\}, \{E \frac{1}{2}\frac{1}{2}0\}', \{C_{2x} \frac{1}{2}\frac{1}{2}0\}', \{C_{2y} \frac{1}{2}\frac{1}{2}0\}', \{C_{2z} \frac{1}{2}\frac{1}{2}0\}'$                                                 |
| 24.53 | $I2_12_12_1$   | $\{E 000\}, \{C_{2x} 0\frac{1}{2}\frac{1}{2}\}, \{C_{2y} \frac{1}{2}\frac{1}{2}0\}, \{C_{2z} \frac{1}{2}0\frac{1}{2}\}$                                                                                                                                    |
| 24.54 | $I2_12_12_11'$ | $\{E 000\}, \{C_{2x} 0\frac{1}{2}\frac{1}{2}\}, \{C_{2y} \frac{1}{2}\frac{1}{2}0\}, \{C_{2z} \frac{1}{2}0\frac{1}{2}\}, \{E 000\}', \{C_{2x} 0\frac{1}{2}\frac{1}{2}\}', \{C_{2y} \frac{1}{2}\frac{1}{2}0\}', \{C_{2z} \frac{1}{2}0\frac{1}{2}\}'$         |
| 24.55 | $I2'_12'_12_1$ | $\{E 000\}, \{C_{2x} 0\frac{1}{2}\frac{1}{2}\}', \{C_{2y} \frac{1}{2}\frac{1}{2}0\}', \{C_{2z} \frac{1}{2}0\frac{1}{2}\}$                                                                                                                                  |
| 24.56 | $I_c2_12_12_1$ | $\{E 000\}, \{C_{2x} 0\frac{1}{2}\frac{1}{2}\}, \{C_{2y} \frac{1}{2}\frac{1}{2}0\}, \{C_{2z} \frac{1}{2}0\frac{1}{2}\}, \{E \frac{1}{2}\frac{1}{2}0\}', \{C_{2x} \frac{1}{2}\frac{1}{2}0\}', \{C_{2y} 000\}', \{C_{2z} 0\frac{1}{2}\frac{1}{2}\}'$         |
| 25.57 | $Pmm2$         | $\{E 000\}, \{C_{2z} 000\}, \{\sigma_x 000\}, \{\sigma_y 000\}$                                                                                                                                                                                            |
| 25.58 | $Pmm21'$       | $\{E 000\}, \{C_{2z} 000\}, \{\sigma_x 000\}, \{\sigma_y 000\}, \{E 000\}', \{C_{2z} 000\}', \{\sigma_x 000\}', \{\sigma_y 000\}'$                                                                                                                         |
| 25.59 | $Pm'm2'$       | $\{E 000\}, \{C_{2z} 000\}', \{\sigma_x 000\}', \{\sigma_y 000\}$                                                                                                                                                                                          |
| 25.60 | $Pm'm'2$       | $\{E 000\}, \{C_{2z} 000\}, \{\sigma_x 000\}', \{\sigma_y 000\}'$                                                                                                                                                                                          |
| 25.61 | $P_cmm2$       | $\{E 000\}, \{C_{2z} 000\}, \{\sigma_x 000\}, \{\sigma_y 000\}, \{E 00\frac{1}{2}\}', \{C_{2z} 00\frac{1}{2}\}', \{\sigma_x 00\frac{1}{2}\}', \{\sigma_y 00\frac{1}{2}\}'$                                                                                 |
| 25.62 | $P_a mm2$      | $\{E 000\}, \{C_{2z} 000\}, \{\sigma_x 000\}, \{\sigma_y 000\}, \{E 0\frac{1}{2}0\}', \{C_{2z} 0\frac{1}{2}0\}', \{\sigma_x 0\frac{1}{2}0\}', \{\sigma_y 0\frac{1}{2}0\}'$                                                                                 |
| 25.63 | $P_C mm2$      | $\{E 000\}, \{C_{2z} 000\}, \{\sigma_x 000\}, \{\sigma_y 000\}, \{E \frac{1}{2}\frac{1}{2}0\}', \{C_{2z} \frac{1}{2}\frac{1}{2}0\}', \{\sigma_x \frac{1}{2}\frac{1}{2}0\}', \{\sigma_y \frac{1}{2}\frac{1}{2}0\}'$                                         |
| 25.64 | $P_A mm2$      | $\{E 000\}, \{C_{2z} 000\}, \{\sigma_x 000\}, \{\sigma_y 000\}, \{E \frac{1}{2}0\frac{1}{2}\}', \{C_{2z} \frac{1}{2}0\frac{1}{2}\}', \{\sigma_x \frac{1}{2}0\frac{1}{2}\}', \{\sigma_y \frac{1}{2}0\frac{1}{2}\}'$                                         |
| 25.65 | $P_I mm2$      | $\{E 000\}, \{C_{2z} 000\}, \{\sigma_x 000\}, \{\sigma_y 000\}, \{E \frac{1}{2}\frac{1}{2}\frac{1}{2}\}', \{C_{2z} \frac{1}{2}\frac{1}{2}\frac{1}{2}\}', \{\sigma_x \frac{1}{2}\frac{1}{2}\frac{1}{2}\}', \{\sigma_y \frac{1}{2}\frac{1}{2}\frac{1}{2}\}'$ |
| 26.66 | $Pmc2_1$       | $\{E 000\}, \{C_{2z} 00\frac{1}{2}\}, \{\sigma_x 000\}, \{\sigma_y 00\frac{1}{2}\}$                                                                                                                                                                        |
| 26.67 | $Pmc2_11'$     | $\{E 000\}, \{C_{2z} 00\frac{1}{2}\}, \{\sigma_x 000\}, \{\sigma_y 00\frac{1}{2}\}, \{E 000\}', \{C_{2z} 00\frac{1}{2}\}', \{\sigma_x 000\}', \{\sigma_y 00\frac{1}{2}\}'$                                                                                 |
| 26.68 | $Pm'c2'_1$     | $\{E 000\}, \{C_{2z} 00\frac{1}{2}\}', \{\sigma_x 000\}', \{\sigma_y 00\frac{1}{2}\}$                                                                                                                                                                      |
| 26.69 | $Pmc'2'_1$     | $\{E 000\}, \{C_{2z} 00\frac{1}{2}\}', \{\sigma_x 000\}, \{\sigma_y 00\frac{1}{2}\}'$                                                                                                                                                                      |
| 26.70 | $Pm'c'2_1$     | $\{E 000\}, \{C_{2z} 00\frac{1}{2}\}, \{\sigma_x 000\}', \{\sigma_y 00\frac{1}{2}\}'$                                                                                                                                                                      |
| 26.71 | $P_a mc2_1$    | $\{E 000\}, \{C_{2z} 00\frac{1}{2}\}, \{\sigma_x 000\}, \{\sigma_y 00\frac{1}{2}\}, \{E 0\frac{1}{2}0\}', \{C_{2z} 0\frac{1}{2}\frac{1}{2}\}', \{\sigma_x 0\frac{1}{2}0\}', \{\sigma_y 0\frac{1}{2}\frac{1}{2}\}'$                                         |
| 26.72 | $P_b mc2_1$    | $\{E 000\}, \{C_{2z} 00\frac{1}{2}\}, \{\sigma_x 000\}, \{\sigma_y 00\frac{1}{2}\}, \{E \frac{1}{2}00\}', \{C_{2z} \frac{1}{2}0\frac{1}{2}\}', \{\sigma_x \frac{1}{2}00\}', \{\sigma_y \frac{1}{2}0\frac{1}{2}\}'$                                         |
| 26.73 | $P_c mc2_1$    | $\{E 000\}, \{C_{2z} 00\frac{1}{2}\}, \{\sigma_x 000\}, \{\sigma_y 00\frac{1}{2}\}, \{E 00\frac{1}{2}\}', \{C_{2z} 000\}', \{\sigma_x 00\frac{1}{2}\}', \{\sigma_y 000\}'$                                                                                 |
| 26.74 | $P_A mc2_1$    | $\{E 000\}, \{C_{2z} 00\frac{1}{2}\}, \{\sigma_x 000\}, \{\sigma_y 00\frac{1}{2}\}, \{E \frac{1}{2}0\frac{1}{2}\}', \{C_{2z} \frac{1}{2}00\}', \{\sigma_x \frac{1}{2}0\frac{1}{2}\}', \{\sigma_y \frac{1}{2}00\}'$                                         |
| 26.75 | $P_B mc2_1$    | $\{E 000\}, \{C_{2z} 00\frac{1}{2}\}, \{\sigma_x 000\}, \{\sigma_y 00\frac{1}{2}\}, \{E 0\frac{1}{2}\frac{1}{2}\}', \{C_{2z} 0\frac{1}{2}0\}', \{\sigma_x 0\frac{1}{2}\frac{1}{2}\}', \{\sigma_y 0\frac{1}{2}0\}'$                                         |
| 26.76 | $P_C mc2_1$    | $\{E 000\}, \{C_{2z} 00\frac{1}{2}\}, \{\sigma_x 000\}, \{\sigma_y 00\frac{1}{2}\}, \{E \frac{1}{2}\frac{1}{2}0\}', \{C_{2z} \frac{1}{2}\frac{1}{2}\frac{1}{2}\}', \{\sigma_x \frac{1}{2}\frac{1}{2}0\}', \{\sigma_y \frac{1}{2}\frac{1}{2}\frac{1}{2}\}'$ |
| 26.77 | $P_I mc2_1$    | $\{E 000\}, \{C_{2z} 00\frac{1}{2}\}, \{\sigma_x 000\}, \{\sigma_y 00\frac{1}{2}\}, \{E \frac{1}{2}\frac{1}{2}\frac{1}{2}\}', \{C_{2z} \frac{1}{2}\frac{1}{2}0\}', \{\sigma_x \frac{1}{2}\frac{1}{2}\frac{1}{2}\}', \{\sigma_y \frac{1}{2}\frac{1}{2}0\}'$ |
| 27.78 | $Pcc2$         | $\{E 000\}, \{C_{2z} 000\}, \{\sigma_x 00\frac{1}{2}\}, \{\sigma_y 00\frac{1}{2}\}$                                                                                                                                                                        |
| 27.79 | $Pcc21'$       | $\{E 000\}, \{C_{2z} 000\}, \{\sigma_x 00\frac{1}{2}\}, \{\sigma_y 00\frac{1}{2}\}, \{E 000\}', \{C_{2z} 000\}', \{\sigma_x 00\frac{1}{2}\}', \{\sigma_y 00\frac{1}{2}\}'$                                                                                 |
| 27.80 | $Pc'c2'$       | $\{E 000\}, \{C_{2z} 000\}', \{\sigma_x 00\frac{1}{2}\}', \{\sigma_y 00\frac{1}{2}\}$                                                                                                                                                                      |
| 27.81 | $Pc'c'2$       | $\{E 000\}, \{C_{2z} 000\}, \{\sigma_x 00\frac{1}{2}\}', \{\sigma_y 00\frac{1}{2}\}'$                                                                                                                                                                      |
| 27.82 | $P_ccc2$       | $\{E 000\}, \{C_{2z} 000\}, \{\sigma_x 00\frac{1}{2}\}, \{\sigma_y 00\frac{1}{2}\}, \{E 00\frac{1}{2}\}', \{C_{2z} 00\frac{1}{2}\}', \{\sigma_x 000\}', \{\sigma_y 000\}'$                                                                                 |

| No.    | Symbol                      | Elements                                                                                                                                                                                                                                                             |
|--------|-----------------------------|----------------------------------------------------------------------------------------------------------------------------------------------------------------------------------------------------------------------------------------------------------------------|
| 27.83  | $P_a cc2$                   | $\{E 000\}, \{C_{2z} 000\}, \{\sigma_x 00\frac{1}{2}\}, \{\sigma_y 00\frac{1}{2}\}, \{E 0\frac{1}{2}0\}', \{C_{2z} 0\frac{1}{2}0\}', \{\sigma_x 0\frac{1}{2}\frac{1}{2}\}', \{\sigma_y 0\frac{1}{2}\frac{1}{2}\}'$                                                   |
| 27.84  | $P_C cc2$                   | $\{E 000\}, \{C_{2z} 000\}, \{\sigma_x 00\frac{1}{2}\}, \{\sigma_y 00\frac{1}{2}\}, \{E \frac{1}{2}\frac{1}{2}0\}', \{C_{2z} \frac{1}{2}\frac{1}{2}0\}', \{\sigma_x \frac{1}{2}\frac{1}{2}\frac{1}{2}\}', \{\sigma_y \frac{1}{2}\frac{1}{2}\frac{1}{2}\}'$           |
| 27.85  | $P_A cc2$                   | $\{E 000\}, \{C_{2z} 000\}, \{\sigma_x 00\frac{1}{2}\}, \{\sigma_y 00\frac{1}{2}\}, \{E \frac{1}{2}0\frac{1}{2}\}', \{C_{2z} \frac{1}{2}0\frac{1}{2}\}', \{\sigma_x \frac{1}{2}00\}', \{\sigma_y \frac{1}{2}00\}'$                                                   |
| 27.86  | $P_I cc2$                   | $\{E 000\}, \{C_{2z} 000\}, \{\sigma_x 00\frac{1}{2}\}, \{\sigma_y 00\frac{1}{2}\}, \{E \frac{1}{2}\frac{1}{2}\frac{1}{2}\}', \{C_{2z} \frac{1}{2}\frac{1}{2}\frac{1}{2}\}', \{\sigma_x \frac{1}{2}\frac{1}{2}0\}', \{\sigma_y \frac{1}{2}\frac{1}{2}0\}'$           |
| 28.87  | $Pma2$ ( $Pbm2$ )           | $\{E 000\}, \{C_{2z} \frac{1}{2}00\}, \{\sigma_x \frac{1}{2}00\}, \{\sigma_y 000\}$                                                                                                                                                                                  |
| 28.88  | $Pma21'$ ( $Pbm21'$ )       | $\{E 000\}, \{C_{2z} \frac{1}{2}00\}, \{\sigma_x \frac{1}{2}00\}, \{\sigma_y 000\}, \{E 000\}', \{C_{2z} \frac{1}{2}00\}', \{\sigma_x \frac{1}{2}00\}', \{\sigma_y 000\}'$                                                                                           |
| 28.89  | $Pm'a2'$ ( $Pbm'2'$ )       | $\{E 000\}, \{C_{2z} \frac{1}{2}00\}', \{\sigma_x \frac{1}{2}00\}, \{\sigma_y 000\}'$                                                                                                                                                                                |
| 28.90  | $Pma'2'$ ( $Pb'm2'$ )       | $\{E 000\}, \{C_{2z} \frac{1}{2}00\}', \{\sigma_x \frac{1}{2}00\}', \{\sigma_y 000\}$                                                                                                                                                                                |
| 28.91  | $Pm'a'2$ ( $Pb'm'2$ )       | $\{E 000\}, \{C_{2z} \frac{1}{2}00\}, \{\sigma_x \frac{1}{2}00\}', \{\sigma_y 000\}'$                                                                                                                                                                                |
| 28.92  | $P_a ma2$ ( $P_b bm2$ )     | $\{E 000\}, \{C_{2z} \frac{1}{2}00\}, \{\sigma_x \frac{1}{2}00\}, \{\sigma_y 000\}, \{E \frac{1}{2}00\}', \{C_{2z} 000\}', \{\sigma_x 000\}', \{\sigma_y \frac{1}{2}00\}'$                                                                                           |
| 28.93  | $P_b ma2$ ( $P_a bm2$ )     | $\{E 000\}, \{C_{2z} \frac{1}{2}00\}, \{\sigma_x \frac{1}{2}00\}, \{\sigma_y 000\}, \{E 0\frac{1}{2}0\}', \{C_{2z} \frac{1}{2}\frac{1}{2}0\}', \{\sigma_x \frac{1}{2}\frac{1}{2}0\}', \{\sigma_y 0\frac{1}{2}0\}'$                                                   |
| 28.94  | $P_c ma2$ ( $P_c bm2$ )     | $\{E 000\}, \{C_{2z} \frac{1}{2}00\}, \{\sigma_x \frac{1}{2}00\}, \{\sigma_y 000\}, \{E 00\frac{1}{2}\}', \{C_{2z} \frac{1}{2}0\frac{1}{2}\}', \{\sigma_x 0\frac{1}{2}\frac{1}{2}\}', \{\sigma_y 00\frac{1}{2}\}'$                                                   |
| 28.95  | $P_A ma2$ ( $P_B bm2$ )     | $\{E 000\}, \{C_{2z} \frac{1}{2}00\}, \{\sigma_x \frac{1}{2}00\}, \{\sigma_y 000\}, \{E 0\frac{1}{2}\frac{1}{2}\}', \{C_{2z} \frac{1}{2}\frac{1}{2}\frac{1}{2}\}', \{\sigma_x \frac{1}{2}\frac{1}{2}\frac{1}{2}\}', \{\sigma_y 0\frac{1}{2}\frac{1}{2}\}'$           |
| 28.96  | $P_B ma2$ ( $P_A bm2$ )     | $\{E 000\}, \{C_{2z} \frac{1}{2}00\}, \{\sigma_x \frac{1}{2}00\}, \{\sigma_y 000\}, \{E \frac{1}{2}0\frac{1}{2}\}', \{C_{2z} 00\frac{1}{2}\}', \{\sigma_x 00\frac{1}{2}\}', \{\sigma_y \frac{1}{2}0\frac{1}{2}\}'$                                                   |
| 28.97  | $P_C ma2$ ( $P_C bm2$ )     | $\{E 000\}, \{C_{2z} \frac{1}{2}00\}, \{\sigma_x \frac{1}{2}00\}, \{\sigma_y 000\}, \{E \frac{1}{2}\frac{1}{2}0\}', \{C_{2z} 0\frac{1}{2}0\}', \{\sigma_x 0\frac{1}{2}0\}', \{\sigma_y \frac{1}{2}\frac{1}{2}0\}'$                                                   |
| 28.98  | $P_I ma2$ ( $P_I bm2$ )     | $\{E 000\}, \{C_{2z} \frac{1}{2}00\}, \{\sigma_x \frac{1}{2}00\}, \{\sigma_y 000\}, \{E \frac{1}{2}\frac{1}{2}\frac{1}{2}\}', \{C_{2z} 0\frac{1}{2}\frac{1}{2}\}', \{\sigma_x 0\frac{1}{2}\frac{1}{2}\}', \{\sigma_y \frac{1}{2}\frac{1}{2}\frac{1}{2}\}'$           |
| 29.99  | $Pca2_1$ ( $Pbc2_1$ )       | $\{E 000\}, \{C_{2z} \frac{1}{2}0\frac{1}{2}\}, \{\sigma_x \frac{1}{2}00\}, \{\sigma_y 00\frac{1}{2}\}$                                                                                                                                                              |
| 29.100 | $Pca2_11'$ ( $Pbc2_11'$ )   | $\{E 000\}, \{C_{2z} \frac{1}{2}0\frac{1}{2}\}, \{\sigma_x \frac{1}{2}00\}, \{\sigma_y 00\frac{1}{2}\}, \{E 000\}', \{C_{2z} \frac{1}{2}0\frac{1}{2}\}', \{\sigma_x \frac{1}{2}00\}', \{\sigma_y 00\frac{1}{2}\}'$                                                   |
| 29.101 | $Pc'a2'_1$ ( $Pbc'2'_1$ )   | $\{E 000\}, \{C_{2z} \frac{1}{2}0\frac{1}{2}\}', \{\sigma_x \frac{1}{2}00\}, \{\sigma_y 00\frac{1}{2}\}'$                                                                                                                                                            |
| 29.102 | $Pca'2'_1$ ( $Pb'c2'_1$ )   | $\{E 000\}, \{C_{2z} \frac{1}{2}0\frac{1}{2}\}', \{\sigma_x \frac{1}{2}00\}', \{\sigma_y 00\frac{1}{2}\}$                                                                                                                                                            |
| 29.103 | $Pc'a'2_1$ ( $Pb'c'2_1$ )   | $\{E 000\}, \{C_{2z} \frac{1}{2}0\frac{1}{2}\}, \{\sigma_x \frac{1}{2}00\}', \{\sigma_y 00\frac{1}{2}\}'$                                                                                                                                                            |
| 29.104 | $P_a ca2_1$ ( $P_b bc2_1$ ) | $\{E 000\}, \{C_{2z} \frac{1}{2}0\frac{1}{2}\}, \{\sigma_x \frac{1}{2}00\}, \{\sigma_y 00\frac{1}{2}\}, \{E \frac{1}{2}00\}', \{C_{2z} 00\frac{1}{2}\}', \{\sigma_x 000\}', \{\sigma_y \frac{1}{2}0\frac{1}{2}\}'$                                                   |
| 29.105 | $P_b ca2_1$ ( $P_a bc2_1$ ) | $\{E 000\}, \{C_{2z} \frac{1}{2}0\frac{1}{2}\}, \{\sigma_x \frac{1}{2}00\}, \{\sigma_y 00\frac{1}{2}\}, \{E 0\frac{1}{2}0\}', \{C_{2z} \frac{1}{2}\frac{1}{2}\frac{1}{2}\}', \{\sigma_x \frac{1}{2}\frac{1}{2}\frac{1}{2}\}', \{\sigma_y 0\frac{1}{2}\frac{1}{2}\}'$ |
| 29.106 | $P_c ca2_1$ ( $P_c bc2_1$ ) | $\{E 000\}, \{C_{2z} \frac{1}{2}0\frac{1}{2}\}, \{\sigma_x \frac{1}{2}00\}, \{\sigma_y 00\frac{1}{2}\}, \{E 00\frac{1}{2}\}', \{C_{2z} \frac{1}{2}00\}', \{\sigma_x \frac{1}{2}0\frac{1}{2}\}', \{\sigma_y 000\}'$                                                   |
| 29.107 | $P_A ca2_1$ ( $P_B bc2_1$ ) | $\{E 000\}, \{C_{2z} \frac{1}{2}0\frac{1}{2}\}, \{\sigma_x \frac{1}{2}00\}, \{\sigma_y 00\frac{1}{2}\}, \{E 0\frac{1}{2}\frac{1}{2}\}', \{C_{2z} \frac{1}{2}\frac{1}{2}0\}', \{\sigma_x \frac{1}{2}\frac{1}{2}\frac{1}{2}\}', \{\sigma_y 0\frac{1}{2}0\}'$           |
| 29.108 | $P_B ca2_1$ ( $P_A bc2_1$ ) | $\{E 000\}, \{C_{2z} \frac{1}{2}0\frac{1}{2}\}, \{\sigma_x \frac{1}{2}00\}, \{\sigma_y 00\frac{1}{2}\}, \{E \frac{1}{2}0\frac{1}{2}\}', \{C_{2z} 000\}', \{\sigma_x 00\frac{1}{2}\}', \{\sigma_y \frac{1}{2}00\}'$                                                   |
| 29.109 | $P_C ca2_1$ ( $P_C bc2_1$ ) | $\{E 000\}, \{C_{2z} \frac{1}{2}0\frac{1}{2}\}, \{\sigma_x \frac{1}{2}00\}, \{\sigma_y 00\frac{1}{2}\}, \{E \frac{1}{2}\frac{1}{2}0\}', \{C_{2z} 0\frac{1}{2}\frac{1}{2}\}', \{\sigma_x 0\frac{1}{2}0\}', \{\sigma_y \frac{1}{2}\frac{1}{2}\frac{1}{2}\}'$           |
| 29.110 | $P_I ca2_1$ ( $P_I bc2_1$ ) | $\{E 000\}, \{C_{2z} \frac{1}{2}0\frac{1}{2}\}, \{\sigma_x \frac{1}{2}00\}, \{\sigma_y 00\frac{1}{2}\}, \{E \frac{1}{2}\frac{1}{2}\frac{1}{2}\}', \{C_{2z} 0\frac{1}{2}0\}', \{\sigma_x 0\frac{1}{2}\frac{1}{2}\}', \{\sigma_y \frac{1}{2}\frac{1}{2}0\}'$           |
| 30.111 | $Pnc2$                      | $\{E 000\}, \{C_{2z} \frac{1}{2}00\}, \{\sigma_x \frac{1}{2}0\frac{1}{2}\}, \{\sigma_y 00\frac{1}{2}\}$                                                                                                                                                              |
| 30.112 | $Pnc21'$                    | $\{E 000\}, \{C_{2z} \frac{1}{2}00\}, \{\sigma_x \frac{1}{2}0\frac{1}{2}\}, \{\sigma_y 00\frac{1}{2}\}, \{E 000\}', \{C_{2z} \frac{1}{2}00\}', \{\sigma_x \frac{1}{2}0\frac{1}{2}\}', \{\sigma_y 00\frac{1}{2}\}'$                                                   |
| 30.113 | $Pn'c2'$                    | $\{E 000\}, \{C_{2z} \frac{1}{2}00\}', \{\sigma_x \frac{1}{2}0\frac{1}{2}\}', \{\sigma_y 00\frac{1}{2}\}$                                                                                                                                                            |
| 30.114 | $Pnc'2'$                    | $\{E 000\}, \{C_{2z} \frac{1}{2}00\}', \{\sigma_x \frac{1}{2}0\frac{1}{2}\}, \{\sigma_y 00\frac{1}{2}\}'$                                                                                                                                                            |
| 30.115 | $Pn'c'2$                    | $\{E 000\}, \{C_{2z} \frac{1}{2}00\}, \{\sigma_x \frac{1}{2}0\frac{1}{2}\}', \{\sigma_y 00\frac{1}{2}\}'$                                                                                                                                                            |
| 30.116 | $P_a nc2$                   | $\{E 000\}, \{C_{2z} \frac{1}{2}00\}, \{\sigma_x \frac{1}{2}0\frac{1}{2}\}, \{\sigma_y 00\frac{1}{2}\}, \{E 0\frac{1}{2}0\}', \{C_{2z} \frac{1}{2}\frac{1}{2}0\}', \{\sigma_x \frac{1}{2}\frac{1}{2}\frac{1}{2}\}', \{\sigma_y 0\frac{1}{2}\frac{1}{2}\}'$           |
| 30.117 | $P_b nc2$                   | $\{E 000\}, \{C_{2z} \frac{1}{2}00\}, \{\sigma_x \frac{1}{2}0\frac{1}{2}\}, \{\sigma_y 00\frac{1}{2}\}, \{E \frac{1}{2}00\}', \{C_{2z} 000\}', \{\sigma_x 00\frac{1}{2}\}', \{\sigma_y \frac{1}{2}0\frac{1}{2}\}'$                                                   |
| 30.118 | $P_c nc2$                   | $\{E 000\}, \{C_{2z} \frac{1}{2}00\}, \{\sigma_x \frac{1}{2}0\frac{1}{2}\}, \{\sigma_y 00\frac{1}{2}\}, \{E 00\frac{1}{2}\}', \{C_{2z} \frac{1}{2}0\frac{1}{2}\}', \{\sigma_x \frac{1}{2}00\}', \{\sigma_y 000\}'$                                                   |

| No.    | Symbol                    | Elements                                                                                                                                                                                                                                                   |
|--------|---------------------------|------------------------------------------------------------------------------------------------------------------------------------------------------------------------------------------------------------------------------------------------------------|
| 30.119 | $P_{Anc}2$                | $\{E 000\}, \{C_{2z} \frac{1}{2}00\}, \{\sigma_x \frac{1}{2}0\frac{1}{2}\}, \{\sigma_y 00\frac{1}{2}\}, \{E \frac{1}{2}0\frac{1}{2}\}', \{C_{2z} 00\frac{1}{2}\}', \{\sigma_x 000\}', \{\sigma_y \frac{1}{2}00\}'$                                         |
| 30.120 | $P_{Bnc}2$                | $\{E 000\}, \{C_{2z} \frac{1}{2}00\}, \{\sigma_x \frac{1}{2}0\frac{1}{2}\}, \{\sigma_y 00\frac{1}{2}\}, \{E 0\frac{1}{2}\frac{1}{2}\}', \{C_{2z} \frac{1}{2}\frac{1}{2}\frac{1}{2}\}', \{\sigma_x \frac{1}{2}\frac{1}{2}0\}', \{\sigma_y 0\frac{1}{2}0\}'$ |
| 30.121 | $P_{Cnc}2$                | $\{E 000\}, \{C_{2z} \frac{1}{2}00\}, \{\sigma_x \frac{1}{2}0\frac{1}{2}\}, \{\sigma_y 00\frac{1}{2}\}, \{E \frac{1}{2}\frac{1}{2}0\}', \{C_{2z} 0\frac{1}{2}0\}', \{\sigma_x 0\frac{1}{2}\frac{1}{2}\}', \{\sigma_y \frac{1}{2}\frac{1}{2}\frac{1}{2}\}'$ |
| 30.122 | $P_{In}c2$                | $\{E 000\}, \{C_{2z} \frac{1}{2}00\}, \{\sigma_x \frac{1}{2}0\frac{1}{2}\}, \{\sigma_y 00\frac{1}{2}\}, \{E \frac{1}{2}\frac{1}{2}\frac{1}{2}\}', \{C_{2z} 0\frac{1}{2}\frac{1}{2}\}', \{\sigma_x 0\frac{1}{2}0\}', \{\sigma_y \frac{1}{2}\frac{1}{2}0\}'$ |
| 31.123 | $Pmn2_1 (Pnm2_1)$         | $\{E 000\}, \{C_{2z} \frac{1}{2}0\frac{1}{2}\}, \{\sigma_x \frac{1}{2}0\frac{1}{2}\}, \{\sigma_y 000\}$                                                                                                                                                    |
| 31.124 | $Pmn2_11' (Pnm2_11')$     | $\{E 000\}, \{C_{2z} \frac{1}{2}0\frac{1}{2}\}, \{\sigma_x \frac{1}{2}0\frac{1}{2}\}, \{\sigma_y 000\}, \{E 000\}', \{C_{2z} \frac{1}{2}0\frac{1}{2}\}', \{\sigma_x \frac{1}{2}0\frac{1}{2}\}', \{\sigma_y 000\}'$                                         |
| 31.125 | $Pm'n2_1' (Pnm'2_1')$     | $\{E 000\}, \{C_{2z} \frac{1}{2}0\frac{1}{2}\}', \{\sigma_x \frac{1}{2}0\frac{1}{2}\}, \{\sigma_y 000\}'$                                                                                                                                                  |
| 31.126 | $Pmn'2_1' (Pn'm2_1')$     | $\{E 000\}, \{C_{2z} \frac{1}{2}0\frac{1}{2}\}', \{\sigma_x \frac{1}{2}0\frac{1}{2}\}', \{\sigma_y 000\}$                                                                                                                                                  |
| 31.127 | $Pm'n'2_1 (Pn'm'2_1)$     | $\{E 000\}, \{C_{2z} \frac{1}{2}0\frac{1}{2}\}, \{\sigma_x \frac{1}{2}0\frac{1}{2}\}', \{\sigma_y 000\}'$                                                                                                                                                  |
| 31.128 | $P_{am}n2_1 (P_{bn}m2_1)$ | $\{E 000\}, \{C_{2z} \frac{1}{2}0\frac{1}{2}\}, \{\sigma_x \frac{1}{2}0\frac{1}{2}\}, \{\sigma_y 000\}, \{E \frac{1}{2}00\}', \{C_{2z} 00\frac{1}{2}\}', \{\sigma_x 00\frac{1}{2}\}', \{\sigma_y \frac{1}{2}00\}'$                                         |
| 31.129 | $P_{bm}n2_1 (P_{an}m2_1)$ | $\{E 000\}, \{C_{2z} \frac{1}{2}0\frac{1}{2}\}, \{\sigma_x \frac{1}{2}0\frac{1}{2}\}, \{\sigma_y 000\}, \{E 0\frac{1}{2}0\}', \{C_{2z} \frac{1}{2}\frac{1}{2}\frac{1}{2}\}', \{\sigma_x \frac{1}{2}\frac{1}{2}\frac{1}{2}\}', \{\sigma_y 0\frac{1}{2}0\}'$ |
| 31.130 | $P_{cm}n2_1 (P_{cn}m2_1)$ | $\{E 000\}, \{C_{2z} \frac{1}{2}0\frac{1}{2}\}, \{\sigma_x \frac{1}{2}0\frac{1}{2}\}, \{\sigma_y 000\}, \{E 00\frac{1}{2}\}', \{C_{2z} \frac{1}{2}00\}', \{\sigma_x \frac{1}{2}00\}', \{\sigma_y 00\frac{1}{2}\}'$                                         |
| 31.131 | $P_{Am}n2_1 (P_{Bn}m2_1)$ | $\{E 000\}, \{C_{2z} \frac{1}{2}0\frac{1}{2}\}, \{\sigma_x \frac{1}{2}0\frac{1}{2}\}, \{\sigma_y 000\}, \{E 0\frac{1}{2}\frac{1}{2}\}', \{C_{2z} \frac{1}{2}\frac{1}{2}0\}', \{\sigma_x \frac{1}{2}\frac{1}{2}0\}', \{\sigma_y 0\frac{1}{2}\frac{1}{2}\}'$ |
| 31.132 | $P_{Bm}n2_1 (P_{An}m2_1)$ | $\{E 000\}, \{C_{2z} \frac{1}{2}0\frac{1}{2}\}, \{\sigma_x \frac{1}{2}0\frac{1}{2}\}, \{\sigma_y 000\}, \{E \frac{1}{2}0\frac{1}{2}\}', \{C_{2z} 000\}', \{\sigma_x 000\}', \{\sigma_y \frac{1}{2}0\frac{1}{2}\}'$                                         |
| 31.133 | $P_{Cm}n2_1 (P_{Cn}m2_1)$ | $\{E 000\}, \{C_{2z} \frac{1}{2}0\frac{1}{2}\}, \{\sigma_x \frac{1}{2}0\frac{1}{2}\}, \{\sigma_y 000\}, \{E \frac{1}{2}\frac{1}{2}0\}', \{C_{2z} 0\frac{1}{2}\frac{1}{2}\}', \{\sigma_x 0\frac{1}{2}\frac{1}{2}\}', \{\sigma_y \frac{1}{2}\frac{1}{2}0\}'$ |
| 31.134 | $P_{Im}n2_1 (P_{In}m2_1)$ | $\{E 000\}, \{C_{2z} \frac{1}{2}0\frac{1}{2}\}, \{\sigma_x \frac{1}{2}0\frac{1}{2}\}, \{\sigma_y 000\}, \{E \frac{1}{2}\frac{1}{2}\frac{1}{2}\}', \{C_{2z} 0\frac{1}{2}0\}', \{\sigma_x 0\frac{1}{2}0\}', \{\sigma_y \frac{1}{2}\frac{1}{2}\frac{1}{2}\}'$ |
| 32.135 | $Pba2$                    | $\{E 000\}, \{C_{2z} \frac{1}{2}\frac{1}{2}0\}, \{\sigma_x \frac{1}{2}00\}, \{\sigma_y 0\frac{1}{2}0\}$                                                                                                                                                    |
| 32.136 | $Pba21'$                  | $\{E 000\}, \{C_{2z} \frac{1}{2}\frac{1}{2}0\}, \{\sigma_x \frac{1}{2}00\}, \{\sigma_y 0\frac{1}{2}0\}, \{E 000\}', \{C_{2z} \frac{1}{2}\frac{1}{2}0\}', \{\sigma_x \frac{1}{2}00\}', \{\sigma_y 0\frac{1}{2}0\}'$                                         |
| 32.137 | $Pb'a2'$                  | $\{E 000\}, \{C_{2z} \frac{1}{2}\frac{1}{2}0\}', \{\sigma_x \frac{1}{2}00\}', \{\sigma_y 0\frac{1}{2}0\}$                                                                                                                                                  |
| 32.138 | $Pb'a'2$                  | $\{E 000\}, \{C_{2z} \frac{1}{2}\frac{1}{2}0\}, \{\sigma_x \frac{1}{2}00\}', \{\sigma_y 0\frac{1}{2}0\}'$                                                                                                                                                  |
| 32.139 | $P_cba2$                  | $\{E 000\}, \{C_{2z} \frac{1}{2}\frac{1}{2}0\}, \{\sigma_x \frac{1}{2}00\}, \{\sigma_y 0\frac{1}{2}0\}, \{E 00\frac{1}{2}\}', \{C_{2z} \frac{1}{2}\frac{1}{2}\frac{1}{2}\}', \{\sigma_x \frac{1}{2}0\frac{1}{2}\}', \{\sigma_y 0\frac{1}{2}\frac{1}{2}\}'$ |
| 32.140 | $P_a ba2$                 | $\{E 000\}, \{C_{2z} \frac{1}{2}\frac{1}{2}0\}, \{\sigma_x \frac{1}{2}00\}, \{\sigma_y 0\frac{1}{2}0\}, \{E 0\frac{1}{2}0\}', \{C_{2z} \frac{1}{2}00\}', \{\sigma_x \frac{1}{2}\frac{1}{2}0\}', \{\sigma_y 000\}'$                                         |
| 32.141 | $P_C ba2$                 | $\{E 000\}, \{C_{2z} \frac{1}{2}\frac{1}{2}0\}, \{\sigma_x \frac{1}{2}00\}, \{\sigma_y 0\frac{1}{2}0\}, \{E \frac{1}{2}\frac{1}{2}0\}', \{C_{2z} 000\}', \{\sigma_x 0\frac{1}{2}0\}', \{\sigma_y \frac{1}{2}00\}'$                                         |
| 32.142 | $P_A ba2$                 | $\{E 000\}, \{C_{2z} \frac{1}{2}\frac{1}{2}0\}, \{\sigma_x \frac{1}{2}00\}, \{\sigma_y 0\frac{1}{2}0\}, \{E \frac{1}{2}0\frac{1}{2}\}', \{C_{2z} 0\frac{1}{2}\frac{1}{2}\}', \{\sigma_x 00\frac{1}{2}\}', \{\sigma_y \frac{1}{2}\frac{1}{2}\frac{1}{2}\}'$ |
| 32.143 | $P_I ba2$                 | $\{E 000\}, \{C_{2z} \frac{1}{2}\frac{1}{2}0\}, \{\sigma_x \frac{1}{2}00\}, \{\sigma_y 0\frac{1}{2}0\}, \{E \frac{1}{2}\frac{1}{2}\frac{1}{2}\}', \{C_{2z} 00\frac{1}{2}\}', \{\sigma_x 0\frac{1}{2}\frac{1}{2}\}', \{\sigma_y \frac{1}{2}0\frac{1}{2}\}'$ |
| 33.144 | $Pna2_1 (Pbn2_1)$         | $\{E 000\}, \{C_{2z} \frac{1}{2}\frac{1}{2}\frac{1}{2}\}, \{\sigma_x \frac{1}{2}00\}, \{\sigma_y 0\frac{1}{2}\frac{1}{2}\}$                                                                                                                                |
| 33.145 | $Pna2_11' (Pbn2_11')$     | $\{E 000\}, \{C_{2z} \frac{1}{2}\frac{1}{2}\frac{1}{2}\}, \{\sigma_x \frac{1}{2}00\}, \{\sigma_y 0\frac{1}{2}\frac{1}{2}\}, \{E 000\}', \{C_{2z} \frac{1}{2}\frac{1}{2}\frac{1}{2}\}', \{\sigma_x \frac{1}{2}00\}', \{\sigma_y 0\frac{1}{2}\frac{1}{2}\}'$ |
| 33.146 | $Pn'a2_1' (Pbn'2_1')$     | $\{E 000\}, \{C_{2z} \frac{1}{2}\frac{1}{2}\frac{1}{2}\}', \{\sigma_x \frac{1}{2}00\}, \{\sigma_y 0\frac{1}{2}\frac{1}{2}\}'$                                                                                                                              |
| 33.147 | $Pna'2_1' (Pb'n2_1')$     | $\{E 000\}, \{C_{2z} \frac{1}{2}\frac{1}{2}\frac{1}{2}\}', \{\sigma_x \frac{1}{2}00\}', \{\sigma_y 0\frac{1}{2}\frac{1}{2}\}$                                                                                                                              |
| 33.148 | $Pn'a'2_1 (Pb'n'2_1)$     | $\{E 000\}, \{C_{2z} \frac{1}{2}\frac{1}{2}\frac{1}{2}\}, \{\sigma_x \frac{1}{2}00\}', \{\sigma_y 0\frac{1}{2}\frac{1}{2}\}'$                                                                                                                              |
| 33.149 | $P_a na2_1 (P_b bn2_1)$   | $\{E 000\}, \{C_{2z} \frac{1}{2}\frac{1}{2}\frac{1}{2}\}, \{\sigma_x \frac{1}{2}00\}, \{\sigma_y 0\frac{1}{2}\frac{1}{2}\}, \{E \frac{1}{2}00\}', \{C_{2z} 0\frac{1}{2}\frac{1}{2}\}', \{\sigma_x 000\}', \{\sigma_y \frac{1}{2}\frac{1}{2}\frac{1}{2}\}'$ |
| 33.150 | $P_b na2_1 (P_a bn2_1)$   | $\{E 000\}, \{C_{2z} \frac{1}{2}\frac{1}{2}\frac{1}{2}\}, \{\sigma_x \frac{1}{2}00\}, \{\sigma_y 0\frac{1}{2}\frac{1}{2}\}, \{E 0\frac{1}{2}0\}', \{C_{2z} \frac{1}{2}0\frac{1}{2}\}', \{\sigma_x \frac{1}{2}\frac{1}{2}0\}', \{\sigma_y 00\frac{1}{2}\}'$ |
| 33.151 | $P_c na2_1 (P_c bn2_1)$   | $\{E 000\}, \{C_{2z} \frac{1}{2}\frac{1}{2}\frac{1}{2}\}, \{\sigma_x \frac{1}{2}00\}, \{\sigma_y 0\frac{1}{2}\frac{1}{2}\}, \{E 00\frac{1}{2}\}', \{C_{2z} \frac{1}{2}\frac{1}{2}0\}', \{\sigma_x \frac{1}{2}0\frac{1}{2}\}', \{\sigma_y 0\frac{1}{2}0\}'$ |
| 33.152 | $P_A na2_1 (P_B bn2_1)$   | $\{E 000\}, \{C_{2z} \frac{1}{2}\frac{1}{2}\frac{1}{2}\}, \{\sigma_x \frac{1}{2}00\}, \{\sigma_y 0\frac{1}{2}\frac{1}{2}\}, \{E 0\frac{1}{2}\frac{1}{2}\}', \{C_{2z} \frac{1}{2}00\}', \{\sigma_x \frac{1}{2}\frac{1}{2}\frac{1}{2}\}', \{\sigma_y 000\}'$ |
| 33.153 | $P_B na2_1 (P_A bn2_1)$   | $\{E 000\}, \{C_{2z} \frac{1}{2}\frac{1}{2}\frac{1}{2}\}, \{\sigma_x \frac{1}{2}00\}, \{\sigma_y 0\frac{1}{2}\frac{1}{2}\}, \{E \frac{1}{2}0\frac{1}{2}\}', \{C_{2z} 0\frac{1}{2}0\}', \{\sigma_x 00\frac{1}{2}\}', \{\sigma_y \frac{1}{2}\frac{1}{2}0\}'$ |
| 33.154 | $P_C na2_1 (P_C bn2_1)$   | $\{E 000\}, \{C_{2z} \frac{1}{2}\frac{1}{2}\frac{1}{2}\}, \{\sigma_x \frac{1}{2}00\}, \{\sigma_y 0\frac{1}{2}\frac{1}{2}\}, \{E \frac{1}{2}\frac{1}{2}0\}', \{C_{2z} 00\frac{1}{2}\}', \{\sigma_x 0\frac{1}{2}0\}', \{\sigma_y \frac{1}{2}0\frac{1}{2}\}'$ |

| No.    | Symbol                      | Elements                                                                                                                                                                                                                                                   |
|--------|-----------------------------|------------------------------------------------------------------------------------------------------------------------------------------------------------------------------------------------------------------------------------------------------------|
| 33.155 | $P_I na2_1$ ( $P_I bn2_1$ ) | $\{E 000\}, \{C_{2z} \frac{1}{2}\frac{1}{2}\frac{1}{2}\}, \{\sigma_x \frac{1}{2}00\}, \{\sigma_y 0\frac{1}{2}\frac{1}{2}\}, \{E \frac{1}{2}\frac{1}{2}\frac{1}{2}\}', \{C_{2z} 000\}', \{\sigma_x 0\frac{1}{2}\frac{1}{2}\}', \{\sigma_y \frac{1}{2}00\}'$ |
| 34.156 | $Pnn2$                      | $\{E 000\}, \{C_{2z} \frac{1}{2}\frac{1}{2}0\}, \{\sigma_x \frac{1}{2}0\frac{1}{2}\}, \{\sigma_y 0\frac{1}{2}\frac{1}{2}\}$                                                                                                                                |
| 34.157 | $Pnn21'$                    | $\{E 000\}, \{C_{2z} \frac{1}{2}\frac{1}{2}0\}, \{\sigma_x \frac{1}{2}0\frac{1}{2}\}, \{\sigma_y 0\frac{1}{2}\frac{1}{2}\}, \{E 000\}', \{C_{2z} \frac{1}{2}\frac{1}{2}0\}', \{\sigma_x \frac{1}{2}0\frac{1}{2}\}', \{\sigma_y 0\frac{1}{2}\frac{1}{2}\}'$ |
| 34.158 | $Pn'n2'$                    | $\{E 000\}, \{C_{2z} \frac{1}{2}\frac{1}{2}0\}', \{\sigma_x \frac{1}{2}0\frac{1}{2}\}', \{\sigma_y 0\frac{1}{2}\frac{1}{2}\}$                                                                                                                              |
| 34.159 | $Pn'n'2$                    | $\{E 000\}, \{C_{2z} \frac{1}{2}\frac{1}{2}0\}, \{\sigma_x \frac{1}{2}0\frac{1}{2}\}', \{\sigma_y 0\frac{1}{2}\frac{1}{2}\}'$                                                                                                                              |
| 34.160 | $P_a nn2$                   | $\{E 000\}, \{C_{2z} \frac{1}{2}\frac{1}{2}0\}, \{\sigma_x \frac{1}{2}0\frac{1}{2}\}, \{\sigma_y 0\frac{1}{2}\frac{1}{2}\}, \{E 0\frac{1}{2}0\}', \{C_{2z} \frac{1}{2}00\}', \{\sigma_x \frac{1}{2}\frac{1}{2}\frac{1}{2}\}', \{\sigma_y 00\frac{1}{2}\}'$ |
| 34.161 | $P_c nn2$                   | $\{E 000\}, \{C_{2z} \frac{1}{2}\frac{1}{2}0\}, \{\sigma_x \frac{1}{2}0\frac{1}{2}\}, \{\sigma_y 0\frac{1}{2}\frac{1}{2}\}, \{E 00\frac{1}{2}\}', \{C_{2z} \frac{1}{2}\frac{1}{2}\frac{1}{2}\}', \{\sigma_x \frac{1}{2}00\}', \{\sigma_y 0\frac{1}{2}0\}'$ |
| 34.162 | $P_A nn2$                   | $\{E 000\}, \{C_{2z} \frac{1}{2}\frac{1}{2}0\}, \{\sigma_x \frac{1}{2}0\frac{1}{2}\}, \{\sigma_y 0\frac{1}{2}\frac{1}{2}\}, \{E \frac{1}{2}0\frac{1}{2}\}', \{C_{2z} 0\frac{1}{2}\frac{1}{2}\}', \{\sigma_x 000\}', \{\sigma_y \frac{1}{2}\frac{1}{2}0\}'$ |
| 34.163 | $P_C nn2$                   | $\{E 000\}, \{C_{2z} \frac{1}{2}\frac{1}{2}0\}, \{\sigma_x \frac{1}{2}0\frac{1}{2}\}, \{\sigma_y 0\frac{1}{2}\frac{1}{2}\}, \{E \frac{1}{2}\frac{1}{2}0\}', \{C_{2z} 000\}', \{\sigma_x 0\frac{1}{2}\frac{1}{2}\}', \{\sigma_y \frac{1}{2}0\frac{1}{2}\}'$ |
| 34.164 | $P_I nn2$                   | $\{E 000\}, \{C_{2z} \frac{1}{2}\frac{1}{2}0\}, \{\sigma_x \frac{1}{2}0\frac{1}{2}\}, \{\sigma_y 0\frac{1}{2}\frac{1}{2}\}, \{E \frac{1}{2}\frac{1}{2}\frac{1}{2}\}', \{C_{2z} 00\frac{1}{2}\}', \{\sigma_x 0\frac{1}{2}0\}', \{\sigma_y \frac{1}{2}00\}'$ |
| 35.165 | $Cmm2$                      | $\{E 000\}, \{C_{2z} 000\}, \{\sigma_x 000\}, \{\sigma_y 000\}$                                                                                                                                                                                            |
| 35.166 | $Cmm21'$                    | $\{E 000\}, \{C_{2z} 000\}, \{\sigma_x 000\}, \{\sigma_y 000\}, \{E 000\}', \{C_{2z} 000\}', \{\sigma_x 000\}', \{\sigma_y 000\}'$                                                                                                                         |
| 35.167 | $Cm'm2'$                    | $\{E 000\}, \{C_{2z} 000\}', \{\sigma_x 000\}', \{\sigma_y 000\}$                                                                                                                                                                                          |
| 35.168 | $Cm'm'2$                    | $\{E 000\}, \{C_{2z} 000\}, \{\sigma_x 000\}', \{\sigma_y 000\}'$                                                                                                                                                                                          |
| 35.169 | $C_c mm2$                   | $\{E 000\}, \{C_{2z} 000\}, \{\sigma_x 000\}, \{\sigma_y 000\}, \{E 00\frac{1}{2}\}', \{C_{2z} 00\frac{1}{2}\}', \{\sigma_x 00\frac{1}{2}\}', \{\sigma_y 00\frac{1}{2}\}'$                                                                                 |
| 35.170 | $C_a mm2$                   | $\{E 000\}, \{C_{2z} 000\}, \{\sigma_x 000\}, \{\sigma_y 000\}, \{E \frac{1}{2}\frac{1}{2}0\}', \{C_{2z} \frac{1}{2}\frac{1}{2}0\}', \{\sigma_x \frac{1}{2}\frac{1}{2}0\}', \{\sigma_y \frac{1}{2}\frac{1}{2}0\}'$                                         |
| 35.171 | $C_A mm2$                   | $\{E 000\}, \{C_{2z} 000\}, \{\sigma_x 000\}, \{\sigma_y 000\}, \{E \frac{1}{2}\frac{1}{2}\frac{1}{2}\}', \{C_{2z} \frac{1}{2}\frac{1}{2}\frac{1}{2}\}', \{\sigma_x \frac{1}{2}\frac{1}{2}\frac{1}{2}\}', \{\sigma_y \frac{1}{2}\frac{1}{2}\frac{1}{2}\}'$ |
| 36.172 | $Cmc2_1$ ( $Ccm2_1$ )       | $\{E 000\}, \{C_{2z} 00\frac{1}{2}\}, \{\sigma_x 00\frac{1}{2}\}, \{\sigma_y 000\}$                                                                                                                                                                        |
| 36.173 | $Cmc2_1'$ ( $Ccm2_1'$ )     | $\{E 000\}, \{C_{2z} 00\frac{1}{2}\}, \{\sigma_x 00\frac{1}{2}\}, \{\sigma_y 000\}, \{E 000\}', \{C_{2z} 00\frac{1}{2}\}', \{\sigma_x 00\frac{1}{2}\}', \{\sigma_y 000\}'$                                                                                 |
| 36.174 | $Cm'c2_1'$ ( $Ccm'2_1'$ )   | $\{E 000\}, \{C_{2z} 00\frac{1}{2}\}', \{\sigma_x 00\frac{1}{2}\}, \{\sigma_y 000\}'$                                                                                                                                                                      |
| 36.175 | $Cm'c'2_1'$ ( $Cc'm'2_1'$ ) | $\{E 000\}, \{C_{2z} 00\frac{1}{2}\}', \{\sigma_x 00\frac{1}{2}\}', \{\sigma_y 000\}$                                                                                                                                                                      |
| 36.176 | $Cm'c'2_1$ ( $Cc'm'2_1$ )   | $\{E 000\}, \{C_{2z} 00\frac{1}{2}\}, \{\sigma_x 00\frac{1}{2}\}', \{\sigma_y 000\}'$                                                                                                                                                                      |
| 36.177 | $C_c mc2_1$ ( $C_c cm2_1$ ) | $\{E 000\}, \{C_{2z} 00\frac{1}{2}\}, \{\sigma_x 00\frac{1}{2}\}, \{\sigma_y 000\}, \{E 00\frac{1}{2}\}', \{C_{2z} 000\}', \{\sigma_x 000\}', \{\sigma_y 00\frac{1}{2}\}'$                                                                                 |
| 36.178 | $C_a mc2_1$ ( $C_a cm2_1$ ) | $\{E 000\}, \{C_{2z} 00\frac{1}{2}\}, \{\sigma_x 00\frac{1}{2}\}, \{\sigma_y 000\}, \{E \frac{1}{2}\frac{1}{2}0\}', \{C_{2z} \frac{1}{2}\frac{1}{2}\frac{1}{2}\}', \{\sigma_x \frac{1}{2}\frac{1}{2}\frac{1}{2}\}', \{\sigma_y \frac{1}{2}\frac{1}{2}0\}'$ |
| 36.179 | $C_A mc2_1$ ( $C_A cm2_1$ ) | $\{E 000\}, \{C_{2z} 00\frac{1}{2}\}, \{\sigma_x 00\frac{1}{2}\}, \{\sigma_y 000\}, \{E \frac{1}{2}\frac{1}{2}\frac{1}{2}\}', \{C_{2z} \frac{1}{2}\frac{1}{2}0\}', \{\sigma_x \frac{1}{2}\frac{1}{2}0\}', \{\sigma_y \frac{1}{2}\frac{1}{2}\frac{1}{2}\}'$ |
| 37.180 | $Ccc2$                      | $\{E 000\}, \{C_{2z} 000\}, \{\sigma_x 00\frac{1}{2}\}, \{\sigma_y 00\frac{1}{2}\}$                                                                                                                                                                        |
| 37.181 | $Ccc21'$                    | $\{E 000\}, \{C_{2z} 000\}, \{\sigma_x 00\frac{1}{2}\}, \{\sigma_y 00\frac{1}{2}\}, \{E 000\}', \{C_{2z} 000\}', \{\sigma_x 00\frac{1}{2}\}', \{\sigma_y 00\frac{1}{2}\}'$                                                                                 |
| 37.182 | $Cc'c2'$                    | $\{E 000\}, \{C_{2z} 000\}', \{\sigma_x 00\frac{1}{2}\}', \{\sigma_y 00\frac{1}{2}\}$                                                                                                                                                                      |
| 37.183 | $Cc'c'2$                    | $\{E 000\}, \{C_{2z} 000\}, \{\sigma_x 00\frac{1}{2}\}', \{\sigma_y 00\frac{1}{2}\}'$                                                                                                                                                                      |
| 37.184 | $C_c cc2$                   | $\{E 000\}, \{C_{2z} 000\}, \{\sigma_x 00\frac{1}{2}\}, \{\sigma_y 00\frac{1}{2}\}, \{E 00\frac{1}{2}\}', \{C_{2z} 00\frac{1}{2}\}', \{\sigma_x 000\}', \{\sigma_y 000\}'$                                                                                 |
| 37.185 | $C_a cc2$                   | $\{E 000\}, \{C_{2z} 000\}, \{\sigma_x 00\frac{1}{2}\}, \{\sigma_y 00\frac{1}{2}\}, \{E \frac{1}{2}\frac{1}{2}0\}', \{C_{2z} \frac{1}{2}\frac{1}{2}0\}', \{\sigma_x \frac{1}{2}\frac{1}{2}\frac{1}{2}\}', \{\sigma_y \frac{1}{2}\frac{1}{2}\frac{1}{2}\}'$ |
| 37.186 | $C_A cc2$                   | $\{E 000\}, \{C_{2z} 000\}, \{\sigma_x 00\frac{1}{2}\}, \{\sigma_y 00\frac{1}{2}\}, \{E \frac{1}{2}\frac{1}{2}\frac{1}{2}\}', \{C_{2z} \frac{1}{2}\frac{1}{2}\frac{1}{2}\}', \{\sigma_x \frac{1}{2}\frac{1}{2}0\}', \{\sigma_y \frac{1}{2}\frac{1}{2}0\}'$ |
| 38.187 | $Amm2$ ( $Cm2m$ )           | $\{E 000\}, \{C_{2y} 000\}, \{\sigma_x 000\}, \{\sigma_z 000\}$                                                                                                                                                                                            |
| 38.188 | $Amm21'$ ( $Cm2m1'$ )       | $\{E 000\}, \{C_{2y} 000\}, \{\sigma_x 000\}, \{\sigma_z 000\}, \{E 000\}', \{C_{2y} 000\}', \{\sigma_x 000\}', \{\sigma_z 000\}'$                                                                                                                         |
| 38.189 | $Am'm2'$ ( $Cm2'm'$ )       | $\{E 000\}, \{C_{2y} 000\}', \{\sigma_x 000\}, \{\sigma_z 000\}'$                                                                                                                                                                                          |
| 38.190 | $Amm'2'$ ( $Cm'2'm$ )       | $\{E 000\}, \{C_{2y} 000\}', \{\sigma_x 000\}', \{\sigma_z 000\}$                                                                                                                                                                                          |

| No.    | Symbol                  | Elements                                                                                                                                                                                                                                                   |
|--------|-------------------------|------------------------------------------------------------------------------------------------------------------------------------------------------------------------------------------------------------------------------------------------------------|
| 38.191 | $Am'm'2$ ( $Cm'2m'$ )   | $\{E 000\}, \{C_{2y} 000\}, \{\sigma_x 000\}', \{\sigma_z 000\}'$                                                                                                                                                                                          |
| 38.192 | $A_a mm2$ ( $C_c m2m$ ) | $\{E 000\}, \{C_{2y} 000\}, \{\sigma_x 000\}, \{\sigma_z 000\}, \{E 00\frac{1}{2}\}', \{C_{2y} 00\frac{1}{2}\}', \{\sigma_x 00\frac{1}{2}\}', \{\sigma_z 00\frac{1}{2}\}'$                                                                                 |
| 38.193 | $A_c mm2$ ( $C_a m2m$ ) | $\{E 000\}, \{C_{2y} 000\}, \{\sigma_x 000\}, \{\sigma_z 000\}, \{E \frac{1}{2}\frac{1}{2}0\}', \{C_{2y} \frac{1}{2}\frac{1}{2}0\}', \{\sigma_x \frac{1}{2}\frac{1}{2}0\}', \{\sigma_z \frac{1}{2}\frac{1}{2}0\}'$                                         |
| 38.194 | $A_C mm2$ ( $C_A m2m$ ) | $\{E 000\}, \{C_{2y} 000\}, \{\sigma_x 000\}, \{\sigma_z 000\}, \{E \frac{1}{2}\frac{1}{2}\frac{1}{2}\}', \{C_{2y} \frac{1}{2}\frac{1}{2}\frac{1}{2}\}', \{\sigma_x \frac{1}{2}\frac{1}{2}\frac{1}{2}\}', \{\sigma_z \frac{1}{2}\frac{1}{2}\frac{1}{2}\}'$ |
| 39.195 | $Abm2$ ( $Cm2a$ )       | $\{E 000\}, \{C_{2y} 000\}, \{\sigma_x \frac{1}{2}\frac{1}{2}0\}, \{\sigma_z \frac{1}{2}\frac{1}{2}0\}$                                                                                                                                                    |
| 39.196 | $Abm21'$ ( $Cm2a1'$ )   | $\{E 000\}, \{C_{2y} 000\}, \{\sigma_x \frac{1}{2}\frac{1}{2}0\}, \{\sigma_z \frac{1}{2}\frac{1}{2}0\}, \{E 000\}', \{C_{2y} 000\}', \{\sigma_x \frac{1}{2}\frac{1}{2}0\}', \{\sigma_z \frac{1}{2}\frac{1}{2}0\}'$                                         |
| 39.197 | $Ab'm2'$ ( $Cm'2a'$ )   | $\{E 000\}, \{C_{2y} 000\}', \{\sigma_x \frac{1}{2}\frac{1}{2}0\}, \{\sigma_z \frac{1}{2}\frac{1}{2}0\}'$                                                                                                                                                  |
| 39.198 | $Abm'2'$ ( $Cm'2'a$ )   | $\{E 000\}, \{C_{2y} 000\}', \{\sigma_x \frac{1}{2}\frac{1}{2}0\}', \{\sigma_z \frac{1}{2}\frac{1}{2}0\}'$                                                                                                                                                 |
| 39.199 | $Ab'm'2$ ( $Cm'2a'$ )   | $\{E 000\}, \{C_{2y} 000\}, \{\sigma_x \frac{1}{2}\frac{1}{2}0\}', \{\sigma_z \frac{1}{2}\frac{1}{2}0\}'$                                                                                                                                                  |
| 39.200 | $A_a bm2$ ( $C_c m2a$ ) | $\{E 000\}, \{C_{2y} 000\}, \{\sigma_x \frac{1}{2}\frac{1}{2}0\}, \{\sigma_z \frac{1}{2}\frac{1}{2}0\}, \{E 00\frac{1}{2}\}', \{C_{2y} 00\frac{1}{2}\}', \{\sigma_x \frac{1}{2}\frac{1}{2}\frac{1}{2}\}', \{\sigma_z \frac{1}{2}\frac{1}{2}\frac{1}{2}\}'$ |
| 39.201 | $A_c bm2$ ( $C_a m2a$ ) | $\{E 000\}, \{C_{2y} 000\}, \{\sigma_x \frac{1}{2}\frac{1}{2}0\}, \{\sigma_z \frac{1}{2}\frac{1}{2}0\}, \{E \frac{1}{2}\frac{1}{2}0\}', \{C_{2y} \frac{1}{2}\frac{1}{2}0\}', \{\sigma_x 000\}', \{\sigma_z 000\}'$                                         |
| 39.202 | $A_C bm2$ ( $C_A m2a$ ) | $\{E 000\}, \{C_{2y} 000\}, \{\sigma_x \frac{1}{2}\frac{1}{2}0\}, \{\sigma_z \frac{1}{2}\frac{1}{2}0\}, \{E \frac{1}{2}\frac{1}{2}\frac{1}{2}\}', \{C_{2y} \frac{1}{2}\frac{1}{2}\frac{1}{2}\}', \{\sigma_x 00\frac{1}{2}\}', \{\sigma_z 00\frac{1}{2}\}'$ |
| 40.203 | $Ama2$ ( $Cc2m$ )       | $\{E 000\}, \{C_{2y} 000\}, \{\sigma_x 00\frac{1}{2}\}, \{\sigma_z 00\frac{1}{2}\}$                                                                                                                                                                        |
| 40.204 | $Ama21'$ ( $Cc2m1'$ )   | $\{E 000\}, \{C_{2y} 000\}, \{\sigma_x 00\frac{1}{2}\}, \{\sigma_z 00\frac{1}{2}\}, \{E 000\}', \{C_{2y} 000\}', \{\sigma_x 00\frac{1}{2}\}', \{\sigma_z 00\frac{1}{2}\}'$                                                                                 |
| 40.205 | $Am'a2'$ ( $Cc2'm'$ )   | $\{E 000\}, \{C_{2y} 000\}', \{\sigma_x 00\frac{1}{2}\}, \{\sigma_z 00\frac{1}{2}\}'$                                                                                                                                                                      |
| 40.206 | $Ama'2'$ ( $Cc'2'm$ )   | $\{E 000\}, \{C_{2y} 000\}', \{\sigma_x 00\frac{1}{2}\}', \{\sigma_z 00\frac{1}{2}\}'$                                                                                                                                                                     |
| 40.207 | $Am'a'2$ ( $Cc'2m'$ )   | $\{E 000\}, \{C_{2y} 000\}, \{\sigma_x 00\frac{1}{2}\}', \{\sigma_z 00\frac{1}{2}\}'$                                                                                                                                                                      |
| 40.208 | $A_a ma2$ ( $C_c c2m$ ) | $\{E 000\}, \{C_{2y} 000\}, \{\sigma_x 00\frac{1}{2}\}, \{\sigma_z 00\frac{1}{2}\}, \{E 00\frac{1}{2}\}', \{C_{2y} 00\frac{1}{2}\}', \{\sigma_x 000\}', \{\sigma_z 000\}'$                                                                                 |
| 40.209 | $A_c ma2$ ( $C_a c2m$ ) | $\{E 000\}, \{C_{2y} 000\}, \{\sigma_x 00\frac{1}{2}\}, \{\sigma_z 00\frac{1}{2}\}, \{E \frac{1}{2}\frac{1}{2}0\}', \{C_{2y} \frac{1}{2}\frac{1}{2}0\}', \{\sigma_x \frac{1}{2}\frac{1}{2}\frac{1}{2}\}', \{\sigma_z \frac{1}{2}\frac{1}{2}\frac{1}{2}\}'$ |
| 40.210 | $A_C ma2$ ( $C_A c2m$ ) | $\{E 000\}, \{C_{2y} 000\}, \{\sigma_x 00\frac{1}{2}\}, \{\sigma_z 00\frac{1}{2}\}, \{E \frac{1}{2}\frac{1}{2}\frac{1}{2}\}', \{C_{2y} \frac{1}{2}\frac{1}{2}\frac{1}{2}\}', \{\sigma_x \frac{1}{2}\frac{1}{2}0\}', \{\sigma_z \frac{1}{2}\frac{1}{2}0\}'$ |
| 41.211 | $Aba2$ ( $Cc2a$ )       | $\{E 000\}, \{C_{2y} 000\}, \{\sigma_x \frac{1}{2}\frac{1}{2}\frac{1}{2}\}, \{\sigma_z \frac{1}{2}\frac{1}{2}\frac{1}{2}\}$                                                                                                                                |
| 41.212 | $Aba21'$ ( $Cc2a1'$ )   | $\{E 000\}, \{C_{2y} 000\}, \{\sigma_x \frac{1}{2}\frac{1}{2}\frac{1}{2}\}, \{\sigma_z \frac{1}{2}\frac{1}{2}\frac{1}{2}\}, \{E 000\}', \{C_{2y} 000\}', \{\sigma_x \frac{1}{2}\frac{1}{2}\frac{1}{2}\}', \{\sigma_z \frac{1}{2}\frac{1}{2}\frac{1}{2}\}'$ |
| 41.213 | $Ab'a2'$ ( $Cc2'a'$ )   | $\{E 000\}, \{C_{2y} 000\}', \{\sigma_x \frac{1}{2}\frac{1}{2}\frac{1}{2}\}, \{\sigma_z \frac{1}{2}\frac{1}{2}\frac{1}{2}\}'$                                                                                                                              |
| 41.214 | $Aba'2'$ ( $Cc'2'a$ )   | $\{E 000\}, \{C_{2y} 000\}', \{\sigma_x \frac{1}{2}\frac{1}{2}\frac{1}{2}\}', \{\sigma_z \frac{1}{2}\frac{1}{2}\frac{1}{2}\}'$                                                                                                                             |
| 41.215 | $Ab'a'2$ ( $Cc'2a'$ )   | $\{E 000\}, \{C_{2y} 000\}, \{\sigma_x \frac{1}{2}\frac{1}{2}\frac{1}{2}\}', \{\sigma_z \frac{1}{2}\frac{1}{2}\frac{1}{2}\}'$                                                                                                                              |
| 41.216 | $A_a ba2$ ( $C_c c2a$ ) | $\{E 000\}, \{C_{2y} 000\}, \{\sigma_x \frac{1}{2}\frac{1}{2}\frac{1}{2}\}, \{\sigma_z \frac{1}{2}\frac{1}{2}\frac{1}{2}\}, \{E 00\frac{1}{2}\}', \{C_{2y} 00\frac{1}{2}\}', \{\sigma_x \frac{1}{2}\frac{1}{2}0\}', \{\sigma_z \frac{1}{2}\frac{1}{2}0\}'$ |
| 41.217 | $A_c ba2$ ( $C_a c2a$ ) | $\{E 000\}, \{C_{2y} 000\}, \{\sigma_x \frac{1}{2}\frac{1}{2}\frac{1}{2}\}, \{\sigma_z \frac{1}{2}\frac{1}{2}\frac{1}{2}\}, \{E \frac{1}{2}\frac{1}{2}0\}', \{C_{2y} \frac{1}{2}\frac{1}{2}0\}', \{\sigma_x 00\frac{1}{2}\}', \{\sigma_z 00\frac{1}{2}\}'$ |
| 41.218 | $A_C ba2$ ( $C_A c2a$ ) | $\{E 000\}, \{C_{2y} 000\}, \{\sigma_x \frac{1}{2}\frac{1}{2}\frac{1}{2}\}, \{\sigma_z \frac{1}{2}\frac{1}{2}\frac{1}{2}\}, \{E \frac{1}{2}\frac{1}{2}\frac{1}{2}\}', \{C_{2y} \frac{1}{2}\frac{1}{2}\frac{1}{2}\}', \{\sigma_x 000\}', \{\sigma_z 000\}'$ |
| 42.219 | $Fmm2$                  | $\{E 000\}, \{C_{2z} 000\}, \{\sigma_x 000\}, \{\sigma_y 000\}$                                                                                                                                                                                            |
| 42.220 | $Fmm21'$                | $\{E 000\}, \{C_{2z} 000\}, \{\sigma_x 000\}, \{\sigma_y 000\}, \{E 000\}', \{C_{2z} 000\}', \{\sigma_x 000\}', \{\sigma_y 000\}'$                                                                                                                         |
| 42.221 | $Fm'm2'$                | $\{E 000\}, \{C_{2z} 000\}', \{\sigma_x 000\}', \{\sigma_y 000\}$                                                                                                                                                                                          |
| 42.222 | $Fm'm'2$                | $\{E 000\}, \{C_{2z} 000\}, \{\sigma_x 000\}', \{\sigma_y 000\}'$                                                                                                                                                                                          |
| 42.223 | $F_s mm2$               | $\{E 000\}, \{C_{2z} 000\}, \{\sigma_x 000\}, \{\sigma_y 000\}, \{E \frac{1}{2}\frac{1}{2}\frac{1}{2}\}', \{C_{2z} \frac{1}{2}\frac{1}{2}\frac{1}{2}\}', \{\sigma_x \frac{1}{2}\frac{1}{2}\frac{1}{2}\}', \{\sigma_y \frac{1}{2}\frac{1}{2}\frac{1}{2}\}'$ |
| 43.224 | $Fdd2$                  | $\{E 000\}, \{C_{2z} 00\frac{1}{2}\}, \{\sigma_x 0\frac{1}{2}0\}, \{\sigma_y \frac{1}{2}00\}$                                                                                                                                                              |
| 43.225 | $Fdd21'$                | $\{E 000\}, \{C_{2z} 00\frac{1}{2}\}, \{\sigma_x 0\frac{1}{2}0\}, \{\sigma_y \frac{1}{2}00\}, \{E 000\}', \{C_{2z} 00\frac{1}{2}\}', \{\sigma_x 0\frac{1}{2}0\}', \{\sigma_y \frac{1}{2}00\}'$                                                             |
| 43.226 | $Fd'd2'$                | $\{E 000\}, \{C_{2z} 00\frac{1}{2}\}', \{\sigma_x 0\frac{1}{2}0\}', \{\sigma_y \frac{1}{2}00\}$                                                                                                                                                            |



| No.    | Symbol              | Elements                                                                                                                                                                                                                                                                                                                                                                                                                                                                                                         |
|--------|---------------------|------------------------------------------------------------------------------------------------------------------------------------------------------------------------------------------------------------------------------------------------------------------------------------------------------------------------------------------------------------------------------------------------------------------------------------------------------------------------------------------------------------------|
| 43.227 | $Fd'd'2$            | $\{E 000\}, \{C_{2z} 00\frac{1}{2}\}, \{\sigma_x 0\frac{1}{2}0\}', \{\sigma_y \frac{1}{2}00\}'$                                                                                                                                                                                                                                                                                                                                                                                                                  |
| 43.228 | $F_sdd2$            | $\{E 000\}, \{C_{2z} 00\frac{1}{2}\}, \{\sigma_x 0\frac{1}{2}0\}, \{\sigma_y \frac{1}{2}00\}, \{E \frac{1}{2}\frac{1}{2}\frac{1}{2}\}', \{C_{2z} \frac{1}{2}\frac{1}{2}0\}', \{\sigma_x \frac{1}{2}0\frac{1}{2}\}', \{\sigma_y 0\frac{1}{2}\frac{1}{2}\}'$                                                                                                                                                                                                                                                       |
| 44.229 | $Imm2$              | $\{E 000\}, \{C_{2z} 000\}, \{\sigma_x 000\}, \{\sigma_y 000\}$                                                                                                                                                                                                                                                                                                                                                                                                                                                  |
| 44.230 | $Imm21'$            | $\{E 000\}, \{C_{2z} 000\}, \{\sigma_x 000\}, \{\sigma_y 000\}, \{E 000\}', \{C_{2z} 000\}', \{\sigma_x 000\}', \{\sigma_y 000\}'$                                                                                                                                                                                                                                                                                                                                                                               |
| 44.231 | $Im'm2'$            | $\{E 000\}, \{C_{2z} 000\}', \{\sigma_x 000\}', \{\sigma_y 000\}$                                                                                                                                                                                                                                                                                                                                                                                                                                                |
| 44.232 | $Im'm'2$            | $\{E 000\}, \{C_{2z} 000\}, \{\sigma_x 000\}', \{\sigma_y 000\}'$                                                                                                                                                                                                                                                                                                                                                                                                                                                |
| 44.233 | $I_cmm2$            | $\{E 000\}, \{C_{2z} 000\}, \{\sigma_x 000\}, \{\sigma_y 000\}, \{E \frac{1}{2}\frac{1}{2}0\}', \{C_{2z} \frac{1}{2}\frac{1}{2}0\}', \{\sigma_x \frac{1}{2}\frac{1}{2}0\}', \{\sigma_y \frac{1}{2}\frac{1}{2}0\}'$                                                                                                                                                                                                                                                                                               |
| 44.234 | $I_a mm2$           | $\{E 000\}, \{C_{2z} 000\}, \{\sigma_x 000\}, \{\sigma_y 000\}, \{E \frac{1}{2}0\frac{1}{2}\}', \{C_{2z} \frac{1}{2}0\frac{1}{2}\}', \{\sigma_x \frac{1}{2}0\frac{1}{2}\}', \{\sigma_y \frac{1}{2}0\frac{1}{2}\}'$                                                                                                                                                                                                                                                                                               |
| 45.235 | $Iba2$              | $\{E 000\}, \{C_{2z} 000\}, \{\sigma_x \frac{1}{2}\frac{1}{2}0\}, \{\sigma_y \frac{1}{2}\frac{1}{2}0\}$                                                                                                                                                                                                                                                                                                                                                                                                          |
| 45.236 | $Iba21'$            | $\{E 000\}, \{C_{2z} 000\}, \{\sigma_x \frac{1}{2}\frac{1}{2}0\}, \{\sigma_y \frac{1}{2}\frac{1}{2}0\}, \{E 000\}', \{C_{2z} 000\}', \{\sigma_x \frac{1}{2}\frac{1}{2}0\}', \{\sigma_y \frac{1}{2}\frac{1}{2}0\}'$                                                                                                                                                                                                                                                                                               |
| 45.237 | $Ib'a2'$            | $\{E 000\}, \{C_{2z} 000\}', \{\sigma_x \frac{1}{2}\frac{1}{2}0\}', \{\sigma_y \frac{1}{2}\frac{1}{2}0\}$                                                                                                                                                                                                                                                                                                                                                                                                        |
| 45.238 | $Ib'a'2$            | $\{E 000\}, \{C_{2z} 000\}, \{\sigma_x \frac{1}{2}\frac{1}{2}0\}', \{\sigma_y \frac{1}{2}\frac{1}{2}0\}'$                                                                                                                                                                                                                                                                                                                                                                                                        |
| 45.239 | $I_cba2$            | $\{E 000\}, \{C_{2z} 000\}, \{\sigma_x \frac{1}{2}\frac{1}{2}0\}, \{\sigma_y \frac{1}{2}\frac{1}{2}0\}, \{E \frac{1}{2}\frac{1}{2}0\}', \{C_{2z} \frac{1}{2}\frac{1}{2}0\}', \{\sigma_x 000\}', \{\sigma_y 000\}'$                                                                                                                                                                                                                                                                                               |
| 45.240 | $I_a ba2$           | $\{E 000\}, \{C_{2z} 000\}, \{\sigma_x \frac{1}{2}\frac{1}{2}0\}, \{\sigma_y \frac{1}{2}\frac{1}{2}0\}, \{E \frac{1}{2}0\frac{1}{2}\}', \{C_{2z} \frac{1}{2}0\frac{1}{2}\}', \{\sigma_x 0\frac{1}{2}\frac{1}{2}\}', \{\sigma_y 0\frac{1}{2}\frac{1}{2}\}'$                                                                                                                                                                                                                                                       |
| 46.241 | $Ima2 (Ibm2)$       | $\{E 000\}, \{C_{2z} 000\}, \{\sigma_x 0\frac{1}{2}\frac{1}{2}\}, \{\sigma_y 0\frac{1}{2}\frac{1}{2}\}$                                                                                                                                                                                                                                                                                                                                                                                                          |
| 46.242 | $Ima21' (Ibm21')$   | $\{E 000\}, \{C_{2z} 000\}, \{\sigma_x 0\frac{1}{2}\frac{1}{2}\}, \{\sigma_y 0\frac{1}{2}\frac{1}{2}\}, \{E 000\}', \{C_{2z} 000\}', \{\sigma_x 0\frac{1}{2}\frac{1}{2}\}', \{\sigma_y 0\frac{1}{2}\frac{1}{2}\}'$                                                                                                                                                                                                                                                                                               |
| 46.243 | $Im'a2' (Ibm'2')$   | $\{E 000\}, \{C_{2z} 000\}', \{\sigma_x 0\frac{1}{2}\frac{1}{2}\}, \{\sigma_y 0\frac{1}{2}\frac{1}{2}\}'$                                                                                                                                                                                                                                                                                                                                                                                                        |
| 46.244 | $Ima'2' (Ib'm2')$   | $\{E 000\}, \{C_{2z} 000\}', \{\sigma_x 0\frac{1}{2}\frac{1}{2}\}', \{\sigma_y 0\frac{1}{2}\frac{1}{2}\}$                                                                                                                                                                                                                                                                                                                                                                                                        |
| 46.245 | $Im'a'2 (Ib'm'2)$   | $\{E 000\}, \{C_{2z} 000\}, \{\sigma_x 0\frac{1}{2}\frac{1}{2}\}', \{\sigma_y 0\frac{1}{2}\frac{1}{2}\}'$                                                                                                                                                                                                                                                                                                                                                                                                        |
| 46.246 | $I_cma2 (I_cbm2)$   | $\{E 000\}, \{C_{2z} 000\}, \{\sigma_x 0\frac{1}{2}\frac{1}{2}\}, \{\sigma_y 0\frac{1}{2}\frac{1}{2}\}, \{E \frac{1}{2}\frac{1}{2}0\}', \{C_{2z} \frac{1}{2}\frac{1}{2}0\}', \{\sigma_x \frac{1}{2}0\frac{1}{2}\}', \{\sigma_y \frac{1}{2}0\frac{1}{2}\}'$                                                                                                                                                                                                                                                       |
| 46.247 | $I_a ma2 (I_bbm2)$  | $\{E 000\}, \{C_{2z} 000\}, \{\sigma_x 0\frac{1}{2}\frac{1}{2}\}, \{\sigma_y 0\frac{1}{2}\frac{1}{2}\}, \{E 0\frac{1}{2}\frac{1}{2}\}', \{C_{2z} 0\frac{1}{2}\frac{1}{2}\}', \{\sigma_x 000\}', \{\sigma_y 000\}'$                                                                                                                                                                                                                                                                                               |
| 46.248 | $I_b ma2 (I_a bm2)$ | $\{E 000\}, \{C_{2z} 000\}, \{\sigma_x 0\frac{1}{2}\frac{1}{2}\}, \{\sigma_y 0\frac{1}{2}\frac{1}{2}\}, \{E \frac{1}{2}0\frac{1}{2}\}', \{C_{2z} \frac{1}{2}0\frac{1}{2}\}', \{\sigma_x \frac{1}{2}\frac{1}{2}0\}', \{\sigma_y \frac{1}{2}\frac{1}{2}0\}'$                                                                                                                                                                                                                                                       |
| 47.249 | $Pmmm$              | $\{E 000\}, \{C_{2x} 000\}, \{C_{2y} 000\}, \{C_{2z} 000\}, \{I 000\}, \{\sigma_x 000\}, \{\sigma_y 000\}, \{\sigma_z 000\}$                                                                                                                                                                                                                                                                                                                                                                                     |
| 47.250 | $Pmmm1'$            | $\{E 000\}, \{C_{2x} 000\}, \{C_{2y} 000\}, \{C_{2z} 000\}, \{I 000\}, \{\sigma_x 000\}, \{\sigma_y 000\}, \{\sigma_z 000\}, \{E 000\}', \{C_{2x} 000\}', \{C_{2y} 000\}', \{C_{2z} 000\}', \{I 000\}', \{\sigma_x 000\}', \{\sigma_y 000\}', \{\sigma_z 000\}'$                                                                                                                                                                                                                                                 |
| 47.251 | $Pm'mm$             | $\{E 000\}, \{C_{2x} 000\}, \{C_{2y} 000\}', \{C_{2z} 000\}', \{I 000\}', \{\sigma_x 000\}', \{\sigma_y 000\}, \{\sigma_z 000\}$                                                                                                                                                                                                                                                                                                                                                                                 |
| 47.252 | $Pm'm'm$            | $\{E 000\}, \{C_{2x} 000\}', \{C_{2y} 000\}', \{C_{2z} 000\}, \{I 000\}, \{\sigma_x 000\}', \{\sigma_y 000\}', \{\sigma_z 000\}$                                                                                                                                                                                                                                                                                                                                                                                 |
| 47.253 | $Pm'm'm'$           | $\{E 000\}, \{C_{2x} 000\}, \{C_{2y} 000\}, \{C_{2z} 000\}, \{I 000\}', \{\sigma_x 000\}', \{\sigma_y 000\}', \{\sigma_z 000\}'$                                                                                                                                                                                                                                                                                                                                                                                 |
| 47.254 | $P_a mmm$           | $\{E 000\}, \{C_{2x} 000\}, \{C_{2y} 000\}, \{C_{2z} 000\}, \{I 000\}, \{\sigma_x 000\}, \{\sigma_y 000\}, \{\sigma_z 000\}, \{E 0\frac{1}{2}0\}', \{C_{2x} 0\frac{1}{2}0\}', \{C_{2y} 0\frac{1}{2}0\}', \{C_{2z} 0\frac{1}{2}0\}', \{I 0\frac{1}{2}0\}', \{\sigma_x 0\frac{1}{2}0\}', \{\sigma_y 0\frac{1}{2}0\}', \{\sigma_z 0\frac{1}{2}0\}'$                                                                                                                                                                 |
| 47.255 | $P_C mmm$           | $\{E 000\}, \{C_{2x} 000\}, \{C_{2y} 000\}, \{C_{2z} 000\}, \{I 000\}, \{\sigma_x 000\}, \{\sigma_y 000\}, \{\sigma_z 000\}, \{E \frac{1}{2}\frac{1}{2}0\}', \{C_{2x} \frac{1}{2}\frac{1}{2}0\}', \{C_{2y} \frac{1}{2}\frac{1}{2}0\}', \{C_{2z} \frac{1}{2}\frac{1}{2}0\}', \{I \frac{1}{2}\frac{1}{2}0\}', \{\sigma_x \frac{1}{2}\frac{1}{2}0\}', \{\sigma_y \frac{1}{2}\frac{1}{2}0\}', \{\sigma_z \frac{1}{2}\frac{1}{2}0\}'$                                                                                 |
| 47.256 | $P_I mmm$           | $\{E 000\}, \{C_{2x} 000\}, \{C_{2y} 000\}, \{C_{2z} 000\}, \{I 000\}, \{\sigma_x 000\}, \{\sigma_y 000\}, \{\sigma_z 000\}, \{E \frac{1}{2}\frac{1}{2}\frac{1}{2}\}', \{C_{2x} \frac{1}{2}\frac{1}{2}\frac{1}{2}\}', \{C_{2y} \frac{1}{2}\frac{1}{2}\frac{1}{2}\}', \{C_{2z} \frac{1}{2}\frac{1}{2}\frac{1}{2}\}', \{I \frac{1}{2}\frac{1}{2}\frac{1}{2}\}', \{\sigma_x \frac{1}{2}\frac{1}{2}\frac{1}{2}\}', \{\sigma_y \frac{1}{2}\frac{1}{2}\frac{1}{2}\}', \{\sigma_z \frac{1}{2}\frac{1}{2}\frac{1}{2}\}'$ |
| 48.257 | $Pnnn$              | $\{E 000\}, \{C_{2x} 000\}, \{C_{2y} 000\}, \{C_{2z} 000\}, \{I \frac{1}{2}\frac{1}{2}\frac{1}{2}\}, \{\sigma_x \frac{1}{2}\frac{1}{2}\frac{1}{2}\}, \{\sigma_y \frac{1}{2}\frac{1}{2}\frac{1}{2}\}, \{\sigma_z \frac{1}{2}\frac{1}{2}\frac{1}{2}\}$                                                                                                                                                                                                                                                             |
| 48.258 | $Pnnn1'$            | $\{E 000\}, \{C_{2x} 000\}, \{C_{2y} 000\}, \{C_{2z} 000\}, \{I \frac{1}{2}\frac{1}{2}\frac{1}{2}\}, \{\sigma_x \frac{1}{2}\frac{1}{2}\frac{1}{2}\}, \{\sigma_y \frac{1}{2}\frac{1}{2}\frac{1}{2}\}, \{\sigma_z \frac{1}{2}\frac{1}{2}\frac{1}{2}\}, \{E 000\}', \{C_{2x} 000\}', \{C_{2y} 000\}', \{C_{2z} 000\}', \{I \frac{1}{2}\frac{1}{2}\frac{1}{2}\}', \{\sigma_x \frac{1}{2}\frac{1}{2}\frac{1}{2}\}', \{\sigma_y \frac{1}{2}\frac{1}{2}\frac{1}{2}\}', \{\sigma_z \frac{1}{2}\frac{1}{2}\frac{1}{2}\}'$ |

[illegible]



| No.    | Symbol              | Elements                                                                                                                                                                                                                                                                                                                                                                                                                                                                                                              |
|--------|---------------------|-----------------------------------------------------------------------------------------------------------------------------------------------------------------------------------------------------------------------------------------------------------------------------------------------------------------------------------------------------------------------------------------------------------------------------------------------------------------------------------------------------------------------|
| 50.286 | $P_{Aban}$          | $\{E 000\}, \{C_{2x} 000\}, \{C_{2y} 000\}, \{C_{2z} 000\}, \{I \frac{1}{2}\frac{1}{2}0\}, \{\sigma_x \frac{1}{2}\frac{1}{2}0\}, \{\sigma_y \frac{1}{2}\frac{1}{2}0\}, \{\sigma_z \frac{1}{2}\frac{1}{2}0\},$<br>$\{E \frac{1}{2}0\frac{1}{2}\}', \{C_{2x} \frac{1}{2}0\frac{1}{2}\}', \{C_{2y} \frac{1}{2}0\frac{1}{2}\}', \{C_{2z} \frac{1}{2}0\frac{1}{2}\}', \{I 0\frac{1}{2}\frac{1}{2}\}', \{\sigma_x 0\frac{1}{2}\frac{1}{2}\}', \{\sigma_y 0\frac{1}{2}\frac{1}{2}\}', \{\sigma_z 0\frac{1}{2}\frac{1}{2}\}'$ |
| 50.287 | $P_{Cban}$          | $\{E 000\}, \{C_{2x} 000\}, \{C_{2y} 000\}, \{C_{2z} 000\}, \{I \frac{1}{2}\frac{1}{2}0\}, \{\sigma_x \frac{1}{2}\frac{1}{2}0\}, \{\sigma_y \frac{1}{2}\frac{1}{2}0\}, \{\sigma_z \frac{1}{2}\frac{1}{2}0\},$<br>$\{E \frac{1}{2}\frac{1}{2}0\}', \{C_{2x} \frac{1}{2}\frac{1}{2}0\}', \{C_{2y} \frac{1}{2}\frac{1}{2}0\}', \{C_{2z} \frac{1}{2}\frac{1}{2}0\}', \{I 000\}', \{\sigma_x 000\}', \{\sigma_y 000\}', \{\sigma_z 000\}'$                                                                                 |
| 50.288 | $P_{Iban}$          | $\{E 000\}, \{C_{2x} 000\}, \{C_{2y} 000\}, \{C_{2z} 000\}, \{I \frac{1}{2}\frac{1}{2}0\}, \{\sigma_x \frac{1}{2}\frac{1}{2}0\}, \{\sigma_y \frac{1}{2}\frac{1}{2}0\}, \{\sigma_z \frac{1}{2}\frac{1}{2}0\},$<br>$\{E \frac{1}{2}\frac{1}{2}\frac{1}{2}\}', \{C_{2x} \frac{1}{2}\frac{1}{2}\frac{1}{2}\}', \{C_{2y} \frac{1}{2}\frac{1}{2}\frac{1}{2}\}', \{C_{2z} \frac{1}{2}\frac{1}{2}\frac{1}{2}\}', \{I 00\frac{1}{2}\}', \{\sigma_x 00\frac{1}{2}\}', \{\sigma_y 00\frac{1}{2}\}', \{\sigma_z 00\frac{1}{2}\}'$ |
| 51.289 | $Pmma (Pcmm)$       | $\{E 000\}, \{C_{2x} 00\frac{1}{2}\}, \{C_{2y} 000\}, \{C_{2z} 00\frac{1}{2}\}, \{I 000\}, \{\sigma_x 00\frac{1}{2}\}, \{\sigma_y 000\}, \{\sigma_z 00\frac{1}{2}\}$                                                                                                                                                                                                                                                                                                                                                  |
| 51.290 | $Pmma1' (Pcmm1')$   | $\{E 000\}, \{C_{2x} 00\frac{1}{2}\}, \{C_{2y} 000\}, \{C_{2z} 00\frac{1}{2}\}, \{I 000\}, \{\sigma_x 00\frac{1}{2}\}, \{\sigma_y 000\}, \{\sigma_z 00\frac{1}{2}\}, \{E 000\}',$<br>$\{C_{2x} 00\frac{1}{2}\}', \{C_{2y} 000\}', \{C_{2z} 00\frac{1}{2}\}', \{I 000\}', \{\sigma_x 00\frac{1}{2}\}', \{\sigma_y 000\}', \{\sigma_z 00\frac{1}{2}\}'$                                                                                                                                                                 |
| 51.291 | $Pm'ma (Pcmm')$     | $\{E 000\}, \{C_{2x} 00\frac{1}{2}\}', \{C_{2y} 000\}', \{C_{2z} 00\frac{1}{2}\}, \{I 000\}', \{\sigma_x 00\frac{1}{2}\}, \{\sigma_y 000\}, \{\sigma_z 00\frac{1}{2}\}'$                                                                                                                                                                                                                                                                                                                                              |
| 51.292 | $Pmm'a (Pcm'm)$     | $\{E 000\}, \{C_{2x} 00\frac{1}{2}\}', \{C_{2y} 000\}, \{C_{2z} 00\frac{1}{2}\}', \{I 000\}', \{\sigma_x 00\frac{1}{2}\}, \{\sigma_y 000\}', \{\sigma_z 00\frac{1}{2}\}$                                                                                                                                                                                                                                                                                                                                              |
| 51.293 | $Pmma' (Pc'mm)$     | $\{E 000\}, \{C_{2x} 00\frac{1}{2}\}, \{C_{2y} 000\}', \{C_{2z} 00\frac{1}{2}\}', \{I 000\}', \{\sigma_x 00\frac{1}{2}\}', \{\sigma_y 000\}, \{\sigma_z 00\frac{1}{2}\}$                                                                                                                                                                                                                                                                                                                                              |
| 51.294 | $Pm'm'a (Pcm'm')$   | $\{E 000\}, \{C_{2x} 00\frac{1}{2}\}, \{C_{2y} 000\}', \{C_{2z} 00\frac{1}{2}\}', \{I 000\}, \{\sigma_x 00\frac{1}{2}\}, \{\sigma_y 000\}', \{\sigma_z 00\frac{1}{2}\}'$                                                                                                                                                                                                                                                                                                                                              |
| 51.295 | $Pmm'a' (Pc'm'm)$   | $\{E 000\}, \{C_{2x} 00\frac{1}{2}\}', \{C_{2y} 000\}', \{C_{2z} 00\frac{1}{2}\}, \{I 000\}, \{\sigma_x 00\frac{1}{2}\}', \{\sigma_y 000\}', \{\sigma_z 00\frac{1}{2}\}$                                                                                                                                                                                                                                                                                                                                              |
| 51.296 | $Pm'ma' (Pc'mm')$   | $\{E 000\}, \{C_{2x} 00\frac{1}{2}\}', \{C_{2y} 000\}, \{C_{2z} 00\frac{1}{2}\}', \{I 000\}, \{\sigma_x 00\frac{1}{2}\}', \{\sigma_y 000\}, \{\sigma_z 00\frac{1}{2}\}'$                                                                                                                                                                                                                                                                                                                                              |
| 51.297 | $Pm'm'a' (Pc'm'm')$ | $\{E 000\}, \{C_{2x} 00\frac{1}{2}\}, \{C_{2y} 000\}, \{C_{2z} 00\frac{1}{2}\}, \{I 000\}', \{\sigma_x 00\frac{1}{2}\}', \{\sigma_y 000\}', \{\sigma_z 00\frac{1}{2}\}'$                                                                                                                                                                                                                                                                                                                                              |
| 51.298 | $P_a mma (P_c cmm)$ | $\{E 000\}, \{C_{2x} 00\frac{1}{2}\}, \{C_{2y} 000\}, \{C_{2z} 00\frac{1}{2}\}, \{I 000\}, \{\sigma_x 00\frac{1}{2}\}, \{\sigma_y 000\}, \{\sigma_z 00\frac{1}{2}\}, \{E 00\frac{1}{2}\}',$<br>$\{C_{2x} 000\}', \{C_{2y} 00\frac{1}{2}\}', \{C_{2z} 000\}', \{I 00\frac{1}{2}\}', \{\sigma_x 000\}', \{\sigma_y 00\frac{1}{2}\}', \{\sigma_z 000\}'$                                                                                                                                                                 |
| 51.299 | $P_b mma (P_b cmm)$ | $\{E 000\}, \{C_{2x} 00\frac{1}{2}\}, \{C_{2y} 000\}, \{C_{2z} 00\frac{1}{2}\}, \{I 000\}, \{\sigma_x 00\frac{1}{2}\}, \{\sigma_y 000\}, \{\sigma_z 00\frac{1}{2}\}, \{E \frac{1}{2}00\}',$<br>$\{C_{2x} \frac{1}{2}0\frac{1}{2}\}', \{C_{2y} \frac{1}{2}00\}', \{C_{2z} \frac{1}{2}0\frac{1}{2}\}', \{I \frac{1}{2}00\}', \{\sigma_x \frac{1}{2}0\frac{1}{2}\}', \{\sigma_y \frac{1}{2}00\}', \{\sigma_z \frac{1}{2}0\frac{1}{2}\}'$                                                                                 |
| 51.300 | $P_c mma (P_a cmm)$ | $\{E 000\}, \{C_{2x} 00\frac{1}{2}\}, \{C_{2y} 000\}, \{C_{2z} 00\frac{1}{2}\}, \{I 000\}, \{\sigma_x 00\frac{1}{2}\}, \{\sigma_y 000\}, \{\sigma_z 00\frac{1}{2}\}, \{E 0\frac{1}{2}0\}',$<br>$\{C_{2x} 0\frac{1}{2}\frac{1}{2}\}', \{C_{2y} 0\frac{1}{2}0\}', \{C_{2z} 0\frac{1}{2}\frac{1}{2}\}', \{I 0\frac{1}{2}0\}', \{\sigma_x 0\frac{1}{2}\frac{1}{2}\}', \{\sigma_y 0\frac{1}{2}0\}', \{\sigma_z 0\frac{1}{2}\frac{1}{2}\}'$                                                                                 |
| 51.301 | $P_A mma (P_C cmm)$ | $\{E 000\}, \{C_{2x} 00\frac{1}{2}\}, \{C_{2y} 000\}, \{C_{2z} 00\frac{1}{2}\}, \{I 000\}, \{\sigma_x 00\frac{1}{2}\}, \{\sigma_y 000\}, \{\sigma_z 00\frac{1}{2}\}, \{E \frac{1}{2}\frac{1}{2}0\}',$<br>$\{C_{2x} \frac{1}{2}\frac{1}{2}\frac{1}{2}\}', \{C_{2y} \frac{1}{2}\frac{1}{2}0\}', \{C_{2z} \frac{1}{2}\frac{1}{2}\frac{1}{2}\}', \{I \frac{1}{2}\frac{1}{2}0\}', \{\sigma_x \frac{1}{2}\frac{1}{2}\frac{1}{2}\}', \{\sigma_y \frac{1}{2}\frac{1}{2}0\}', \{\sigma_z \frac{1}{2}\frac{1}{2}\frac{1}{2}\}'$ |
| 51.302 | $P_B mma (P_B cmm)$ | $\{E 000\}, \{C_{2x} 00\frac{1}{2}\}, \{C_{2y} 000\}, \{C_{2z} 00\frac{1}{2}\}, \{I 000\}, \{\sigma_x 00\frac{1}{2}\}, \{\sigma_y 000\}, \{\sigma_z 00\frac{1}{2}\}, \{E 0\frac{1}{2}\frac{1}{2}\}',$<br>$\{C_{2x} 0\frac{1}{2}0\}', \{C_{2y} 0\frac{1}{2}\frac{1}{2}\}', \{C_{2z} 0\frac{1}{2}0\}', \{I 0\frac{1}{2}\frac{1}{2}\}', \{\sigma_x 0\frac{1}{2}0\}', \{\sigma_y 0\frac{1}{2}\frac{1}{2}\}', \{\sigma_z 0\frac{1}{2}0\}'$                                                                                 |
| 51.303 | $P_C mma (P_A cmm)$ | $\{E 000\}, \{C_{2x} 00\frac{1}{2}\}, \{C_{2y} 000\}, \{C_{2z} 00\frac{1}{2}\}, \{I 000\}, \{\sigma_x 00\frac{1}{2}\}, \{\sigma_y 000\}, \{\sigma_z 00\frac{1}{2}\}, \{E \frac{1}{2}0\frac{1}{2}\}',$<br>$\{C_{2x} \frac{1}{$                                                                                                                                                                                                                                                                                         |

[illegible]

| No.    | Symbol                | Elements                                                                                                                                                                                                                                                                                                                                                                                                                                                                                                         |
|--------|-----------------------|------------------------------------------------------------------------------------------------------------------------------------------------------------------------------------------------------------------------------------------------------------------------------------------------------------------------------------------------------------------------------------------------------------------------------------------------------------------------------------------------------------------|
| 54.338 | $Pcca1' (Pcaa1')$     | $\{E 000\}, \{C_{2x} 00\frac{1}{2}\}, \{C_{2y} 000\}, \{C_{2z} 00\frac{1}{2}\}, \{I 0\frac{1}{2}0\}, \{\sigma_x 0\frac{1}{2}\frac{1}{2}\}, \{\sigma_y 0\frac{1}{2}0\}, \{\sigma_z 0\frac{1}{2}\frac{1}{2}\}, \{E 000\}', \{C_{2x} 00\frac{1}{2}\}', \{C_{2y} 000\}', \{C_{2z} 00\frac{1}{2}\}', \{I 0\frac{1}{2}0\}', \{\sigma_x 0\frac{1}{2}\frac{1}{2}\}', \{\sigma_y 0\frac{1}{2}0\}', \{\sigma_z 0\frac{1}{2}\frac{1}{2}\}'$                                                                                 |
| 54.339 | $Pc'ca (Pcaa')$       | $\{E 000\}, \{C_{2x} 00\frac{1}{2}\}', \{C_{2y} 000\}', \{C_{2z} 00\frac{1}{2}\}, \{I 0\frac{1}{2}0\}', \{\sigma_x 0\frac{1}{2}\frac{1}{2}\}, \{\sigma_y 0\frac{1}{2}0\}, \{\sigma_z 0\frac{1}{2}\frac{1}{2}\}'$                                                                                                                                                                                                                                                                                                 |
| 54.340 | $Pcc'a (Pca'a)$       | $\{E 000\}, \{C_{2x} 00\frac{1}{2}\}', \{C_{2y} 000\}, \{C_{2z} 00\frac{1}{2}\}', \{I 0\frac{1}{2}0\}', \{\sigma_x 0\frac{1}{2}\frac{1}{2}\}, \{\sigma_y 0\frac{1}{2}0\}', \{\sigma_z 0\frac{1}{2}\frac{1}{2}\}$                                                                                                                                                                                                                                                                                                 |
| 54.341 | $Pcca' (Pc'aa)$       | $\{E 000\}, \{C_{2x} 00\frac{1}{2}\}, \{C_{2y} 000\}', \{C_{2z} 00\frac{1}{2}\}', \{I 0\frac{1}{2}0\}', \{\sigma_x 0\frac{1}{2}\frac{1}{2}\}', \{\sigma_y 0\frac{1}{2}0\}, \{\sigma_z 0\frac{1}{2}\frac{1}{2}\}$                                                                                                                                                                                                                                                                                                 |
| 54.342 | $Pc'c'a (Pca'a')$     | $\{E 000\}, \{C_{2x} 00\frac{1}{2}\}, \{C_{2y} 000\}', \{C_{2z} 00\frac{1}{2}\}', \{I 0\frac{1}{2}0\}, \{\sigma_x 0\frac{1}{2}\frac{1}{2}\}, \{\sigma_y 0\frac{1}{2}0\}', \{\sigma_z 0\frac{1}{2}\frac{1}{2}\}'$                                                                                                                                                                                                                                                                                                 |
| 54.343 | $Pcc'a' (Pc'a'a)$     | $\{E 000\}, \{C_{2x} 00\frac{1}{2}\}', \{C_{2y} 000\}', \{C_{2z} 00\frac{1}{2}\}, \{I 0\frac{1}{2}0\}, \{\sigma_x 0\frac{1}{2}\frac{1}{2}\}', \{\sigma_y 0\frac{1}{2}0\}', \{\sigma_z 0\frac{1}{2}\frac{1}{2}\}$                                                                                                                                                                                                                                                                                                 |
| 54.344 | $Pc'ca' (Pc'aa')$     | $\{E 000\}, \{C_{2x} 00\frac{1}{2}\}', \{C_{2y} 000\}, \{C_{2z} 00\frac{1}{2}\}', \{I 0\frac{1}{2}0\}, \{\sigma_x 0\frac{1}{2}\frac{1}{2}\}', \{\sigma_y 0\frac{1}{2}0\}, \{\sigma_z 0\frac{1}{2}\frac{1}{2}\}'$                                                                                                                                                                                                                                                                                                 |
| 54.345 | $Pc'c'a' (Pc'a'a')$   | $\{E 000\}, \{C_{2x} 00\frac{1}{2}\}, \{C_{2y} 000\}, \{C_{2z} 00\frac{1}{2}\}, \{I 0\frac{1}{2}0\}', \{\sigma_x 0\frac{1}{2}\frac{1}{2}\}', \{\sigma_y 0\frac{1}{2}0\}', \{\sigma_z 0\frac{1}{2}\frac{1}{2}\}'$                                                                                                                                                                                                                                                                                                 |
| 54.346 | $Pa_{cca} (P_{ccaa})$ | $\{E 000\}, \{C_{2x} 00\frac{1}{2}\}, \{C_{2y} 000\}, \{C_{2z} 00\frac{1}{2}\}, \{I 0\frac{1}{2}0\}, \{\sigma_x 0\frac{1}{2}\frac{1}{2}\}, \{\sigma_y 0\frac{1}{2}0\}, \{\sigma_z 0\frac{1}{2}\frac{1}{2}\}, \{E 00\frac{1}{2}\}', \{C_{2x} 000\}', \{C_{2y} 00\frac{1}{2}\}', \{C_{2z} 000\}', \{I 0\frac{1}{2}\frac{1}{2}\}', \{\sigma_x 0\frac{1}{2}0\}', \{\sigma_y 0\frac{1}{2}\frac{1}{2}\}', \{\sigma_z 0\frac{1}{2}0\}'$                                                                                 |
| 54.347 | $P_bcca (P_bcaa)$     | $\{E 000\}, \{C_{2x} 00\frac{1}{2}\}, \{C_{2y} 000\}, \{C_{2z} 00\frac{1}{2}\}, \{I 0\frac{1}{2}0\}, \{\sigma_x 0\frac{1}{2}\frac{1}{2}\}, \{\sigma_y 0\frac{1}{2}0\}, \{\sigma_z 0\frac{1}{2}\frac{1}{2}\}, \{E \frac{1}{2}00\}', \{C_{2x} \frac{1}{2}0\frac{1}{2}\}', \{C_{2y} \frac{1}{2}00\}', \{C_{2z} \frac{1}{2}0\frac{1}{2}\}', \{I \frac{1}{2}\frac{1}{2}0\}', \{\sigma_x \frac{1}{2}\frac{1}{2}\frac{1}{2}\}', \{\sigma_y \frac{1}{2}\frac{1}{2}0\}', \{\sigma_z \frac{1}{2}\frac{1}{2}\frac{1}{2}\}'$ |
| 54.348 | $P_{ccca} (P_{acaa})$ | $\{E 000\}, \{C_{2x} 00\frac{1}{2}\}, \{C_{2y} 000\}, \{C_{2z} 00\frac{1}{2}\}, \{I 0\frac{1}{2}0\}, \{\sigma_x 0\frac{1}{2}\frac{1}{2}\}, \{\sigma_y 0\frac{1}{2}0\}, \{\sigma_z 0\frac{1}{2}\frac{1}{2}\}, \{E 0\frac{1}{2}0\}', \{C_{2x} 0\frac{1}{2}\frac{1}{2}\}', \{C_{2y} 0\frac{1}{2}0\}', \{C_{2z} 0\frac{1}{2}\frac{1}{2}\}', \{I 000\}', \{\sigma_x 00\frac{1}{2}\}', \{\sigma_y 000\}', \{\sigma_z 00\frac{1}{2}\}'$                                                                                 |
| 54.349 | $PA_{cca} (P_{Ccaa})$ | $\{E 000\}, \{C_{2x} 00\frac{1}{2}\}, \{C_{2y} 000\}, \{C_{2z} 00\frac{1}{2}\}, \{I 0\frac{1}{2}0\}, \{\sigma_x 0\frac{1}{2}\frac{1}{2}\}, \{\sigma_y 0\frac{1}{2}0\}, \{\sigma_z 0\frac{1}{2}\frac{1}{2}\}, \{E \frac{1}{2}\frac{1}{2}0\}', \{C_{2x} \frac{1}{2}\frac{1}{2}\frac{1}{2}\}', \{C_{2y} \frac{1}{2}\frac{1}{2}0\}', \{C_{2z} \frac{1}{2}\frac{1}{2}\frac{1}{2}\}', \{I \frac{1}{2}00\}', \{\sigma_x \frac{1}{2}0\frac{1}{2}\}', \{\sigma_y \frac{1}{2}00\}', \{\sigma_z \frac{1}{2}0\frac{1}{2}\}'$ |
| 54.350 | $P_Bcca (P_Bcaa)$     | $\{E 000\}, \{C_{2x} 00\frac{1}{2}\}, \{C_{2y} 000\}, \{C_{2z} 00\frac{1}{2}\}, \{I 0\frac{1}{2}0\}, \{\sigma_x 0\frac{1}{2}\frac{1}{2}\}, \{\sigma_y 0\frac{1}{2}0\}, \{\sigma_z 0\frac{1}{2}\frac{1}{2}\}, \{E 0\frac{1}{2}\frac{1}{2}\}', \{C_{2x} 0\frac{1}{2}0\}', \{C_{2y} 0\frac{1}{2}\frac{1}{2}\}', \{C_{2z} 0\frac{1}{2}0\}', \{I 00\frac{1}{2}\}', \{\sigma_x 000\}', \{\sigma_y 00\frac{1}{2}\}', \{\sigma_z 000\}'$                                                                                 |
| 54.351 | $P_Ccca (P_Acaa)$     | $\{E 000\}, \{C_{2x} 00\frac{1}{2}\}, \{C_{2y} 000\}, \{C_{2z} 00\frac{1}{2}\}, \{I 0\frac{1}{2}0\}, \{\sigma_x 0\frac{1}{2}\frac{1}{2}\}, \{\sigma_y 0\frac{1}{2}0\}, \{\sigma_z 0\frac{1}{2}\frac{1}{2}\}, \{E \frac{1}{2}0\frac{1}{2}\}', \{C_{2x} \frac{1}{2}00\}', \{C_{2y} \frac{1}{2}0\frac{1}{2}\}', \{C_{2z} \frac{1}{2}00\}', \{I \frac{1}{2}\frac{1}{2}\frac{1}{2}\}', \{\sigma_x \frac{1}{2}\frac{1}{2}0\}', \{\sigma_y \frac{1}{2}\frac{1}{2}\frac{1}{2}\}', \{\sigma_z \frac{1}{2}\frac{1}{2}0\}'$ |
| 54.352 | $P_{Icca} (P_{Icaa})$ | $\{E 000\}, \{C_{2x} 00\frac{1}{2}\}, \{C_{2y} 000\}, \{C_{2z} 00\frac{1}{2}\}, \{I 0\frac{1}{2}0\}, \{\sigma_x 0\frac{1}{2}\frac{1}{2}\}, \{\sigma_y 0\frac{1}{2}0\}, \{\sigma_z 0\frac{1}{2}\frac{1}{2}\}, \{E \frac{1}{2}\frac{1}{2}\frac{1}{2}\}', \{C_{2x} \frac{1}{2}\frac{1}{2}0\}', \{C_{2y} \frac{1}{2}\frac{1}{2}\frac{1}{2}\}', \{C_{2z} \frac{1}{2}\frac{1}{2}0\}', \{I \frac{1}{2}0\frac{1}{2}\}', \{\sigma_x \frac{1}{2}00\}', \{\sigma_y \frac{1}{2}0\frac{1}{2}\}', \{\sigma_z \frac{1}{2}00\}'$ |
| 55.353 | $Pbam$                | $\{E 000\}, \{C_{2x} \frac{1}{2}\frac{1}{2}0\}, \{C_{2y} \frac{1}{2}\frac{1}{2}0\}, \{C_{2z} 000\}, \{I 000\}, \{\sigma_x \frac{1}{2}\frac{1}{2}0\}, \{\sigma_y \frac{1}{2}\frac{1}{2}0\}, \{\sigma_z 000\}$                                                                                                                                                                                                                                                                                                     |
| 55.354 | $Pbam1'$              | $\{E 000\}, \{C_{2x} \frac{1}{2}\frac{1}{2}0\}, \{C_{2y} \frac{1}{2}\frac{1}{2}0\}, \{C_{2z} 000\}, \{I 000\}, \{\sigma_x \frac{1}{2}\frac{1}{2}0\}, \{\sigma_y \frac{1}{2}\frac{1}{2}0\}, \{\sigma_z 000\}, \{E 000\}', \{C_{2x} \frac{1}{2}\frac{1}{2}0\}', \{C_{2y} \frac{1}{2}\frac{1}{2}0\}', \{C_{2z} 0$                                                                                                                                                                                                   |

[illegible]

[illegible]

[illegible]



[illegible]

[illegible]



[illegible]

[illegible]

[illegible]

| No.   | Symbol       | Elements                                                                                                                                                                                                                                                                                                                                                                                                                                                                                                                 |
|-------|--------------|--------------------------------------------------------------------------------------------------------------------------------------------------------------------------------------------------------------------------------------------------------------------------------------------------------------------------------------------------------------------------------------------------------------------------------------------------------------------------------------------------------------------------|
| 78.21 | $P4'_3$      | $\{E 000\}, \{C_{2z} 00\frac{1}{2}\}, \{C_{4z}^+ 00\frac{3}{4}\}', \{C_{4z}^- 00\frac{1}{4}\}'$                                                                                                                                                                                                                                                                                                                                                                                                                          |
| 78.22 | $P_c4_3$     | $\{E 000\}, \{C_{2z} 00\frac{1}{2}\}, \{C_{4z}^+ 00\frac{3}{4}\}, \{C_{4z}^- 00\frac{1}{4}\}, \{E 00\frac{1}{2}\}', \{C_{2z} 000\}', \{C_{4z}^+ 00\frac{1}{4}\}', \{C_{4z}^- 00\frac{3}{4}\}'$                                                                                                                                                                                                                                                                                                                           |
| 78.23 | $P_C4_3$     | $\{E 000\}, \{C_{2z} 00\frac{1}{2}\}, \{C_{4z}^+ 00\frac{3}{4}\}, \{C_{4z}^- 00\frac{1}{4}\}, \{E \frac{1}{2}\frac{1}{2}0\}', \{C_{2z} \frac{1}{2}\frac{1}{2}\frac{1}{2}\}', \{C_{4z}^+ \frac{1}{2}\frac{1}{2}\frac{3}{4}\}', \{C_{4z}^- \frac{1}{2}\frac{1}{2}\frac{1}{4}\}'$                                                                                                                                                                                                                                           |
| 78.24 | $P_I4_3$     | $\{E 000\}, \{C_{2z} 00\frac{1}{2}\}, \{C_{4z}^+ 00\frac{3}{4}\}, \{C_{4z}^- 00\frac{1}{4}\}, \{E \frac{1}{2}\frac{1}{2}\frac{1}{2}\}', \{C_{2z} \frac{1}{2}\frac{1}{2}0\}', \{C_{4z}^+ \frac{1}{2}\frac{1}{2}\frac{1}{4}\}', \{C_{4z}^- \frac{1}{2}\frac{1}{2}\frac{3}{4}\}'$                                                                                                                                                                                                                                           |
| 79.25 | $I4$         | $\{E 000\}, \{C_{2z} 000\}, \{C_{4z}^+ 000\}, \{C_{4z}^- 000\}$                                                                                                                                                                                                                                                                                                                                                                                                                                                          |
| 79.26 | $I41'$       | $\{E 000\}, \{C_{2z} 000\}, \{C_{4z}^+ 000\}, \{C_{4z}^- 000\}, \{E 000\}', \{C_{2z} 000\}', \{C_{4z}^+ 000\}', \{C_{4z}^- 000\}'$                                                                                                                                                                                                                                                                                                                                                                                       |
| 79.27 | $I4'$        | $\{E 000\}, \{C_{2z} 000\}, \{C_{4z}^+ 000\}', \{C_{4z}^- 000\}'$                                                                                                                                                                                                                                                                                                                                                                                                                                                        |
| 79.28 | $I_c4$       | $\{E 000\}, \{C_{2z} 000\}, \{C_{4z}^+ 000\}, \{C_{4z}^- 000\}, \{E \frac{1}{2}\frac{1}{2}0\}', \{C_{2z} \frac{1}{2}\frac{1}{2}0\}', \{C_{4z}^+ \frac{1}{2}\frac{1}{2}0\}', \{C_{4z}^- \frac{1}{2}\frac{1}{2}0\}'$                                                                                                                                                                                                                                                                                                       |
| 80.29 | $I4_1$       | $\{E 000\}, \{C_{2z} 000\}, \{C_{4z}^+ \frac{3}{4}\frac{1}{4}\frac{1}{2}\}, \{C_{4z}^- \frac{3}{4}\frac{1}{4}\frac{1}{2}\}$                                                                                                                                                                                                                                                                                                                                                                                              |
| 80.30 | $I4_11'$     | $\{E 000\}, \{C_{2z} 000\}, \{C_{4z}^+ \frac{3}{4}\frac{1}{4}\frac{1}{2}\}, \{C_{4z}^- \frac{3}{4}\frac{1}{4}\frac{1}{2}\}, \{E 000\}', \{C_{2z} 000\}', \{C_{4z}^+ \frac{3}{4}\frac{1}{4}\frac{1}{2}\}', \{C_{4z}^- \frac{3}{4}\frac{1}{4}\frac{1}{2}\}'$                                                                                                                                                                                                                                                               |
| 80.31 | $I4'_1$      | $\{E 000\}, \{C_{2z} 000\}, \{C_{4z}^+ \frac{3}{4}\frac{1}{4}\frac{1}{2}\}', \{C_{4z}^- \frac{3}{4}\frac{1}{4}\frac{1}{2}\}'$                                                                                                                                                                                                                                                                                                                                                                                            |
| 80.32 | $I_c4_1$     | $\{E 000\}, \{C_{2z} 000\}, \{C_{4z}^+ \frac{3}{4}\frac{1}{4}\frac{1}{2}\}, \{C_{4z}^- \frac{3}{4}\frac{1}{4}\frac{1}{2}\}, \{E \frac{1}{2}\frac{1}{2}0\}', \{C_{2z} \frac{1}{2}\frac{1}{2}0\}', \{C_{4z}^+ \frac{1}{4}\frac{3}{4}\frac{1}{2}\}', \{C_{4z}^- \frac{1}{4}\frac{3}{4}\frac{1}{2}\}'$                                                                                                                                                                                                                       |
| 81.33 | $P\bar{4}$   | $\{E 000\}, \{C_{2z} 000\}, \{S_{4z}^- 000\}, \{S_{4z}^+ 000\}$                                                                                                                                                                                                                                                                                                                                                                                                                                                          |
| 81.34 | $P\bar{4}1'$ | $\{E 000\}, \{C_{2z} 000\}, \{S_{4z}^- 000\}, \{S_{4z}^+ 000\}, \{E 000\}', \{C_{2z} 000\}', \{S_{4z}^- 000\}', \{S_{4z}^+ 000\}'$                                                                                                                                                                                                                                                                                                                                                                                       |
| 81.35 | $P\bar{4}'$  | $\{E 000\}, \{C_{2z} 000\}, \{S_{4z}^- 000\}', \{S_{4z}^+ 000\}'$                                                                                                                                                                                                                                                                                                                                                                                                                                                        |
| 81.36 | $P_c\bar{4}$ | $\{E 000\}, \{C_{2z} 000\}, \{S_{4z}^- 000\}, \{S_{4z}^+ 000\}, \{E 00\frac{1}{2}\}', \{C_{2z} 00\frac{1}{2}\}', \{S_{4z}^- 00\frac{1}{2}\}', \{S_{4z}^+ 00\frac{1}{2}\}'$                                                                                                                                                                                                                                                                                                                                               |
| 81.37 | $P_C\bar{4}$ | $\{E 000\}, \{C_{2z} 000\}, \{S_{4z}^- 000\}, \{S_{4z}^+ 000\}, \{E \frac{1}{2}\frac{1}{2}0\}', \{C_{2z} \frac{1}{2}\frac{1}{2}0\}', \{S_{4z}^- \frac{1}{2}\frac{1}{2}0\}', \{S_{4z}^+ \frac{1}{2}\frac{1}{2}0\}'$                                                                                                                                                                                                                                                                                                       |
| 81.38 | $P_I\bar{4}$ | $\{E 000\}, \{C_{2z} 000\}, \{S_{4z}^- 000\}, \{S_{4z}^+ 000\}, \{E \frac{1}{2}\frac{1}{2}\frac{1}{2}\}', \{C_{2z} \frac{1}{2}\frac{1}{2}\frac{1}{2}\}', \{S_{4z}^- \frac{1}{2}\frac{1}{2}\frac{1}{2}\}', \{S_{4z}^+ \frac{1}{2}\frac{1}{2}\frac{1}{2}\}'$                                                                                                                                                                                                                                                               |
| 82.39 | $I\bar{4}$   | $\{E 000\}, \{C_{2z} 000\}, \{S_{4z}^- 000\}, \{S_{4z}^+ 000\}$                                                                                                                                                                                                                                                                                                                                                                                                                                                          |
| 82.40 | $I\bar{4}1'$ | $\{E 000\}, \{C_{2z} 000\}, \{S_{4z}^- 000\}, \{S_{4z}^+ 000\}, \{E 000\}', \{C_{2z} 000\}', \{S_{4z}^- 000\}', \{S_{4z}^+ 000\}'$                                                                                                                                                                                                                                                                                                                                                                                       |
| 82.41 | $I\bar{4}'$  | $\{E 000\}, \{C_{2z} 000\}, \{S_{4z}^- 000\}', \{S_{4z}^+ 000\}'$                                                                                                                                                                                                                                                                                                                                                                                                                                                        |
| 82.42 | $I_c\bar{4}$ | $\{E 000\}, \{C_{2z} 000\}, \{S_{4z}^- 000\}, \{S_{4z}^+ 000\}, \{E \frac{1}{2}\frac{1}{2}0\}', \{C_{2z} \frac{1}{2}\frac{1}{2}0\}', \{S_{4z}^- \frac{1}{2}\frac{1}{2}0\}', \{S_{4z}^+ \frac{1}{2}\frac{1}{2}0\}'$                                                                                                                                                                                                                                                                                                       |
| 83.43 | $P4/m$       | $\{E 000\}, \{C_{2z} 000\}, \{C_{4z}^+ 000\}, \{C_{4z}^- 000\}, \{I 000\}, \{\sigma_z 000\}, \{S_{4z}^- 000\}, \{S_{4z}^+ 000\}$                                                                                                                                                                                                                                                                                                                                                                                         |
| 83.44 | $P4/m1'$     | $\{E 000\}, \{C_{2z} 000\}, \{C_{4z}^+ 000\}, \{C_{4z}^- 000\}, \{I 000\}, \{\sigma_z 000\}, \{S_{4z}^- 000\}, \{S_{4z}^+ 000\}, \{E 000\}', \{C_{2z} 000\}', \{C_{4z}^+ 000\}', \{C_{4z}^- 000\}', \{I 000\}', \{\sigma_z 000\}', \{S_{4z}^- 000\}', \{S_{4z}^+ 000\}'$                                                                                                                                                                                                                                                 |
| 83.45 | $P4'/m$      | $\{E 000\}, \{C_{2z} 000\}, \{C_{4z}^+ 000\}', \{C_{4z}^- 000\}', \{I 000\}, \{\sigma_z 000\}, \{S_{4z}^- 000\}', \{S_{4z}^+ 000\}'$                                                                                                                                                                                                                                                                                                                                                                                     |
| 83.46 | $P4/m'$      | $\{E 000\}, \{C_{2z} 000\}, \{C_{4z}^+ 000\}, \{C_{4z}^- 000\}, \{I 000\}', \{\sigma_z 000\}', \{S_{4z}^- 000\}', \{S_{4z}^+ 000\}'$                                                                                                                                                                                                                                                                                                                                                                                     |
| 83.47 | $P4'/m'$     | $\{E 000\}, \{C_{2z} 000\}, \{C_{4z}^+ 000\}', \{C_{4z}^- 000\}', \{I 000\}', \{\sigma_z 000\}', \{S_{4z}^- 000\}, \{S_{4z}^+ 000\}$                                                                                                                                                                                                                                                                                                                                                                                     |
| 83.48 | $P_c4/m$     | $\{E 000\}, \{C_{2z} 000\}, \{C_{4z}^+ 000\}, \{C_{4z}^- 000\}, \{I 000\}, \{\sigma_z 000\}, \{S_{4z}^- 000\}, \{S_{4z}^+ 000\}, \{E 00\frac{1}{2}\}', \{C_{2z} 00\frac{1}{2}\}', \{C_{4z}^+ 00\frac{1}{2}\}', \{C_{4z}^- 00\frac{1}{2}\}', \{I 00\frac{1}{2}\}', \{\sigma_z 00\frac{1}{2}\}', \{S_{4z}^- 00\frac{1}{2}\}', \{S_{4z}^+ 00\frac{1}{2}\}'$                                                                                                                                                                 |
| 83.49 | $P_C4/m$     | $\{E 000\}, \{C_{2z} 000\}, \{C_{4z}^+ 000\}, \{C_{4z}^- 000\}, \{I 000\}, \{\sigma_z 000\}, \{S_{4z}^- 000\}, \{S_{4z}^+ 000\}, \{E \frac{1}{2}\frac{1}{2}0\}', \{C_{2z} \frac{1}{2}\frac{1}{2}0\}', \{C_{4z}^+ \frac{1}{2}\frac{1}{2}0\}', \{C_{4z}^- \frac{1}{2}\frac{1}{2}0\}', \{I \frac{1}{2}\frac{1}{2}0\}', \{\sigma_z \frac{1}{2}\frac{1}{2}0\}', \{S_{4z}^- \frac{1}{2}\frac{1}{2}0\}', \{S_{4z}^+ \frac{1}{2}\frac{1}{2}0\}'$                                                                                 |
| 83.50 | $P_I4/m$     | $\{E 000\}, \{C_{2z} 000\}, \{C_{4z}^+ 000\}, \{C_{4z}^- 000\}, \{I 000\}, \{\sigma_z 000\}, \{S_{4z}^- 000\}, \{S_{4z}^+ 000\}, \{E \frac{1}{2}\frac{1}{2}\frac{1}{2}\}', \{C_{2z} \frac{1}{2}\frac{1}{2}\frac{1}{2}\}', \{C_{4z}^+ \frac{1}{2}\frac{1}{2}\frac{1}{2}\}', \{C_{4z}^- \frac{1}{2}\frac{1}{2}\frac{1}{2}\}', \{I \frac{1}{2}\frac{1}{2}\frac{1}{2}\}', \{\sigma_z \frac{1}{2}\frac{1}{2}\frac{1}{2}\}', \{S_{4z}^- \frac{1}{2}\frac{1}{2}\frac{1}{2}\}', \{S_{4z}^+ \frac{1}{2}\frac{1}{2}\frac{1}{2}\}'$ |
| 84.51 | $P4_2/m$     | $\{E 000\}, \{C_{2z} 000\}, \{C_{4z}^+ 00\frac{1}{2}\}, \{C_{4z}^- 00\frac{1}{2}\}, \{I 00\frac{1}{2}\}, \{\sigma_z 00\frac{1}{2}\}, \{S_{4z}^- 000\}, \{S_{4z}^+ 000\}$                                                                                                                                                                                                                                                                                                                                                 |
| 84.52 | $P4_2/m1'$   | $\{E 000\}, \{C_{2z} 000\}, \{C_{4z}^+ 00\frac{1}{2}\}, \{C_{4z}^- 00\frac{1}{2}\}, \{I 00\frac{1}{2}\}, \{\sigma_z 00\frac{1}{2}\}, \{S_{4z}^- 000\}, \{S_{4z}^+ 000\}, \{E 000\}', \{C_{2z} 000\}', \{C_{4z}^+ 00\frac{1}{2}\}', \{C_{4z}^- 00\frac{1}{2}\}', \{I 00\frac{1}{2}\}', \{\sigma_z 00\frac{1}{2}\}', \{S_{4z}^- 000\}', \{S_{4z}^+ 000\}'$                                                                                                                                                                 |
| 84.53 | $P4'_2/m$    | $\{E 000\}, \{C_{2z} 000\}, \{C_{4z}^+ 00\frac{1}{2}\}', \{C_{4z}^- 00\frac{1}{2}\}', \{I 00\frac{1}{2}\}, \{\sigma_z 00\frac{1}{2}\}, \{S_{4z}^- 000\}', \{S_{4z}^+ 000\}'$                                                                                                                                                                                                                                                                                                                                             |

[illegible]

| No.   | Symbol     | Elements                                                                                                                                                                                                                                                                                                                                                                                                                                                                                                                                                                                                           |
|-------|------------|--------------------------------------------------------------------------------------------------------------------------------------------------------------------------------------------------------------------------------------------------------------------------------------------------------------------------------------------------------------------------------------------------------------------------------------------------------------------------------------------------------------------------------------------------------------------------------------------------------------------|
| 87.79 | $I4'/m'$   | $\{E 000\}, \{C_{2z} 000\}, \{C_{4z}^+ 000\}', \{C_{4z}^- 000\}', \{I 000\}', \{\sigma_z 000\}', \{S_{4z}^- 000\}, \{S_{4z}^+ 000\}$                                                                                                                                                                                                                                                                                                                                                                                                                                                                               |
| 87.80 | $I_c4/m$   | $\{E 000\}, \{C_{2z} 000\}, \{C_{4z}^+ 000\}, \{C_{4z}^- 000\}, \{I 000\}, \{\sigma_z 000\}, \{S_{4z}^- 000\}, \{S_{4z}^+ 000\}, \{E \frac{1}{2}\frac{1}{2}0\}',$<br>$\{C_{2z} \frac{1}{2}\frac{1}{2}0\}', \{C_{4z}^+ \frac{1}{2}\frac{1}{2}0\}', \{C_{4z}^- \frac{1}{2}\frac{1}{2}0\}', \{I \frac{1}{2}\frac{1}{2}0\}', \{\sigma_z \frac{1}{2}\frac{1}{2}0\}', \{S_{4z}^- \frac{1}{2}\frac{1}{2}0\}', \{S_{4z}^+ \frac{1}{2}\frac{1}{2}0\}'$                                                                                                                                                                      |
| 88.81 | $I4_1/a$   | $\{E 000\}, \{C_{2z} 000\}, \{C_{4z}^+ \frac{3}{4}\frac{1}{4}\frac{1}{2}\}, \{C_{4z}^- \frac{3}{4}\frac{1}{4}\frac{1}{2}\}, \{I \frac{3}{4}\frac{1}{4}\frac{1}{2}\}, \{\sigma_z \frac{3}{4}\frac{1}{4}\frac{1}{2}\}, \{S_{4z}^- 000\}, \{S_{4z}^+ 000\}$                                                                                                                                                                                                                                                                                                                                                           |
| 88.82 | $I4_1/a1'$ | $\{E 000\}, \{C_{2z} 000\}, \{C_{4z}^+ \frac{3}{4}\frac{1}{4}\frac{1}{2}\}, \{C_{4z}^- \frac{3}{4}\frac{1}{4}\frac{1}{2}\}, \{I \frac{3}{4}\frac{1}{4}\frac{1}{2}\}, \{\sigma_z \frac{3}{4}\frac{1}{4}\frac{1}{2}\}, \{S_{4z}^- 000\}, \{S_{4z}^+ 000\},$<br>$\{E 000\}', \{C_{2z} 000\}', \{C_{4z}^+ \frac{3}{4}\frac{1}{4}\frac{1}{2}\}', \{C_{4z}^- \frac{3}{4}\frac{1}{4}\frac{1}{2}\}', \{I \frac{3}{4}\frac{1}{4}\frac{1}{2}\}', \{\sigma_z \frac{3}{4}\frac{1}{4}\frac{1}{2}\}', \{S_{4z}^- 000\}', \{S_{4z}^+ 000\}'$                                                                                      |
| 88.83 | $I4_1'/a$  | $\{E 000\}, \{C_{2z} 000\}, \{C_{4z}^+ \frac{3}{4}\frac{1}{4}\frac{1}{2}\}', \{C_{4z}^- \frac{3}{4}\frac{1}{4}\frac{1}{2}\}', \{I \frac{3}{4}\frac{1}{4}\frac{1}{2}\}, \{\sigma_z \frac{3}{4}\frac{1}{4}\frac{1}{2}\}, \{S_{4z}^- 000\}', \{S_{4z}^+ 000\}'$                                                                                                                                                                                                                                                                                                                                                       |
| 88.84 | $I4_1/a'$  | $\{E 000\}, \{C_{2z} 000\}, \{C_{4z}^+ \frac{3}{4}\frac{1}{4}\frac{1}{2}\}, \{C_{4z}^- \frac{3}{4}\frac{1}{4}\frac{1}{2}\}, \{I \frac{3}{4}\frac{1}{4}\frac{1}{2}\}', \{\sigma_z \frac{3}{4}\frac{1}{4}\frac{1}{2}\}', \{S_{4z}^- 000\}', \{S_{4z}^+ 000\}'$                                                                                                                                                                                                                                                                                                                                                       |
| 88.85 | $I4_1'/a'$ | $\{E 000\}, \{C_{2z} 000\}, \{C_{4z}^+ \frac{3}{4}\frac{1}{4}\frac{1}{2}\}', \{C_{4z}^- \frac{3}{4}\frac{1}{4}\frac{1}{2}\}', \{I \frac{3}{4}\frac{1}{4}\frac{1}{2}\}', \{\sigma_z \frac{3}{4}\frac{1}{4}\frac{1}{2}\}', \{S_{4z}^- 000\}, \{S_{4z}^+ 000\}$                                                                                                                                                                                                                                                                                                                                                       |
| 88.86 | $I_c4_1/a$ | $\{E 000\}, \{C_{2z} 000\}, \{C_{4z}^+ \frac{3}{4}\frac{1}{4}\frac{1}{2}\}, \{C_{4z}^- \frac{3}{4}\frac{1}{4}\frac{1}{2}\}, \{I \frac{3}{4}\frac{1}{4}\frac{1}{2}\}, \{\sigma_z \frac{3}{4}\frac{1}{4}\frac{1}{2}\}, \{S_{4z}^- 000\}, \{S_{4z}^+ 000\},$<br>$\{E \frac{1}{2}\frac{1}{2}0\}', \{C_{2z} \frac{1}{2}\frac{1}{2}0\}', \{C_{4z}^+ \frac{1}{4}\frac{3}{4}\frac{1}{2}\}', \{C_{4z}^- \frac{1}{4}\frac{3}{4}\frac{1}{2}\}', \{I \frac{1}{4}\frac{3}{4}\frac{1}{2}\}', \{\sigma_z \frac{1}{4}\frac{3}{4}\frac{1}{2}\}', \{S_{4z}^- \frac{1}{2}\frac{1}{2}0\}',$<br>$\{S_{4z}^+ \frac{1}{2}\frac{1}{2}0\}'$ |
| 89.87 | $P422$     | $\{E 000\}, \{C_{2x} 000\}, \{C_{2y} 000\}, \{C_{2z} 000\}, \{C_{4z}^+ 000\}, \{C_{4z}^- 000\}, \{C_{2a} 000\}, \{C_{2b} 000\}$                                                                                                                                                                                                                                                                                                                                                                                                                                                                                    |
| 89.88 | $P4221'$   | $\{E 000\}, \{C_{2x} 000\}, \{C_{2y} 000\}, \{C_{2z} 000\}, \{C_{4z}^+ 000\}, \{C_{4z}^- 000\}, \{C_{2a} 000\}, \{C_{2b} 000\},$<br>$\{E 000\}', \{C_{2x} 000\}', \{C_{2y} 000\}', \{C_{2z} 000\}', \{C_{4z}^+ 000\}', \{C_{4z}^- 000\}', \{C_{2a} 000\}', \{C_{2b} 000\}'$                                                                                                                                                                                                                                                                                                                                        |
| 89.89 | $P4'22'$   | $\{E 000\}, \{C_{2x} 000\}, \{C_{2y} 000\}, \{C_{2z} 000\}, \{C_{4z}^+ 000\}', \{C_{4z}^- 000\}', \{C_{2a} 000\}', \{C_{2b} 000\}'$                                                                                                                                                                                                                                                                                                                                                                                                                                                                                |
| 89.90 | $P42'2'$   | $\{E 000\}, \{C_{2x} 000\}', \{C_{2y} 000\}', \{C_{2z} 000\}, \{C_{4z}^+ 000\}, \{C_{4z}^- 000\}, \{C_{2a} 000\}', \{C_{2b} 000\}'$                                                                                                                                                                                                                                                                                                                                                                                                                                                                                |
| 89.91 | $P4'2'2$   | $\{E 000\}, \{C_{2x} 000\}', \{C_{2y} 000\}', \{C_{2z} 000\}, \{C_{4z}^+ 000\}', \{C_{4z}^- 000\}', \{C_{2a} 000\}, \{C_{2b} 000\}$                                                                                                                                                                                                                                                                                                                                                                                                                                                                                |
| 89.92 | $P_c422$   | $\{E 000\}, \{C_{2x} 000\}, \{C_{2y} 000\}, \{C_{2z} 000\}, \{C_{4z}^+ 000\}, \{C_{4z}^- 000\}, \{C_{2a} 000\}, \{C_{2b} 000\},$<br>$\{E 00\frac{1}{2}\}', \{C_{2x} 00\frac{1}{2}\}', \{C_{2y} 00\frac{1}{2}\}', \{C_{2z} 00\frac{1}{2}\}', \{C_{4z}^+ 00\frac{1}{2}\}', \{C_{4z}^- 00\frac{1}{2}\}', \{C_{2a} 00\frac{1}{2}\}',$<br>$\{C_{2b} 00\frac{1}{2}\}'$                                                                                                                                                                                                                                                   |
| 89.93 | $P_C422$   | $\{E 000\}, \{C_{2x} 000\}, \{C_{2y} 000\}, \{C_{2z} 000\}, \{C_{4z}^+ 000\}, \{C_{4z}^- 000\}, \{C_{2a} 000\}, \{C_{2b} 000\},$<br>$\{E \frac{1}{2}\frac{1}{2}0\}', \{C_{2x} \frac{1}{2}\frac{1}{2}0\}', \{C_{2y} \frac{1}{2}\frac{1}{2}0\}', \{C_{2z} \frac{1}{2}\frac{1}{2}0\}', \{C_{4z}^+ \frac{1}{2}\frac{1}{2}0\}', \{C_{4z}^- \frac{1}{2}\frac{1}{2}0\}', \{C_{2a} \frac{1}{2}\frac{1}{2}0\}',$<br>$\{C_{2b} \frac{1}{2}\frac{1}{2}0\}'$                                                                                                                                                                   |
| 89.94 | $P_I422$   | $\{E 000\}, \{C_{2x} 000\}, \{C_{2y} 000\}, \{C_{2z} 000\}, \{C_{4z}^+ 000\}, \{C_{4z}^- 000\}, \{C_{2a} 000\}, \{C_{2b} 000\},$<br>$\{E \frac{1}{2}\frac{1}{2}\frac{1}{2}\}', \{C_{2x} \frac{1}{2}\frac{1}{2}\frac{1}{2}\}', \{C_{2y} \frac{1}{2}\frac{1}{2}\frac{1}{2}\}', \{C_{2z} \frac{1}{2}\frac{1}{2}\frac{1}{2}\}', \{C_{4z}^+ \frac{1}{2}\frac{1}{2}\frac{1}{2}\}', \{C_{4z}^- \frac{1}{2}\frac{1}{2}\frac{1}{2}\}', \{C_{2a} \frac{1}{2}\frac{1}{2}\frac{1}{2}\}',$<br>$\{C_{2b} \frac{1}{2}\frac{1}{2}\frac{1}{2}\}'$                                                                                   |
| 90.95 | $P42_12$   | $\{E 000\}, \{C_{2x} \frac{1}{2}\frac{1}{2}0\}, \{C_{2y} \frac{1}{2}\frac{1}{2}0\}, \{C_{2z} 000\}, \{C_{4z}^+ 000\}, \{C_{4z}^- 000\}, \{C_{2a} \frac{1}{2}\frac{1}{2}0\}, \{C_{2b} \frac{1}{2}\frac{1}{2}0\}$                                                                                                                                                                                                                                                                                                                                                                                                    |
| 90.96 | $P42_121'$ | $\{E 000\}, \{C_{2x} \frac{1}{2}\frac{1}{2}0\}, \{C_{2y} \frac{1}{2}\frac{1}{2}0\}, \{C_{2z} 000\}, \{C_{4z}^+ 000\}, \{C_{4z}^- 000\}, \{C_{2a} \frac{1}{2}\frac{1}{2}0\}, \{C_{2b}$                                                                                                                                                                                                                                                                                                                                                                                                                              |

[illegible]



[illegible]



[illegible]

[illegible]

[illegible]

[illegible]

[illegible]

[illegible]

[illegible]



[illegible]



| No.     | Symbol               | Elements                                                                                                                                                                                                                                                                                                                                                                                                                                                                                                                                                                                                                                                                                                                                     |
|---------|----------------------|----------------------------------------------------------------------------------------------------------------------------------------------------------------------------------------------------------------------------------------------------------------------------------------------------------------------------------------------------------------------------------------------------------------------------------------------------------------------------------------------------------------------------------------------------------------------------------------------------------------------------------------------------------------------------------------------------------------------------------------------|
| 122.335 | $\bar{1}\bar{4}'2'd$ | $\{E 000\}, \{C_{2x} \frac{1}{4}\frac{3}{4}\frac{1}{2}\}', \{C_{2y} \frac{1}{4}\frac{3}{4}\frac{1}{2}\}', \{C_{2z} 000\}, \{S_{4z}^- 000\}', \{S_{4z}^+ 000\}', \{\sigma_{da} \frac{1}{4}\frac{3}{4}\frac{1}{2}\}, \{\sigma_{db} \frac{1}{4}\frac{3}{4}\frac{1}{2}\}$                                                                                                                                                                                                                                                                                                                                                                                                                                                                        |
| 122.336 | $\bar{1}\bar{4}'2d'$ | $\{E 000\}, \{C_{2x} \frac{1}{4}\frac{3}{4}\frac{1}{2}\}, \{C_{2y} \frac{1}{4}\frac{3}{4}\frac{1}{2}\}, \{C_{2z} 000\}, \{S_{4z}^- 000\}', \{S_{4z}^+ 000\}', \{\sigma_{da} \frac{1}{4}\frac{3}{4}\frac{1}{2}\}', \{\sigma_{db} \frac{1}{4}\frac{3}{4}\frac{1}{2}\}'$                                                                                                                                                                                                                                                                                                                                                                                                                                                                        |
| 122.337 | $\bar{1}\bar{4}2'd'$ | $\{E 000\}, \{C_{2x} \frac{1}{4}\frac{3}{4}\frac{1}{2}\}', \{C_{2y} \frac{1}{4}\frac{3}{4}\frac{1}{2}\}', \{C_{2z} 000\}, \{S_{4z}^- 000\}, \{S_{4z}^+ 000\}, \{\sigma_{da} \frac{1}{4}\frac{3}{4}\frac{1}{2}\}', \{\sigma_{db} \frac{1}{4}\frac{3}{4}\frac{1}{2}\}'$                                                                                                                                                                                                                                                                                                                                                                                                                                                                        |
| 122.338 | $I_c\bar{4}2d$       | $\{E 000\}, \{C_{2x} \frac{1}{4}\frac{3}{4}\frac{1}{2}\}, \{C_{2y} \frac{1}{4}\frac{3}{4}\frac{1}{2}\}, \{C_{2z} 000\}, \{S_{4z}^- 000\}, \{S_{4z}^+ 000\}, \{\sigma_{da} \frac{1}{4}\frac{3}{4}\frac{1}{2}\}, \{\sigma_{db} \frac{1}{4}\frac{3}{4}\frac{1}{2}\}, \{E \frac{1}{2}\frac{1}{2}0\}', \{C_{2x} \frac{3}{4}\frac{1}{4}\frac{1}{2}\}', \{C_{2y} \frac{3}{4}\frac{1}{4}\frac{1}{2}\}', \{C_{2z} \frac{1}{2}\frac{1}{2}0\}', \{S_{4z}^- \frac{1}{2}\frac{1}{2}0\}', \{S_{4z}^+ \frac{1}{2}\frac{1}{2}0\}', \{\sigma_{da} \frac{3}{4}\frac{1}{4}\frac{1}{2}\}', \{\sigma_{db} \frac{3}{4}\frac{1}{4}\frac{1}{2}\}'$                                                                                                                   |
| 123.339 | $P4/mmm$             | $\{E 000\}, \{C_{2x} 000\}, \{C_{2y} 000\}, \{C_{2z} 000\}, \{C_{4z}^+ 000\}, \{C_{4z}^- 000\}, \{C_{2a} 000\}, \{C_{2b} 000\}, \{I 000\}, \{\sigma_x 000\}, \{\sigma_y 000\}, \{\sigma_z 000\}, \{S_{4z}^- 000\}, \{S_{4z}^+ 000\}, \{\sigma_{da} 000\}, \{\sigma_{db} 000\}$                                                                                                                                                                                                                                                                                                                                                                                                                                                               |
| 123.340 | $P4/mmm1'$           | $\{E 000\}, \{C_{2x} 000\}, \{C_{2y} 000\}, \{C_{2z} 000\}, \{C_{4z}^+ 000\}, \{C_{4z}^- 000\}, \{C_{2a} 000\}, \{C_{2b} 000\}, \{I 000\}, \{\sigma_x 000\}, \{\sigma_y 000\}, \{\sigma_z 000\}, \{S_{4z}^- 000\}, \{S_{4z}^+ 000\}, \{\sigma_{da} 000\}, \{\sigma_{db} 000\}, \{E 000\}', \{C_{2x} 000\}', \{C_{2y} 000\}', \{C_{2z} 000\}', \{C_{4z}^+ 000\}', \{C_{4z}^- 000\}', \{C_{2a} 000\}', \{C_{2b} 000\}', \{I 000\}', \{\sigma_x 000\}', \{\sigma_y 000\}', \{\sigma_z 000\}', \{S_{4z}^- 000\}', \{S_{4z}^+ 000\}', \{\sigma_{da} 000\}', \{\sigma_{db} 000\}'$                                                                                                                                                                 |
| 123.341 | $P4/m'mm$            | $\{E 000\}, \{C_{2x} 000\}', \{C_{2y} 000\}', \{C_{2z} 000\}, \{C_{4z}^+ 000\}, \{C_{4z}^- 000\}, \{C_{2a} 000\}', \{C_{2b} 000\}', \{I 000\}', \{\sigma_x 000\}, \{\sigma_y 000\}, \{\sigma_z 000\}', \{S_{4z}^- 000\}', \{S_{4z}^+ 000\}', \{\sigma_{da} 000\}, \{\sigma_{db} 000\}$                                                                                                                                                                                                                                                                                                                                                                                                                                                       |
| 123.342 | $P4'/mm'm$           | $\{E 000\}, \{C_{2x} 000\}', \{C_{2y} 000\}', \{C_{2z} 000\}, \{C_{4z}^+ 000\}', \{C_{4z}^- 000\}', \{C_{2a} 000\}, \{C_{2b} 000\}, \{I 000\}, \{\sigma_x 000\}', \{\sigma_y 000\}', \{\sigma_z 000\}, \{S_{4z}^- 000\}', \{S_{4z}^+ 000\}', \{\sigma_{da} 000\}, \{\sigma_{db} 000\}$                                                                                                                                                                                                                                                                                                                                                                                                                                                       |
| 123.343 | $P4'/mmm'$           | $\{E 000\}, \{C_{2x} 000\}, \{C_{2y} 000\}, \{C_{2z} 000\}, \{C_{4z}^+ 000\}', \{C_{4z}^- 000\}', \{C_{2a} 000\}', \{C_{2b} 000\}', \{I 000\}, \{\sigma_x 000\}, \{\sigma_y 000\}, \{\sigma_z 000\}, \{S_{4z}^- 000\}', \{S_{4z}^+ 000\}', \{\sigma_{da} 000\}', \{\sigma_{db} 000\}'$                                                                                                                                                                                                                                                                                                                                                                                                                                                       |
| 123.344 | $P4'/m'm'm$          | $\{E 000\}, \{C_{2x} 000\}, \{C_{2y} 000\}, \{C_{2z} 000\}, \{C_{4z}^+ 000\}', \{C_{4z}^- 000\}', \{C_{2a} 000\}', \{C_{2b} 000\}', \{I 000\}', \{\sigma_x 000\}', \{\sigma_y 000\}', \{\sigma_z 000\}', \{S_{4z}^- 000\}, \{S_{4z}^+ 000\}, \{\sigma_{da} 000\}, \{\sigma_{db} 000\}$                                                                                                                                                                                                                                                                                                                                                                                                                                                       |
| 123.345 | $P4/mm'm'$           | $\{E 000\}, \{C_{2x} 000\}', \{C_{2y} 000\}', \{C_{2z} 000\}, \{C_{4z}^+ 000\}, \{C_{4z}^- 000\}, \{C_{2a} 000\}', \{C_{2b} 000\}', \{I 000\}, \{\sigma_x 000\}', \{\sigma_y 000\}', \{\sigma_z 000\}, \{S_{4z}^- 000\}, \{S_{4z}^+ 000\}, \{\sigma_{da} 000\}', \{\sigma_{db} 000\}'$                                                                                                                                                                                                                                                                                                                                                                                                                                                       |
| 123.346 | $P4'/m'mm'$          | $\{E 000\}, \{C_{2x} 000\}', \{C_{2y} 000\}', \{C_{2z} 000\}, \{C_{4z}^+ 000\}', \{C_{4z}^- 000\}', \{C_{2a} 000\}, \{C_{2b} 000\}, \{I 000\}', \{\sigma_x 000\}, \{\sigma_y 000\}, \{\sigma_z 000\}', \{S_{4z}^- 000\}, \{S_{4z}^+ 000\}, \{\sigma_{da} 000\}', \{\sigma_{db} 000\}'$                                                                                                                                                                                                                                                                                                                                                                                                                                                       |
| 123.347 | $P4/m'm'm'$          | $\{E 000\}, \{C_{2x} 000\}, \{C_{2y} 000\}, \{C_{2z} 000\}, \{C_{4z}^+ 000\}, \{C_{4z}^- 000\}, \{C_{2a} 000\}, \{C_{2b} 000\}, \{I 000\}', \{\sigma_x 000\}', \{\sigma_y 000\}', \{\sigma_z 000\}', \{S_{4z}^- 000\}', \{S_{4z}^+ 000\}', \{\sigma_{da} 000\}', \{\sigma_{db} 000\}'$                                                                                                                                                                                                                                                                                                                                                                                                                                                       |
| 123.348 | $P_c4/mmm$           | $\{E 000\}, \{C_{2x} 000\}, \{C_{2y} 000\}, \{C_{2z} 000\}, \{C_{4z}^+ 000\}, \{C_{4z}^- 000\}, \{C_{2a} 000\}, \{C_{2b} 000\}, \{I 000\}, \{\sigma_x 000\}, \{\sigma_y 000\}, \{\sigma_z 000\}, \{S_{4z}^- 000\}, \{S_{4z}^+ 000\}, \{\sigma_{da} 000\}, \{\sigma_{db} 000\}, \{E 00\frac{1}{2}\}', \{C_{2x} 00\frac{1}{2}\}', \{C_{2y} 00\frac{1}{2}\}', \{C_{2z} 00\frac{1}{2}\}', \{C_{4z}^+ 00\frac{1}{2}\}', \{C_{4z}^- 00\frac{1}{2}\}', \{C_{2a} 00\frac{1}{2}\}', \{C_{2b} 00\frac{1}{2}\}', \{I 00\frac{1}{2}\}', \{\sigma_x 00\frac{1}{2}\}', \{\sigma_y 00\frac{1}{2}\}', \{\sigma_z 00\frac{1}{2}\}', \{S_{4z}^- 00\frac{1}{2}\}', \{S_{4z}^+ 00\frac{1}{2}\}', \{\sigma_{da} 00\frac{1}{2}\}', \{\sigma_{db} 00\frac{1}{2}\}'$ |
| 123.349 | $P_C4/mmm$           | $\{E 000\}, \{C_{2x} 000\}, \{C_{2y} 000\}, \{C_{2z} 000\}, \{C_{4z}^+ 000\}, \{C_{4z}^- 000\}, \{C_{2a} 000\}, \{C_{2b} 000\}, \{I 000\}, \{\sigma_x 000\}, \{\sigma_y 000\}, \{\sigma_z 000\}, \{S_{4z}^- 000\}, \{S_{4z}^+ 000\}, \{\sigma_{da} 000\}, \{\sigma_{db} 000\}, \{E \frac{1}{2}\frac{1}{2}0\}', \{C_{2x} \frac{1}{2}\frac{1}{2}0\}', \{C_{2y} \frac{1}{2}\frac{1}{2}0\}', \{C_{2z} \frac{1}{2}\frac{1}{2}0\}', \{C_{4z}^+ \frac{1}{2}\frac{1}{2}0\}', \{C_{4z$                                                                                                                                                                                                                                                                |

[illegible]

[illegible]

[illegible]

[illegible]

[illegible]

[illegible]



[illegible]



[illegible]

[illegible]

[illegible]

[illegible]

[illegible]

[illegible]

[illegible]



[illegible]



| No.     | Symbol        | Elements                                                                                                                                                                                                                                                                                                                                                                                                                                                                                                                                                                                                                                                                                                                                                                                                                                                                                                                                                                                                                                                                     |
|---------|---------------|------------------------------------------------------------------------------------------------------------------------------------------------------------------------------------------------------------------------------------------------------------------------------------------------------------------------------------------------------------------------------------------------------------------------------------------------------------------------------------------------------------------------------------------------------------------------------------------------------------------------------------------------------------------------------------------------------------------------------------------------------------------------------------------------------------------------------------------------------------------------------------------------------------------------------------------------------------------------------------------------------------------------------------------------------------------------------|
| 142.570 | $I_c 4_1/acd$ | $\{E 000\}, \{C_{2x} \frac{1}{2}\frac{1}{2}0\}, \{C_{2y} 0\frac{1}{2}\frac{1}{2}\}, \{C_{2z} \frac{1}{2}0\frac{1}{2}\}, \{C_{4z}^+ \frac{1}{2}00\}, \{C_{4z}^- \frac{1}{2}\frac{1}{2}\frac{1}{2}\}, \{C_{2a} 0\frac{1}{2}0\}, \{C_{2b} 00\frac{1}{2}\}, \{I 000\}, \{\sigma_x \frac{1}{2}\frac{1}{2}0\}, \{\sigma_y 0\frac{1}{2}\frac{1}{2}\}, \{\sigma_z \frac{1}{2}0\frac{1}{2}\}, \{S_{4z}^- \frac{1}{2}00\}, \{S_{4z}^+ \frac{1}{2}\frac{1}{2}\frac{1}{2}\}, \{\sigma_{da} 0\frac{1}{2}0\}, \{\sigma_{db} 00\frac{1}{2}\}, \{E \frac{1}{2}\frac{1}{2}0\}', \{C_{2x} 000\}', \{C_{2y} \frac{1}{2}0\frac{1}{2}\}', \{C_{2z} 0\frac{1}{2}\frac{1}{2}\}', \{C_{4z}^+ 0\frac{1}{2}0\}', \{C_{4z}^- 00\frac{1}{2}\}', \{C_{2a} \frac{1}{2}00\}', \{C_{2b} \frac{1}{2}\frac{1}{2}\frac{1}{2}\}', \{I \frac{1}{2}\frac{1}{2}0\}', \{\sigma_x 000\}', \{\sigma_y 0\frac{1}{2}\frac{1}{2}\}', \{\sigma_z 0\frac{1}{2}\frac{1}{2}\}', \{S_{4z}^- 0\frac{1}{2}0\}', \{S_{4z}^+ 00\frac{1}{2}\}', \{\sigma_{da} \frac{1}{2}00\}', \{\sigma_{db} \frac{1}{2}\frac{1}{2}\frac{1}{2}\}'$ |
| 143.1   | $P3$          | $\{E 000\}, \{C_3^+ 000\}, \{C_3^- 000\}$                                                                                                                                                                                                                                                                                                                                                                                                                                                                                                                                                                                                                                                                                                                                                                                                                                                                                                                                                                                                                                    |
| 143.2   | $P31'$        | $\{E 000\}, \{C_3^+ 000\}, \{C_3^- 000\}, \{E 000\}', \{C_3^+ 000\}', \{C_3^- 000\}'$                                                                                                                                                                                                                                                                                                                                                                                                                                                                                                                                                                                                                                                                                                                                                                                                                                                                                                                                                                                        |
| 143.3   | $P_c3$        | $\{E 000\}, \{C_3^+ 000\}, \{C_3^- 000\}, \{E 00\frac{1}{2}\}', \{C_3^+ 00\frac{1}{2}\}', \{C_3^- 00\frac{1}{2}\}'$                                                                                                                                                                                                                                                                                                                                                                                                                                                                                                                                                                                                                                                                                                                                                                                                                                                                                                                                                          |
| 144.4   | $P3_1$        | $\{E 000\}, \{C_3^+ 00\frac{1}{3}\}, \{C_3^- 00\frac{2}{3}\}$                                                                                                                                                                                                                                                                                                                                                                                                                                                                                                                                                                                                                                                                                                                                                                                                                                                                                                                                                                                                                |
| 144.5   | $P3_11'$      | $\{E 000\}, \{C_3^+ 00\frac{1}{3}\}, \{C_3^- 00\frac{2}{3}\}, \{E 000\}', \{C_3^+ 00\frac{1}{3}\}', \{C_3^- 00\frac{2}{3}\}'$                                                                                                                                                                                                                                                                                                                                                                                                                                                                                                                                                                                                                                                                                                                                                                                                                                                                                                                                                |
| 144.6   | $P_c3_1$      | $\{E 000\}, \{C_3^+ 00\frac{1}{3}\}, \{C_3^- 00\frac{2}{3}\}, \{E 00\frac{1}{2}\}', \{C_3^+ 00\frac{5}{6}\}', \{C_3^- 00\frac{1}{6}\}'$                                                                                                                                                                                                                                                                                                                                                                                                                                                                                                                                                                                                                                                                                                                                                                                                                                                                                                                                      |
| 145.7   | $P3_2$        | $\{E 000\}, \{C_3^+ 00\frac{2}{3}\}, \{C_3^- 00\frac{1}{3}\}$                                                                                                                                                                                                                                                                                                                                                                                                                                                                                                                                                                                                                                                                                                                                                                                                                                                                                                                                                                                                                |
| 145.8   | $P3_21'$      | $\{E 000\}, \{C_3^+ 00\frac{2}{3}\}, \{C_3^- 00\frac{1}{3}\}, \{E 000\}', \{C_3^+ 00\frac{2}{3}\}', \{C_3^- 00\frac{1}{3}\}'$                                                                                                                                                                                                                                                                                                                                                                                                                                                                                                                                                                                                                                                                                                                                                                                                                                                                                                                                                |
| 145.9   | $P_c3_2$      | $\{E 000\}, \{C_3^+ 00\frac{2}{3}\}, \{C_3^- 00\frac{1}{3}\}, \{E 00\frac{1}{2}\}', \{C_3^+ 00\frac{1}{6}\}', \{C_3^- 00\frac{5}{6}\}'$                                                                                                                                                                                                                                                                                                                                                                                                                                                                                                                                                                                                                                                                                                                                                                                                                                                                                                                                      |
| 146.10  | $R3$          | $\{E 000\}, \{C_3^+ 000\}, \{C_3^- 000\}$                                                                                                                                                                                                                                                                                                                                                                                                                                                                                                                                                                                                                                                                                                                                                                                                                                                                                                                                                                                                                                    |
| 146.11  | $R31'$        | $\{E 000\}, \{C_3^+ 000\}, \{C_3^- 000\}, \{E 000\}', \{C_3^+ 000\}', \{C_3^- 000\}'$                                                                                                                                                                                                                                                                                                                                                                                                                                                                                                                                                                                                                                                                                                                                                                                                                                                                                                                                                                                        |
| 146.12  | $R_I3$        | $\{E 000\}, \{C_3^+ 000\}, \{C_3^- 000\}, \{E \frac{1}{2}\frac{1}{2}\frac{1}{2}\}', \{C_3^+ \frac{1}{2}\frac{1}{2}\frac{1}{2}\}', \{C_3^- \frac{1}{2}\frac{1}{2}\frac{1}{2}\}'$                                                                                                                                                                                                                                                                                                                                                                                                                                                                                                                                                                                                                                                                                                                                                                                                                                                                                              |
| 147.13  | $P\bar{3}$    | $\{E 000\}, \{I 000\}, \{C_3^+ 000\}, \{C_3^- 000\}, \{S_6^- 000\}, \{S_6^+ 000\}$                                                                                                                                                                                                                                                                                                                                                                                                                                                                                                                                                                                                                                                                                                                                                                                                                                                                                                                                                                                           |
| 147.14  | $P\bar{3}1'$  | $\{E 000\}, \{I 000\}, \{C_3^+ 000\}, \{C_3^- 000\}, \{S_6^- 000\}, \{S_6^+ 000\}, \{E 000\}', \{I 000\}', \{C_3^+ 000\}', \{C_3^- 000\}', \{S_6^- 000\}', \{S_6^+ 000\}'$                                                                                                                                                                                                                                                                                                                                                                                                                                                                                                                                                                                                                                                                                                                                                                                                                                                                                                   |
| 147.15  | $P\bar{3}'$   | $\{E 000\}, \{I 000\}', \{C_3^+ 000\}, \{C_3^- 000\}, \{S_6^- 000\}', \{S_6^+ 000\}'$                                                                                                                                                                                                                                                                                                                                                                                                                                                                                                                                                                                                                                                                                                                                                                                                                                                                                                                                                                                        |
| 147.16  | $P_c\bar{3}$  | $\{E 000\}, \{I 000\}, \{C_3^+ 000\}, \{C_3^- 000\}, \{S_6^- 000\}, \{S_6^+ 000\}, \{E 00\frac{1}{2}\}', \{I 00\frac{1}{2}\}', \{C_3^+ 00\frac{1}{2}\}', \{C_3^- 00\frac{1}{2}\}', \{S_6^- 00\frac{1}{2}\}', \{S_6^+ 00\frac{1}{2}\}'$                                                                                                                                                                                                                                                                                                                                                                                                                                                                                                                                                                                                                                                                                                                                                                                                                                       |
| 148.17  | $R\bar{3}$    | $\{E 000\}, \{I 000\}, \{C_3^+ 000\}, \{C_3^- 000\}, \{S_6^- 000\}, \{S_6^+ 000\}$                                                                                                                                                                                                                                                                                                                                                                                                                                                                                                                                                                                                                                                                                                                                                                                                                                                                                                                                                                                           |
| 148.18  | $R\bar{3}1'$  | $\{E 000\}, \{I 000\}, \{C_3^+ 000\}, \{C_3^- 000\}, \{S_6^- 000\}, \{S_6^+ 000\}, \{E 000\}', \{I 000\}', \{C_3^+ 000\}', \{C_3^- 000\}', \{S_6^- 000\}', \{S_6^+ 000\}'$                                                                                                                                                                                                                                                                                                                                                                                                                                                                                                                                                                                                                                                                                                                                                                                                                                                                                                   |
| 148.19  | $R\bar{3}'$   | $\{E 000\}, \{I 000\}', \{C_3^+ 000\}, \{C_3^- 000\}, \{S_6^- 000\}', \{S_6^+ 000\}'$                                                                                                                                                                                                                                                                                                                                                                                                                                                                                                                                                                                                                                                                                                                                                                                                                                                                                                                                                                                        |
| 148.20  | $R_I\bar{3}$  | $\{E 000\}, \{I 000\}, \{C_3^+ 000\}, \{C_3^- 000\}, \{S_6^- 000\}, \{S_6^+ 000\}, \{E \frac{1}{2}\frac{1}{2}\frac{1}{2}\}', \{I \frac{1}{2}\frac{1}{2}\frac{1}{2}\}', \{C_3^+ \frac{1}{2}\frac{1}{2}\frac{1}{2}\}', \{C_3^- \frac{1}{2}\frac{1}{2}\frac{1}{2}\}', \{S_6^- \frac{1}{2}\frac{1}{2}\frac{1}{2}\}', \{S_6^+ \frac{1}{2}\frac{1}{2}\frac{1}{2}\}'$                                                                                                                                                                                                                                                                                                                                                                                                                                                                                                                                                                                                                                                                                                               |
| 149.21  | $P312$        | $\{E 000\}, \{C_3^+ 000\}, \{C_3^- 000\}, \{C'_{21} 000\}, \{C'_{22} 000\}, \{C'_{23} 000\}$                                                                                                                                                                                                                                                                                                                                                                                                                                                                                                                                                                                                                                                                                                                                                                                                                                                                                                                                                                                 |
| 149.22  | $P3121'$      | $\{E 000\}, \{C_3^+ 000\}, \{C_3^- 000\}, \{C'_{21} 000\}, \{C'_{22} 000\}, \{C'_{23} 000\}, \{E 000\}', \{C_3^+ 000\}', \{C_3^- 000\}', \{C'_{21} 000\}', \{C'_{22} 000\}', \{C'_{23} 000\}'$                                                                                                                                                                                                                                                                                                                                                                                                                                                                                                                                                                                                                                                                                                                                                                                                                                                                               |
| 149.23  | $P312'$       | $\{E 000\}, \{C_3^+ 000\}, \{C_3^- 000\}, \{C'_{21} 000\}', \{C'_{22} 000\}', \{C'_{23} 000\}'$                                                                                                                                                                                                                                                                                                                                                                                                                                                                                                                                                                                                                                                                                                                                                                                                                                                                                                                                                                              |
| 149.24  | $P_c312$      | $\{E 000\}, \{C_3^+ 000\}, \{C_3^- 000\}, \{C'_{21} 000\}, \{C'_{22} 000\}, \{C'_{23} 000\}, \{E 00\frac{1}{2}\}', \{C_3^+ 00\frac{1}{2}\}', \{C_3^- 00\frac{1}{2}\}', \{C'_{21} 00\frac{1}{2}\}', \{C'_{22} 00\frac{1}{2}\}', \{C'_{23} 00\frac{1}{2}\}'$                                                                                                                                                                                                                                                                                                                                                                                                                                                                                                                                                                                                                                                                                                                                                                                                                   |
| 150.25  | $P321$        | $\{E 000\}, \{C_3^+ 000\}, \{C_3^- 000\}, \{C''_{21} 000\}, \{C''_{22} 000\}, \{C''_{23} 000\}$                                                                                                                                                                                                                                                                                                                                                                                                                                                                                                                                                                                                                                                                                                                                                                                                                                                                                                                                                                              |
| 150.26  | $P3211'$      | $\{E 000\}, \{C_3^+ 000\}, \{C_3^- 000\}, \{C''_{21} 000\}, \{C''_{22} 000\}, \{C''_{23} 000\}, \{E 000\}', \{C_3^+ 000\}', \{C_3^- 000\}', \{C''_{21} 000\}', \{C''_{22} 000\}', \{C''_{23} 000\}'$                                                                                                                                                                                                                                                                                                                                                                                                                                                                                                                                                                                                                                                                                                                                                                                                                                                                         |
| 150.27  | $P32'1$       | $\{E 000\}, \{C_3^+ 000\}, \{C_3^- 000\}, \{C''_{21} 000\}', \{C''_{22} 000\}', \{C''_{23} 000\}'$                                                                                                                                                                                                                                                                                                                                                                                                                                                                                                                                                                                                                                                                                                                                                                                                                                                                                                                                                                           |

| No.    | Symbol     | Elements                                                                                                                                                                                                                                                                                                                                                                           |
|--------|------------|------------------------------------------------------------------------------------------------------------------------------------------------------------------------------------------------------------------------------------------------------------------------------------------------------------------------------------------------------------------------------------|
| 150.28 | $P_c321$   | $\{E 000\}, \{C_3^+ 000\}, \{C_3^- 000\}, \{C_{21}'' 000\}, \{C_{22}'' 000\}, \{C_{23}'' 000\}, \{E 00\frac{1}{2}\}', \{C_3^+ 00\frac{1}{2}\}', \{C_3^- 00\frac{1}{2}\}', \{C_{21}' 00\frac{1}{2}\}', \{C_{22}' 00\frac{1}{2}\}', \{C_{23}' 00\frac{1}{2}\}'$                                                                                                                      |
| 151.29 | $P3_112$   | $\{E 000\}, \{C_3^+ 00\frac{1}{3}\}, \{C_3^- 00\frac{2}{3}\}, \{C_{21}' 00\frac{2}{3}\}, \{C_{22}' 00\frac{1}{3}\}, \{C_{23}' 000\}$                                                                                                                                                                                                                                               |
| 151.30 | $P3_1121'$ | $\{E 000\}, \{C_3^+ 00\frac{1}{3}\}, \{C_3^- 00\frac{2}{3}\}, \{C_{21}' 00\frac{2}{3}\}, \{C_{22}' 00\frac{1}{3}\}, \{C_{23}' 000\}, \{E 000\}', \{C_3^+ 00\frac{1}{3}\}', \{C_3^- 00\frac{2}{3}\}', \{C_{21}' 00\frac{2}{3}\}', \{C_{22}' 00\frac{1}{3}\}', \{C_{23}' 000\}'$                                                                                                     |
| 151.31 | $P3_112'$  | $\{E 000\}, \{C_3^+ 00\frac{1}{3}\}, \{C_3^- 00\frac{2}{3}\}, \{C_{21}' 00\frac{2}{3}\}', \{C_{22}' 00\frac{1}{3}\}', \{C_{23}' 000\}'$                                                                                                                                                                                                                                            |
| 151.32 | $P_c3_112$ | $\{E 000\}, \{C_3^+ 00\frac{1}{3}\}, \{C_3^- 00\frac{2}{3}\}, \{C_{21}' 00\frac{2}{3}\}, \{C_{22}' 00\frac{1}{3}\}, \{C_{23}' 000\}, \{E 00\frac{1}{2}\}', \{C_3^+ 00\frac{5}{6}\}', \{C_3^- 00\frac{1}{6}\}', \{C_{21}' 00\frac{1}{6}\}', \{C_{22}' 00\frac{5}{6}\}', \{C_{23}' 00\frac{1}{2}\}'$                                                                                 |
| 152.33 | $P3_121$   | $\{E 000\}, \{C_3^+ 00\frac{1}{3}\}, \{C_3^- 00\frac{2}{3}\}, \{C_{21}'' 00\frac{2}{3}\}, \{C_{22}'' 00\frac{1}{3}\}, \{C_{23}'' 000\}$                                                                                                                                                                                                                                            |
| 152.34 | $P3_1211'$ | $\{E 000\}, \{C_3^+ 00\frac{1}{3}\}, \{C_3^- 00\frac{2}{3}\}, \{C_{21}'' 00\frac{2}{3}\}, \{C_{22}'' 00\frac{1}{3}\}, \{C_{23}'' 000\}, \{E 000\}', \{C_3^+ 00\frac{1}{3}\}', \{C_3^- 00\frac{2}{3}\}', \{C_{21}'' 00\frac{2}{3}\}', \{C_{22}'' 00\frac{1}{3}\}', \{C_{23}'' 000\}'$                                                                                               |
| 152.35 | $P3_12'1$  | $\{E 000\}, \{C_3^+ 00\frac{1}{3}\}, \{C_3^- 00\frac{2}{3}\}, \{C_{21}'' 00\frac{2}{3}\}', \{C_{22}'' 00\frac{1}{3}\}', \{C_{23}'' 000\}'$                                                                                                                                                                                                                                         |
| 152.36 | $P_c3_121$ | $\{E 000\}, \{C_3^+ 00\frac{1}{3}\}, \{C_3^- 00\frac{2}{3}\}, \{C_{21}'' 00\frac{2}{3}\}, \{C_{22}'' 00\frac{1}{3}\}, \{C_{23}'' 000\}, \{E 00\frac{1}{2}\}', \{C_3^+ 00\frac{5}{6}\}', \{C_3^- 00\frac{1}{6}\}', \{C_{21}'' 00\frac{1}{6}\}', \{C_{22}'' 00\frac{5}{6}\}', \{C_{23}'' 00\frac{1}{2}\}'$                                                                           |
| 153.37 | $P3_212$   | $\{E 000\}, \{C_3^+ 00\frac{2}{3}\}, \{C_3^- 00\frac{1}{3}\}, \{C_{21}' 00\frac{1}{3}\}, \{C_{22}' 00\frac{2}{3}\}, \{C_{23}' 000\}$                                                                                                                                                                                                                                               |
| 153.38 | $P3_2121'$ | $\{E 000\}, \{C_3^+ 00\frac{2}{3}\}, \{C_3^- 00\frac{1}{3}\}, \{C_{21}' 00\frac{1}{3}\}, \{C_{22}' 00\frac{2}{3}\}, \{C_{23}' 000\}, \{E 000\}', \{C_3^+ 00\frac{2}{3}\}', \{C_3^- 00\frac{1}{3}\}', \{C_{21}' 00\frac{1}{3}\}', \{C_{22}' 00\frac{2}{3}\}', \{C_{23}' 000\}'$                                                                                                     |
| 153.39 | $P3_212'$  | $\{E 000\}, \{C_3^+ 00\frac{2}{3}\}, \{C_3^- 00\frac{1}{3}\}, \{C_{21}' 00\frac{1}{3}\}', \{C_{22}' 00\frac{2}{3}\}', \{C_{23}' 000\}'$                                                                                                                                                                                                                                            |
| 153.40 | $P_c3_212$ | $\{E 000\}, \{C_3^+ 00\frac{2}{3}\}, \{C_3^- 00\frac{1}{3}\}, \{C_{21}' 00\frac{1}{3}\}, \{C_{22}' 00\frac{2}{3}\}, \{C_{23}' 000\}, \{E 00\frac{1}{2}\}', \{C_3^+ 00\frac{1}{6}\}', \{C_3^- 00\frac{5}{6}\}', \{C_{21}' 00\frac{5}{6}\}', \{C_{22}' 00\frac{1}{6}\}', \{C_{23}' 00\frac{1}{2}\}'$                                                                                 |
| 154.41 | $P3_221$   | $\{E 000\}, \{C_3^+ 00\frac{2}{3}\}, \{C_3^- 00\frac{1}{3}\}, \{C_{21}'' 00\frac{1}{3}\}, \{C_{22}'' 00\frac{2}{3}\}, \{C_{23}'' 000\}$                                                                                                                                                                                                                                            |
| 154.42 | $P3_2211'$ | $\{E 000\}, \{C_3^+ 00\frac{2}{3}\}, \{C_3^- 00\frac{1}{3}\}, \{C_{21}'' 00\frac{1}{3}\}, \{C_{22}'' 00\frac{2}{3}\}, \{C_{23}'' 000\}, \{E 000\}', \{C_3^+ 00\frac{2}{3}\}', \{C_3^- 00\frac{1}{3}\}', \{C_{21}'' 00\frac{1}{3}\}', \{C_{22}'' 00\frac{2}{3}\}', \{C_{23}'' 000\}'$                                                                                               |
| 154.43 | $P3_22'1$  | $\{E 000\}, \{C_3^+ 00\frac{2}{3}\}, \{C_3^- 00\frac{1}{3}\}, \{C_{21}'' 00\frac{1}{3}\}', \{C_{22}'' 00\frac{2}{3}\}', \{C_{23}'' 000\}'$                                                                                                                                                                                                                                         |
| 154.44 | $P_c3_221$ | $\{E 000\}, \{C_3^+ 00\frac{2}{3}\}, \{C_3^- 00\frac{1}{3}\}, \{C_{21}'' 00\frac{1}{3}\}, \{C_{22}'' 00\frac{2}{3}\}, \{C_{23}'' 000\}, \{E 00\frac{1}{2}\}', \{C_3^+ 00\frac{1}{6}\}', \{C_3^- 00\frac{5}{6}\}', \{C_{21}'' 00\frac{5}{6}\}', \{C_{22}'' 00\frac{1}{6}\}', \{C_{23}'' 00\frac{1}{2}\}'$                                                                           |
| 155.45 | $R32$      | $\{E 000\}, \{C_3^+ 000\}, \{C_3^- 000\}, \{C_{21}' 000\}, \{C_{22}' 000\}, \{C_{23}' 000\}$                                                                                                                                                                                                                                                                                       |
| 155.46 | $R321'$    | $\{E 000\}, \{C_3^+ 000\}, \{C_3^- 000\}, \{C_{21}' 000\}, \{C_{22}' 000\}, \{C_{23}' 000\}, \{E 000\}', \{C_3^+ 000\}', \{C_3^- 000\}', \{C_{21}' 000\}', \{C_{22}' 000\}', \{C_{23}' 000\}'$                                                                                                                                                                                     |
| 155.47 | $R32'$     | $\{E 000\}, \{C_3^+ 000\}, \{C_3^- 000\}, \{C_{21}' 000\}', \{C_{22}' 000\}', \{C_{23}' 000\}'$                                                                                                                                                                                                                                                                                    |
| 155.48 | $R_132$    | $\{E 000\}, \{C_3^+ 000\}, \{C_3^- 000\}, \{C_{21}' 000\}, \{C_{22}' 000\}, \{C_{23}' 000\}, \{E \frac{1}{2}\frac{1}{2}\frac{1}{2}\}', \{C_3^+ \frac{1}{2}\frac{1}{2}\frac{1}{2}\}', \{C_3^- \frac{1}{2}\frac{1}{2}\frac{1}{2}\}', \{C_{21}' \frac{1}{2}\frac{1}{2}\frac{1}{2}\}', \{C_{22}' \frac{1}{2}\frac{1}{2}\frac{1}{2}\}', \{C_{23}' \frac{1}{2}\frac{1}{2}\frac{1}{2}\}'$ |
| 156.49 | $P3m1$     | $\{E 000\}, \{C_3^+ 000\}, \{C_3^- 000\}, \{\sigma_{v1} 000\}, \{\sigma_{v2} 000\}, \{\sigma_{v3} 000\}$                                                                                                                                                                                                                                                                           |
| 156.50 | $P3m11'$   | $\{E 000\}, \{C_3^+ 000\}, \{C_3^- 000\}, \{\sigma_{v1} 000\}, \{\sigma_{v2} 000\}, \{\sigma_{v3} 000\}, \{E 000\}', \{C_3^+ 000\}', \{C_3^- 000\}', \{\sigma_{v1} 000\}', \{\sigma_{v2} 000\}', \{\sigma_{v3} 000\}'$                                                                                                                                                             |
| 156.51 | $P3m'1$    | $\{E 000\}, \{C_3^+ 000\}, \{C_3^- 000\}, \{\sigma_{v1} 000\}', \{\sigma_{v2} 000\}', \{\sigma_{v3} 000\}'$                                                                                                                                                                                                                                                                        |
| 156.52 | $P_c3m1$   | $\{E 000\}, \{C_3^+ 000\}, \{C_3^- 000\}, \{\sigma_{v1} 000\}, \{\sigma_{v2} 000\}, \{\sigma_{v3} 000\}, \{E 00\frac{1}{2}\}', \{C_3^+ 00\frac{1}{2}\}', \{C_3^- 00\frac{1}{2}\}', \{\sigma_{v1} 00\frac{1}{2}\}', \{\sigma_{v2} 00\frac{1}{2}\}', \{\sigma_{v3} 00\frac{1}{2}\}'$                                                                                                 |
| 157.53 | $P31m$     | $\{E 000\}, \{C_3^+ 000\}, \{C_3^- 000\}, \{\sigma_{d1} 000\}, \{\sigma_{d2} 000\}, \{\sigma_{d3} 000\}$                                                                                                                                                                                                                                                                           |

[illegible]

[illegible]

[illegible]

| No.     | Symbol       | Elements                                                                                                                                                                                                                                                                                                                                                               |
|---------|--------------|------------------------------------------------------------------------------------------------------------------------------------------------------------------------------------------------------------------------------------------------------------------------------------------------------------------------------------------------------------------------|
| 169.116 | $P_c6_1$     | $\{E 000\}, \{C_6^+ 00\frac{1}{6}\}, \{C_3^+ 00\frac{1}{3}\}, \{C_2 00\frac{1}{2}\}, \{C_3^- 00\frac{2}{3}\}, \{C_6^- 00\frac{5}{6}\}, \{E 00\frac{1}{2}\}', \{C_6^+ 00\frac{2}{3}\}', \{C_3^+ 00\frac{5}{6}\}', \{C_2 000\}', \{C_3^- 00\frac{1}{6}\}', \{C_6^- 00\frac{1}{3}\}'$                                                                                     |
| 170.117 | $P6_5$       | $\{E 000\}, \{C_6^+ 00\frac{5}{6}\}, \{C_3^+ 00\frac{2}{3}\}, \{C_2 00\frac{1}{2}\}, \{C_3^- 00\frac{1}{3}\}, \{C_6^- 00\frac{1}{6}\}$                                                                                                                                                                                                                                 |
| 170.118 | $P6_51'$     | $\{E 000\}, \{C_6^+ 00\frac{5}{6}\}, \{C_3^+ 00\frac{2}{3}\}, \{C_2 00\frac{1}{2}\}, \{C_3^- 00\frac{1}{3}\}, \{C_6^- 00\frac{1}{6}\}, \{E 000\}', \{C_6^+ 00\frac{5}{6}\}', \{C_3^+ 00\frac{2}{3}\}', \{C_2 00\frac{1}{2}\}', \{C_3^- 00\frac{1}{3}\}', \{C_6^- 00\frac{1}{6}\}'$                                                                                     |
| 170.119 | $P6_5'$      | $\{E 000\}, \{C_6^+ 00\frac{5}{6}\}', \{C_3^+ 00\frac{2}{3}\}, \{C_2 00\frac{1}{2}\}', \{C_3^- 00\frac{1}{3}\}, \{C_6^- 00\frac{1}{6}\}'$                                                                                                                                                                                                                              |
| 170.120 | $P_c6_5$     | $\{E 000\}, \{C_6^+ 00\frac{5}{6}\}, \{C_3^+ 00\frac{2}{3}\}, \{C_2 00\frac{1}{2}\}, \{C_3^- 00\frac{1}{3}\}, \{C_6^- 00\frac{1}{6}\}, \{E 00\frac{1}{2}\}', \{C_6^+ 00\frac{1}{3}\}', \{C_3^+ 00\frac{1}{6}\}', \{C_2 000\}', \{C_3^- 00\frac{5}{6}\}', \{C_6^- 00\frac{2}{3}\}'$                                                                                     |
| 171.121 | $P6_2$       | $\{E 000\}, \{C_6^+ 00\frac{1}{3}\}, \{C_3^+ 00\frac{2}{3}\}, \{C_2 000\}, \{C_3^- 00\frac{1}{3}\}, \{C_6^- 00\frac{2}{3}\}$                                                                                                                                                                                                                                           |
| 171.122 | $P6_21'$     | $\{E 000\}, \{C_6^+ 00\frac{1}{3}\}, \{C_3^+ 00\frac{2}{3}\}, \{C_2 000\}, \{C_3^- 00\frac{1}{3}\}, \{C_6^- 00\frac{2}{3}\}, \{E 000\}', \{C_6^+ 00\frac{1}{3}\}', \{C_3^+ 00\frac{2}{3}\}', \{C_2 000\}', \{C_3^- 00\frac{1}{3}\}', \{C_6^- 00\frac{2}{3}\}'$                                                                                                         |
| 171.123 | $P6_2'$      | $\{E 000\}, \{C_6^+ 00\frac{1}{3}\}', \{C_3^+ 00\frac{2}{3}\}, \{C_2 000\}', \{C_3^- 00\frac{1}{3}\}, \{C_6^- 00\frac{2}{3}\}'$                                                                                                                                                                                                                                        |
| 171.124 | $P_c6_2$     | $\{E 000\}, \{C_6^+ 00\frac{1}{3}\}, \{C_3^+ 00\frac{2}{3}\}, \{C_2 000\}, \{C_3^- 00\frac{1}{3}\}, \{C_6^- 00\frac{2}{3}\}, \{E 00\frac{1}{2}\}', \{C_6^+ 00\frac{5}{6}\}', \{C_3^+ 00\frac{1}{6}\}', \{C_2 00\frac{1}{2}\}', \{C_3^- 00\frac{5}{6}\}', \{C_6^- 00\frac{1}{6}\}'$                                                                                     |
| 172.125 | $P6_4$       | $\{E 000\}, \{C_6^+ 00\frac{2}{3}\}, \{C_3^+ 00\frac{1}{3}\}, \{C_2 000\}, \{C_3^- 00\frac{2}{3}\}, \{C_6^- 00\frac{1}{3}\}$                                                                                                                                                                                                                                           |
| 172.126 | $P6_41'$     | $\{E 000\}, \{C_6^+ 00\frac{2}{3}\}, \{C_3^+ 00\frac{1}{3}\}, \{C_2 000\}, \{C_3^- 00\frac{2}{3}\}, \{C_6^- 00\frac{1}{3}\}, \{E 000\}', \{C_6^+ 00\frac{2}{3}\}', \{C_3^+ 00\frac{1}{3}\}', \{C_2 000\}', \{C_3^- 00\frac{2}{3}\}', \{C_6^- 00\frac{1}{3}\}'$                                                                                                         |
| 172.127 | $P6_4'$      | $\{E 000\}, \{C_6^+ 00\frac{2}{3}\}', \{C_3^+ 00\frac{1}{3}\}, \{C_2 000\}', \{C_3^- 00\frac{2}{3}\}, \{C_6^- 00\frac{1}{3}\}'$                                                                                                                                                                                                                                        |
| 172.128 | $P_c6_4$     | $\{E 000\}, \{C_6^+ 00\frac{2}{3}\}, \{C_3^+ 00\frac{1}{3}\}, \{C_2 000\}, \{C_3^- 00\frac{2}{3}\}, \{C_6^- 00\frac{1}{3}\}, \{E 00\frac{1}{2}\}', \{C_6^+ 00\frac{1}{6}\}', \{C_3^+ 00\frac{5}{6}\}', \{C_2 00\frac{1}{2}\}', \{C_3^- 00\frac{5}{6}\}', \{C_6^- 00\frac{5}{6}\}'$                                                                                     |
| 173.129 | $P6_3$       | $\{E 000\}, \{C_6^+ 00\frac{1}{2}\}, \{C_3^+ 000\}, \{C_2 00\frac{1}{2}\}, \{C_3^- 000\}, \{C_6^- 00\frac{1}{2}\}$                                                                                                                                                                                                                                                     |
| 173.130 | $P6_31'$     | $\{E 000\}, \{C_6^+ 00\frac{1}{2}\}, \{C_3^+ 000\}, \{C_2 00\frac{1}{2}\}, \{C_3^- 000\}, \{C_6^- 00\frac{1}{2}\}, \{E 000\}', \{C_6^+ 00\frac{1}{2}\}', \{C_3^+ 000\}', \{C_2 00\frac{1}{2}\}', \{C_3^- 000\}', \{C_6^- 00\frac{1}{2}\}'$                                                                                                                             |
| 173.131 | $P6_3'$      | $\{E 000\}, \{C_6^+ 00\frac{1}{2}\}', \{C_3^+ 000\}, \{C_2 00\frac{1}{2}\}', \{C_3^- 000\}, \{C_6^- 00\frac{1}{2}\}'$                                                                                                                                                                                                                                                  |
| 173.132 | $P_c6_3$     | $\{E 000\}, \{C_6^+ 00\frac{1}{2}\}, \{C_3^+ 000\}, \{C_2 00\frac{1}{2}\}, \{C_3^- 000\}, \{C_6^- 00\frac{1}{2}\}, \{E 00\frac{1}{2}\}', \{C_6^+ 000\}', \{C_3^+ 00\frac{1}{2}\}', \{C_2 000\}', \{C_3^- 00\frac{1}{2}\}', \{C_6^- 000\}'$                                                                                                                             |
| 174.133 | $P\bar{6}$   | $\{E 000\}, \{C_3^+ 000\}, \{C_3^- 000\}, \{S_3^- 000\}, \{\sigma_h 000\}, \{S_3^+ 000\}$                                                                                                                                                                                                                                                                              |
| 174.134 | $P\bar{6}1'$ | $\{E 000\}, \{C_3^+ 000\}, \{C_3^- 000\}, \{S_3^- 000\}, \{\sigma_h 000\}, \{S_3^+ 000\}, \{E 000\}', \{C_3^+ 000\}', \{C_3^- 000\}', \{S_3^- 000\}', \{\sigma_h 000\}', \{S_3^+ 000\}'$                                                                                                                                                                               |
| 174.135 | $P\bar{6}'$  | $\{E 000\}, \{C_3^+ 000\}, \{C_3^- 000\}, \{S_3^- 000\}', \{\sigma_h 000\}', \{S_3^+ 000\}'$                                                                                                                                                                                                                                                                           |
| 174.136 | $P_c\bar{6}$ | $\{E 000\}, \{C_3^+ 000\}, \{C_3^- 000\}, \{S_3^- 000\}, \{\sigma_h 000\}, \{S_3^+ 000\}, \{E 00\frac{1}{2}\}', \{C_3^+ 00\frac{1}{2}\}', \{C_3^- 00\frac{1}{2}\}', \{S_3^- 00\frac{1}{2}\}', \{\sigma_h 00\frac{1}{2}\}', \{S_3^+ 00\frac{1}{2}\}'$                                                                                                                   |
| 175.137 | $P6/m$       | $\{E 000\}, \{I 000\}, \{C_6^+ 000\}, \{C_3^+ 000\}, \{C_2 000\}, \{C_3^- 000\}, \{C_6^- 000\}, \{S_3^- 000\}, \{S_6^- 000\}, \{\sigma_h 000\}, \{S_6^+ 000\}, \{S_3^+ 000\}$                                                                                                                                                                                          |
| 175.138 | $P6/m1'$     | $\{E 000\}, \{I 000\}, \{C_6^+ 000\}, \{C_3^+ 000\}, \{C_2 000\}, \{C_3^- 000\}, \{C_6^- 000\}, \{S_3^- 000\}, \{S_6^- 000\}, \{\sigma_h 000\}, \{S_6^+ 000\}, \{S_3^+ 000\}, \{E 000\}', \{I 000\}', \{C_6^+ 000\}', \{C_3^+ 000\}', \{C_2 000\}', \{C_3^- 000\}', \{C_6^- 000\}', \{S_3^- 000\}', \{S_6^- 000\}', \{\sigma_h 000\}', \{S_6^+ 000\}', \{S_3^+ 000\}'$ |
| 175.139 | $P6'/m$      | $\{E 000\}, \{I 000\}', \{C_6^+ 000\}', \{C_3^+ 000\}, \{C_2 000\}', \{C_3^- 000\}, \{C_6^- 000\}', \{S_3^- 000\}, \{S_6^- 000\}', \{\sigma_h 000\}, \{S_6^+ 000\}', \{S_3^+ 000\}$                                                                                                                                                                                    |

| No.     | Symbol     | Elements                                                                                                                                                                                                                                                                                                                                                                                                                                                                                                                                                                                                                                                                            |
|---------|------------|-------------------------------------------------------------------------------------------------------------------------------------------------------------------------------------------------------------------------------------------------------------------------------------------------------------------------------------------------------------------------------------------------------------------------------------------------------------------------------------------------------------------------------------------------------------------------------------------------------------------------------------------------------------------------------------|
| 175.140 | $P6/m'$    | $\{E 000\}$ , $\{I 000\}'$ , $\{C_6^+ 000\}$ , $\{C_3^+ 000\}$ , $\{C_2 000\}$ , $\{C_3^- 000\}$ , $\{C_6^- 000\}$ , $\{S_3^- 000\}'$ , $\{S_6^- 000\}'$ , $\{\sigma_h 000\}'$ , $\{S_6^+ 000\}'$ , $\{S_3^+ 000\}'$                                                                                                                                                                                                                                                                                                                                                                                                                                                                |
| 175.141 | $P6'/m'$   | $\{E 000\}$ , $\{I 000\}$ , $\{C_6^+ 000\}'$ , $\{C_3^+ 000\}$ , $\{C_2 000\}'$ , $\{C_3^- 000\}$ , $\{C_6^- 000\}'$ , $\{S_3^- 000\}'$ , $\{S_6^- 000\}$ , $\{\sigma_h 000\}'$ , $\{S_6^+ 000\}$ , $\{S_3^+ 000\}'$                                                                                                                                                                                                                                                                                                                                                                                                                                                                |
| 175.142 | $P_c6/m$   | $\{E 000\}$ , $\{I 000\}$ , $\{C_6^+ 000\}$ , $\{C_3^+ 000\}$ , $\{C_2 000\}$ , $\{C_3^- 000\}$ , $\{C_6^- 000\}$ , $\{S_3^- 000\}$ , $\{S_6^- 000\}$ , $\{\sigma_h 000\}$ , $\{S_6^+ 000\}$ , $\{S_3^+ 000\}$ , $\{E 00\frac{1}{2}\}'$ , $\{I 00\frac{1}{2}\}'$ , $\{C_6^+ 00\frac{1}{2}\}'$ , $\{C_3^+ 00\frac{1}{2}\}'$ , $\{C_2 00\frac{1}{2}\}'$ , $\{C_3^- 00\frac{1}{2}\}'$ , $\{C_6^- 00\frac{1}{2}\}'$ , $\{S_3^- 00\frac{1}{2}\}'$ , $\{S_6^- 00\frac{1}{2}\}'$ , $\{\sigma_h 00\frac{1}{2}\}'$ , $\{S_6^+ 00\frac{1}{2}\}'$ , $\{S_3^+ 00\frac{1}{2}\}'$                                                                                                                 |
| 176.143 | $P6_3/m$   | $\{E 000\}$ , $\{I 00\frac{1}{2}\}$ , $\{C_6^+ 00\frac{1}{2}\}$ , $\{C_3^+ 000\}$ , $\{C_2 00\frac{1}{2}\}$ , $\{C_3^- 000\}$ , $\{C_6^- 00\frac{1}{2}\}$ , $\{S_3^- 000\}$ , $\{S_6^- 00\frac{1}{2}\}$ , $\{\sigma_h 000\}$ , $\{S_6^+ 00\frac{1}{2}\}$ , $\{S_3^+ 000\}$                                                                                                                                                                                                                                                                                                                                                                                                          |
| 176.144 | $P6_3/m1'$ | $\{E 000\}$ , $\{I 00\frac{1}{2}\}$ , $\{C_6^+ 00\frac{1}{2}\}$ , $\{C_3^+ 000\}$ , $\{C_2 00\frac{1}{2}\}$ , $\{C_3^- 000\}$ , $\{C_6^- 00\frac{1}{2}\}$ , $\{S_3^- 000\}$ , $\{S_6^- 00\frac{1}{2}\}$ , $\{\sigma_h 000\}$ , $\{S_6^+ 00\frac{1}{2}\}$ , $\{S_3^+ 000\}$ , $\{E 000\}'$ , $\{I 00\frac{1}{2}\}'$ , $\{C_6^+ 00\frac{1}{2}\}'$ , $\{C_3^+ 000\}'$ , $\{C_2 00\frac{1}{2}\}'$ , $\{C_3^- 000\}'$ , $\{C_6^- 00\frac{1}{2}\}'$ , $\{S_3^- 000\}'$ , $\{S_6^- 00\frac{1}{2}\}'$ , $\{\sigma_h 000\}'$ , $\{S_6^+ 00\frac{1}{2}\}'$ , $\{S_3^+ 000\}'$                                                                                                                 |
| 176.145 | $P6_3'/m$  | $\{E 000\}$ , $\{I 00\frac{1}{2}\}'$ , $\{C_6^+ 00\frac{1}{2}\}'$ , $\{C_3^+ 000\}$ , $\{C_2 00\frac{1}{2}\}'$ , $\{C_3^- 000\}$ , $\{C_6^- 00\frac{1}{2}\}'$ , $\{S_3^- 000\}$ , $\{S_6^- 00\frac{1}{2}\}'$ , $\{\sigma_h 000\}$ , $\{S_6^+ 00\frac{1}{2}\}'$ , $\{S_3^+ 000\}$                                                                                                                                                                                                                                                                                                                                                                                                    |
| 176.146 | $P6_3/m'$  | $\{E 000\}$ , $\{I 00\frac{1}{2}\}'$ , $\{C_6^+ 00\frac{1}{2}\}$ , $\{C_3^+ 000\}$ , $\{C_2 00\frac{1}{2}\}$ , $\{C_3^- 000\}$ , $\{C_6^- 00\frac{1}{2}\}$ , $\{S_3^- 000\}'$ , $\{S_6^- 00\frac{1}{2}\}'$ , $\{\sigma_h 000\}'$ , $\{S_6^+ 00\frac{1}{2}\}'$ , $\{S_3^+ 000\}'$                                                                                                                                                                                                                                                                                                                                                                                                    |
| 176.147 | $P6_3'/m'$ | $\{E 000\}$ , $\{I 00\frac{1}{2}\}$ , $\{C_6^+ 00\frac{1}{2}\}'$ , $\{C_3^+ 000\}$ , $\{C_2 00\frac{1}{2}\}'$ , $\{C_3^- 000\}$ , $\{C_6^- 00\frac{1}{2}\}'$ , $\{S_3^- 000\}'$ , $\{S_6^- 00\frac{1}{2}\}'$ , $\{\sigma_h 000\}'$ , $\{S_6^+ 00\frac{1}{2}\}'$ , $\{S_3^+ 000\}'$                                                                                                                                                                                                                                                                                                                                                                                                  |
| 176.148 | $P_c6_3/m$ | $\{E 000\}$ , $\{I 00\frac{1}{2}\}$ , $\{C_6^+ 00\frac{1}{2}\}$ , $\{C_3^+ 000\}$ , $\{C_2 00\frac{1}{2}\}$ , $\{C_3^- 000\}$ , $\{C_6^- 00\frac{1}{2}\}$ , $\{S_3^- 000\}$ , $\{S_6^- 00\frac{1}{2}\}$ , $\{\sigma_h 000\}$ , $\{S_6^+ 00\frac{1}{2}\}$ , $\{S_3^+ 000\}$ , $\{E 00\frac{1}{2}\}'$ , $\{I 000\}'$ , $\{C_6^+ 000\}'$ , $\{C_3^+ 00\frac{1}{2}\}'$ , $\{C_2 000\}'$ , $\{C_3^- 00\frac{1}{2}\}'$ , $\{C_6^- 000\}'$ , $\{S_3^- 00\frac{1}{2}\}'$ , $\{S_6^- 000\}'$ , $\{\sigma_h 00\frac{1}{2}\}'$ , $\{S_6^+ 000\}'$ , $\{S_3^+ 00\frac{1}{2}\}'$                                                                                                                 |
| 177.149 | $P622$     | $\{E 000\}$ , $\{C_6^+ 000\}$ , $\{C_3^+ 000\}$ , $\{C_2 000\}$ , $\{C_3^- 000\}$ , $\{C_6^- 000\}$ , $\{C'_{21} 000\}$ , $\{C'_{22} 000\}$ , $\{C'_{23} 000\}$ , $\{C''_{21} 000\}$ , $\{C''_{22} 000\}$ , $\{C''_{23} 000\}$                                                                                                                                                                                                                                                                                                                                                                                                                                                      |
| 177.150 | $P6221'$   | $\{E 000\}$ , $\{C_6^+ 000\}$ , $\{C_3^+ 000\}$ , $\{C_2 000\}$ , $\{C_3^- 000\}$ , $\{C_6^- 000\}$ , $\{C'_{21} 000\}$ , $\{C'_{22} 000\}$ , $\{C'_{23} 000\}$ , $\{C''_{21} 000\}$ , $\{C''_{22} 000\}$ , $\{C''_{23} 000\}$ , $\{E 000\}'$ , $\{C_6^+ 000\}'$ , $\{C_3^+ 000\}'$ , $\{C_2 000\}'$ , $\{C_3^- 000\}'$ , $\{C_6^- 000\}'$ , $\{C'_{21} 000\}'$ , $\{C'_{22} 000\}'$ , $\{C'_{23} 000\}'$ , $\{C''_{21} 000\}'$ , $\{C''_{22} 000\}'$ , $\{C''_{23} 000\}'$                                                                                                                                                                                                         |
| 177.151 | $P6'2'2$   | $\{E 000\}$ , $\{C_6^+ 000\}'$ , $\{C_3^+ 000\}$ , $\{C_2 000\}'$ , $\{C_3^- 000\}$ , $\{C_6^- 000\}'$ , $\{C'_{21} 000\}$ , $\{C'_{22} 000\}$ , $\{C'_{23} 000\}$ , $\{C''_{21} 000\}'$ , $\{C''_{22} 000\}'$ , $\{C''_{23} 000\}'$                                                                                                                                                                                                                                                                                                                                                                                                                                                |
| 177.152 | $P6'22'$   | $\{E 000\}$ , $\{C_6^+ 000\}'$ , $\{C_3^+ 000\}$ , $\{C_2 000\}'$ , $\{C_3^- 000\}$ , $\{C_6^- 000\}'$ , $\{C'_{21} 000\}'$ , $\{C'_{22} 000\}'$ , $\{C'_{23} 000\}'$ , $\{C''_{21} 000\}$ , $\{C''_{22} 000\}$ , $\{C''_{23} 000\}$                                                                                                                                                                                                                                                                                                                                                                                                                                                |
| 177.153 | $P62'2'$   | $\{E 000\}$ , $\{C_6^+ 000\}$ , $\{C_3^+ 000\}$ , $\{C_2 000\}$ , $\{C_3^- 000\}$ , $\{C_6^- 000\}$ , $\{C'_{21} 000\}'$ , $\{C'_{22} 000\}'$ , $\{C'_{23} 000\}'$ , $\{C''_{21} 000\}'$ , $\{C''_{22} 000\}'$ , $\{C''_{23} 000\}'$                                                                                                                                                                                                                                                                                                                                                                                                                                                |
| 177.154 | $P_c622$   | $\{E 000\}$ , $\{C_6^+ 000\}$ , $\{C_3^+ 000\}$ , $\{C_2 000\}$ , $\{C_3^- 000\}$ , $\{C_6^- 000\}$ , $\{C'_{21} 000\}$ , $\{C'_{22} 000\}$ , $\{C'_{23} 000\}$ , $\{C''_{21} 000\}$ , $\{C''_{22} 000\}$ , $\{C''_{23} 000\}$ , $\{E 00\frac{1}{2}\}'$ , $\{C_6^+ 00\frac{1}{2}\}'$ , $\{C_3^+ 00\frac{1}{2}\}'$ , $\{C_2 00\frac{1}{2}\}'$ , $\{C_3^- 00\frac{1}{2}\}'$ , $\{C_6^- 00\frac{1}{2}\}'$ , $\{C'_{21} 00\frac{1}{2}\}'$ , $\{C'_{22} 00\frac{1}{2}\}'$ , $\{C'_{23} 00\frac{1}{2}\}'$ , $\{C''_{21} 00\frac{1}{2}\}'$ , $\{C''_{22} 00\frac{1}{2}\}'$ , $\{C''_{23} 00\frac{1}{2}\}'$                                                                                 |
| 178.155 | $P6_122$   | $\{E 000\}$ , $\{C_6^+ 00\frac{1}{6}\}$ , $\{C_3^+ 00\frac{1}{3}\}$ , $\{C_2 00\frac{1}{2}\}$ , $\{C_3^- 00\frac{2}{3}\}$ , $\{C_6^- 00\frac{5}{6}\}$ , $\{C'_{21} 000\}$ , $\{C'_{22} 00\frac{2}{3}\}$ , $\{C'_{23} 00\frac{1}{3}\}$ , $\{C''_{21} 00\frac{1}{2}\}$ , $\{C''_{22} 00\frac{1}{6}\}$ , $\{C''_{23} 00\frac{5}{6}\}$                                                                                                                                                                                                                                                                                                                                                  |
| 178.156 | $P6_1221'$ | $\{E 000\}$ , $\{C_6^+ 00\frac{1}{6}\}$ , $\{C_3^+ 00\frac{1}{3}\}$ , $\{C_2 00\frac{1}{2}\}$ , $\{C_3^- 00\frac{2}{3}\}$ , $\{C_6^- 00\frac{5}{6}\}$ , $\{C'_{21} 000\}$ , $\{C'_{22} 00\frac{2}{3}\}$ , $\{C'_{23} 00\frac{1}{3}\}$ , $\{C''_{21} 00\frac{1}{2}\}$ , $\{C''_{22} 00\frac{1}{6}\}$ , $\{C''_{23} 00\frac{5}{6}\}$ , $\{E 000\}'$ , $\{C_6^+ 00\frac{1}{6}\}'$ , $\{C_3^+ 00\frac{1}{3}\}'$ , $\{C_2 00\frac{1}{2}\}'$ , $\{C_3^- 00\frac{2}{3}\}'$ , $\{C_6^- 00\frac{5}{6}\}'$ , $\{C'_{21} 000\}'$ , $\{C'_{22} 00\frac{2}{3}\}'$ , $\{C'_{23} 00\frac{1}{3}\}'$ , $\{C''_{21} 00\frac{1}{2}\}'$ , $\{C''_{22} 00\frac{1}{6}\}'$ , $\{C''_{23} 00\frac{5}{6}\}'$ |



[illegible]



| No.     | Symbol     | Elements                                                                                                                                                                                                                                                                                                                                                                                                                                                                                                                                                                                                                                                                            |
|---------|------------|-------------------------------------------------------------------------------------------------------------------------------------------------------------------------------------------------------------------------------------------------------------------------------------------------------------------------------------------------------------------------------------------------------------------------------------------------------------------------------------------------------------------------------------------------------------------------------------------------------------------------------------------------------------------------------------|
| 181.173 | $P6_422$   | $\{E 000\}$ , $\{C_6^+ 00\frac{2}{3}\}$ , $\{C_3^+ 00\frac{1}{3}\}$ , $\{C_2 000\}$ , $\{C_3^- 00\frac{2}{3}\}$ , $\{C_6^- 00\frac{1}{3}\}$ , $\{C'_{21} 000\}$ , $\{C'_{22} 00\frac{2}{3}\}$ , $\{C'_{23} 00\frac{1}{3}\}$ , $\{C''_{21} 000\}$ , $\{C''_{22} 00\frac{2}{3}\}$ , $\{C''_{23} 00\frac{1}{3}\}$                                                                                                                                                                                                                                                                                                                                                                      |
| 181.174 | $P6_4221'$ | $\{E 000\}$ , $\{C_6^+ 00\frac{2}{3}\}$ , $\{C_3^+ 00\frac{1}{3}\}$ , $\{C_2 000\}$ , $\{C_3^- 00\frac{2}{3}\}$ , $\{C_6^- 00\frac{1}{3}\}$ , $\{C'_{21} 000\}$ , $\{C'_{22} 00\frac{2}{3}\}$ , $\{C'_{23} 00\frac{1}{3}\}$ , $\{C''_{21} 000\}$ , $\{C''_{22} 00\frac{2}{3}\}$ , $\{C''_{23} 00\frac{1}{3}\}$ , $\{E 000\}'$ , $\{C_6^+ 00\frac{2}{3}\}'$ , $\{C_3^+ 00\frac{1}{3}\}'$ , $\{C_2 000\}'$ , $\{C_3^- 00\frac{2}{3}\}'$ , $\{C_6^- 00\frac{1}{3}\}'$ , $\{C'_{21} 000\}'$ , $\{C'_{22} 00\frac{2}{3}\}'$ , $\{C'_{23} 00\frac{1}{3}\}'$ , $\{C''_{21} 000\}'$ , $\{C''_{22} 00\frac{2}{3}\}'$ , $\{C''_{23} 00\frac{1}{3}\}'$                                         |
| 181.175 | $P6'_42'2$ | $\{E 000\}$ , $\{C_6^+ 00\frac{2}{3}\}'$ , $\{C_3^+ 00\frac{1}{3}\}$ , $\{C_2 000\}'$ , $\{C_3^- 00\frac{2}{3}\}$ , $\{C_6^- 00\frac{1}{3}\}'$ , $\{C'_{21} 000\}$ , $\{C'_{22} 00\frac{2}{3}\}$ , $\{C'_{23} 00\frac{1}{3}\}$ , $\{C''_{21} 000\}'$ , $\{C''_{22} 00\frac{2}{3}\}'$ , $\{C''_{23} 00\frac{1}{3}\}'$                                                                                                                                                                                                                                                                                                                                                                |
| 181.176 | $P6'_422'$ | $\{E 000\}$ , $\{C_6^+ 00\frac{2}{3}\}'$ , $\{C_3^+ 00\frac{1}{3}\}$ , $\{C_2 000\}'$ , $\{C_3^- 00\frac{2}{3}\}$ , $\{C_6^- 00\frac{1}{3}\}'$ , $\{C'_{21} 000\}'$ , $\{C'_{22} 00\frac{2}{3}\}'$ , $\{C'_{23} 00\frac{1}{3}\}'$ , $\{C''_{21} 000\}$ , $\{C''_{22} 00\frac{2}{3}\}$ , $\{C''_{23} 00\frac{1}{3}\}$                                                                                                                                                                                                                                                                                                                                                                |
| 181.177 | $P6_42'2'$ | $\{E 000\}$ , $\{C_6^+ 00\frac{2}{3}\}$ , $\{C_3^+ 00\frac{1}{3}\}$ , $\{C_2 000\}$ , $\{C_3^- 00\frac{2}{3}\}$ , $\{C_6^- 00\frac{1}{3}\}$ , $\{C'_{21} 000\}'$ , $\{C'_{22} 00\frac{2}{3}\}'$ , $\{C'_{23} 00\frac{1}{3}\}'$ , $\{C''_{21} 000\}'$ , $\{C''_{22} 00\frac{2}{3}\}'$ , $\{C''_{23} 00\frac{1}{3}\}'$                                                                                                                                                                                                                                                                                                                                                                |
| 181.178 | $P_c6_422$ | $\{E 000\}$ , $\{C_6^+ 00\frac{2}{3}\}$ , $\{C_3^+ 00\frac{1}{3}\}$ , $\{C_2 000\}$ , $\{C_3^- 00\frac{2}{3}\}$ , $\{C_6^- 00\frac{1}{3}\}$ , $\{C'_{21} 000\}$ , $\{C'_{22} 00\frac{2}{3}\}$ , $\{C'_{23} 00\frac{1}{3}\}$ , $\{C''_{21} 000\}$ , $\{C''_{22} 00\frac{2}{3}\}$ , $\{C''_{23} 00\frac{1}{3}\}$ , $\{E 00\frac{1}{2}\}'$ , $\{C_6^+ 00\frac{1}{6}\}'$ , $\{C_3^+ 00\frac{5}{6}\}'$ , $\{C_2 00\frac{1}{2}\}'$ , $\{C_3^- 00\frac{1}{6}\}'$ , $\{C_6^- 00\frac{5}{6}\}'$ , $\{C'_{21} 00\frac{1}{2}\}'$ , $\{C'_{22} 00\frac{1}{6}\}'$ , $\{C'_{23} 00\frac{5}{6}\}'$ , $\{C''_{21} 00\frac{1}{2}\}'$ , $\{C''_{22} 00\frac{1}{6}\}'$ , $\{C''_{23} 00\frac{5}{6}\}'$ |
| 182.179 | $P6_322$   | $\{E 000\}$ , $\{C_6^+ 00\frac{1}{2}\}$ , $\{C_3^+ 000\}$ , $\{C_2 00\frac{1}{2}\}$ , $\{C_3^- 000\}$ , $\{C_6^- 00\frac{1}{2}\}$ , $\{C'_{21} 000\}$ , $\{C'_{22} 000\}$ , $\{C'_{23} 000\}$ , $\{C''_{21} 00\frac{1}{2}\}$ , $\{C''_{22} 00\frac{1}{2}\}$ , $\{C''_{23} 00\frac{1}{2}\}$                                                                                                                                                                                                                                                                                                                                                                                          |
| 182.180 | $P6_3221'$ | $\{E 000\}$ , $\{C_6^+ 00\frac{1}{2}\}$ , $\{C_3^+ 000\}$ , $\{C_2 00\frac{1}{2}\}$ , $\{C_3^- 000\}$ , $\{C_6^- 00\frac{1}{2}\}$ , $\{C'_{21} 000\}$ , $\{C'_{22} 000\}$ , $\{C'_{23} 000\}$ , $\{C''_{21} 00\frac{1}{2}\}$ , $\{C''_{22} 00\frac{1}{2}\}$ , $\{C''_{23} 00\frac{1}{2}\}$ , $\{E 000\}'$ , $\{C_6^+ 00\frac{1}{2}\}'$ , $\{C_3^+ 000\}'$ , $\{C_2 00\frac{1}{2}\}'$ , $\{C_3^- 000\}'$ , $\{C_6^- 00\frac{1}{2}\}'$ , $\{C'_{21} 000\}'$ , $\{C'_{22} 000\}'$ , $\{C'_{23} 000\}'$ , $\{C''_{21} 00\frac{1}{2}\}'$ , $\{C''_{22} 00\frac{1}{2}\}'$ , $\{C''_{23} 00\frac{1}{2}\}'$                                                                                 |
| 182.181 | $P6'_32'2$ | $\{E 000\}$ , $\{C_6^+ 00\frac{1}{2}\}'$ , $\{C_3^+ 000\}$ , $\{C_2 00\frac{1}{2}\}'$ , $\{C_3^- 000\}$ , $\{C_6^- 00\frac{1}{2}\}'$ , $\{C'_{21} 000\}$ , $\{C'_{22} 000\}$ , $\{C'_{23} 000\}$ , $\{C''_{21} 00\frac{1}{2}\}'$ , $\{C''_{22} 00\frac{1}{2}\}'$ , $\{C''_{23} 00\frac{1}{2}\}'$                                                                                                                                                                                                                                                                                                                                                                                    |
| 182.182 | $P6'_322'$ | $\{E 000\}$ , $\{C_6^+ 00\frac{1}{2}\}'$ , $\{C_3^+ 000\}$ , $\{C_2 00\frac{1}{2}\}'$ , $\{C_3^- 000\}$ , $\{C_6^- 00\frac{1}{2}\}'$ , $\{C'_{21} 000\}'$ , $\{C'_{22} 000\}'$ , $\{C'_{23} 000\}'$ , $\{C''_{21} 00\frac{1}{2}\}$ , $\{C''_{22} 00\frac{1}{2}\}$ , $\{C''_{23} 00\frac{1}{2}\}$                                                                                                                                                                                                                                                                                                                                                                                    |
| 182.183 | $P6_32'2'$ | $\{E 000\}$ , $\{C_6^+ 00\frac{1}{2}\}$ , $\{C_3^+ 000\}$ , $\{C_2 00\frac{1}{2}\}$ , $\{C_3^- 000\}$ , $\{C_6^- 00\frac{1}{2}\}$ , $\{C'_{21} 000\}'$ , $\{C'_{22} 000\}'$ , $\{C'_{23} 000\}'$ , $\{C''_{21} 00\frac{1}{2}\}'$ , $\{C''_{22} 00\frac{1}{2}\}'$ , $\{C''_{23} 00\frac{1}{2}\}'$                                                                                                                                                                                                                                                                                                                                                                                    |
| 182.184 | $P_c6_322$ | $\{E 000\}$ , $\{C_6^+ 00\frac{1}{2}\}$ , $\{C_3^+ 000\}$ , $\{C_2 00\frac{1}{2}\}$ , $\{C_3^- 000\}$ , $\{C_6^- 00\frac{1}{2}\}$ , $\{C'_{21} 000\}$ , $\{C'_{22} 000\}$ , $\{C'_{23} 000\}$ , $\{C''_{21} 00\frac{1}{2}\}$ , $\{C''_{22} 00\frac{1}{2}\}$ , $\{C''_{23} 00\frac{1}{2}\}$ , $\{E 00\frac{1}{2}\}'$ , $\{C_6^+ 000\}'$ , $\{C_3^+ 00\frac{1}{2}\}'$ , $\{C_2 000\}'$ , $\{C_3^- 00\frac{1}{2}\}'$ , $\{C_6^- 000\}'$ , $\{C'_{21} 00\frac{1}{2}\}'$ , $\{C'_{22} 00\frac{1}{2}\}'$ , $\{C'_{23} 00\frac{1}{2}\}'$ , $\{C''_{21} 000\}'$ , $\{C''_{22} 000\}'$ , $\{C''_{23} 000\}'$                                                                                 |
| 183.185 | $P6mm$     | $\{E 000\}$ , $\{C_6^+ 000\}$ , $\{C_3^+ 000\}$ , $\{C_2 000\}$ , $\{C_3^- 000\}$ , $\{C_6^- 000\}$ , $\{\sigma_{d1} 000\}$ , $\{\sigma_{d2} 000\}$ , $\{\sigma_{d3} 000\}$ , $\{\sigma_{v1} 000\}$ , $\{\sigma_{v2} 000\}$ , $\{\sigma_{v3} 000\}$                                                                                                                                                                                                                                                                                                                                                                                                                                 |
| 183.186 | $P6mm1'$   | $\{E 000\}$ , $\{C_6^+ 000\}$ , $\{C_3^+ 000\}$ , $\{C_2 000\}$ , $\{C_3^- 000\}$ , $\{C_6^- 000\}$ , $\{\sigma_{d1} 000\}$ , $\{\sigma_{d2} 000\}$ , $\{\sigma_{d3} 000\}$ , $\{\sigma_{v1} 000\}$ , $\{\sigma_{v2} 000\}$ , $\{\sigma_{v3} 000\}$ , $\{E 000\}'$ , $\{C_6^+ 000\}'$ , $\{C_3^+ 000\}'$ , $\{C_2 000\}'$ , $\{C_3^- 000\}'$ , $\{C_6^- 000\}'$ , $\{\sigma_{d1} 000\}'$ , $\{\sigma_{d2} 000\}'$ , $\{\sigma_{d3} 000\}'$ , $\{\sigma_{v1} 000\}'$ , $\{\sigma_{v2} 000\}'$ , $\{\sigma_{v3} 000\}'$                                                                                                                                                               |
| 183.187 | $P6'm'm$   | $\{E 000\}$ , $\{C_6^+ 000\}'$ , $\{C_3^+ 000\}$ , $\{C_2 000\}'$ , $\{C_3^- 000\}$ , $\{C_6^- 000\}'$ , $\{\sigma_{d1} 000\}$ , $\{\sigma_{d2} 000\}$ , $\{\sigma_{d3} 000\}$ , $\{\sigma_{v1} 000\}'$ , $\{\sigma_{v2} 000\}'$ , $\{\sigma_{v3} 000\}'$                                                                                                                                                                                                                                                                                                                                                                                                                           |
| 183.188 | $P6'mm'$   | $\{E 000\}$ , $\{C_6^+ 000\}'$ , $\{C_3^+ 000\}$ , $\{C_2 000\}'$ , $\{C_3^- 000\}$ , $\{C_6^- 000\}'$ , $\{\sigma_{d1} 000\}'$ , $\{\sigma_{d2} 000\}'$ , $\{\sigma_{d3} 000\}'$ , $\{\sigma_{v1} 000\}$ , $\{\sigma_{v2} 000\}$ , $\{\sigma_{v3} 000\}$                                                                                                                                                                                                                                                                                                                                                                                                                           |
| 183.189 | $P6m'm'$   | $\{E 000\}$ , $\{C_6^+ 000\}$ , $\{C_3^+ 000\}$ , $\{C_2 000\}$ , $\{C_3^- 000\}$ , $\{C_6^- 000\}$ , $\{\sigma_{d1} 000\}'$ , $\{\sigma_{d2} 000\}'$ , $\{\sigma_{d3} 000\}'$ , $\{\sigma_{v1} 000\}'$ , $\{\sigma_{v2} 000\}'$ , $\{\sigma_{v3} 000\}'$                                                                                                                                                                                                                                                                                                                                                                                                                           |

[illegible]

[illegible]

| No.     | Symbol         | Elements                                                                                                                                                                                                                                                                                                                                                                                                                                                                                                                                                                                                                                                                                                                                                                                                                                                                                       |
|---------|----------------|------------------------------------------------------------------------------------------------------------------------------------------------------------------------------------------------------------------------------------------------------------------------------------------------------------------------------------------------------------------------------------------------------------------------------------------------------------------------------------------------------------------------------------------------------------------------------------------------------------------------------------------------------------------------------------------------------------------------------------------------------------------------------------------------------------------------------------------------------------------------------------------------|
| 189.226 | $P_c\bar{6}2m$ | $\{E 000\}, \{C_3^+ 000\}, \{C_3^- 000\}, \{C_{21}' 000\}, \{C_{22}' 000\}, \{C_{23}' 000\}, \{S_3^- 000\}, \{\sigma_h 000\}$ ,<br>$\{S_3^+ 000\}, \{\sigma_{d1} 000\}, \{\sigma_{d2} 000\}, \{\sigma_{d3} 000\}, \{E 00\frac{1}{2}\}', \{C_3^+ 00\frac{1}{2}\}', \{C_3^- 00\frac{1}{2}\}', \{C_{21}' 00\frac{1}{2}\}'$ ,<br>$\{C_{22}' 00\frac{1}{2}\}', \{C_{23}' 00\frac{1}{2}\}', \{S_3^- 00\frac{1}{2}\}', \{\sigma_h 00\frac{1}{2}\}', \{S_3^+ 00\frac{1}{2}\}', \{\sigma_{d1} 00\frac{1}{2}\}', \{\sigma_{d2} 00\frac{1}{2}\}', \{\sigma_{d3} 00\frac{1}{2}\}'$                                                                                                                                                                                                                                                                                                                         |
| 190.227 | $P\bar{6}2c$   | $\{E 000\}, \{C_3^+ 000\}, \{C_3^- 000\}, \{C_{21}' 00\frac{1}{2}\}, \{C_{22}' 00\frac{1}{2}\}, \{C_{23}' 00\frac{1}{2}\}, \{S_3^- 000\}, \{\sigma_h 000\}$ ,<br>$\{S_3^+ 000\}, \{\sigma_{d1} 00\frac{1}{2}\}, \{\sigma_{d2} 00\frac{1}{2}\}, \{\sigma_{d3} 00\frac{1}{2}\}$                                                                                                                                                                                                                                                                                                                                                                                                                                                                                                                                                                                                                  |
| 190.228 | $P\bar{6}2c1'$ | $\{E 000\}, \{C_3^+ 000\}, \{C_3^- 000\}, \{C_{21}' 00\frac{1}{2}\}, \{C_{22}' 00\frac{1}{2}\}, \{C_{23}' 00\frac{1}{2}\}, \{S_3^- 000\}, \{\sigma_h 000\}$ ,<br>$\{S_3^+ 000\}, \{\sigma_{d1} 00\frac{1}{2}\}, \{\sigma_{d2} 00\frac{1}{2}\}, \{\sigma_{d3} 00\frac{1}{2}\}, \{E 000\}', \{C_3^+ 000\}', \{C_3^- 000\}', \{C_{21}' 00\frac{1}{2}}'\,$<br>$\{C_{22}' 00\frac{1}{2}}'\,, \{C_{23}' 00\frac{1}{2}}'\,, \{S_3^- 000\}', \{\sigma_h 000\}', \{S_3^+ 000\}', \{\sigma_{d1} 00\frac{1}{2}}'\,, \{\sigma_{d2} 00\frac{1}{2}}'\,, \{\sigma_{d3} 00\frac{1}{2}}'\)$                                                                                                                                                                                                                                                                                                                     |
| 190.229 | $P\bar{6}2'c$  | $\{E 000\}, \{C_3^+ 000\}, \{C_3^- 000\}, \{C_{21}' 00\frac{1}{2}\}', \{C_{22}' 00\frac{1}{2}\}', \{C_{23}' 00\frac{1}{2}\}', \{S_3^- 000\}', \{\sigma_h 000\}'$ ,<br>$\{S_3^+ 000\}', \{\sigma_{d1} 00\frac{1}{2}\}, \{\sigma_{d2} 00\frac{1}{2}\}, \{\sigma_{d3} 00\frac{1}{2}\}$                                                                                                                                                                                                                                                                                                                                                                                                                                                                                                                                                                                                            |
| 190.230 | $P\bar{6}2'c'$ | $\{E 000\}, \{C_3^+ 000\}, \{C_3^- 000\}, \{C_{21}' 00\frac{1}{2}\}, \{C_{22}' 00\frac{1}{2}\}, \{C_{23}' 00\frac{1}{2}\}, \{S_3^- 000\}', \{\sigma_h 000\}'$ ,<br>$\{S_3^+ 000\}', \{\sigma_{d1} 00\frac{1}{2}\}', \{\sigma_{d2} 00\frac{1}{2}\}', \{\sigma_{d3} 00\frac{1}{2}\}'$                                                                                                                                                                                                                                                                                                                                                                                                                                                                                                                                                                                                            |
| 190.231 | $P\bar{6}2'c'$ | $\{E 000\}, \{C_3^+ 000\}, \{C_3^- 000\}, \{C_{21}' 00\frac{1}{2}\}', \{C_{22}' 00\frac{1}{2}\}', \{C_{23}' 00\frac{1}{2}\}', \{S_3^- 000\}, \{\sigma_h 000\}$ ,<br>$\{S_3^+ 000\}, \{\sigma_{d1} 00\frac{1}{2}\}', \{\sigma_{d2} 00\frac{1}{2}\}', \{\sigma_{d3} 00\frac{1}{2}\}'$                                                                                                                                                                                                                                                                                                                                                                                                                                                                                                                                                                                                            |
| 190.232 | $P_c\bar{6}2c$ | $\{E 000\}, \{C_3^+ 000\}, \{C_3^- 000\}, \{C_{21}' 00\frac{1}{2}\}, \{C_{22}' 00\frac{1}{2}\}, \{C_{23}' 00\frac{1}{2}\}, \{S_3^- 000\}, \{\sigma_h 000\}$ ,<br>$\{S_3^+ 000\}, \{\sigma_{d1} 00\frac{1}{2}\}, \{\sigma_{d2} 00\frac{1}{2}\}, \{\sigma_{d3} 00\frac{1}{2}\}, \{E 00\frac{1}{2}\}', \{C_3^+ 00\frac{1}{2}\}', \{C_3^- 00\frac{1}{2}\}', \{C_{21}' 000\}'$ ,<br>$\{C_{22}' 000\}', \{C_{23}' 000\}', \{S_3^- 00\frac{1}{2}\}', \{\sigma_h 00\frac{1}{2}\}', \{S_3^+ 00\frac{1}{2}\}', \{\sigma_{d1} 000\}', \{\sigma_{d2} 000\}', \{\sigma_{d3} 000\}'$                                                                                                                                                                                                                                                                                                                         |
| 191.233 | $P6/mmm$       | $\{E 000\}, \{I 000\}, \{C_6^+ 000\}, \{C_3^+ 000\}, \{C_2 000\}, \{C_3^- 000\}, \{C_6^- 000\}, \{C_{21}' 000\}, \{C_{22}' 000\}$ ,<br>$\{C_{23}' 000\}, \{C_{21}'' 000\}, \{C_{22}'' 000\}, \{C_{23}'' 000\}, \{S_3^- 000\}, \{S_6^- 000\}, \{\sigma_h 000\}, \{S_6^+ 000\}$ ,<br>$\{S_3^+ 000\}, \{\sigma_{d1} 000\}, \{\sigma_{d2} 000\}, \{\sigma_{d3} 000\}, \{\sigma_{v1} 000\}, \{\sigma_{v2} 000\}, \{\sigma_{v3} 000\}$                                                                                                                                                                                                                                                                                                                                                                                                                                                               |
| 191.234 | $P6'/mmm1'$    | $\{E 000\}, \{I 000\}, \{C_6^+ 000\}, \{C_3^+ 000\}, \{C_2 000\}, \{C_3^- 000\}, \{C_6^- 000\}, \{C_{21}' 000\}, \{C_{22}' 000\}$ ,<br>$\{C_{23}' 000\}, \{C_{21}'' 000\}, \{C_{22}'' 000\}, \{C_{23}'' 000\}, \{S_3^- 000\}, \{S_6^- 000\}, \{\sigma_h 000\}, \{S_6^+ 000\}$ ,<br>$\{S_3^+ 000\}, \{\sigma_{d1} 000\}, \{\sigma_{d2} 000\}, \{\sigma_{d3} 000\}, \{\sigma_{v1} 000\}, \{\sigma_{v2} 000\}, \{\sigma_{v3} 000\}, \{E 000\}'$ ,<br>$\{I 000\}', \{C_6^+ 000\}', \{C_3^+ 000\}', \{C_2 000\}', \{C_3^- 000\}', \{C_6^- 000\}', \{C_{21}' 000\}', \{C_{22}' 000\}'$ ,<br>$\{C_{23}' 000\}', \{C_{21}'' 000\}', \{C_{22}'' 000\}', \{C_{23}'' 000\}', \{S_3^- 000\}', \{S_6^- 000\}', \{\sigma_h 000\}', \{S_6^+ 000\}'$ ,<br>$\{S_3^+ 000\}', \{\sigma_{d1} 000\}', \{\sigma_{d2} 000\}', \{\sigma_{d3} 000\}', \{\sigma_{v1} 000\}', \{\sigma_{v2} 000\}', \{\sigma_{v3} 000\}'$ |
| 191.235 | $P6/m'mm$      | $\{E 000\}, \{I 000\}', \{C_6^+ 000\}, \{C_3^+ 000\}, \{C_2 000\}, \{C_3^- 000\}, \{C_6^- 000\}, \{C_{21}' 000\}'$ ,<br>$\{C_{22}' 000\}', \{C_{23}' 000\}', \{C_{21}'' 000\}', \{C_{22}'' 000\}', \{C_{23}'' 000\}', \{S_3^- 000\}', \{S_6^- 000\}', \{\sigma_h 000\}'$ ,<br>$\{S_6^+ 000\}', \{S_3^+ 000\}', \{\sigma_{d1} 000\}, \{\sigma_{d2} 000\}, \{\sigma_{d3} 000\}, \{\sigma_{v1} 000\}, \{\sigma_{v2} 000\}, \{\sigma_{v3} 000\}$                                                                                                                                                                                                                                                                                                                                                                                                                                                   |
| 191.236 | $P6'/mm'm$     | $\{E 000\}, \{I 000\}', \{C_6^+ 000\}', \{C_3^+ 000\}, \{C_2 000\}', \{C_3^- 000\}, \{C_6^- 000\}', \{C_{21}' 000\}'$ ,<br>$\{C_{22}' 000\}', \{C_{23}' 000\}', \{C_{21}'' 000\}, \{C_{22}'' 000\}, \{C_{23}'' 000\}, \{S_3^- 000\}, \{S_6^- 000\}', \{\sigma_h 000\}$ ,<br>$\{S_6^+ 000\}', \{S_3^+ 000\}, \{\sigma_{d1} 000\}, \{\sigma_{d2} 000\}, \{\sigma_{d3} 000\}, \{\sigma_{v1} 000\}', \{\sigma_{v2} 000\}', \{\sigma_{v3} 000\}'$                                                                                                                                                                                                                                                                                                                                                                                                                                                   |
| 191.237 | $P6'/mmm'$     | $\{E 000\}, \{I 000\}', \{C_6^+ 000\}', \{C_3^+ 000\}, \{C_2 000\}', \{C_3^- 000\}, \{C_6^- 000\}', \{C_{21}' 000\}$ ,<br>$\{C_{22}' 000\}, \{C_{23}' 000\}, \{C_{21}'' 000\}', \{C_{22}'' 000\}', \{C_{23}'' 000\}', \{S_3^- 000\}, \{S_6^- 000\}', \{\$                                                                                                                                                                                                                                                                                                                                                                                                                                                                                                                                                                                                                                      |

[illegible]

[illegible]

[illegible]



[illegible]



[illegible]

[illegible]

[illegible]

[illegible]

[illegible]

[illegible]

| No.    | Symbol         | Elements                                                                                                                                                                                                                                                                                                                                                                                                                                                                                                                                                                                                                                                                                                                                                                                                                                                                                                                                                                                                                                                                                                                                                                                                                                                                                                                                                                                                                                                                                                                                                                                                                                                                                                                 |
|--------|----------------|--------------------------------------------------------------------------------------------------------------------------------------------------------------------------------------------------------------------------------------------------------------------------------------------------------------------------------------------------------------------------------------------------------------------------------------------------------------------------------------------------------------------------------------------------------------------------------------------------------------------------------------------------------------------------------------------------------------------------------------------------------------------------------------------------------------------------------------------------------------------------------------------------------------------------------------------------------------------------------------------------------------------------------------------------------------------------------------------------------------------------------------------------------------------------------------------------------------------------------------------------------------------------------------------------------------------------------------------------------------------------------------------------------------------------------------------------------------------------------------------------------------------------------------------------------------------------------------------------------------------------------------------------------------------------------------------------------------------------|
| 214.68 | $I4_1321'$     | $\{E 000\}, \{C_{2x} \frac{1}{2}\frac{1}{2}0\}, \{C_{2y} 0\frac{1}{2}\frac{1}{2}\}, \{C_{2z} \frac{1}{2}0\frac{1}{2}\}, \{C_{31}^+ 000\}, \{C_{32}^+ 0\frac{1}{2}\frac{1}{2}\}, \{C_{33}^+ \frac{1}{2}0\frac{1}{2}\}, \{C_{34}^+ \frac{1}{2}\frac{1}{2}0\},$<br>$\{C_{31}^- 000\}, \{C_{32}^- \frac{1}{2}\frac{1}{2}0\}, \{C_{33}^- 0\frac{1}{2}\frac{1}{2}\}, \{C_{34}^- \frac{1}{2}0\frac{1}{2}\}, \{C_{4x}^+ 00\frac{1}{2}\}, \{C_{4y}^+ \frac{1}{2}00\}, \{C_{4z}^+ 0\frac{1}{2}0\}, \{C_{4x}^- \frac{1}{2}00\},$<br>$\{C_{4y}^- 0\frac{1}{2}0\}, \{C_{4z}^- 00\frac{1}{2}\}, \{C_{2a} \frac{1}{2}00\}, \{C_{2b} \frac{1}{2}\frac{1}{2}\frac{1}{2}\}, \{C_{2c} 00\frac{1}{2}\}, \{C_{2d} 0\frac{1}{2}0\}, \{C_{2e} \frac{1}{2}\frac{1}{2}\frac{1}{2}\}, \{C_{2f} \frac{1}{2}\frac{1}{2}\frac{1}{2}\},$<br>$\{E 000\}', \{C_{2x} \frac{1}{2}\frac{1}{2}0\}', \{C_{2y} 0\frac{1}{2}\frac{1}{2}\}', \{C_{2z} \frac{1}{2}0\frac{1}{2}\}', \{C_{31}^+ 000\}', \{C_{32}^+ 0\frac{1}{2}\frac{1}{2}\}', \{C_{33}^+ \frac{1}{2}0\frac{1}{2}\}', \{C_{34}^+ \frac{1}{2}\frac{1}{2}0\}',$<br>$\{C_{31}^- \frac{1}{2}\frac{1}{2}0\}', \{C_{31}^- 000\}', \{C_{32}^- \frac{1}{2}\frac{1}{2}0\}', \{C_{33}^- 0\frac{1}{2}\frac{1}{2}\}', \{C_{34}^- \frac{1}{2}0\frac{1}{2}\}', \{C_{4x}^+ 00\frac{1}{2}\}', \{C_{4y}^+ \frac{1}{2}00\}', \{C_{4z}^+ 0\frac{1}{2}0\}',$<br>$\{C_{4x}^- 0\frac{1}{2}0\}', \{C_{4x}^- \frac{1}{2}00\}', \{C_{4y}^- 0\frac{1}{2}0\}', \{C_{4z}^- 00\frac{1}{2}\}', \{C_{2a} \frac{1}{2}00\}', \{C_{2b} \frac{1}{2}\frac{1}{2}\frac{1}{2}\}', \{C_{2c} 00\frac{1}{2}\}',$<br>$\{C_{2d} 0\frac{1}{2}0\}', \{C_{2e} \frac{1}{2}\frac{1}{2}\frac{1}{2}\}', \{C_{2f} \frac{1}{2}\frac{1}{2}\frac{1}{2}\}'$ |
| 214.69 | $I4_1'32'$     | $\{E 000\}, \{C_{2x} \frac{1}{2}\frac{1}{2}0\}, \{C_{2y} 0\frac{1}{2}\frac{1}{2}\}, \{C_{2z} \frac{1}{2}0\frac{1}{2}\}, \{C_{31}^+ 000\}, \{C_{32}^+ 0\frac{1}{2}\frac{1}{2}\}, \{C_{33}^+ \frac{1}{2}0\frac{1}{2}\}, \{C_{34}^+ \frac{1}{2}\frac{1}{2}0\},$<br>$\{C_{31}^- 000\}, \{C_{32}^- \frac{1}{2}\frac{1}{2}0\}, \{C_{33}^- 0\frac{1}{2}\frac{1}{2}\}, \{C_{34}^- \frac{1}{2}0\frac{1}{2}\}, \{C_{4x}^+ 00\frac{1}{2}\}', \{C_{4y}^+ \frac{1}{2}00\}', \{C_{4z}^+ 0\frac{1}{2}0\}',$<br>$\{C_{4x}^- \frac{1}{2}00\}', \{C_{4y}^- 0\frac{1}{2}0\}', \{C_{4z}^- 00\frac{1}{2}\}', \{C_{2a} \frac{1}{2}00\}', \{C_{2b} \frac{1}{2}\frac{1}{2}\frac{1}{2}\}', \{C_{2c} 00\frac{1}{2}\}', \{C_{2d} 0\frac{1}{2}0\}',$<br>$\{C_{2e} \frac{1}{2}\frac{1}{2}\frac{1}{2}\}', \{C_{2f} \frac{1}{2}\frac{1}{2}\frac{1}{2}\}'$                                                                                                                                                                                                                                                                                                                                                                                                                                                                                                                                                                                                                                                                                                                                                                                                                                                                                               |
| 215.70 | $P\bar{4}3m$   | $\{E 000\}, \{C_{2x} 000\}, \{C_{2y} 000\}, \{C_{2z} 000\}, \{C_{31}^+ 000\}, \{C_{32}^+ 000\}, \{C_{33}^+ 000\}, \{C_{34}^+ 000\},$<br>$\{C_{31}^- 000\}, \{C_{32}^- 000\}, \{C_{33}^- 000\}, \{C_{34}^- 000\}, \{S_{4x}^+ 000\}, \{S_{4y}^+ 000\}, \{S_{4z}^+ 000\}, \{S_{4x}^- 000\},$<br>$\{S_{4y}^+ 000\}, \{S_{4z}^+ 000\}, \{\sigma_{da} 000\}, \{\sigma_{db} 000\}, \{\sigma_{dc} 000\}, \{\sigma_{dd} 000\}, \{\sigma_{de} 000\}, \{\sigma_{df} 000\}$                                                                                                                                                                                                                                                                                                                                                                                                                                                                                                                                                                                                                                                                                                                                                                                                                                                                                                                                                                                                                                                                                                                                                                                                                                                          |
| 215.71 | $P\bar{4}3m1'$ | $\{E 000\}, \{C_{2x} 000\}, \{C_{2y} 000\}, \{C_{2z} 000\}, \{C_{31}^+ 000\}, \{C_{32}^+ 000\}, \{C_{33}^+ 000\}, \{C_{34}^+ 000\},$<br>$\{C_{31}^- 000\}, \{C_{32}^- 000\}, \{C_{33}^- 000\}, \{C_{34}^- 000\}, \{S_{4x}^+ 000\}, \{S_{4y}^+ 000\}, \{S_{4z}^+ 000\}, \{S_{4x}^- 000\},$<br>$\{S_{4y}^+ 000\}, \{S_{4z}^+ 000\}, \{\sigma_{da} 000\}, \{\sigma_{db} 000\}, \{\sigma_{dc} 000\}, \{\sigma_{dd} 000\}, \{\sigma_{de} 000\}, \{\sigma_{df} 000\},$<br>$\{E 000\}', \{C_{2x} 000\}', \{C_{2y} 000\}', \{C_{2z} 000\}', \{C_{31}^+ 000\}', \{C_{32}^+ 000\}', \{C_{33}^+ 000\}', \{C_{34}^+ 000\}',$<br>$\{C_{31}^- 000\}', \{C_{32}^- 000\}', \{C_{33}^- 000\}', \{C_{34}^- 000\}', \{S_{4x}^+ 000\}', \{S_{4y}^+ 000\}', \{S_{4z}^+ 000\}', \{S_{4x}^- 000\}',$<br>$\{S_{4y}^+ 000\}', \{S_{4z}^+ 000\}', \{\sigma_{da} 000\}', \{\sigma_{db} 000\}', \{\sigma_{dc} 000\}', \{\sigma_{dd} 000\}', \{\sigma_{de} 000\}', \{\sigma_{df} 000\}'$                                                                                                                                                                                                                                                                                                                                                                                                                                                                                                                                                                                                                                                                                                                                                              |
| 215.72 | $P\bar{4}'3m'$ | $\{E 000\}, \{C_{2x} 000\}, \{C_{2y} 000\}, \{C_{2z} 000\}, \{C_{31}^+ 000\}, \{C_{32}^+ 000\}, \{C_{33}^+ 000\}, \{C_{34}^+ 000\},$<br>$\{C_{31}^- 000\}, \{C_{32}^- 000\}, \{C_{33}^- 000\}, \{C_{34}^- 000\}, \{S_{4x}^+ 000\}', \{S_{4y}^+ 000\}', \{S_{4z}^+ 000\}', \{S_{4x}^- 000\}',$<br>$\{S_{4y}^+ 000\}', \{S_{4z}^+ 000\}', \{\sigma_{da} 000\}', \{\sigma_{db} 000\}', \{\sigma_{dc} 000\}', \{\sigma_{dd} 000\}', \{\sigma_{de} 000\}', \{\sigma_{df} 000\}'$                                                                                                                                                                                                                                                                                                                                                                                                                                                                                                                                                                                                                                                                                                                                                                                                                                                                                                                                                                                                                                                                                                                                                                                                                                              |
| 215.73 | $P_I\bar{4}3m$ | $\{E 000\}, \{C_{2x} 000\}, \{C_{2y} 000\}, \{C_{2z} 000\}, \{C_{31}^+ 000\}, \{C_{32}^+ 000\}, \{C_{33}^+ 000\}, \{C_{34}^+ 000\},$<br>$\{C_{31}^- 000\}, \{C_{32}^- 000\}, \{C_{33}^- 000\}, \{C_{34}^- 000\}, \{S_{4x}^+ 000\}, \{S_{4y}^+ 000\}, \{S_{4z}^+ 000\}, \{S_{4x}^- 000\},$<br>$\{S_{4y}^+ 000\}, \{S_{4z}^+ 000\}, \{\sigma_{da} 000\}, \{\sigma_{db} 000\}, \{\sigma_{dc} 000\}, \{\sigma_{dd} 000\}, \{\sigma_{de} 000\}, \{\sigma_{df} 000\},$<br>$\{E \frac{1}{2}\frac{1}{2}\frac{1}{2}\}', \{C_{2x} \frac{1}{2}\frac{1}{2}\frac{1}{2}\}', \{C_{2y} \frac{1}{2}\frac{1}{2}\frac{1}{2}\}', \{C_{2z} \frac{1}{2}\frac{1}{2}\frac{1}{2}\}', \{C_{31}^+ \frac{1}{2}\frac{1}{2}\frac{1}{2}\}', \{C_{32}^+ \frac{1}{2}\frac{1}{2}\frac{1}{2}\}', \{C_{33}^+ \frac{1}{2}\frac{1}{2}\frac{1}{2}\}',$<br>$\{C_{34}^+ \frac{1}{2}\frac{1}{2}\frac{1}{2}\}', \{C_{31}^- \frac{1}{2}\frac{1}{2}\frac{1}{2}\}', \{C_{32}^- \frac{1}{2}\frac{1}{2}\frac{1}{2}\}', \{C_{33}^- \frac{1}{2}\frac{1}{2}\frac{1}{2}\}', \{C_{34}^- \frac{1}{2}\frac{1}{2}\frac{1}{2}\}', \{S_{4x}^+ \frac{1}{2}\frac{1}{2}\frac{1}{2}\}', \{S_{4y}^+ \frac{1}{2}\frac{1}{2}\frac{1}{2}\}',$<br>$\{S_{4z}^+ \frac{1}{2}\frac{1}{2}\frac{1}{2}\}', \{S_{4x}^- \frac{1}{2}\frac{1}{2}\frac{1}{2}\}', \{S_{4y}^+ \frac{1}{2}\frac{1}{2}\frac{1$                                                                                                                                                                                                                                                                                                                                                                                              |

[illegible]



[illegible]

[illegible]

[illegible]

[illegible]

[illegible]

[illegible]

[illegible]

[illegible]



[illegible]

[illegible]

[illegible]

[illegible]

| No.     | Symbol          | Elements                                                                                                                                                                                                                                                                                                                                                                                                                                                                                                                                                                                                                                                                                                                                                                                                                                                                                                                                                                                                                                                                                                                                                                                                                                                                                                                                                                                                                                                                                                                                                                                                                                                                                                                                                                                                                                                                                                                                                                                                                                                                                                                                                                                                                                                                                                                                                                                                                                                                                                                                                                                                                                                                                                                                                                                                                                                                                                                                                                                                                                                                                                                                                                                                                                                                                                                                                                                                                                             |
|---------|-----------------|------------------------------------------------------------------------------------------------------------------------------------------------------------------------------------------------------------------------------------------------------------------------------------------------------------------------------------------------------------------------------------------------------------------------------------------------------------------------------------------------------------------------------------------------------------------------------------------------------------------------------------------------------------------------------------------------------------------------------------------------------------------------------------------------------------------------------------------------------------------------------------------------------------------------------------------------------------------------------------------------------------------------------------------------------------------------------------------------------------------------------------------------------------------------------------------------------------------------------------------------------------------------------------------------------------------------------------------------------------------------------------------------------------------------------------------------------------------------------------------------------------------------------------------------------------------------------------------------------------------------------------------------------------------------------------------------------------------------------------------------------------------------------------------------------------------------------------------------------------------------------------------------------------------------------------------------------------------------------------------------------------------------------------------------------------------------------------------------------------------------------------------------------------------------------------------------------------------------------------------------------------------------------------------------------------------------------------------------------------------------------------------------------------------------------------------------------------------------------------------------------------------------------------------------------------------------------------------------------------------------------------------------------------------------------------------------------------------------------------------------------------------------------------------------------------------------------------------------------------------------------------------------------------------------------------------------------------------------------------------------------------------------------------------------------------------------------------------------------------------------------------------------------------------------------------------------------------------------------------------------------------------------------------------------------------------------------------------------------------------------------------------------------------------------------------------------------|
| 229.144 | $Im'\bar{3}'m'$ | $\{E 000\}, \{C_{2x} 000\}, \{C_{2y} 000\}, \{C_{2z} 000\}, \{C_{31}^+ 000\}, \{C_{32}^+ 000\}, \{C_{33}^+ 000\}, \{C_{34}^+ 000\},$<br>$\{C_{31}^- 000\}, \{C_{32}^- 000\}, \{C_{33}^- 000\}, \{C_{34}^- 000\}, \{C_{4x}^+ 000\}, \{C_{4y}^+ 000\}, \{C_{4z}^+ 000\}, \{C_{4x}^- 000\},$<br>$\{C_{4y}^- 000\}, \{C_{4z}^- 000\}, \{C_{2a} 000\}, \{C_{2b} 000\}, \{C_{2c} 000\}, \{C_{2d} 000\}, \{C_{2e} 000\}, \{C_{2f} 000\},$<br>$\{I 000\}', \{\sigma_x 000\}', \{\sigma_y 000\}', \{\sigma_z 000\}', \{S_{61}^- 000\}', \{S_{62}^- 000\}', \{S_{63}^- 000\}', \{S_{64}^- 000\}',$<br>$\{S_{61}^+ 000\}', \{S_{62}^+ 000\}', \{S_{63}^+ 000\}', \{S_{64}^+ 000\}', \{S_{4x}^- 000\}', \{S_{4y}^- 000\}', \{S_{4z}^- 000\}', \{S_{4x}^+ 000\}',$<br>$\{S_{4y}^+ 000\}', \{S_{4z}^+ 000\}', \{\sigma_{da} 000\}', \{\sigma_{db} 000\}', \{\sigma_{dc} 000\}', \{\sigma_{dd} 000\}', \{\sigma_{de} 000\}', \{\sigma_{df} 000\}'$                                                                                                                                                                                                                                                                                                                                                                                                                                                                                                                                                                                                                                                                                                                                                                                                                                                                                                                                                                                                                                                                                                                                                                                                                                                                                                                                                                                                                                                                                                                                                                                                                                                                                                                                                                                                                                                                                                                                                                                                                                                                                                                                                                                                                                                                                                                                                                                                                                                                                                                  |
| 230.145 | $Ia\bar{3}d$    | $\{E 000\}, \{C_{2x} \frac{1}{2}\frac{1}{2}0\}, \{C_{2y} 0\frac{1}{2}\frac{1}{2}\}, \{C_{2z} \frac{1}{2}0\frac{1}{2}\}, \{C_{31}^+ 000\}, \{C_{32}^+ 0\frac{1}{2}\frac{1}{2}\}, \{C_{33}^+ \frac{1}{2}0\frac{1}{2}\}, \{C_{34}^+ \frac{1}{2}\frac{1}{2}0\},$<br>$\{C_{31}^- 000\}, \{C_{32}^- \frac{1}{2}\frac{1}{2}0\}, \{C_{33}^- 0\frac{1}{2}\frac{1}{2}\}, \{C_{34}^- \frac{1}{2}0\frac{1}{2}\}, \{C_{4x}^+ 00\frac{1}{2}\}, \{C_{4y}^+ \frac{1}{2}00\}, \{C_{4z}^+ 0\frac{1}{2}0\}, \{C_{4x}^- \frac{1}{2}00\},$<br>$\{C_{4y}^- 0\frac{1}{2}0\}, \{C_{4z}^- 00\frac{1}{2}\}, \{C_{2a} \frac{1}{2}00\}, \{C_{2b} \frac{1}{2}\frac{1}{2}\frac{1}{2}\}, \{C_{2c} 00\frac{1}{2}\}, \{C_{2d} 0\frac{1}{2}0\}, \{C_{2e} \frac{1}{2}\frac{1}{2}\frac{1}{2}\}, \{C_{2f} \frac{1}{2}\frac{1}{2}\frac{1}{2}\},$<br>$\{I 000\}, \{\sigma_x \frac{1}{2}\frac{1}{2}0\}, \{\sigma_y 0\frac{1}{2}\frac{1}{2}\}, \{\sigma_z \frac{1}{2}0\frac{1}{2}\}, \{S_{61}^- 000\}, \{S_{62}^- 0\frac{1}{2}\frac{1}{2}\}, \{S_{63}^- \frac{1}{2}0\frac{1}{2}\}, \{S_{64}^- \frac{1}{2}\frac{1}{2}0\},$<br>$\{S_{61}^+ 000\}, \{S_{62}^+ \frac{1}{2}\frac{1}{2}0\}, \{S_{63}^+ 0\frac{1}{2}\frac{1}{2}\}, \{S_{64}^+ \frac{1}{2}0\frac{1}{2}\}, \{S_{4x}^- 00\frac{1}{2}\}, \{S_{4y}^- \frac{1}{2}00\}, \{S_{4z}^- 0\frac{1}{2}0\}, \{S_{4x}^+ \frac{1}{2}00\},$<br>$\{S_{4y}^+ 0\frac{1}{2}0\}, \{S_{4z}^+ 00\frac{1}{2}\}, \{\sigma_{da} \frac{1}{2}00\}, \{\sigma_{db} \frac{1}{2}\frac{1}{2}\frac{1}{2}\}, \{\sigma_{dc} 00\frac{1}{2}\}, \{\sigma_{dd} 0\frac{1}{2}0\}, \{\sigma_{de} \frac{1}{2}\frac{1}{2}\frac{1}{2}\}, \{\sigma_{df} \frac{1}{2}\frac{1}{2}\frac{1}{2}\}$                                                                                                                                                                                                                                                                                                                                                                                                                                                                                                                                                                                                                                                                                                                                                                                                                                                                                                                                                                                                                                                                                                                                                                                                                                                                                                                                                                                                                                                                                                                                                                                                                                                                                                                                                                                          |
| 230.146 | $Ia\bar{3}d1'$  | $\{E 000\}, \{C_{2x} \frac{1}{2}\frac{1}{2}0\}, \{C_{2y} 0\frac{1}{2}\frac{1}{2}\}, \{C_{2z} \frac{1}{2}0\frac{1}{2}\}, \{C_{31}^+ 000\}, \{C_{32}^+ 0\frac{1}{2}\frac{1}{2}\}, \{C_{33}^+ \frac{1}{2}0\frac{1}{2}\}, \{C_{34}^+ \frac{1}{2}\frac{1}{2}0\},$<br>$\{C_{31}^- 000\}, \{C_{32}^- \frac{1}{2}\frac{1}{2}0\}, \{C_{33}^- 0\frac{1}{2}\frac{1}{2}\}, \{C_{34}^- \frac{1}{2}0\frac{1}{2}\}, \{C_{4x}^+ 00\frac{1}{2}\}, \{C_{4y}^+ \frac{1}{2}00\}, \{C_{4z}^+ 0\frac{1}{2}0\}, \{C_{4x}^- \frac{1}{2}00\},$<br>$\{C_{4y}^- 0\frac{1}{2}0\}, \{C_{4z}^- 00\frac{1}{2}\}, \{C_{2a} \frac{1}{2}00\}, \{C_{2b} \frac{1}{2}\frac{1}{2}\frac{1}{2}\}, \{C_{2c} 00\frac{1}{2}\}, \{C_{2d} 0\frac{1}{2}0\}, \{C_{2e} \frac{1}{2}\frac{1}{2}\frac{1}{2}\}, \{C_{2f} \frac{1}{2}\frac{1}{2}\frac{1}{2}\},$<br>$\{I 000\}, \{\sigma_x \frac{1}{2}\frac{1}{2}0\}, \{\sigma_y 0\frac{1}{2}\frac{1}{2}\}, \{\sigma_z \frac{1}{2}0\frac{1}{2}\}, \{S_{61}^- 000\}, \{S_{62}^- 0\frac{1}{2}\frac{1}{2}\}, \{S_{63}^- \frac{1}{2}0\frac{1}{2}\}, \{S_{64}^- \frac{1}{2}\frac{1}{2}0\},$<br>$\{S_{61}^+ 000\}, \{S_{62}^+ \frac{1}{2}\frac{1}{2}0\}, \{S_{63}^+ 0\frac{1}{2}\frac{1}{2}\}, \{S_{64}^+ \frac{1}{2}0\frac{1}{2}\}, \{S_{4x}^- 00\frac{1}{2}\}, \{S_{4y}^- \frac{1}{2}00\}, \{S_{4z}^- 0\frac{1}{2}0\}, \{S_{4x}^+ \frac{1}{2}00\},$<br>$\{S_{4y}^+ 0\frac{1}{2}0\}, \{S_{4z}^+ 00\frac{1}{2}\}, \{\sigma_{da} \frac{1}{2}00\}, \{\sigma_{db} \frac{1}{2}\frac{1}{2}\frac{1}{2}\}, \{\sigma_{dc} 00\frac{1}{2}\}, \{\sigma_{dd} 0\frac{1}{2}0\}, \{\sigma_{de} \frac{1}{2}\frac{1}{2}\frac{1}{2}\}, \{\sigma_{df} \frac{1}{2}\frac{1}{2}\frac{1}{2}\},$<br>$\{E 000\}', \{C_{2x} \frac{1}{2}\frac{1}{2}0\}', \{C_{2y} 0\frac{1}{2}\frac{1}{2}\}', \{C_{2z} \frac{1}{2}0\frac{1}{2}\}', \{C_{31}^+ 000\}', \{C_{32}^+ 0\frac{1}{2}\frac{1}{2}\}', \{C_{33}^+ \frac{1}{2}0\frac{1}{2}\}', \{C_{34}^+ \frac{1}{2}\frac{1}{2}0\}',$<br>$\{C_{31}^- \frac{1}{2}\frac{1}{2}0\}', \{C_{31}^- 000\}', \{C_{32}^- \frac{1}{2}\frac{1}{2}0\}', \{C_{33}^- 0\frac{1}{2}\frac{1}{2}\}', \{C_{34}^- \frac{1}{2}0\frac{1}{2}\}', \{C_{4x}^+ 00\frac{1}{2}\}', \{C_{4y}^+ \frac{1}{2}00\}', \{C_{4z}^+ 0\frac{1}{2}0\}',$<br>$\{C_{4x}^- \frac{1}{2}00\}', \{C_{4x}^- 0\frac{1}{2}0\}', \{C_{4y}^- 0\frac{1}{2}0\}', \{C_{4z}^- 00\frac{1}{2}\}', \{C_{2a} \frac{1}{2}00\}', \{C_{2b} \frac{1}{2}\frac{1}{2}\frac{1}{2}\}', \{C_{2c} 00\frac{1}{2}\}',$<br>$\{C_{2d} 0\frac{1}{2}0\}', \{C_{2e} \frac{1}{2}\frac{1}{2}\frac{1}{2}\}', \{C_{2f} \frac{1}{2}\frac{1}{2}\frac{1}{2}\}', \{I 000\}', \{\sigma_x \frac{1}{2}\frac{1}{2}0\}', \{\sigma_y 0\frac{1}{2}\frac{1}{2}\}', \{\sigma_z \frac{1}{2}0\frac{1}{2}\}', \{S_{61}^- 000\}',$<br>$\{S_{62}^- 0\frac{1}{2}\frac{1}{2}\}', \{S_{63}^- \frac{1}{2}0\frac{1}{2}\}', \{S_{64}^- \frac{1}{2}\frac{1}{2}0\}', \{S_{61}^+ 000\}', \{S_{62}^+ \frac{1}{2}\frac{1}{2}0\}', \{S_{63}^+ 0\frac{1}{2}\frac{1}{2}\}', \{S_{64}^+ \frac{1}{2}0\frac{1}{2}\}',$<br>$\{S_{4x}^- 00\frac{1}{2}\}', \{S_{4y}^- \frac{1}{2}00\}', \{S_{4z}^- 0\frac{1}{2}0\}', \{S_{4x}^+ \frac{1}{2}00\}', \{S_{4y}^+ 0\frac{1}{2}0\}', \{S_{4z}^+ 00\frac{1}{2}\}', \{\sigma_{da} \frac{1}{2}00\}',$<br>$\{\sigma_{db} \frac{1}{2}\frac{1}{2}\frac{1}{2}\}', \{\sigma_{dc} 00\frac{1}{2}\}', \{\sigma_{dd} 0\frac{1}{2}0\}', \{\sigma_{de} \frac{1}{2}\frac{1}{2}\frac{1}{2}\}', \{\sigma_{df} \frac{1}{2}\frac{1}{2}\frac{1}{2}\}'$ |
| 230.147 | $Ia'\bar{3}'d$  | $\{E 000\}, \{C_{2x} \frac{1}{2}\frac{1}{2}0\}, \{C_{2y} 0\$                                                                                                                                                                                                                                                                                                                                                                                                                                                                                                                                                                                                                                                                                                                                                                                                                                                                                                                                                                                                                                                                                                                                                                                                                                                                                                                                                                                                                                                                                                                                                                                                                                                                                                                                                                                                                                                                                                                                                                                                                                                                                                                                                                                                                                                                                                                                                                                                                                                                                                                                                                                                                                                                                                                                                                                                                                                                                                                                                                                                                                                                                                                                                                                                                                                                                                                                                                                         |

230.149  $Ia'\bar{3}'d'$ 

$\{E|000\}$ ,  $\{C_{2x}|\frac{1}{2}\frac{1}{2}0\}$ ,  $\{C_{2y}|0\frac{1}{2}\frac{1}{2}\}$ ,  $\{C_{2z}|\frac{1}{2}0\frac{1}{2}\}$ ,  $\{C_{31}^+|000\}$ ,  $\{C_{32}^+|0\frac{1}{2}\frac{1}{2}\}$ ,  $\{C_{33}^+|\frac{1}{2}0\frac{1}{2}\}$ ,  $\{C_{34}^+|\frac{1}{2}\frac{1}{2}0\}$ ,  
 $\{C_{31}^-|000\}$ ,  $\{C_{32}^-|\frac{1}{2}\frac{1}{2}0\}$ ,  $\{C_{33}^-|0\frac{1}{2}\frac{1}{2}\}$ ,  $\{C_{34}^-|\frac{1}{2}0\frac{1}{2}\}$ ,  $\{C_{4x}^+|00\frac{1}{2}\}$ ,  $\{C_{4y}^+|\frac{1}{2}00\}$ ,  $\{C_{4z}^+|0\frac{1}{2}0\}$ ,  $\{C_{4x}^-|\frac{1}{2}00\}$ ,  
 $\{C_{4y}^-|0\frac{1}{2}0\}$ ,  $\{C_{4z}^-|00\frac{1}{2}\}$ ,  $\{C_{2a}|\frac{1}{2}00\}$ ,  $\{C_{2b}|\frac{1}{2}\frac{1}{2}\frac{1}{2}\}$ ,  $\{C_{2c}|00\frac{1}{2}\}$ ,  $\{C_{2d}|0\frac{1}{2}0\}$ ,  $\{C_{2e}|\frac{1}{2}\frac{1}{2}\frac{1}{2}\}$ ,  $\{C_{2f}|\frac{1}{2}\frac{1}{2}\frac{1}{2}\}$ ,  
 $\{I|000\}'$ ,  $\{\sigma_x|\frac{1}{2}\frac{1}{2}0\}'$ ,  $\{\sigma_y|0\frac{1}{2}\frac{1}{2}\}'$ ,  $\{\sigma_z|\frac{1}{2}0\frac{1}{2}\}'$ ,  $\{S_{61}^-|000\}'$ ,  $\{S_{62}^-|0\frac{1}{2}\frac{1}{2}\}'$ ,  $\{S_{63}^-|\frac{1}{2}0\frac{1}{2}\}'$ ,  $\{S_{64}^-|\frac{1}{2}\frac{1}{2}0\}'$ ,  
 $\{S_{61}^+|000\}'$ ,  $\{S_{62}^+|\frac{1}{2}\frac{1}{2}0\}'$ ,  $\{S_{63}^+|0\frac{1}{2}\frac{1}{2}\}'$ ,  $\{S_{64}^+|\frac{1}{2}0\frac{1}{2}\}'$ ,  $\{S_{4x}^-|00\frac{1}{2}\}'$ ,  $\{S_{4y}^-|\frac{1}{2}00\}'$ ,  $\{S_{4z}^-|0\frac{1}{2}0\}'$ ,  
 $\{S_{4x}^+|\frac{1}{2}00\}'$ ,  $\{S_{4y}^+|0\frac{1}{2}0\}'$ ,  $\{S_{4z}^+|00\frac{1}{2}\}'$ ,  $\{\sigma_{da}|\frac{1}{2}00\}'$ ,  $\{\sigma_{db}|\frac{1}{2}\frac{1}{2}\frac{1}{2}\}'$ ,  $\{\sigma_{dc}|00\frac{1}{2}\}'$ ,  $\{\sigma_{dd}|0\frac{1}{2}0\}'$ ,  
 $\{\sigma_{de}|\frac{1}{2}\frac{1}{2}\frac{1}{2}\}'$ ,  $\{\sigma_{df}|\frac{1}{2}\frac{1}{2}\frac{1}{2}\}'$
